# Supplementary material for: Physics at a 100 TeV pp collider: Higgs and EW symmetry breaking studies
Source: arXiv:1606.09408 source file (2016-06-30)
Supplement: Supplementary file 1 [file vbf_100TeV.pdf]

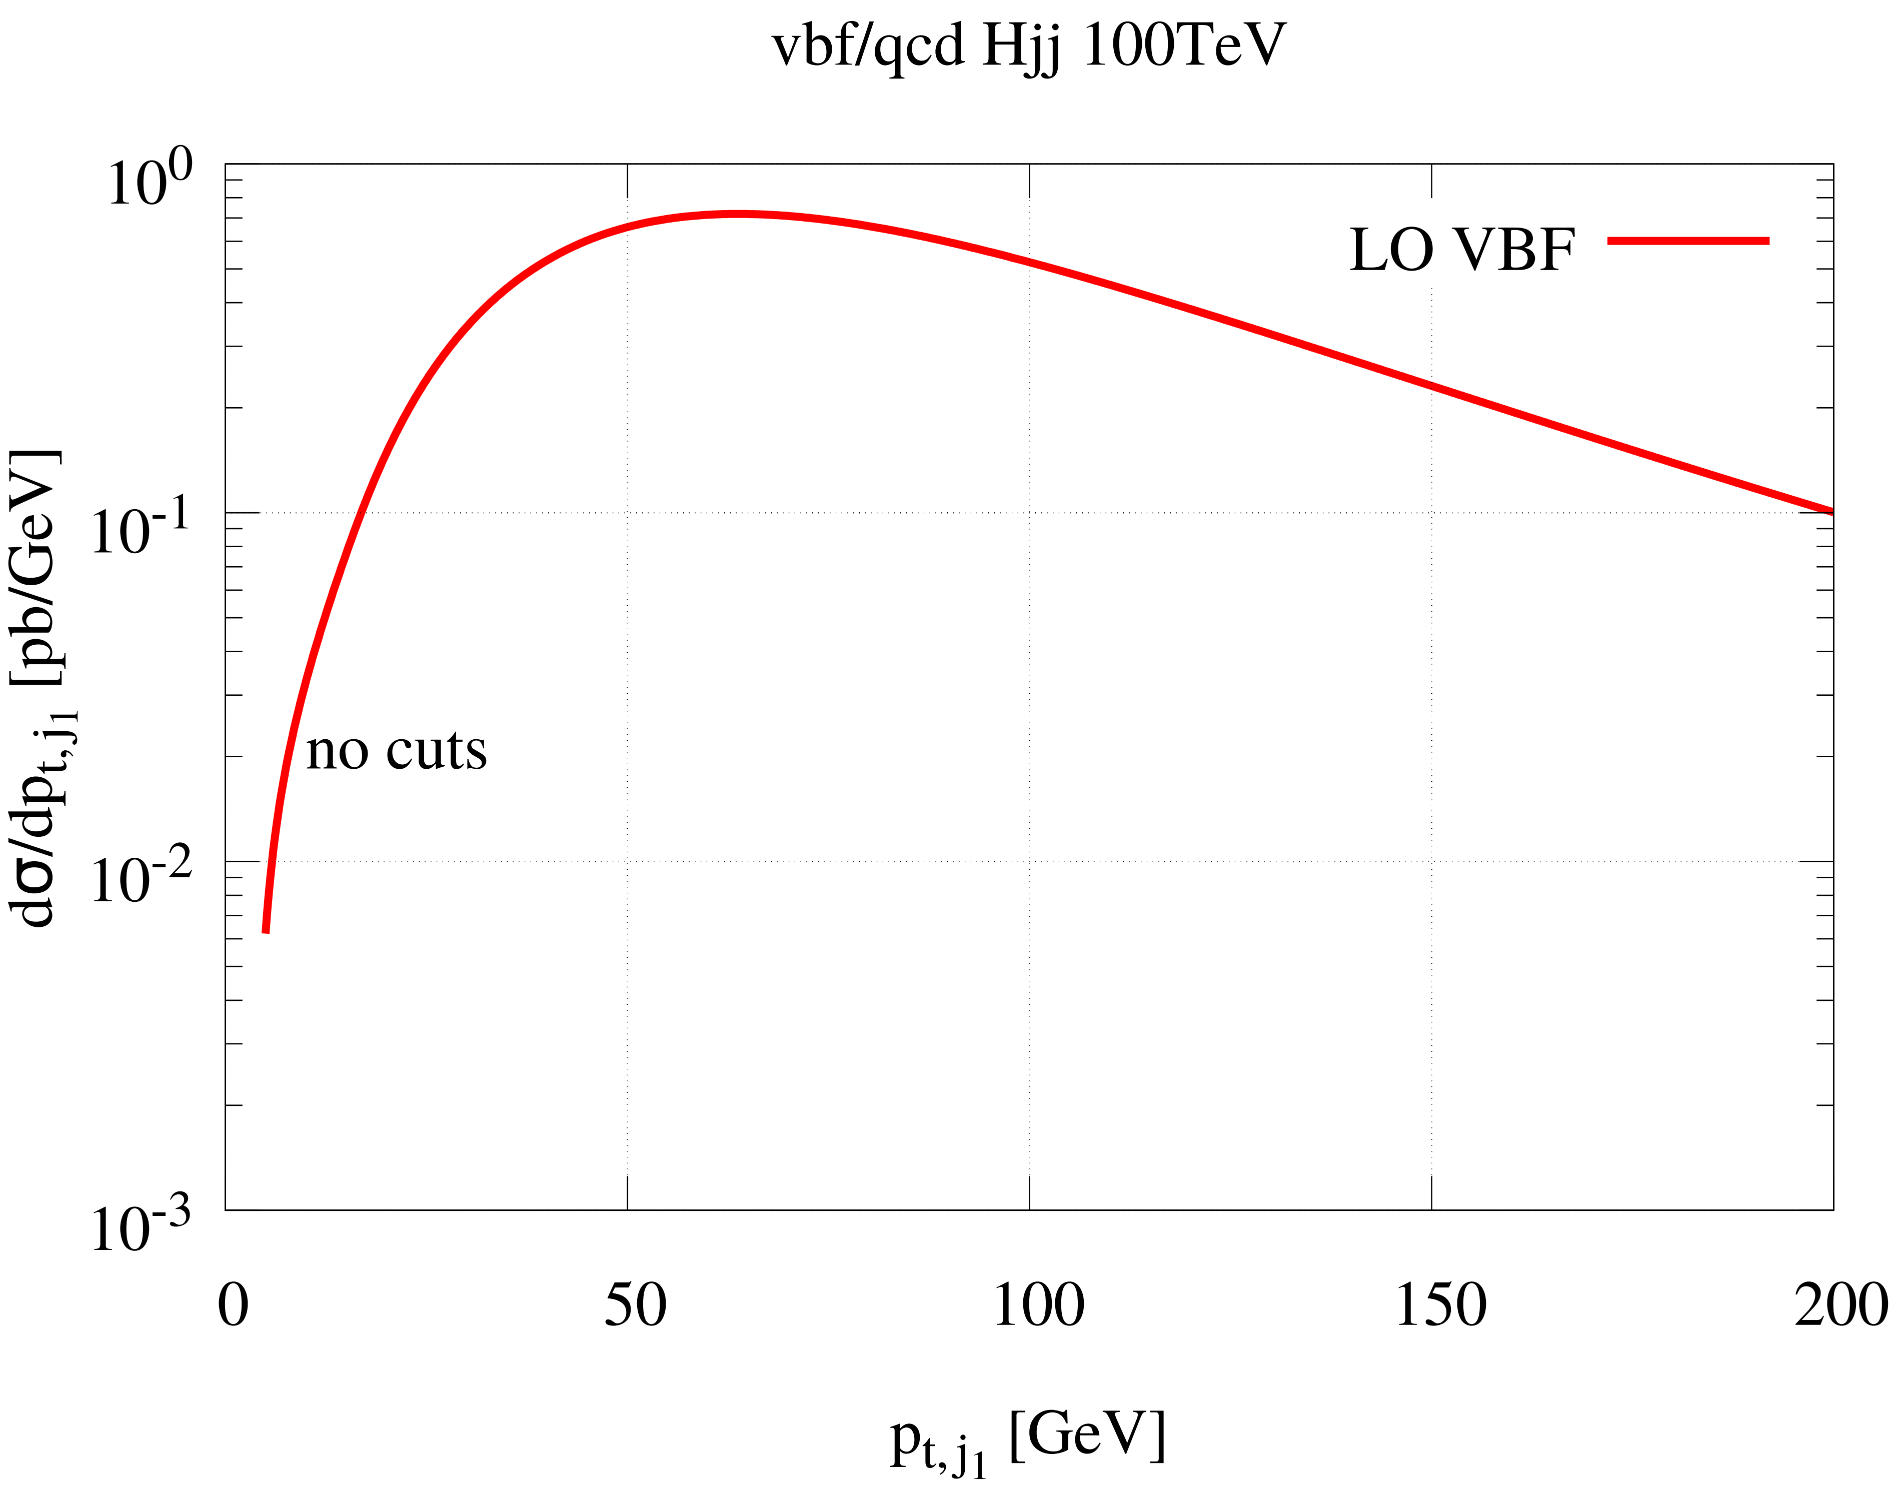

vbf/qcd Hjj 100TeV
LO VBF
no cuts
$10^0$
$10^{-1}$
$10^{-2}$
$10^{-3}$
0
50
100
150
200
$d\sigma/dp_{t,j_1}$ [pb/GeV]
$p_{t,j_1}$ [GeV]

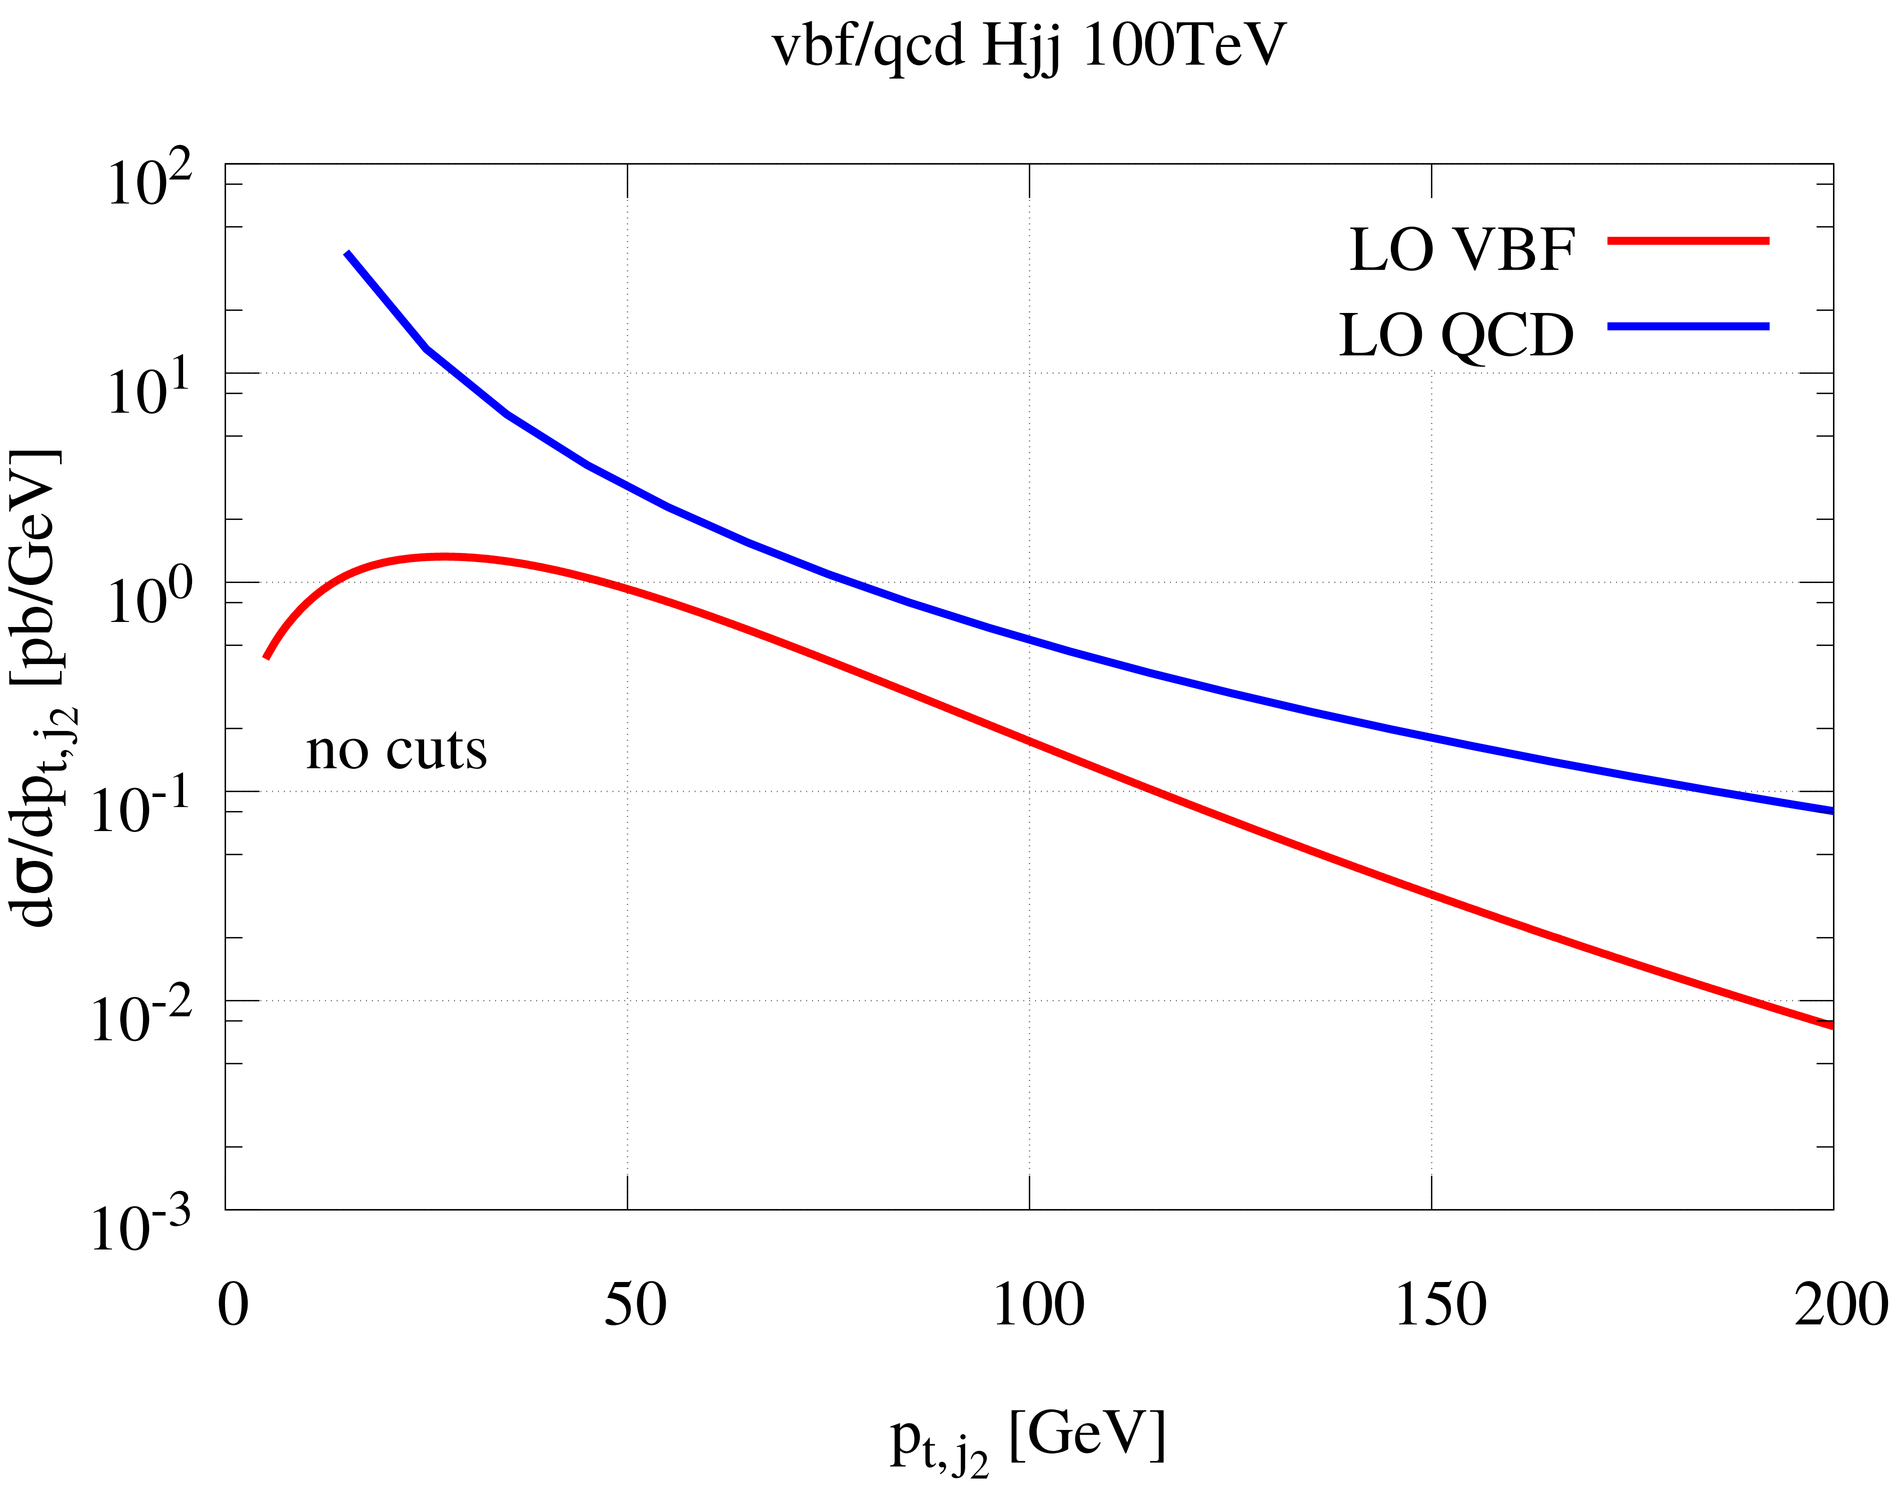

vbf/qcd Hjj 100TeV
LO VBF
LO QCD
no cuts
$10^{2}$
$10^{1}$
$10^{0}$
$10^{-1}$
$10^{-2}$
$10^{-3}$
0
50
100
150
200
$d\sigma/dp_{t,j_2}$ [pb/GeV]
$p_{t,j_2}$ [GeV]

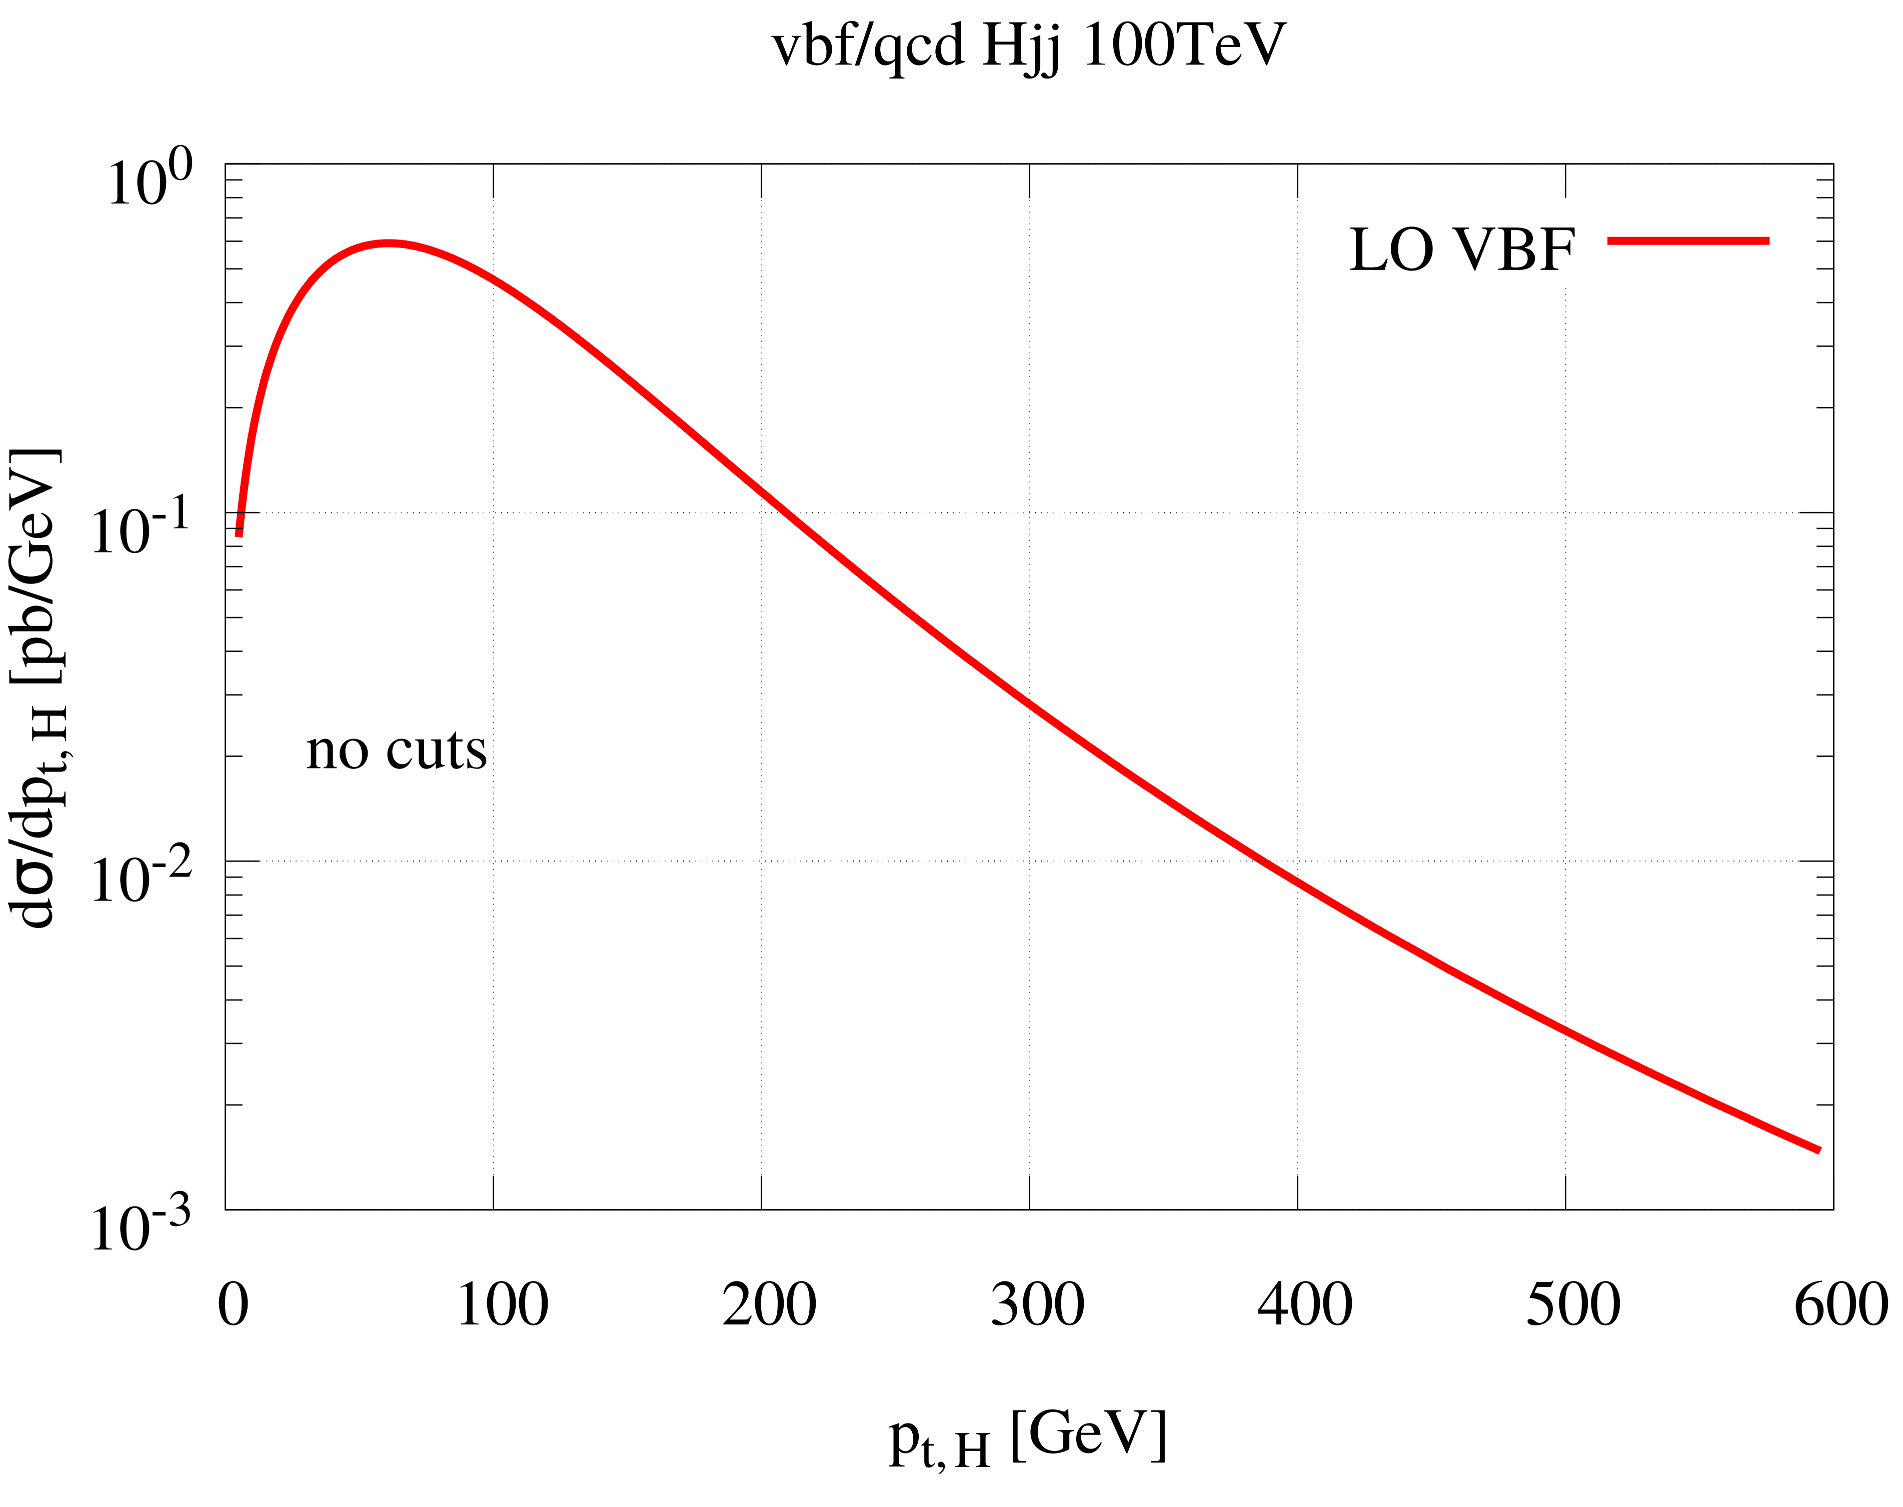

vbf/qcd Hjj 100TeV
LO VBF
no cuts
$d\sigma/dp_{t,H}$ [pb/GeV]
$p_{t,H}$ [GeV]
$10^0$
$10^{-1}$
$10^{-2}$
$10^{-3}$
0
100
200
300
400
500
600

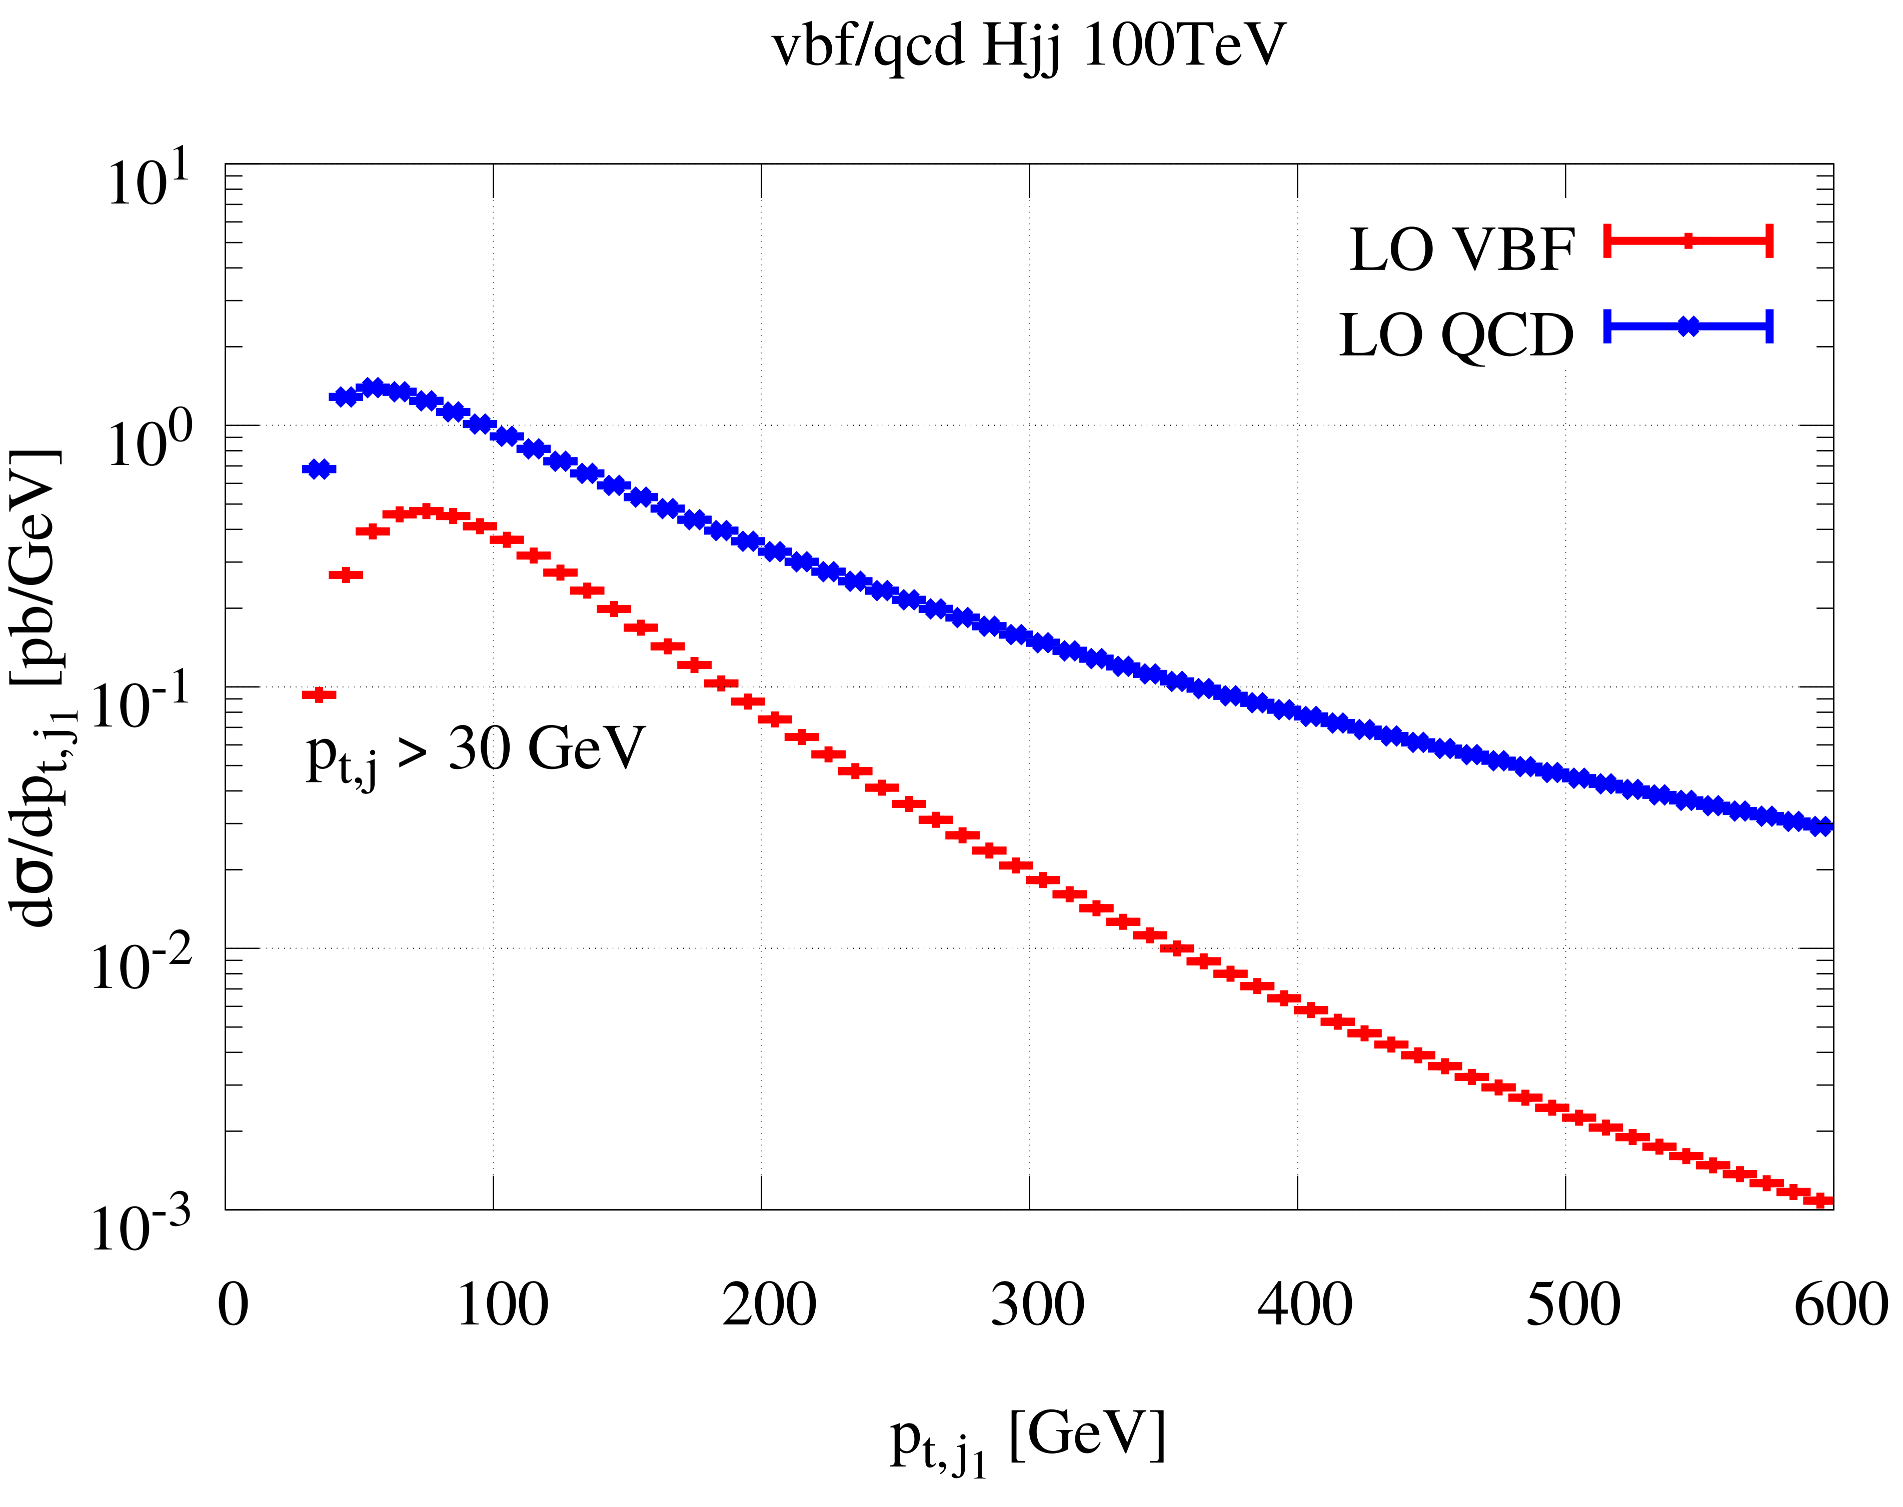
vbf/qcd Hjj 100TeV
LO VBF
LO QCD
$p_{t,j} > 30$ GeV
$d\sigma/dp_{t,j_1}$ [pb/GeV]
$p_{t,j_1}$ [GeV]
$10^{1}$
$10^{0}$
$10^{-1}$
$10^{-2}$
$10^{-3}$
0
100
200
300
400
500
600

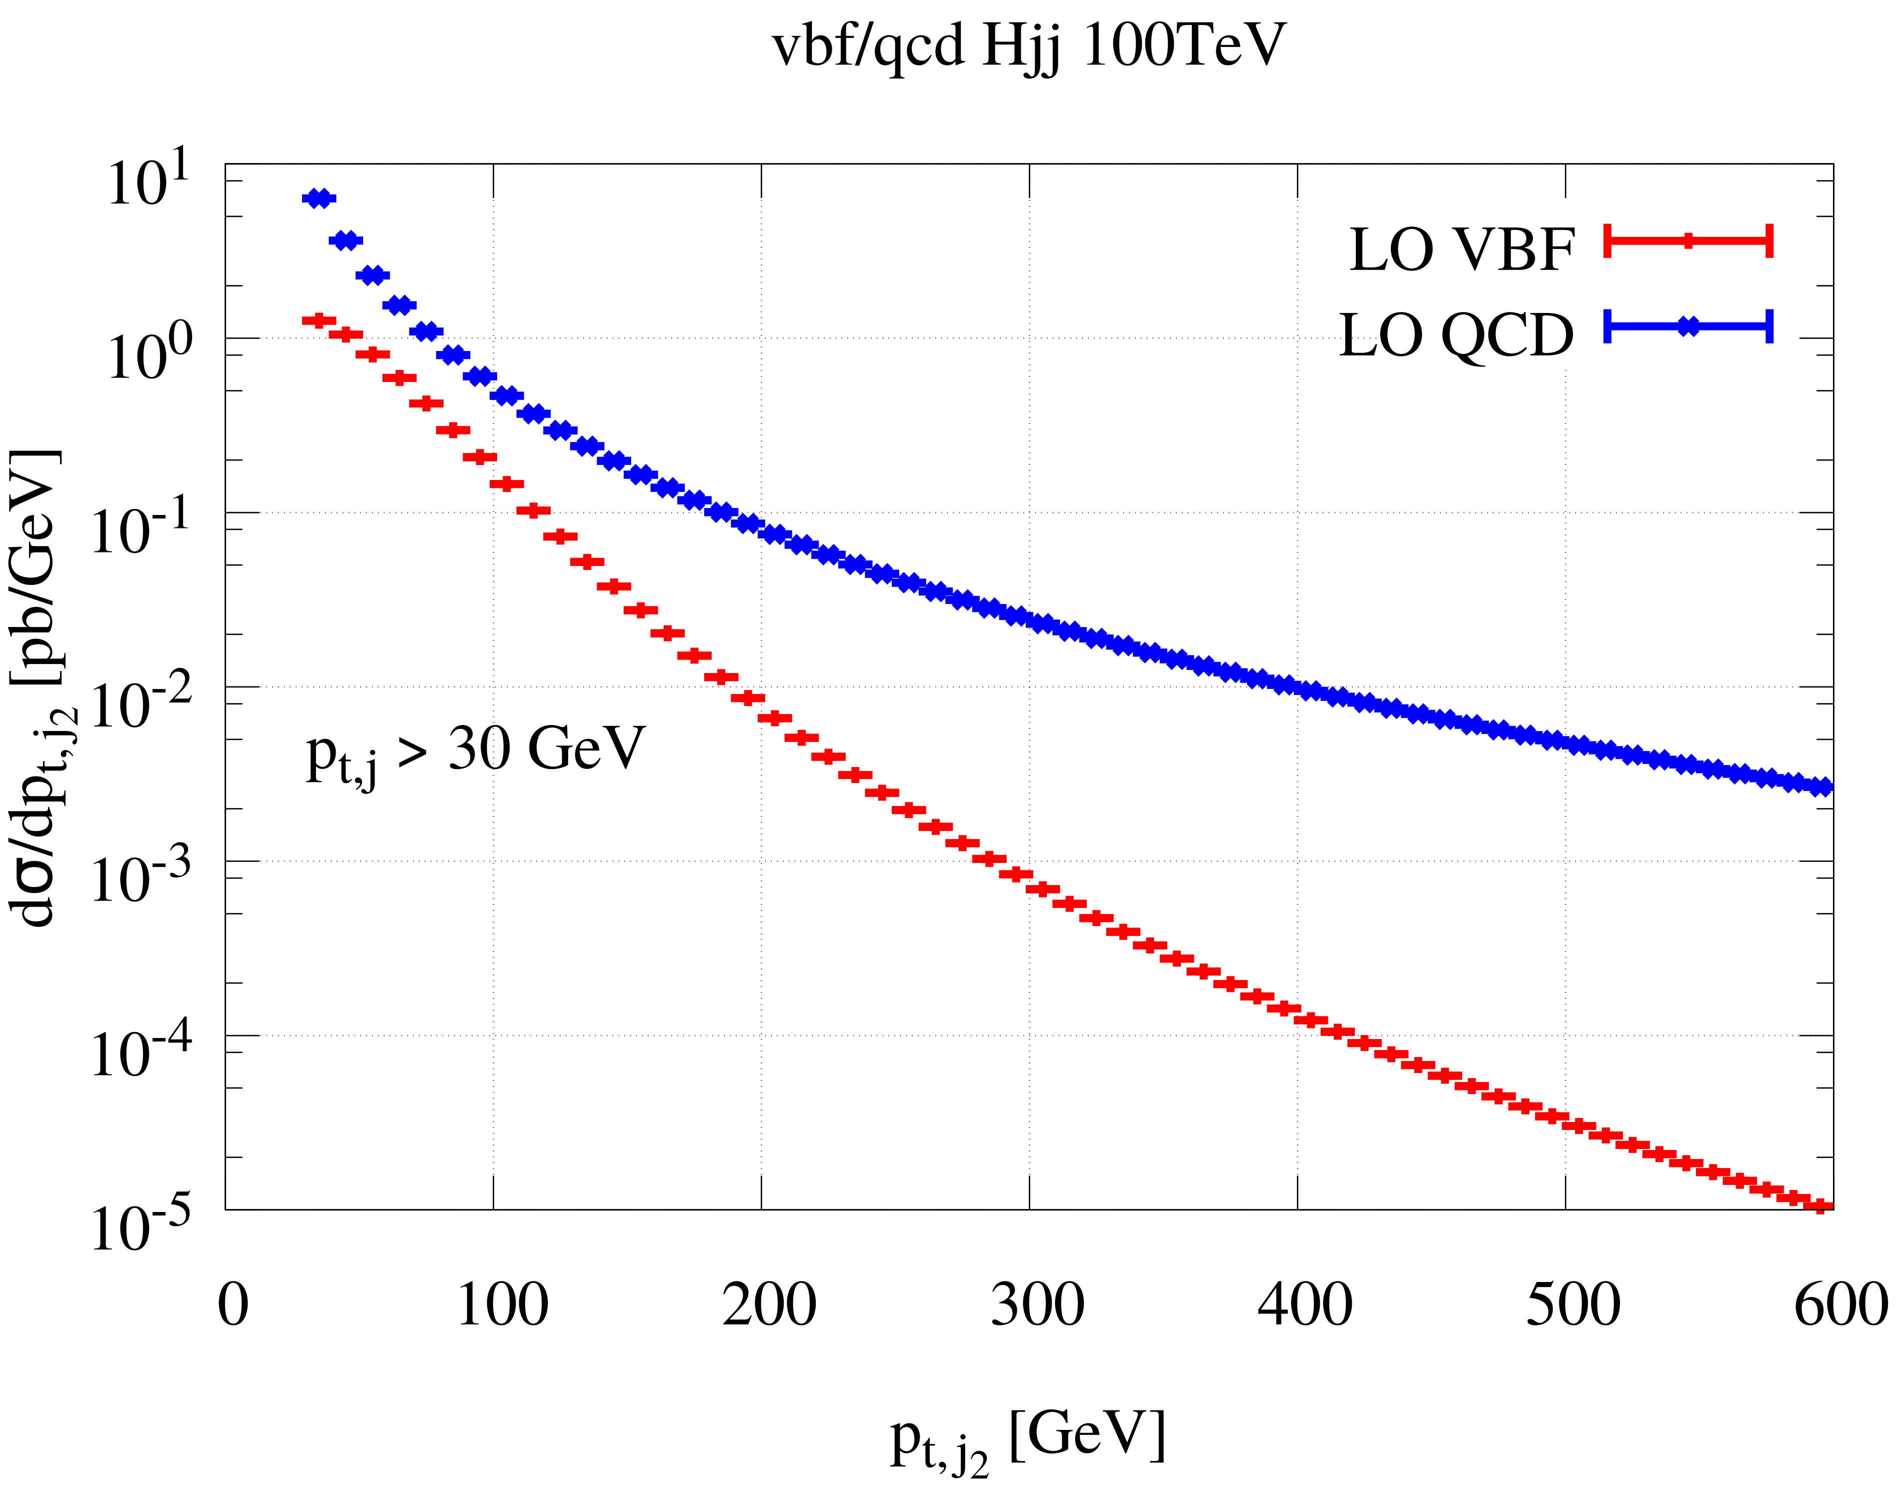

vbf/qcd Hjj 100TeV
LO VBF
LO QCD
$p_{t,j}$ > 30 GeV
$d\sigma/dp_{t,j_2}$ [pb/GeV]
$p_{t,j_2}$ [GeV]
$10^{1}$
$10^{0}$
$10^{-1}$
$10^{-2}$
$10^{-3}$
$10^{-4}$
$10^{-5}$
0
100
200
300
400
500
600

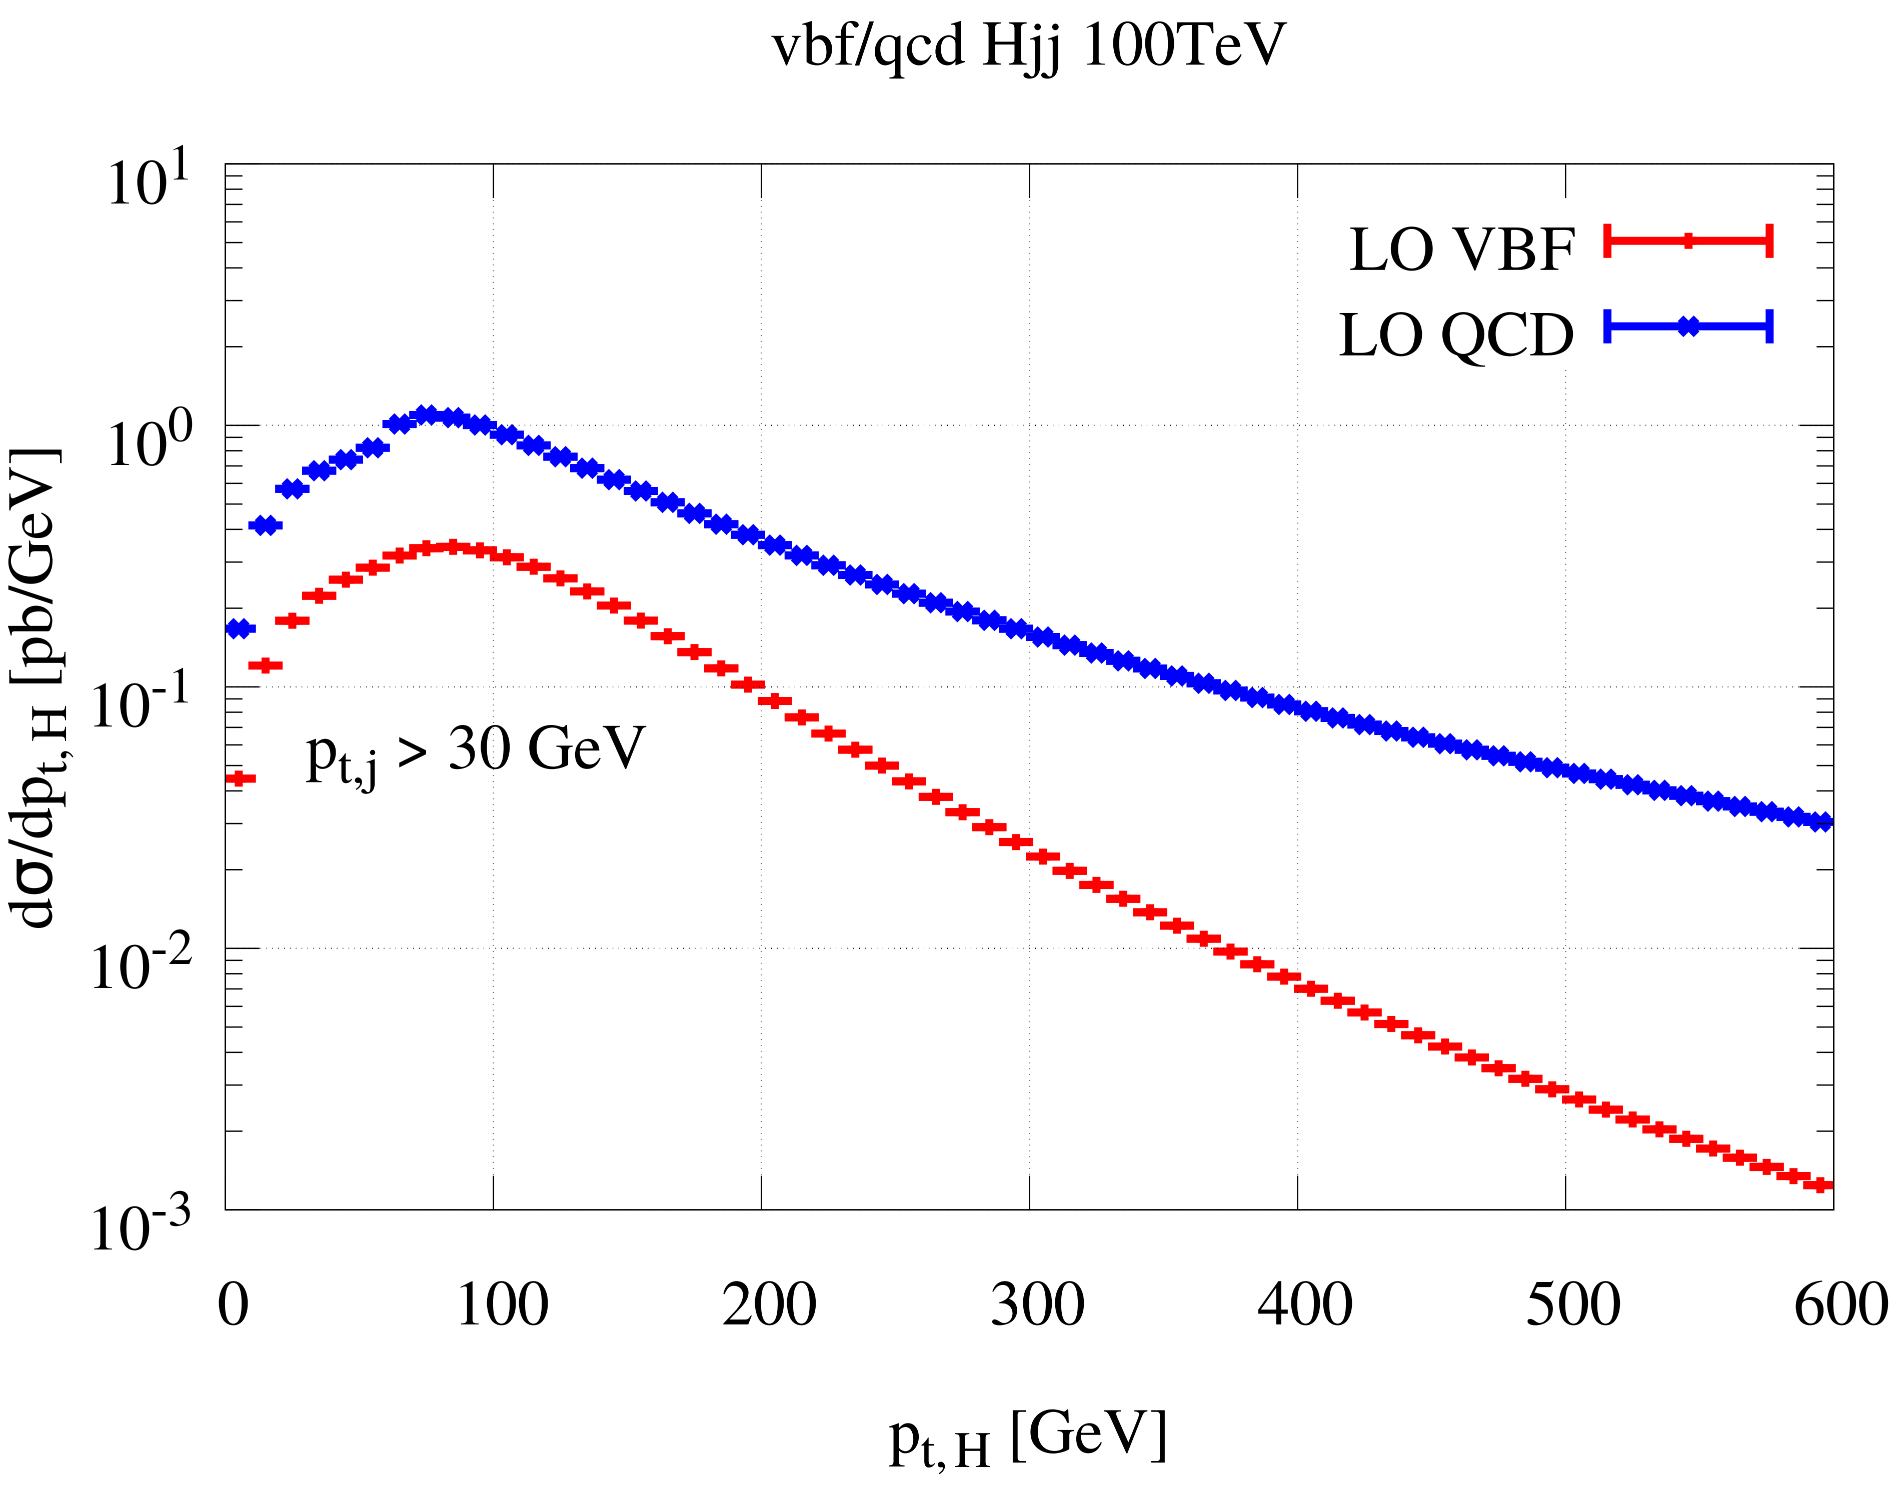

vbf/qcd Hjj 100TeV
LO VBF
LO QCD
$p_{t,j}$ > 30 GeV
$d\sigma/dp_{t,H}$ [pb/GeV]
$p_{t,H}$ [GeV]
$10^{1}$
$10^{0}$
$10^{-1}$
$10^{-2}$
$10^{-3}$
0
100
200
300
400
500
600

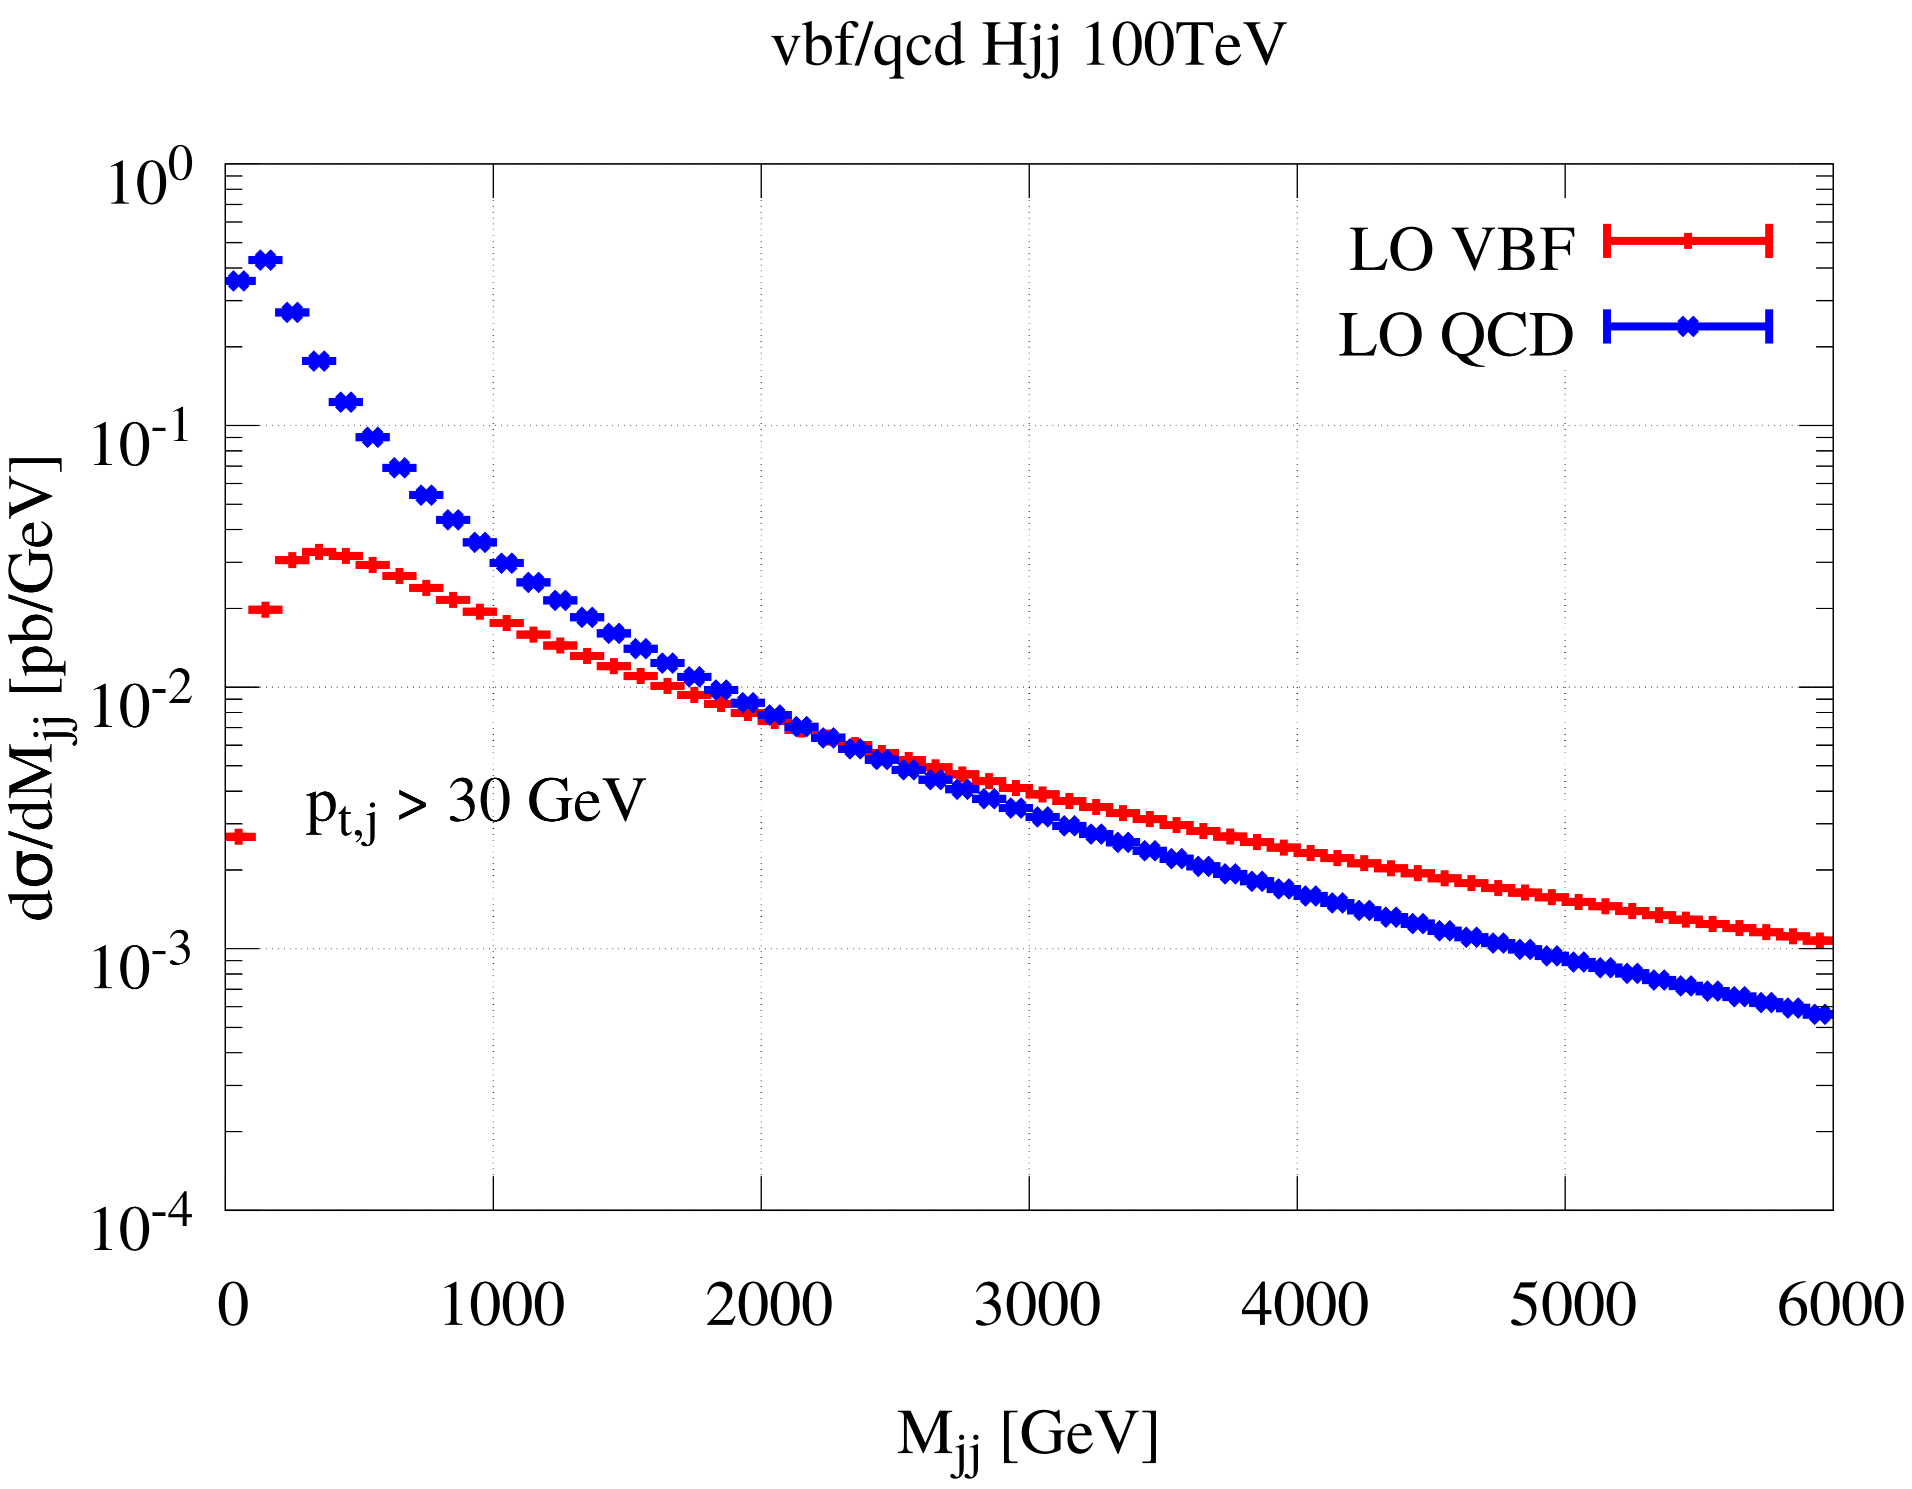

vbf/qcd Hjj 100TeV
LO VBF
LO QCD
$p_{t,j}$ > 30 GeV
$d\sigma/dM_{jj}$ [pb/GeV]
$M_{jj}$ [GeV]
$10^{0}$
$10^{-1}$
$10^{-2}$
$10^{-3}$
$10^{-4}$
0
1000
2000
3000
4000
5000
6000

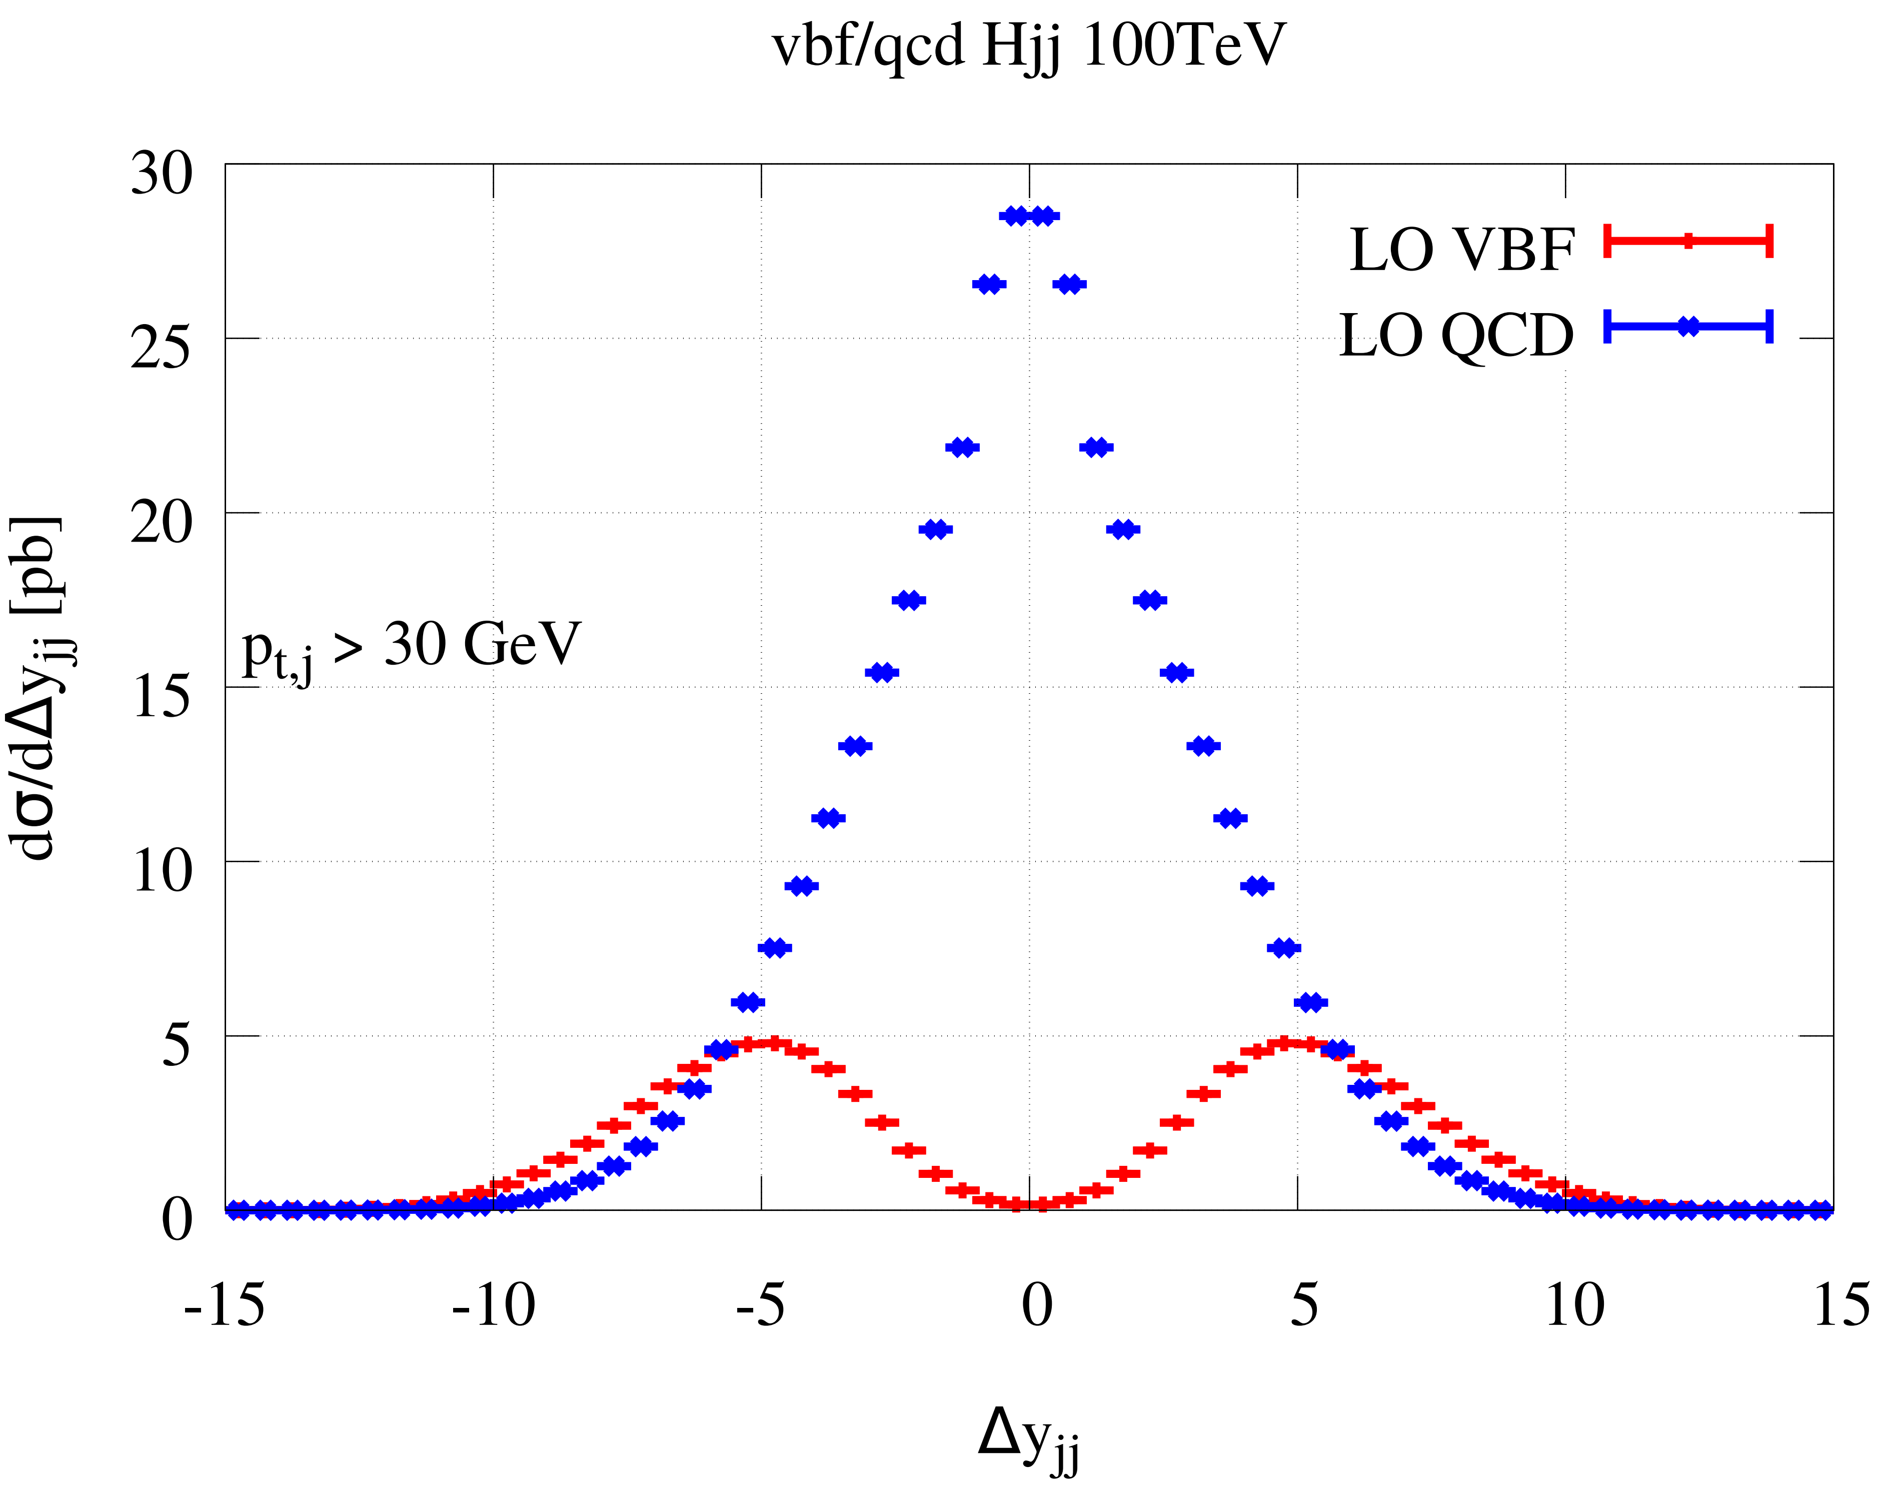

vbf/qcd Hjj 100TeV
LO VBF
LO QCD
$p_{t,j} > 30$ GeV
$d\sigma/d\Delta y_{jj}$ [pb]
$\Delta y_{jj}$
30
25
20
15
10
5
0
-15
-10
-5
0
5
10
15

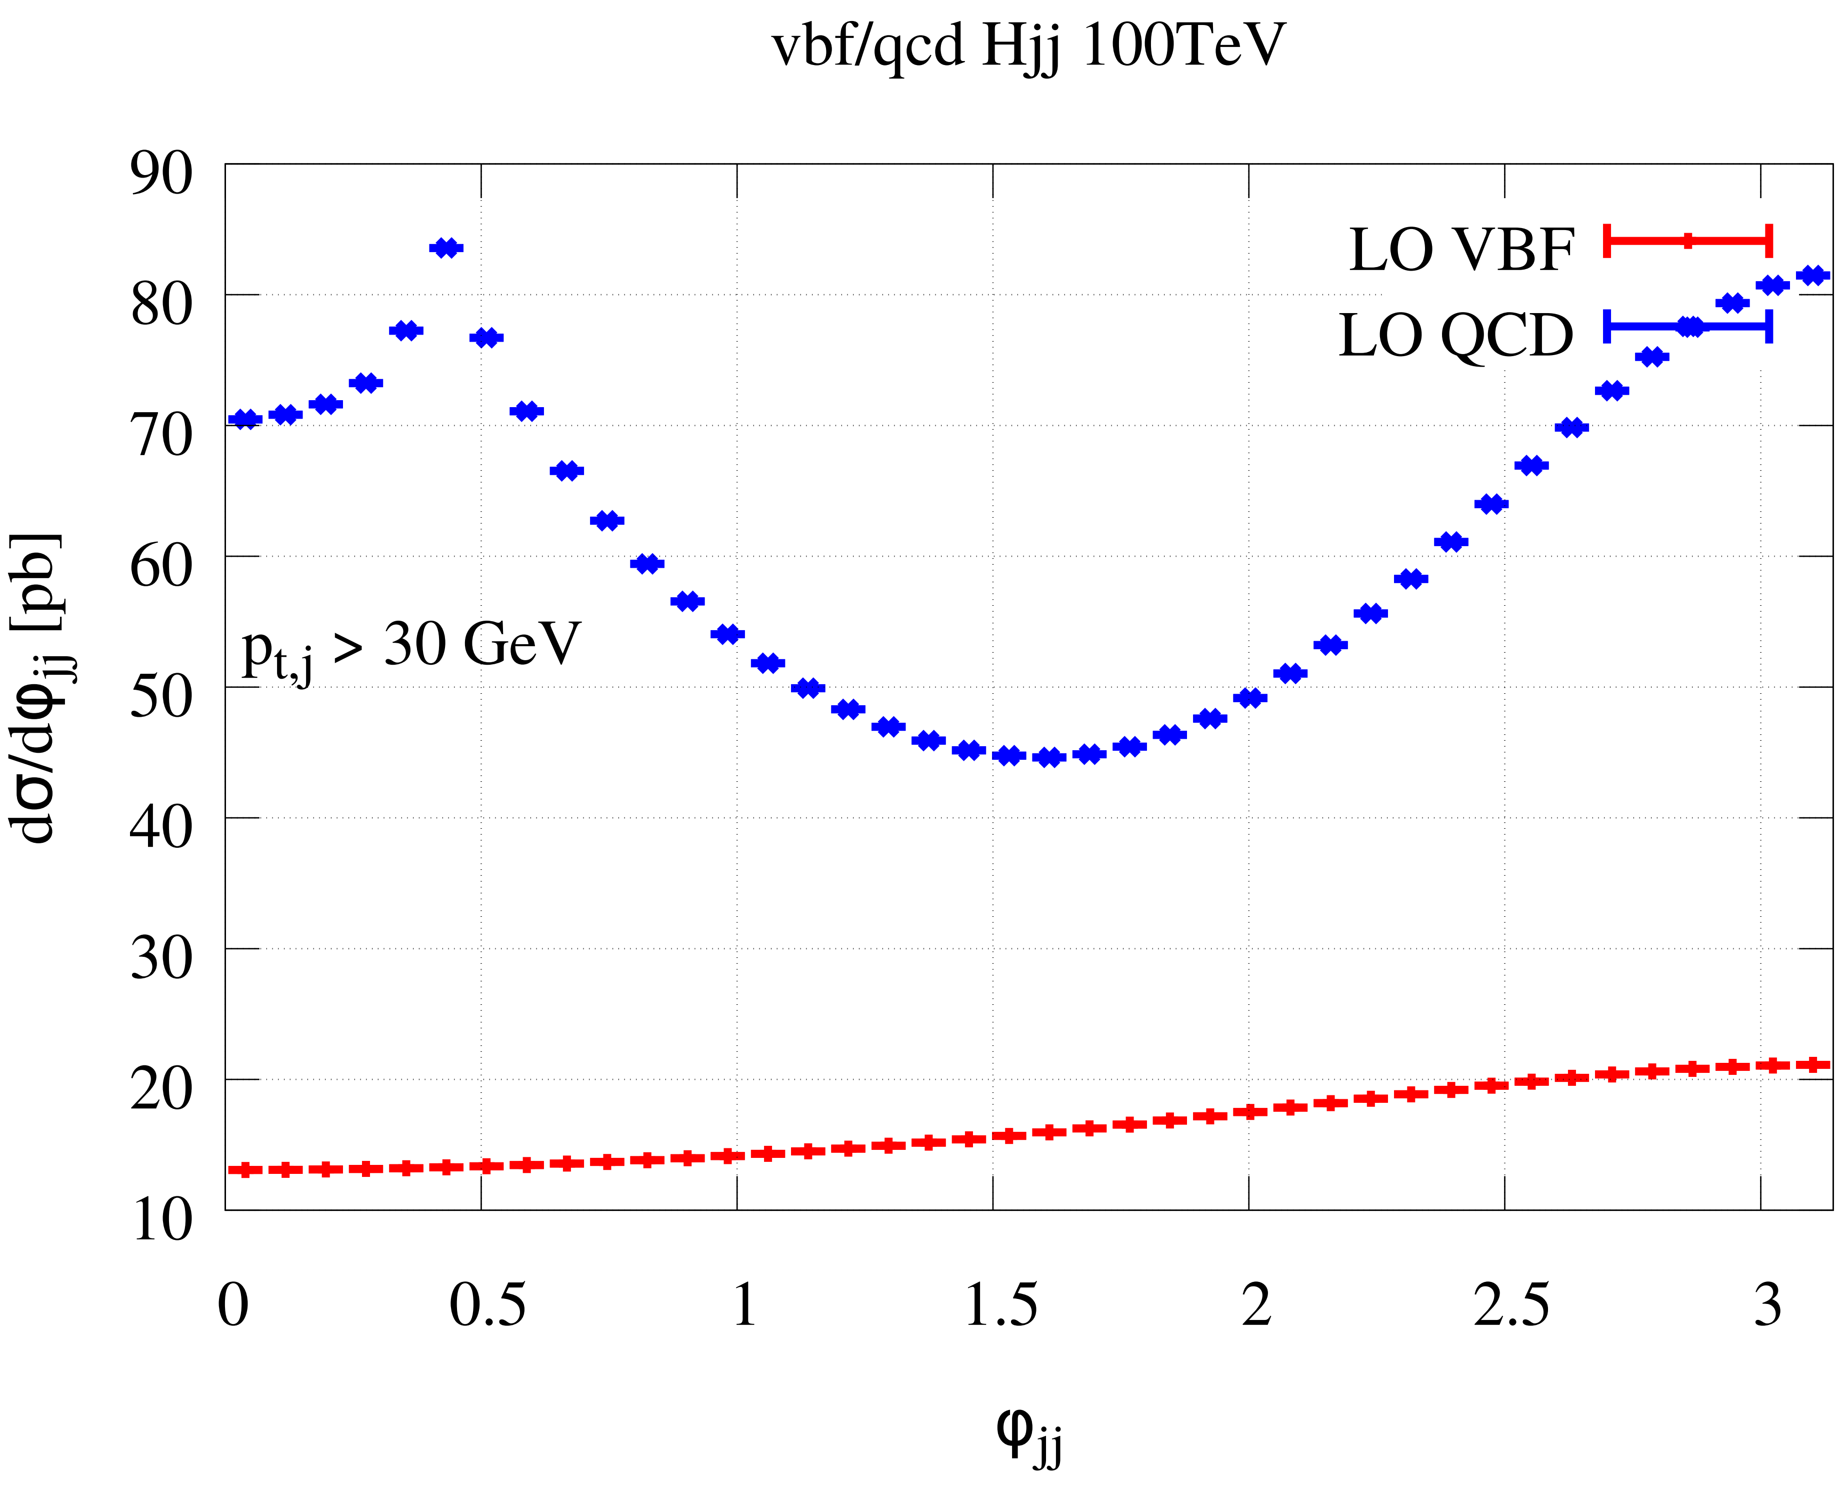
vbf/qcd Hjj 100TeV
LO VBF
LO QCD
$p_{t,j}$ > 30 GeV
$d\sigma/d\varphi_{jj}$ [pb]
$\varphi_{jj}$
10
20
30
40
50
60
70
80
90
0
0.5
1
1.5
2
2.5
3

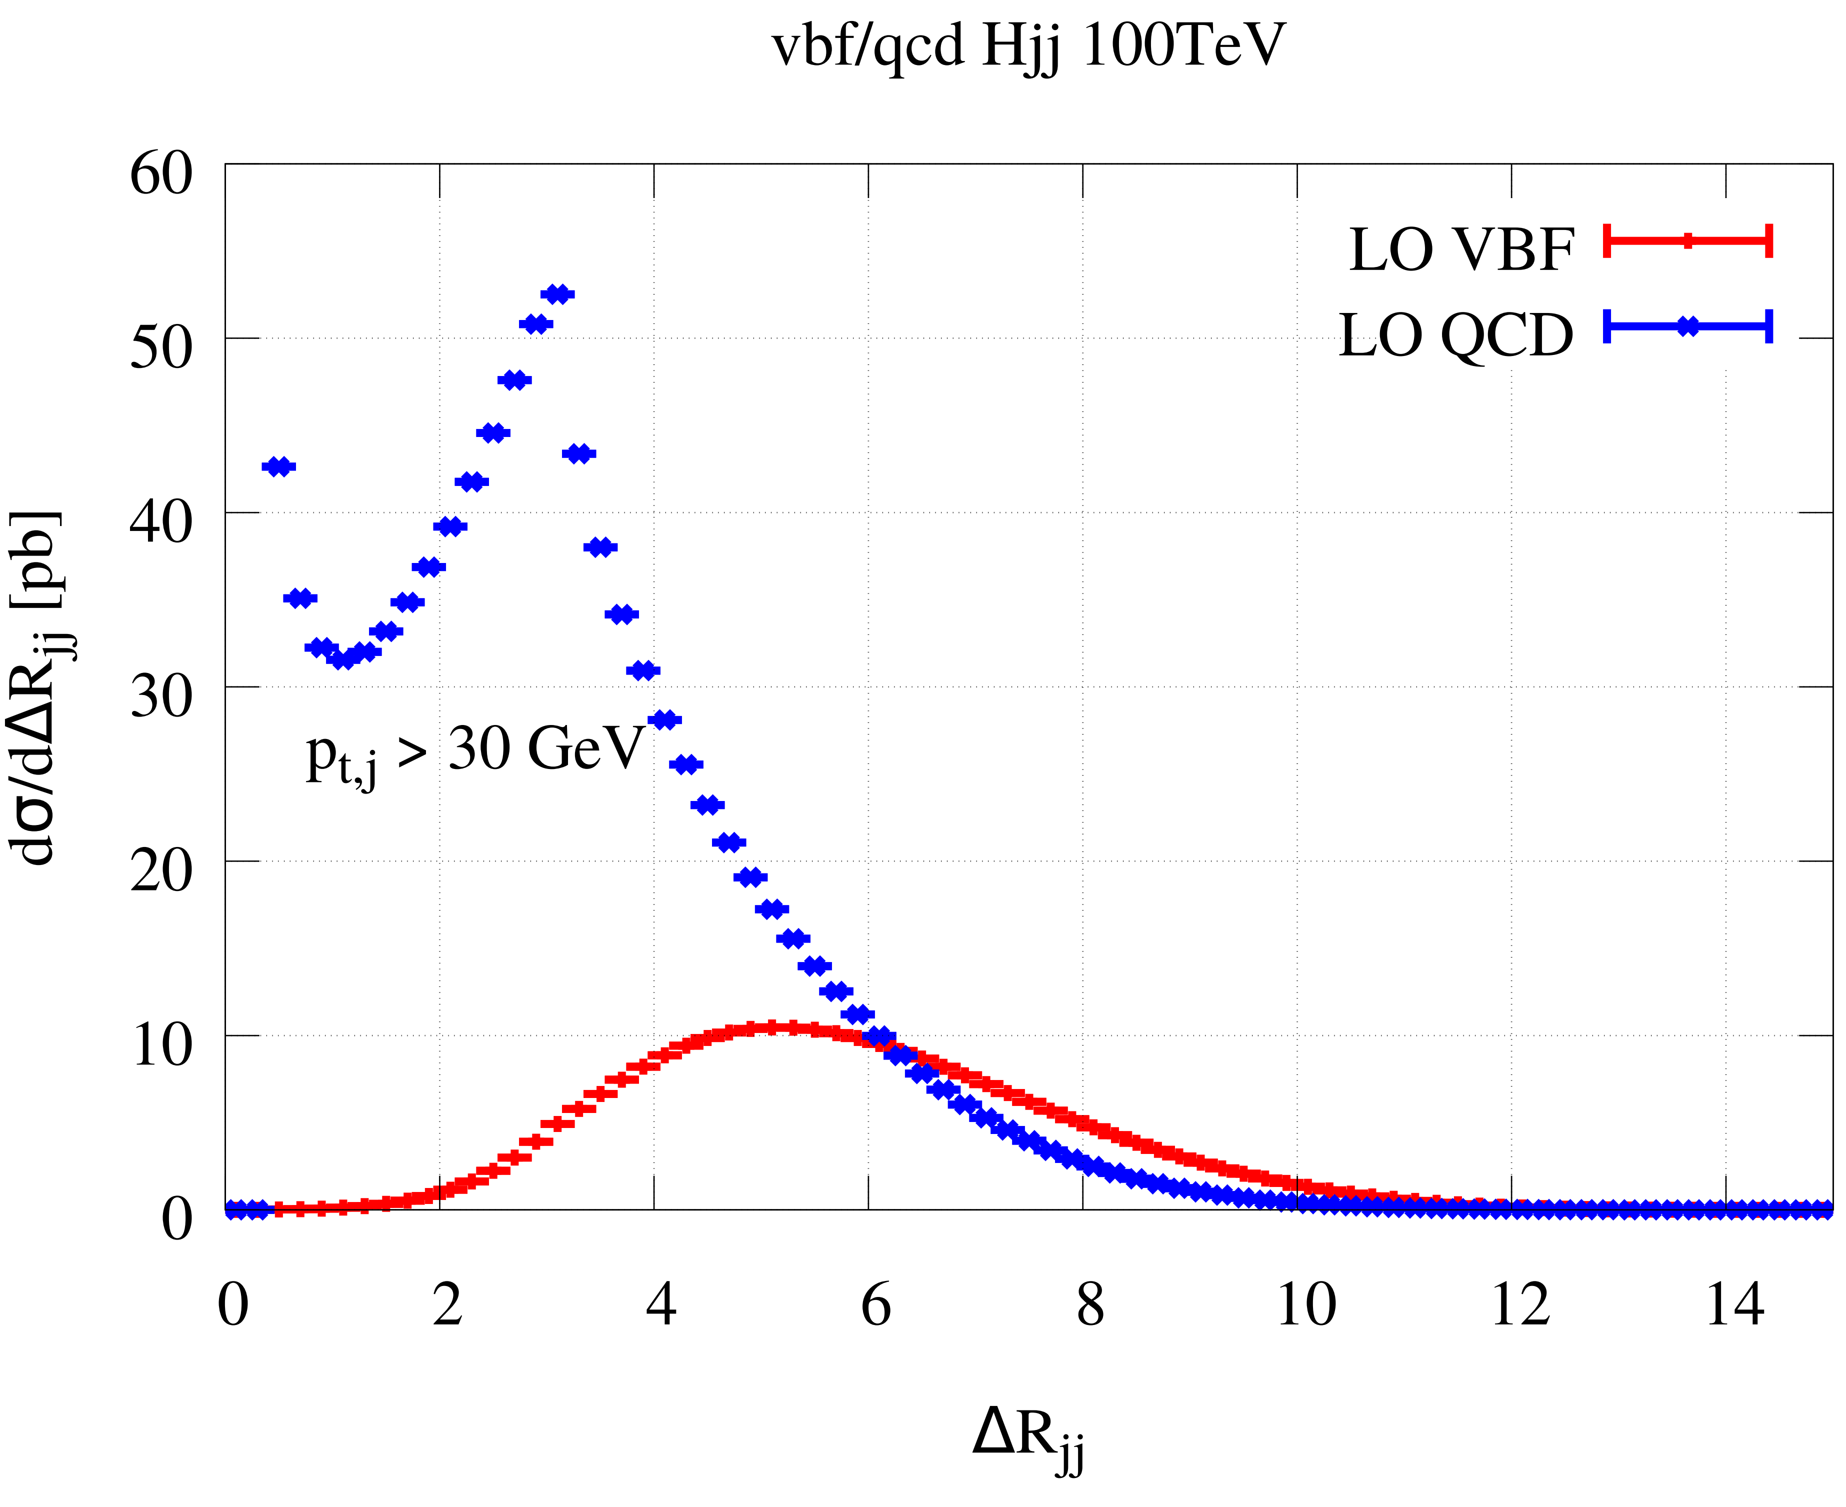

vbf/qcd Hjj 100TeV
LO VBF
LO QCD
$p_{t,j}$ > 30 GeV
$d\sigma/d\Delta R_{jj}$ [pb]
$\Delta R_{jj}$
0
10
20
30
40
50
60
0
2
4
6
8
10
12
14

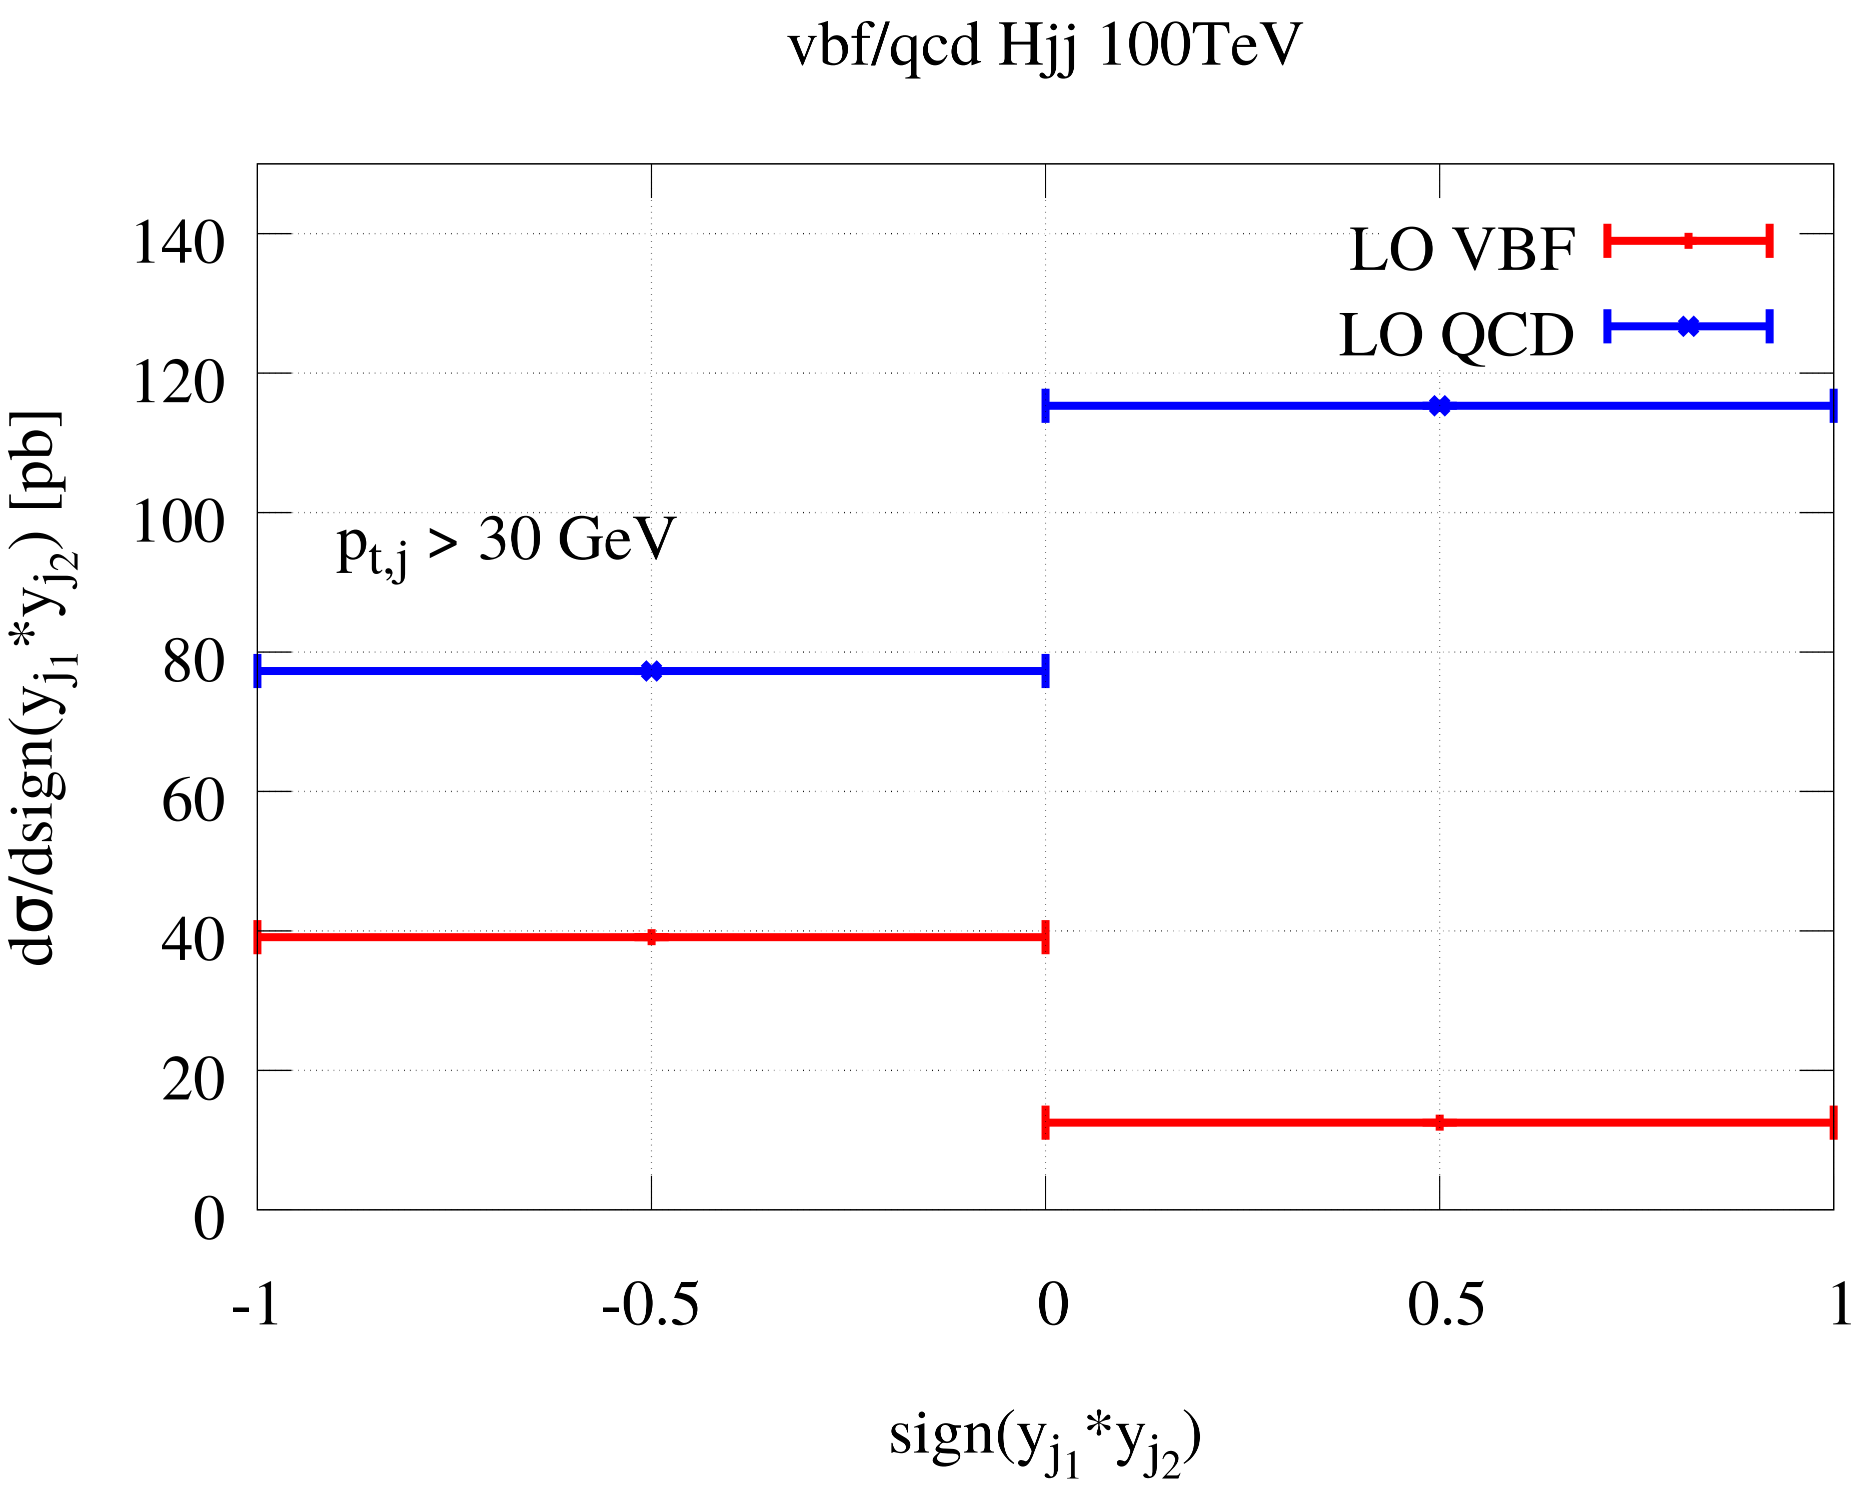

vbf/qcd Hjj 100TeV
LO VBF
LO QCD
$p_{t,j}$ > 30 GeV
$d\sigma/dsign(y_{j_1}*y_{j_2})$ [pb]
$sign(y_{j_1}*y_{j_2})$
0
20
40
60
80
100
120
140
-1
-0.5
0
0.5
1

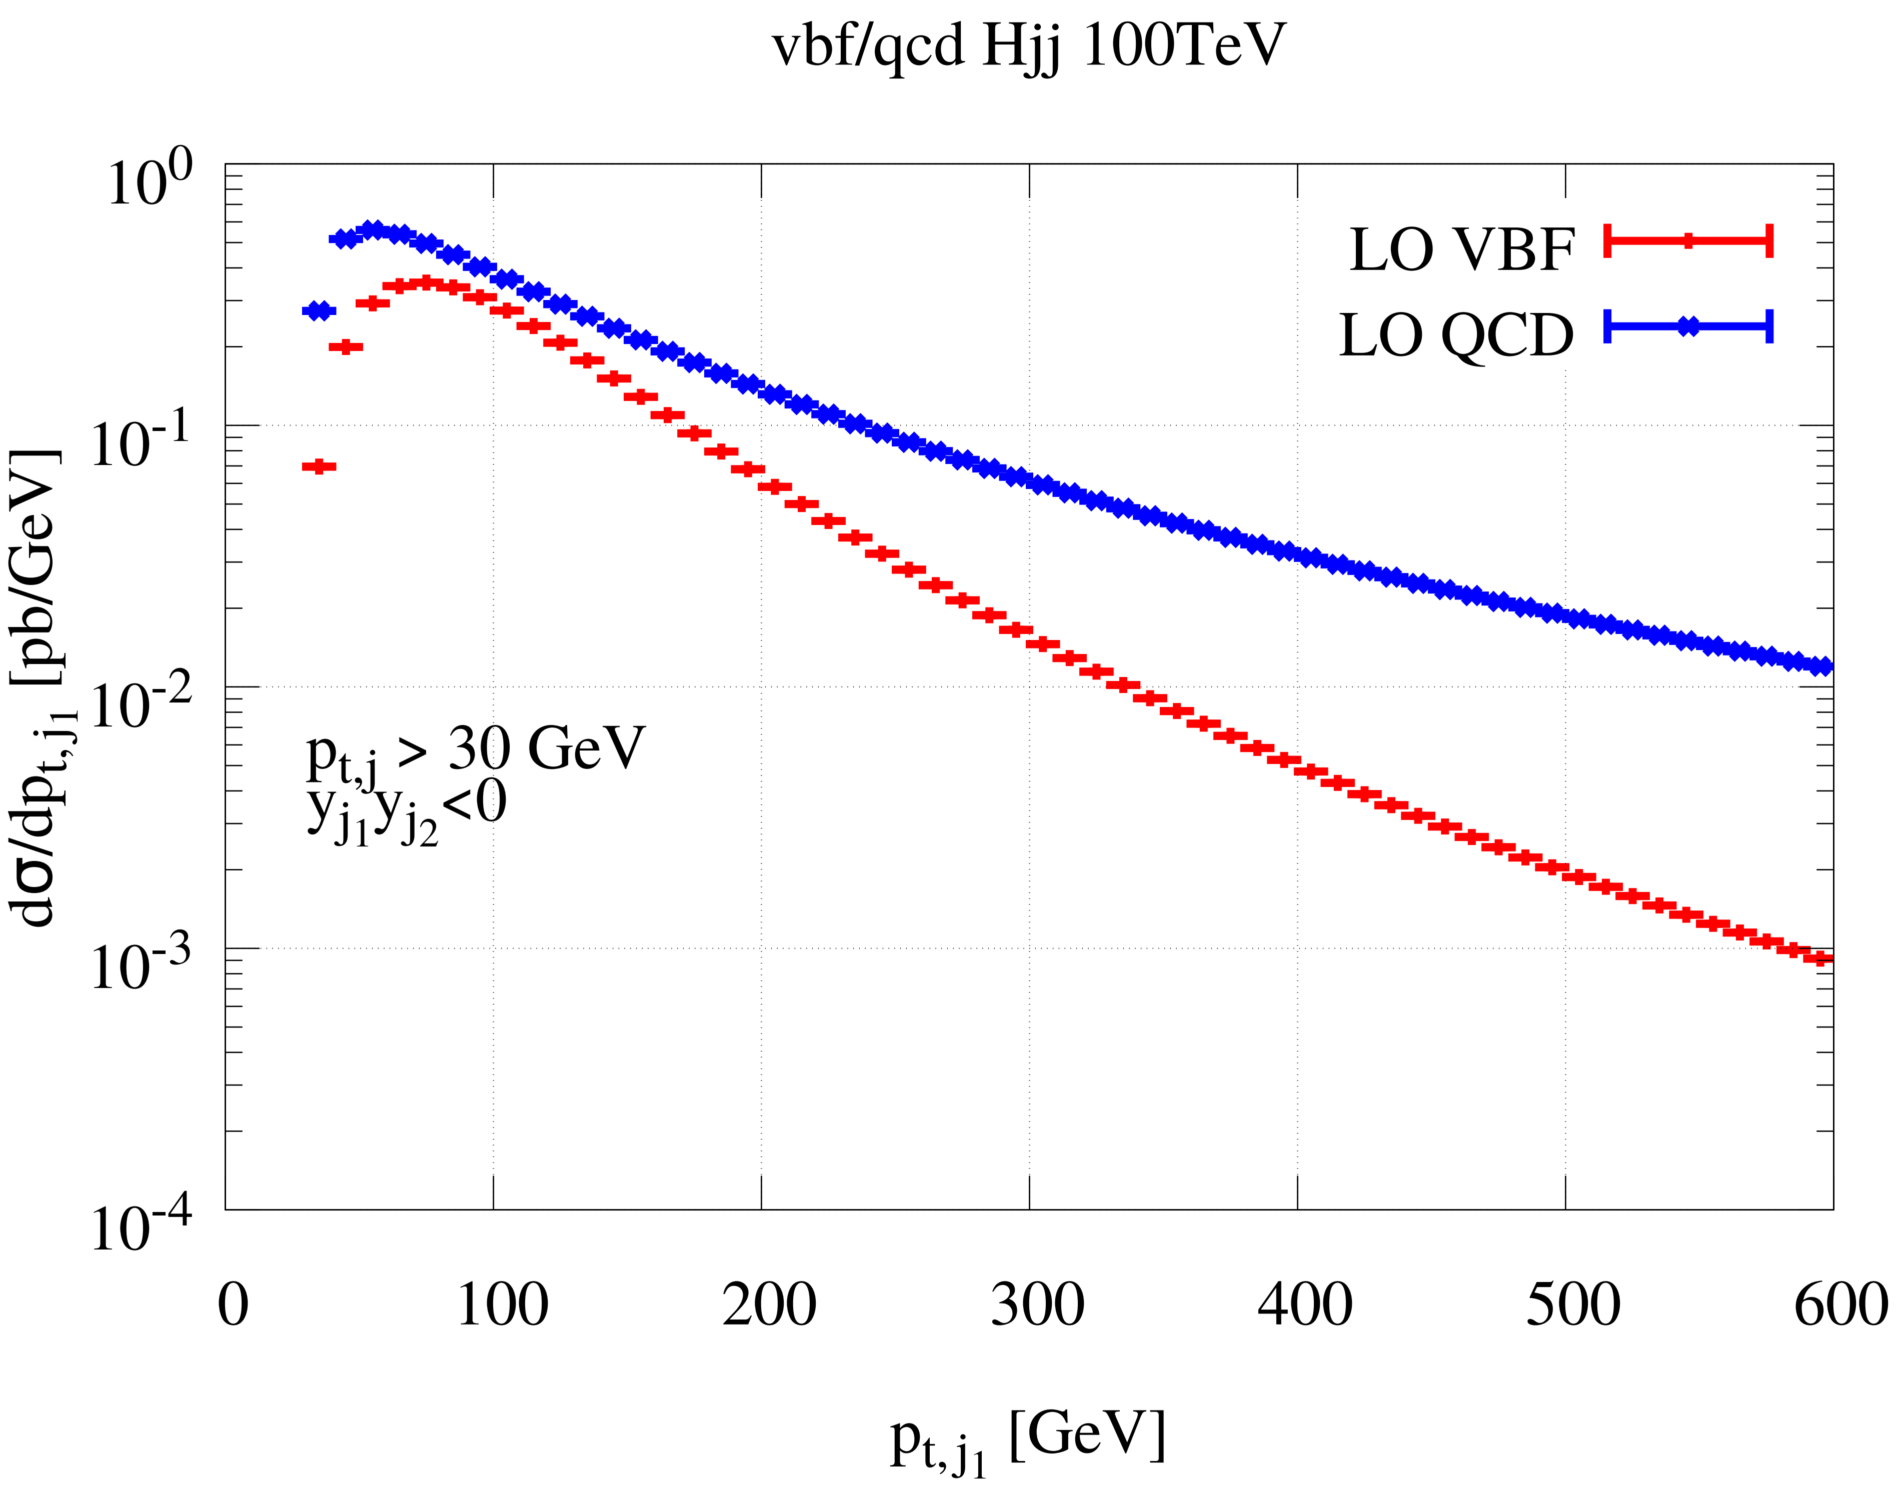
vbf/qcd Hjj 100TeV
LO VBF
LO QCD
$p_{t,j}$ > 30 GeV
$y_{j_1}y_{j_2}<0$
$d\sigma/dp_{t,j_1}$ [pb/GeV]
$p_{t,j_1}$ [GeV]
$10^0$
$10^{-1}$
$10^{-2}$
$10^{-3}$
$10^{-4}$
0
100
200
300
400
500
600

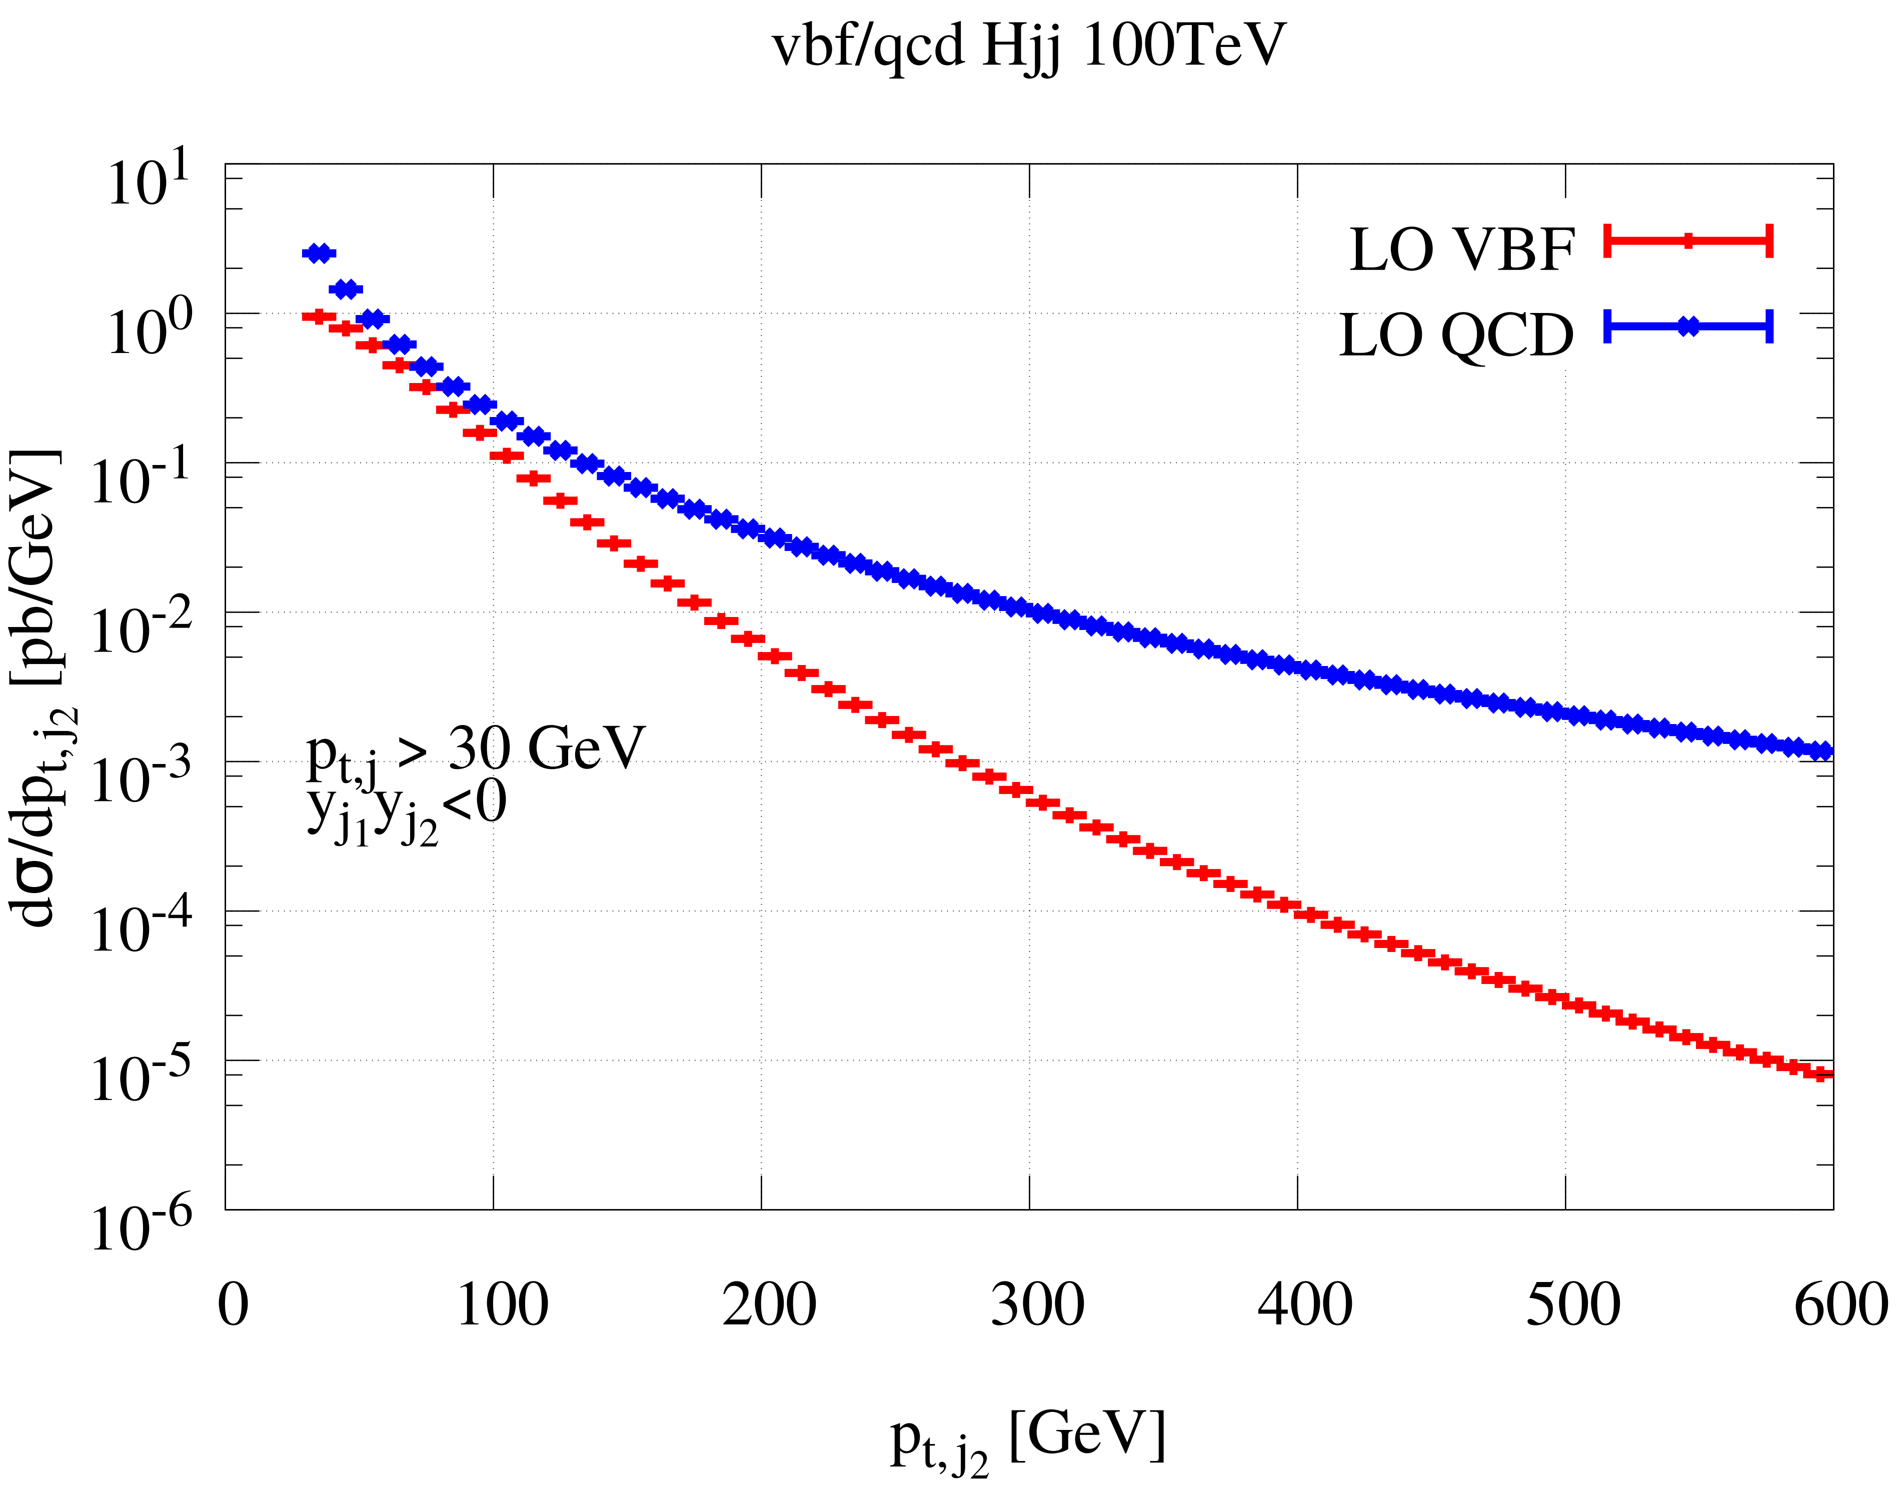

vbf/qcd Hjj 100TeV
LO VBF
LO QCD
$p_{t,j}$ > 30 GeV
$y_{j_1}y_{j_2}$<0
$d\sigma/dp_{t,j_2}$ [pb/GeV]
$p_{t,j_2}$ [GeV]
$10^{1}$
$10^{0}$
$10^{-1}$
$10^{-2}$
$10^{-3}$
$10^{-4}$
$10^{-5}$
$10^{-6}$
0
100
200
300
400
500
600

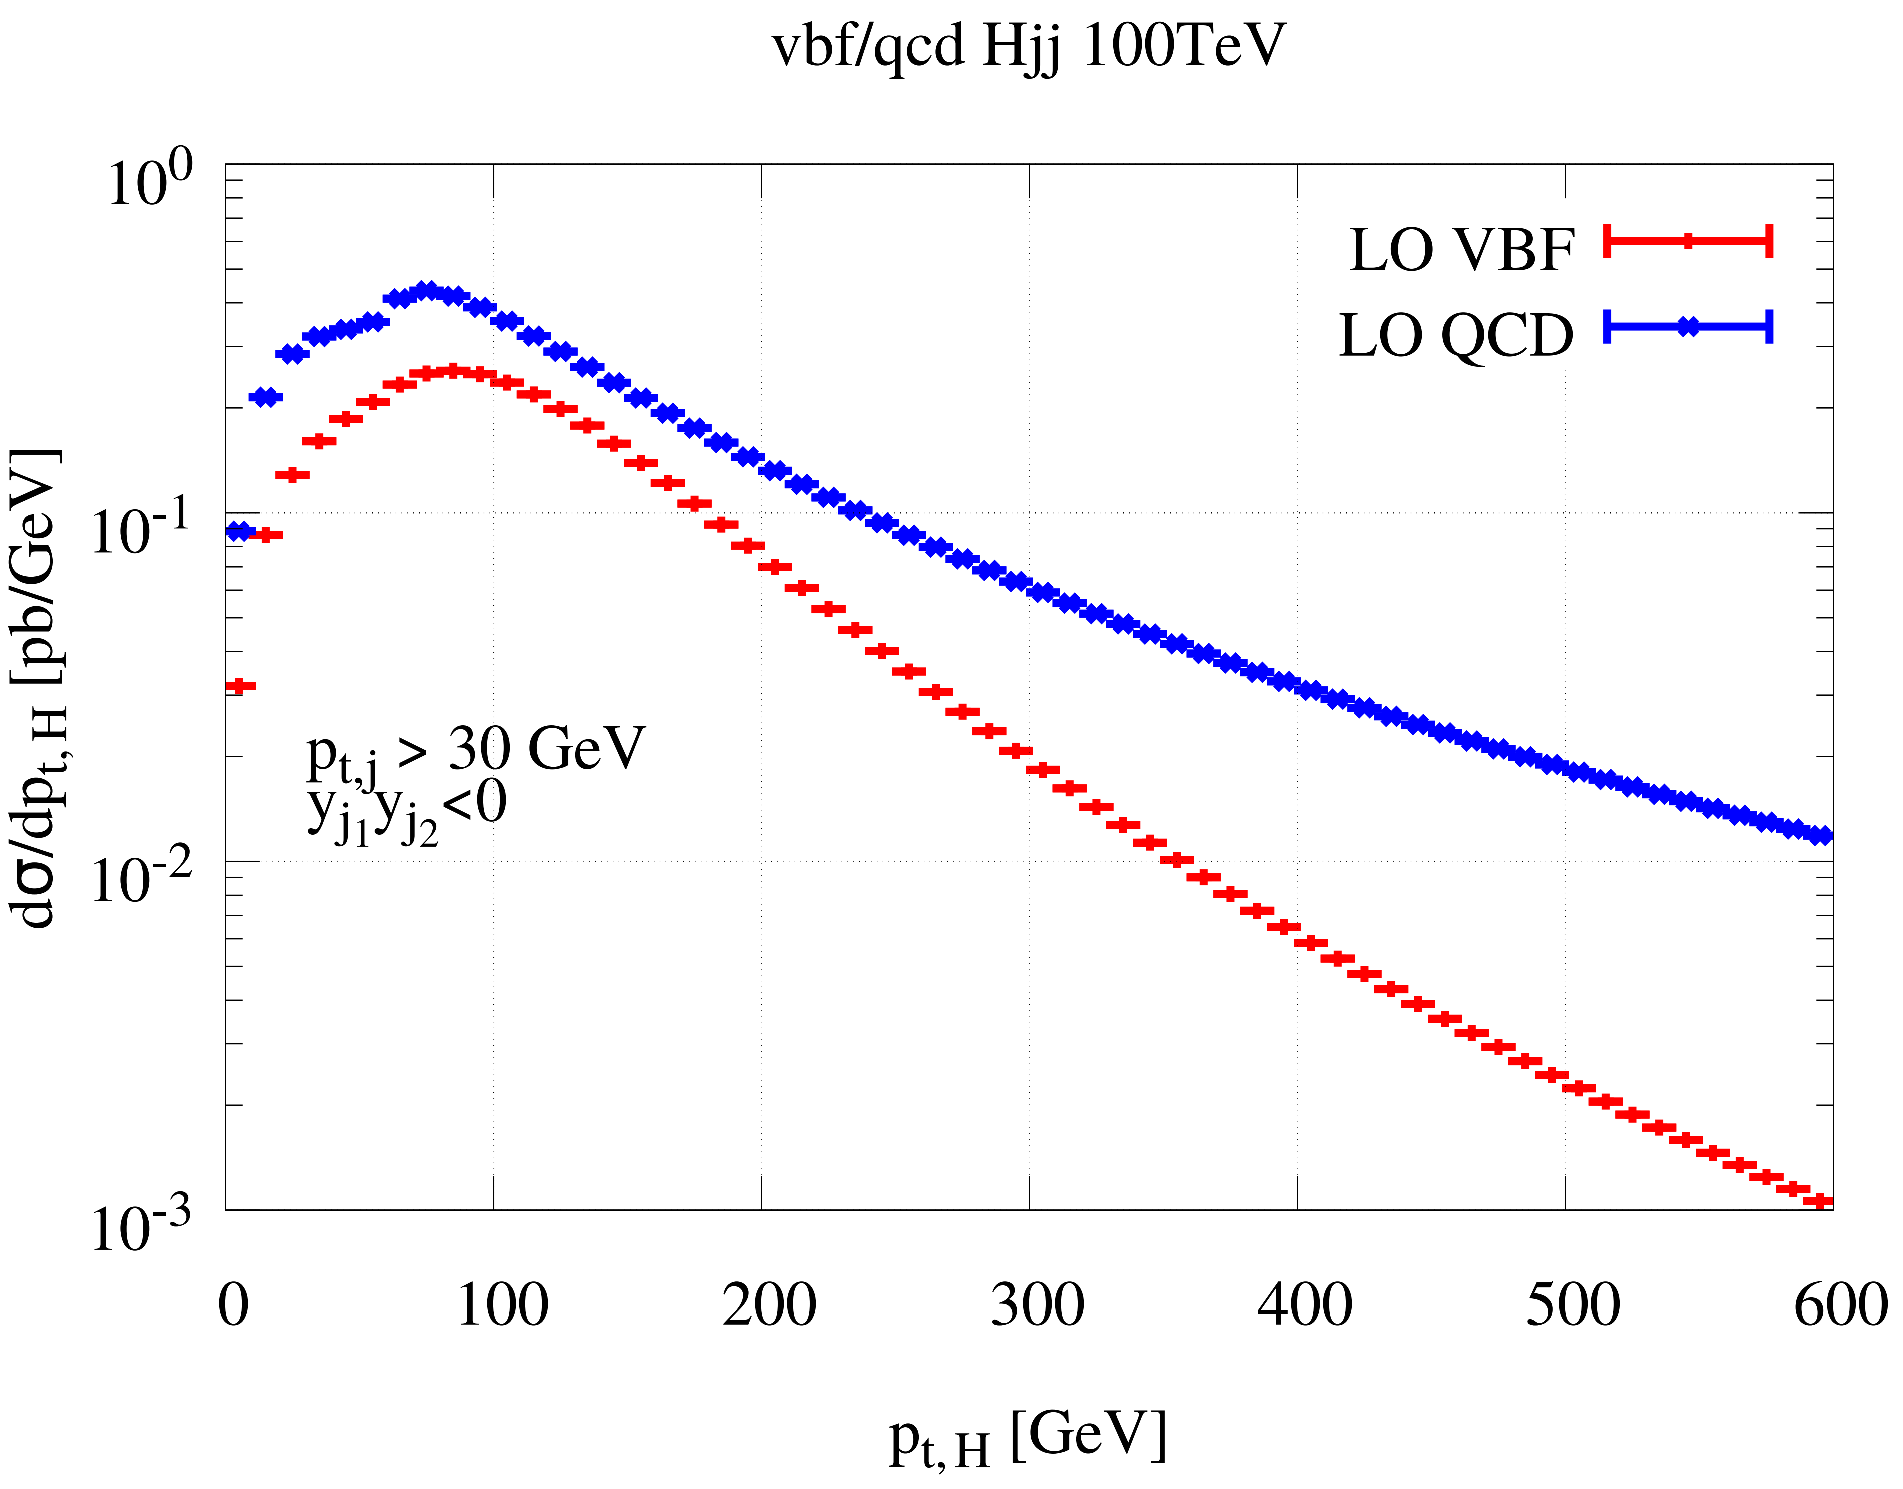
vbf/qcd Hjj 100TeV
LO VBF
LO QCD
$p_{t,j}$ > 30 GeV
$y_{j_1}y_{j_2}<0$
$d\sigma/dp_{t,H}$ [pb/GeV]
$p_{t,H}$ [GeV]
$10^{0}$
$10^{-1}$
$10^{-2}$
$10^{-3}$
0
100
200
300
400
500
600

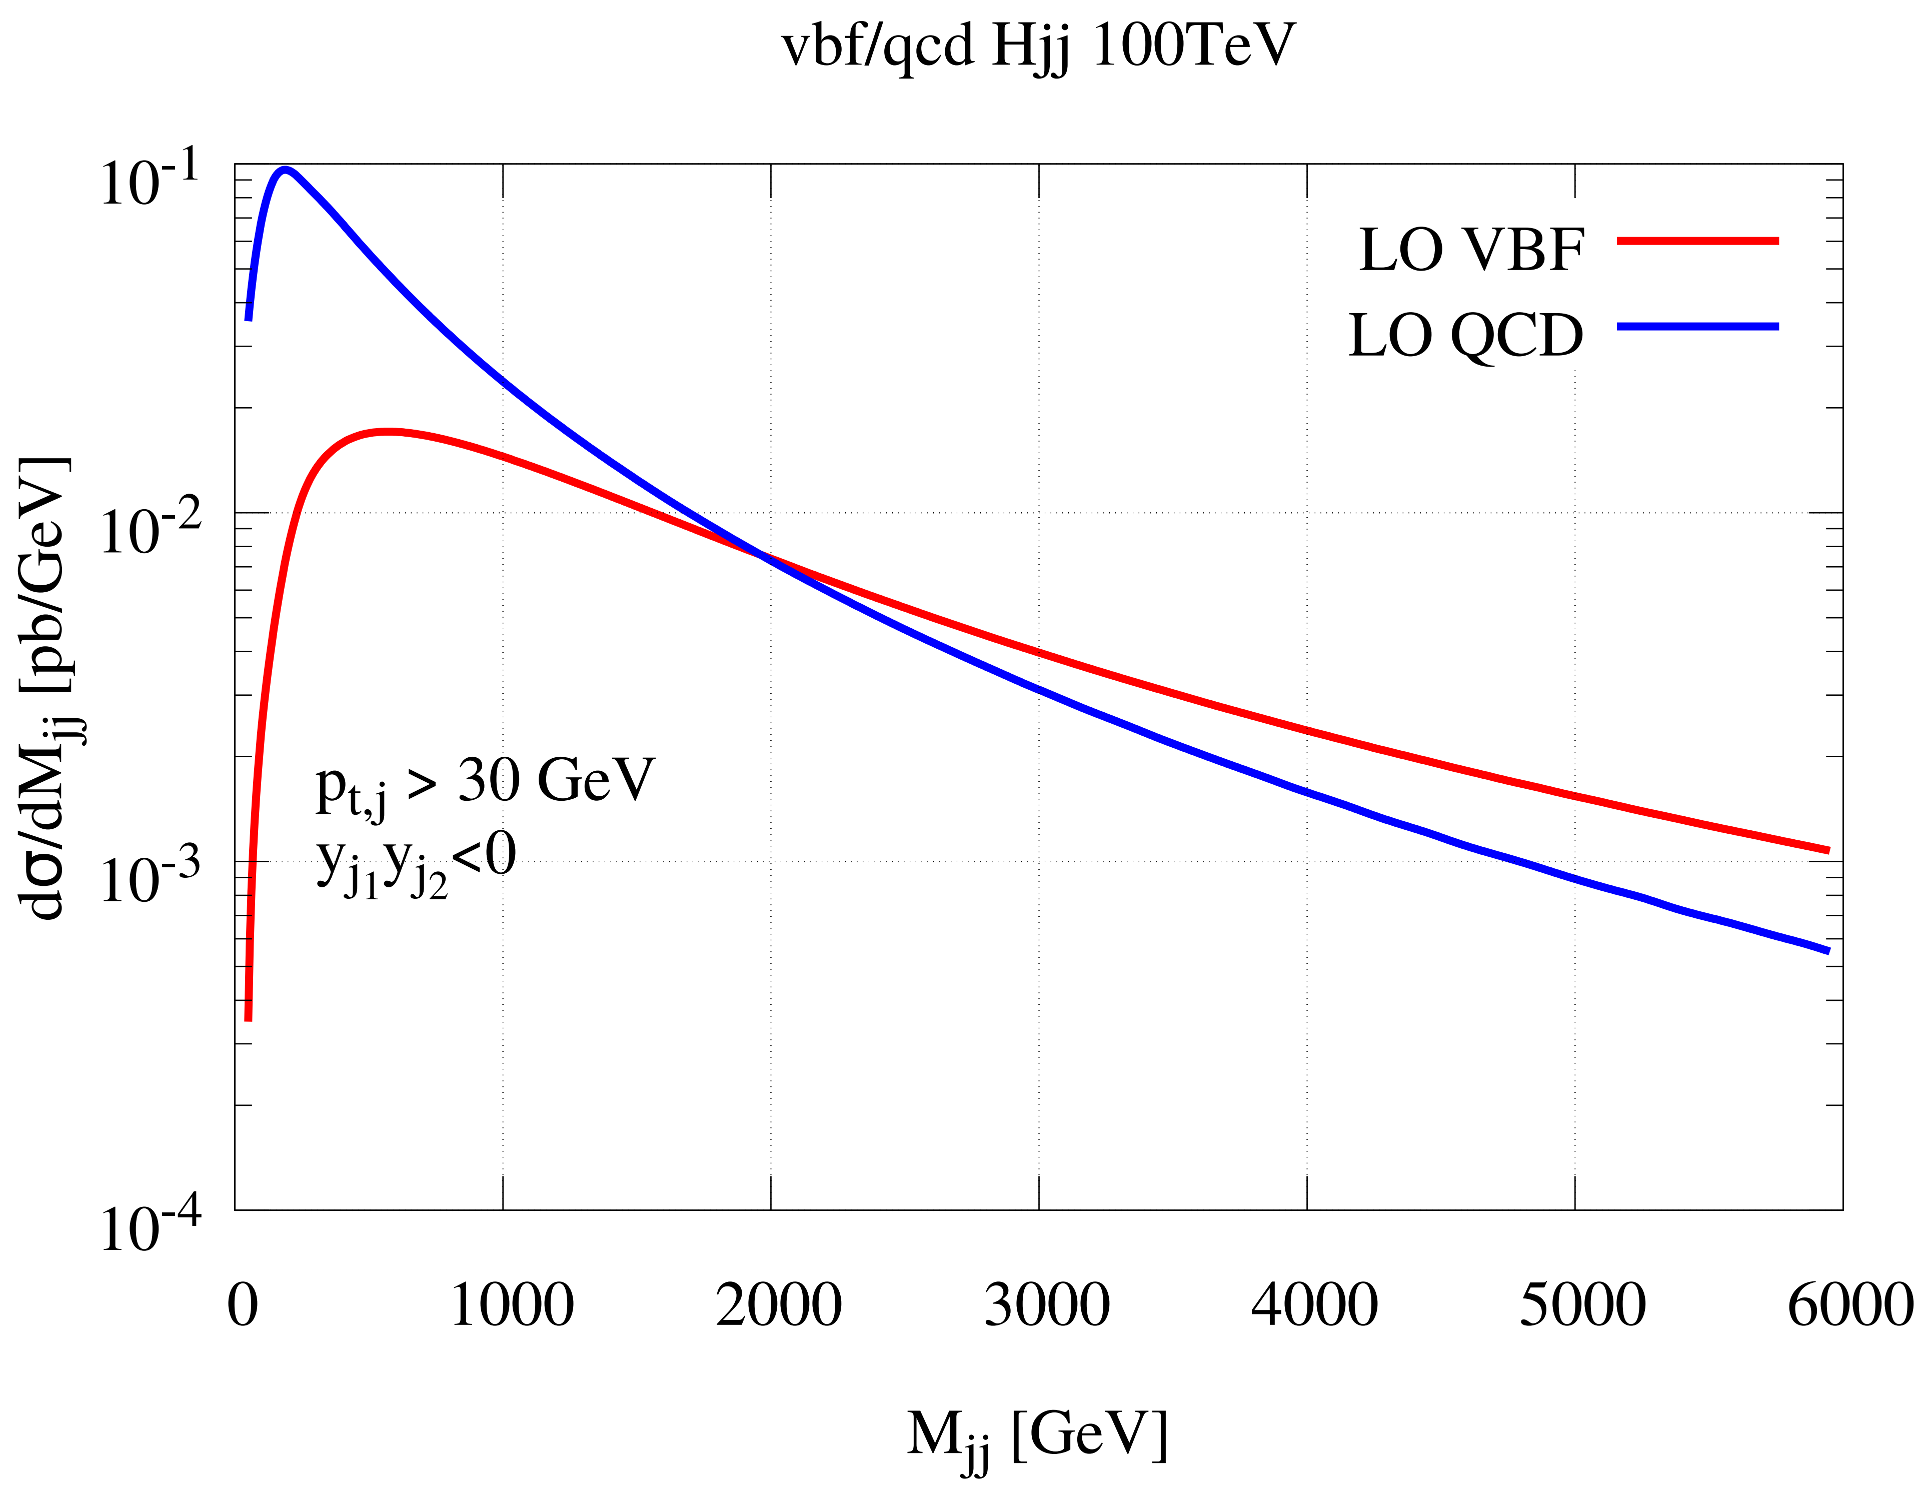
vbf/qcd Hjj 100TeV
LO VBF
LO QCD
$p_{t,j}$ > 30 GeV
$y_{j_1}y_{j_2}<0$
$d\sigma/dM_{jj}$ [pb/GeV]
$10^{-1}$
$10^{-2}$
$10^{-3}$
$10^{-4}$
0
1000
2000
3000
4000
5000
6000
$M_{jj}$ [GeV]

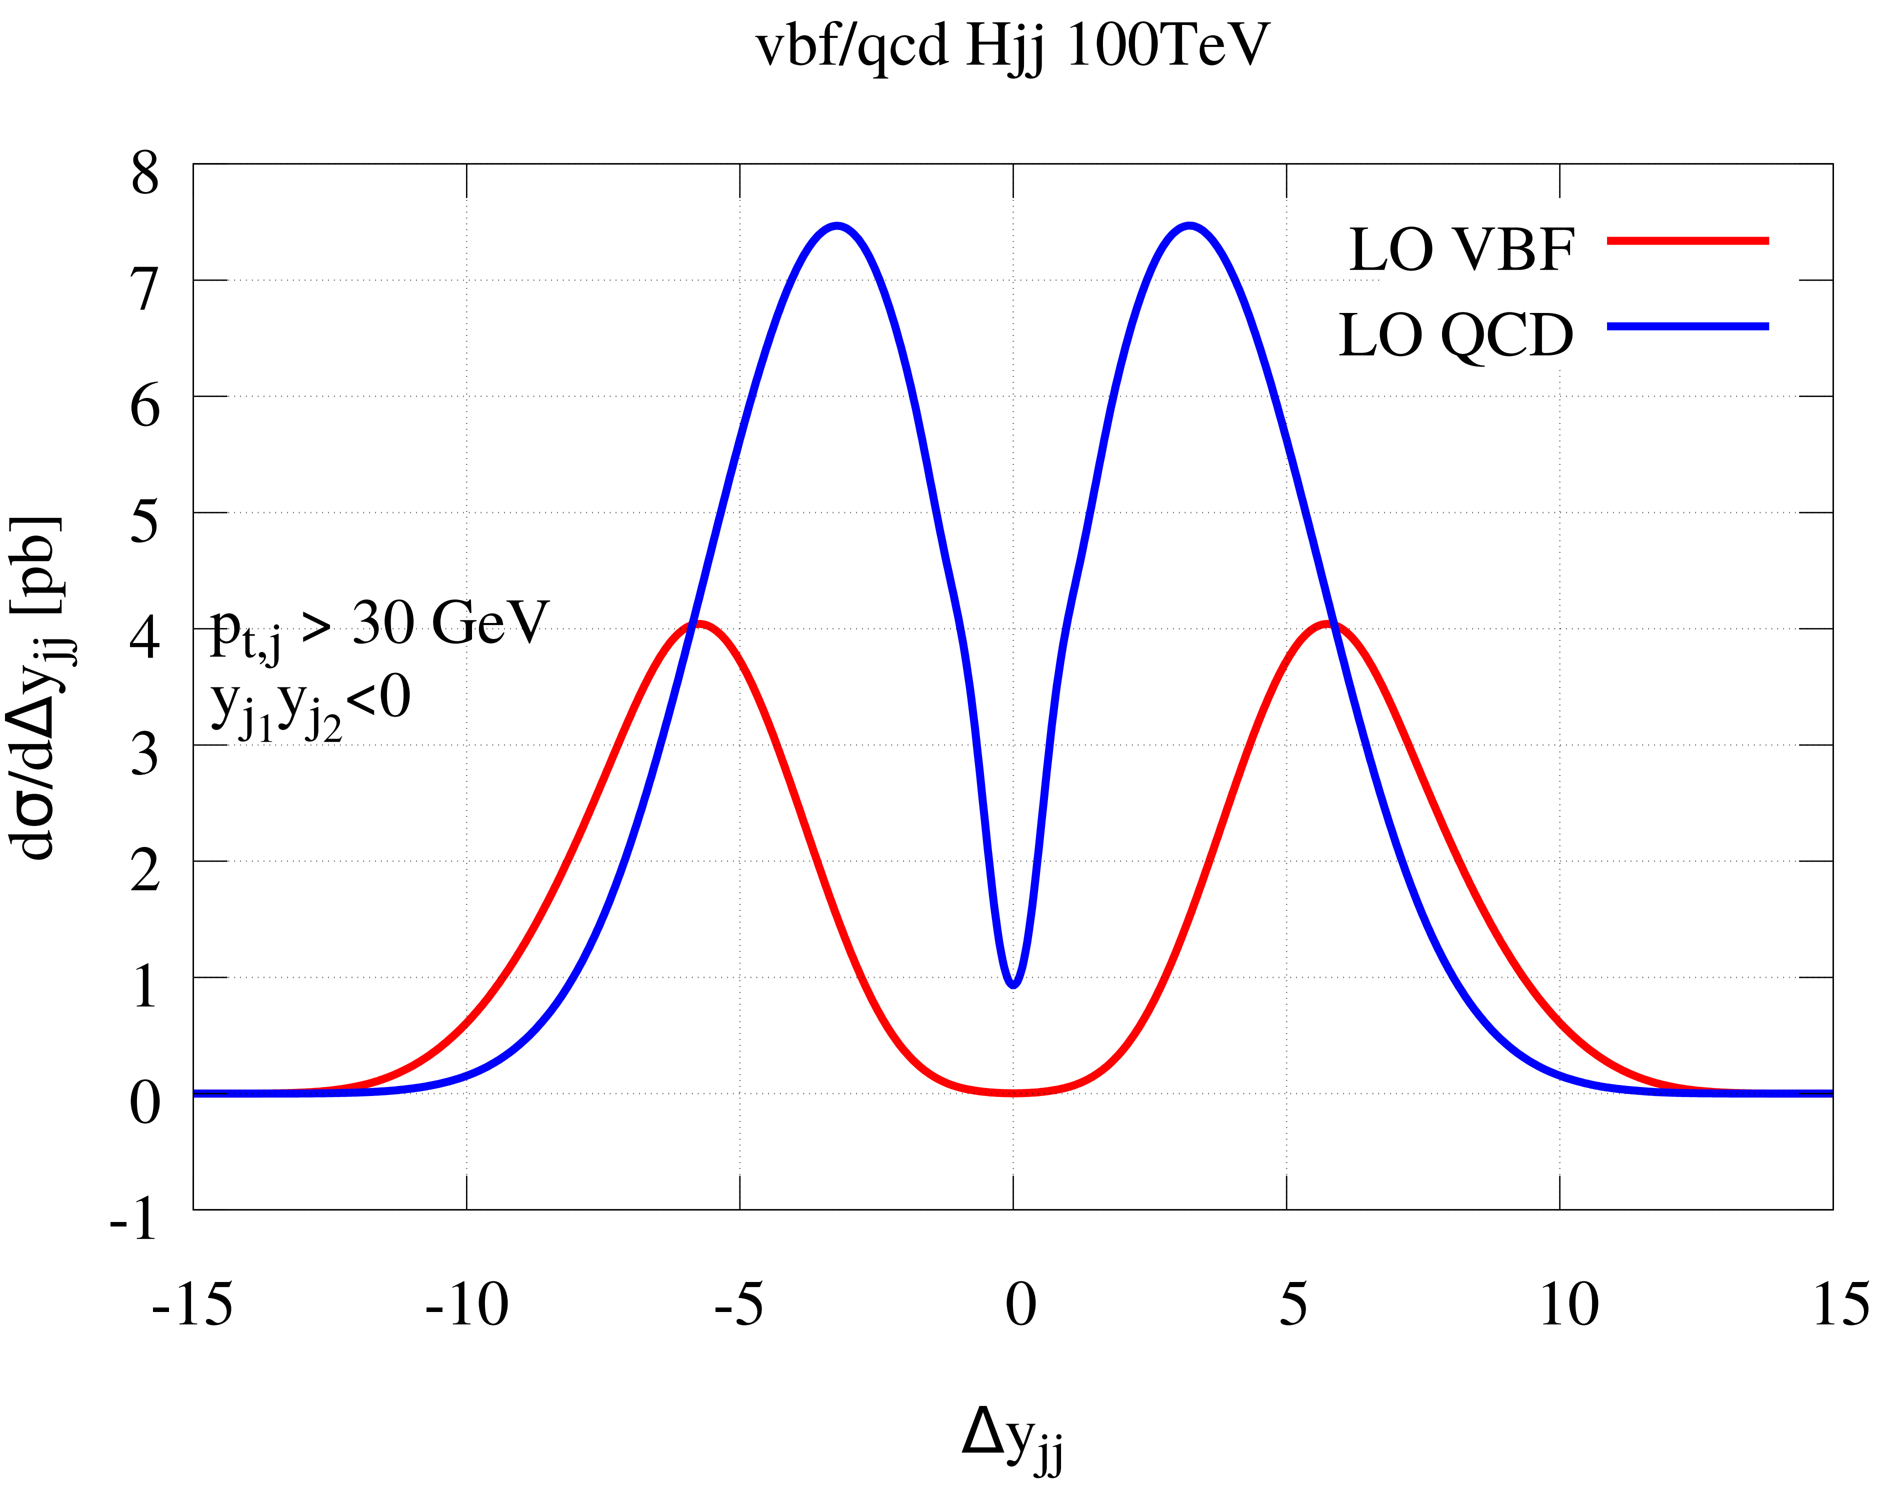

vbf/qcd Hjj 100TeV
dσ/dΔy_jj [pb]
Δy_jj
LO VBF
LO QCD
p_t,j > 30 GeV
y_j1 y_j2 <0
8
7
6
5
4
3
2
1
0
-1
-15
-10
-5
0
5
10
15

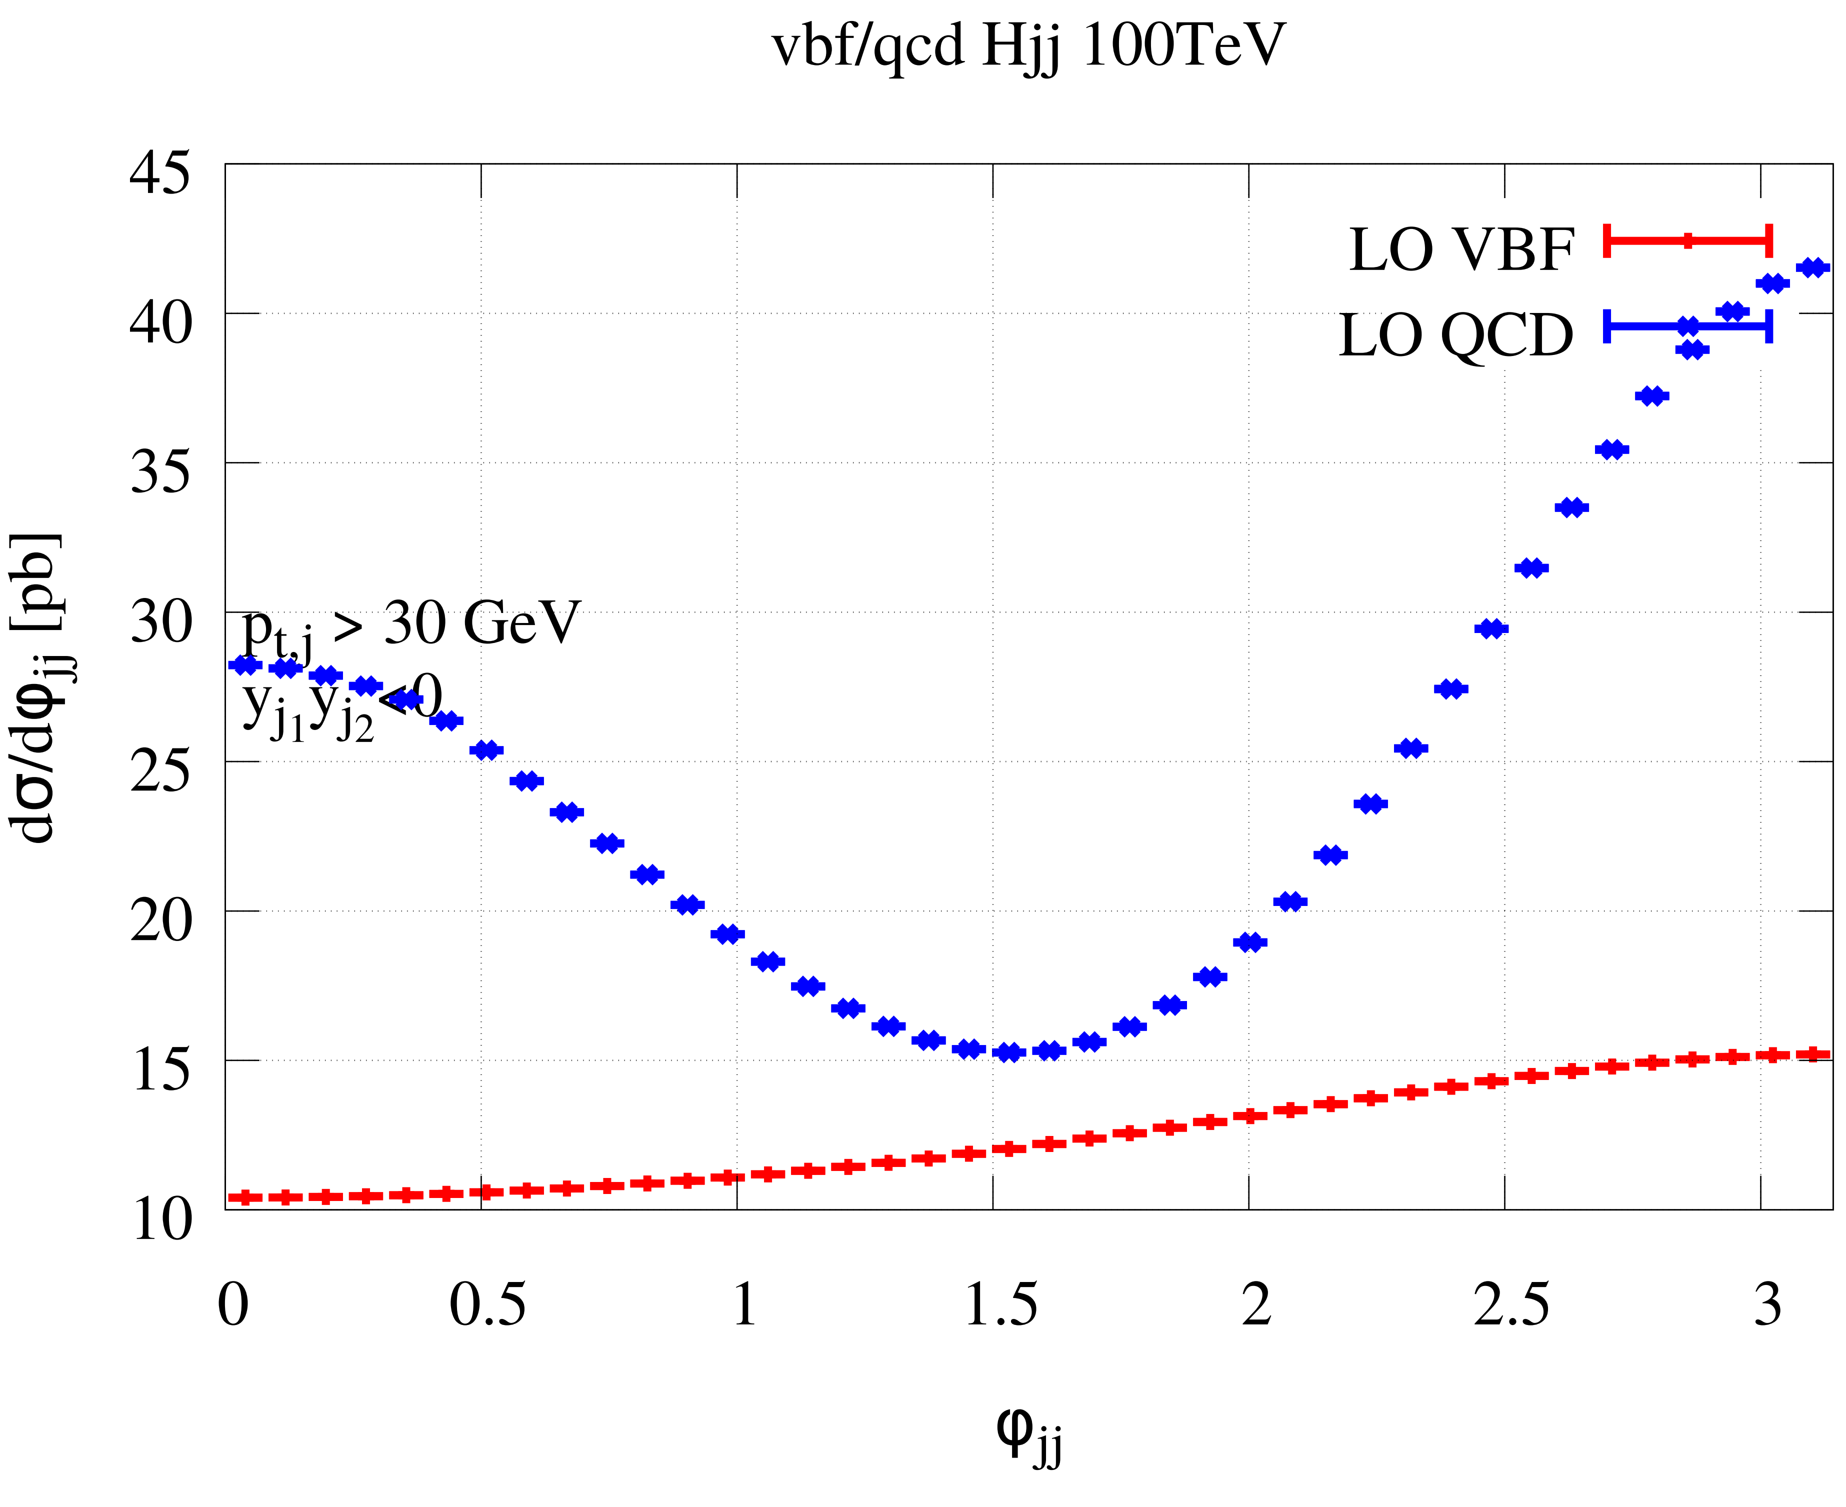

vbf/qcd Hjj 100TeV
LO VBF
LO QCD
$p_{t,j}$ > 30 GeV
$y_{j_1} y_{j_2} < 0$
dσ/dφ$_{jj}$ [pb]
φ$_{jj}$
45
40
35
30
25
20
15
10
0
0.5
1
1.5
2
2.5
3

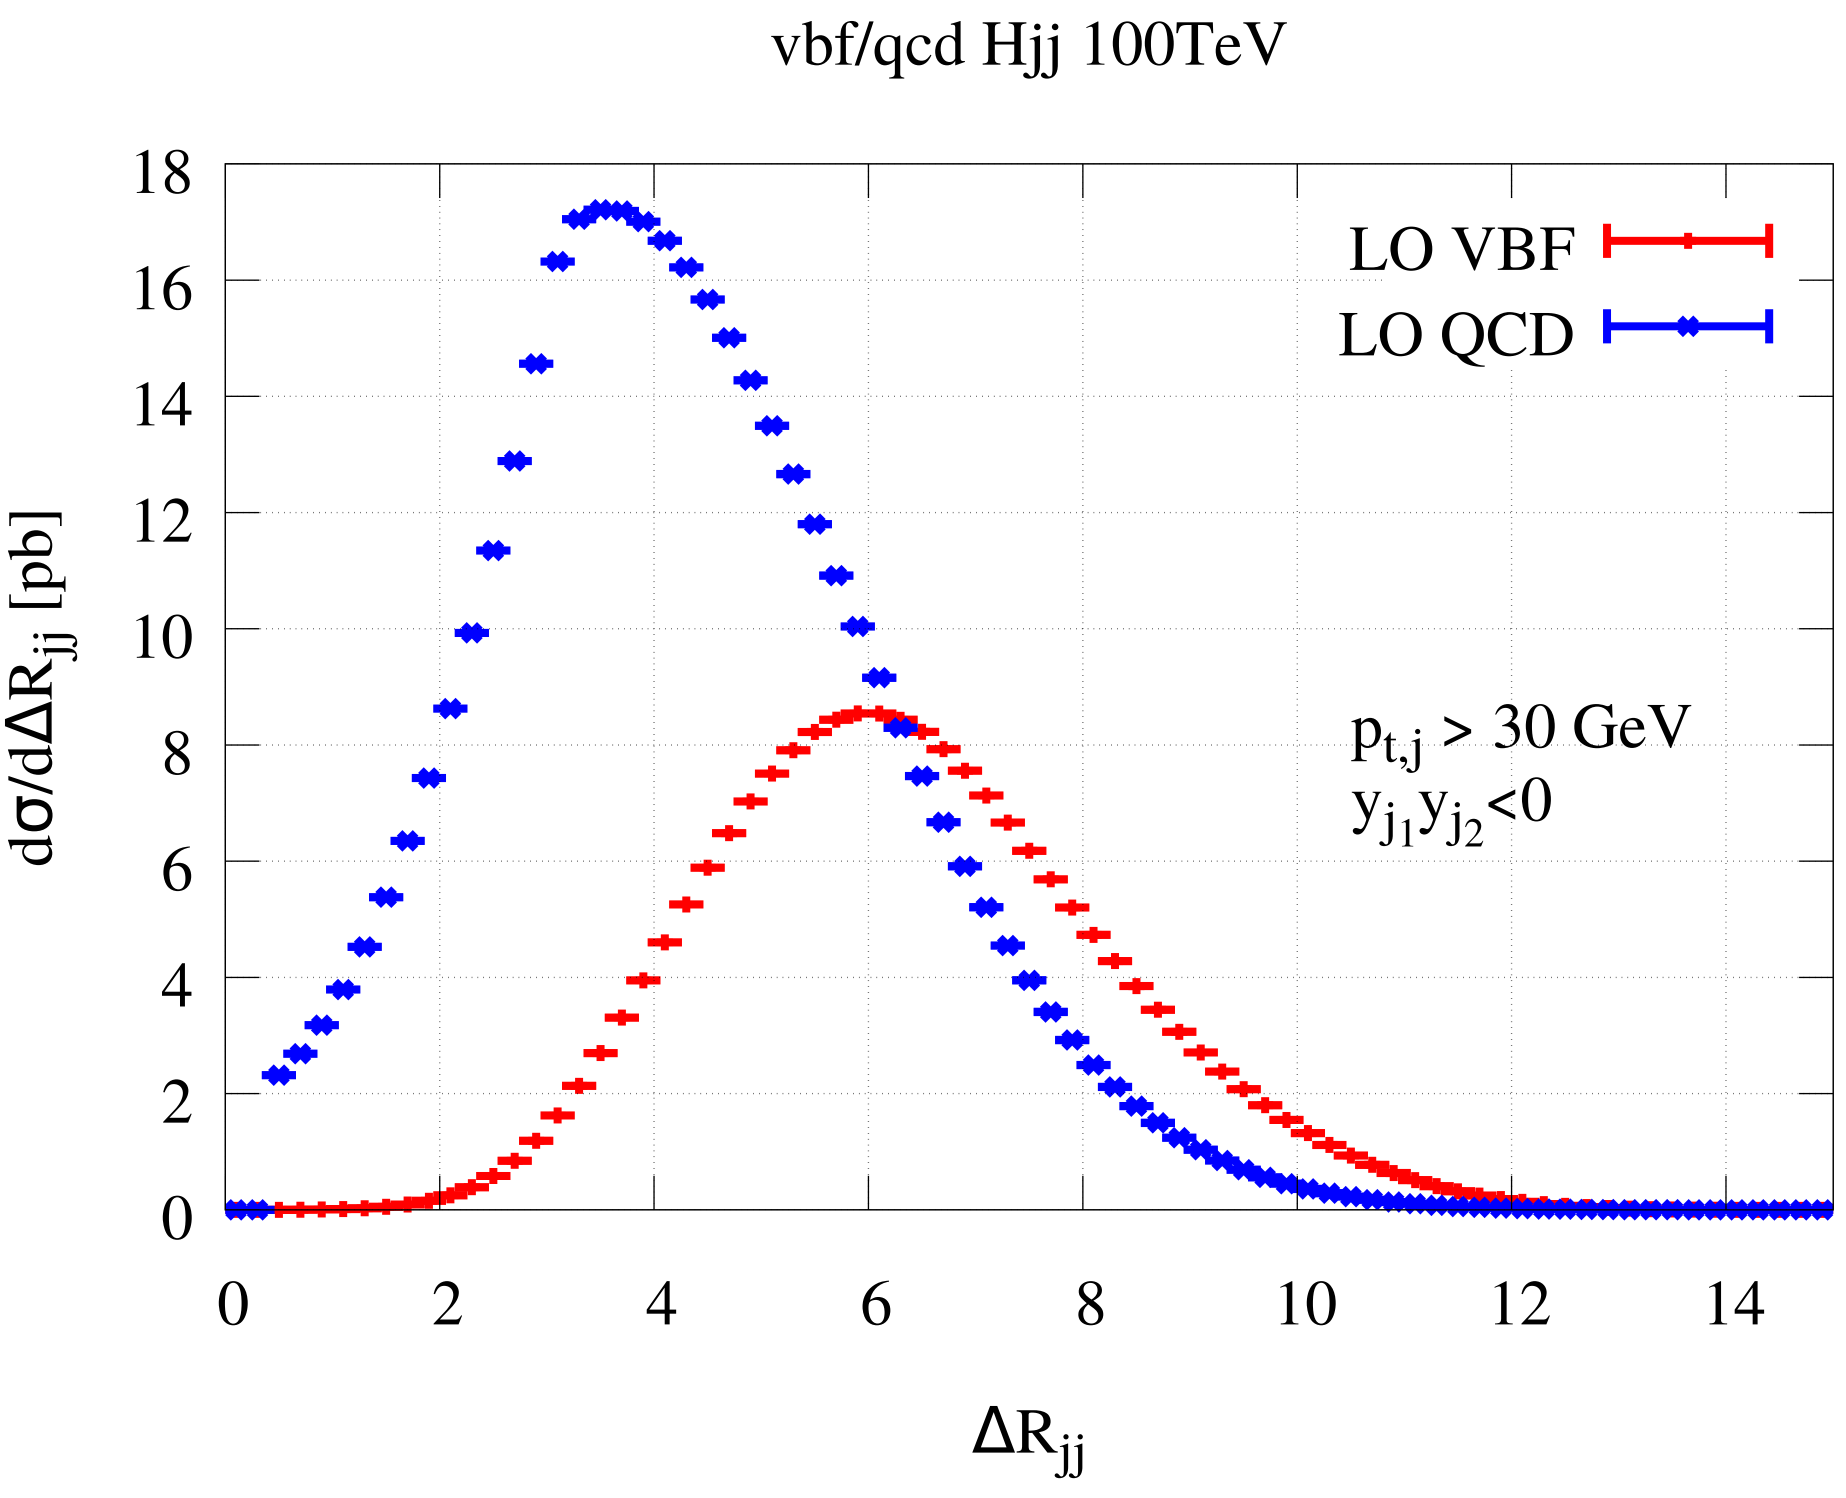

vbf/qcd Hjj 100TeV
LO VBF
LO QCD
$p_{t,j}$ > 30 GeV
$y_{j_1}y_{j_2}<0$
$d\sigma/d\Delta R_{jj}$ [pb]
$\Delta R_{jj}$
0
2
4
6
8
10
12
14
16
18

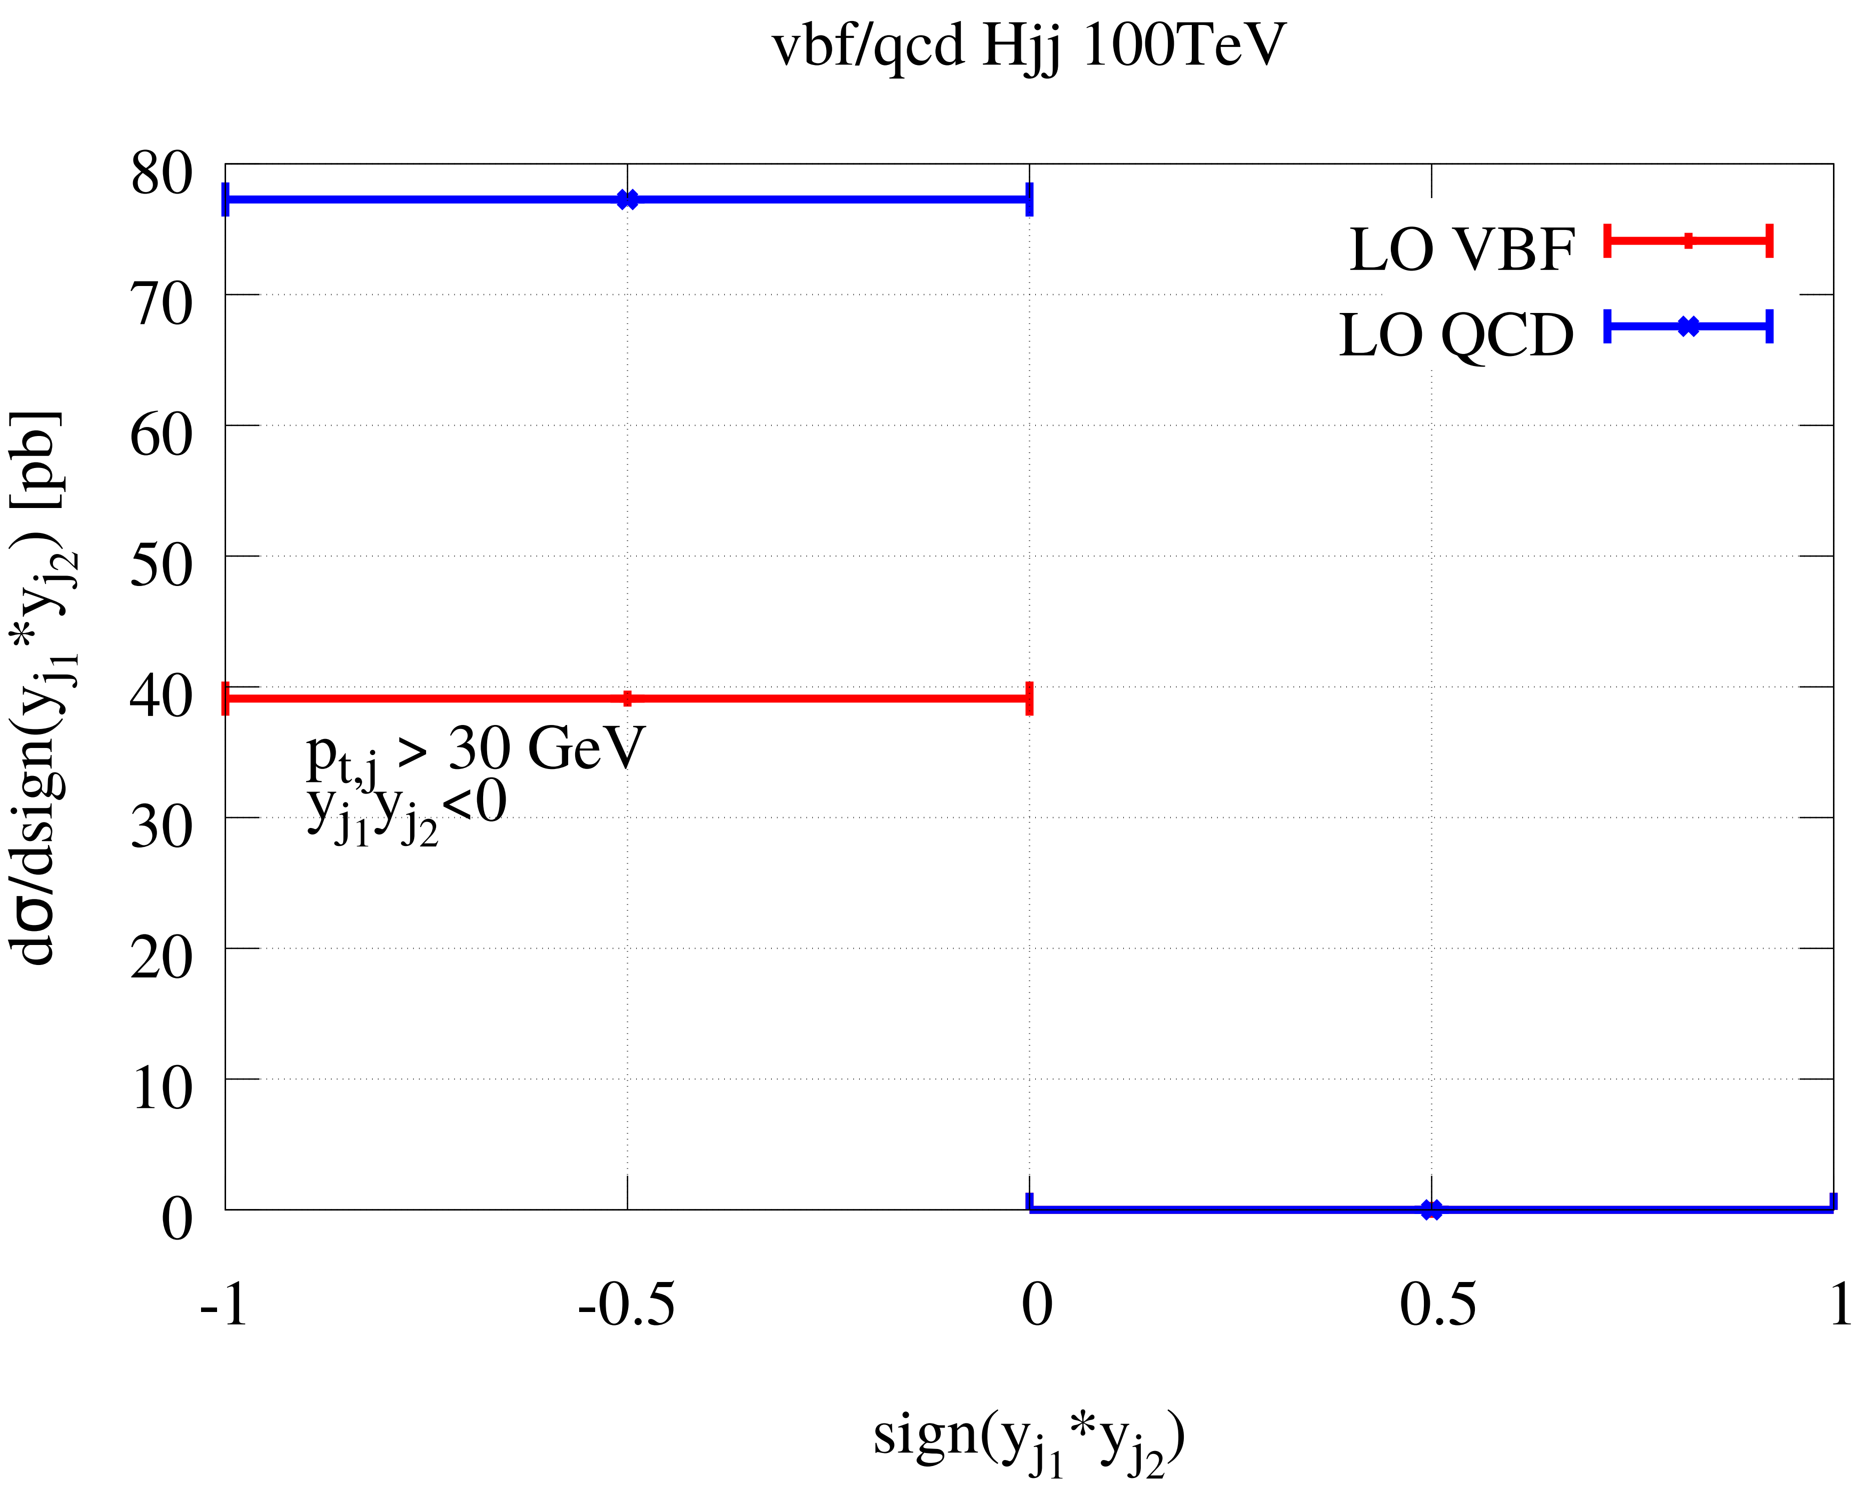

vbf/qcd Hjj 100TeV
LO VBF
LO QCD
$p_{t,j}$ > 30 GeV
$y_{j_1} y_{j_2}$<0
$d\sigma/d\text{sign}(y_{j_1} * y_{j_2})$ [pb]
$\text{sign}(y_{j_1} * y_{j_2})$
80
70
60
50
40
30
20
10
0
-1
-0.5
0
0.5
1

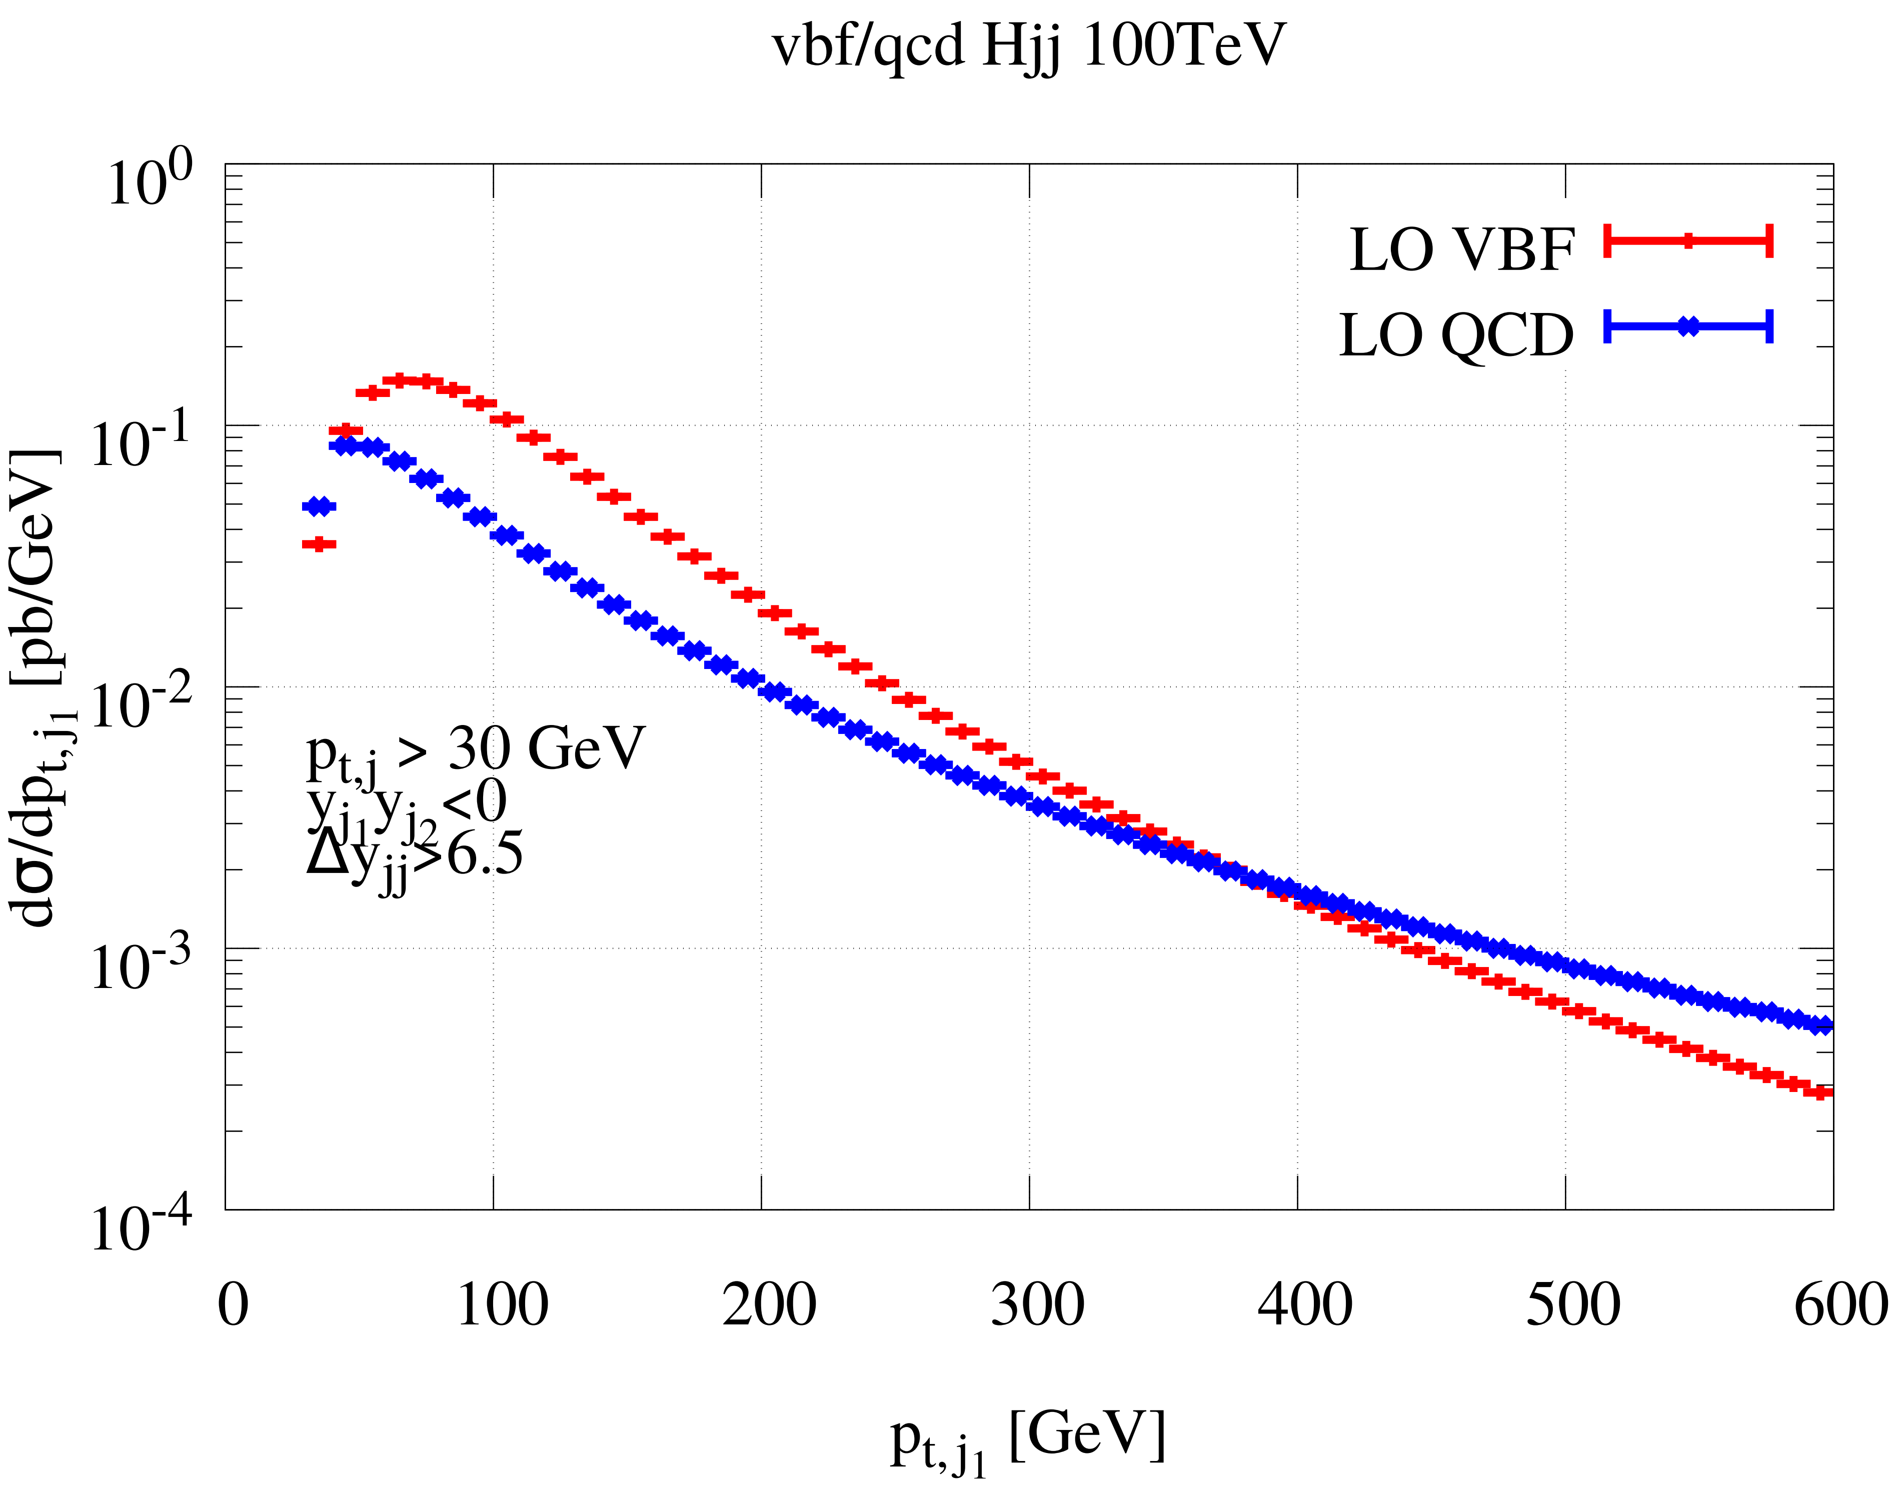

vbf/qcd Hjj 100TeV
LO VBF
LO QCD
$p_{t,j}$ > 30 GeV
$y_{j_1} y_{j_2} < 0$
$\Delta y_{jj} > 6.5$
$d\sigma/dp_{t,j_1}$ [pb/GeV]
$p_{t,j_1}$ [GeV]
$10^0$
$10^{-1}$
$10^{-2}$
$10^{-3}$
$10^{-4}$
0
100
200
300
400
500
600

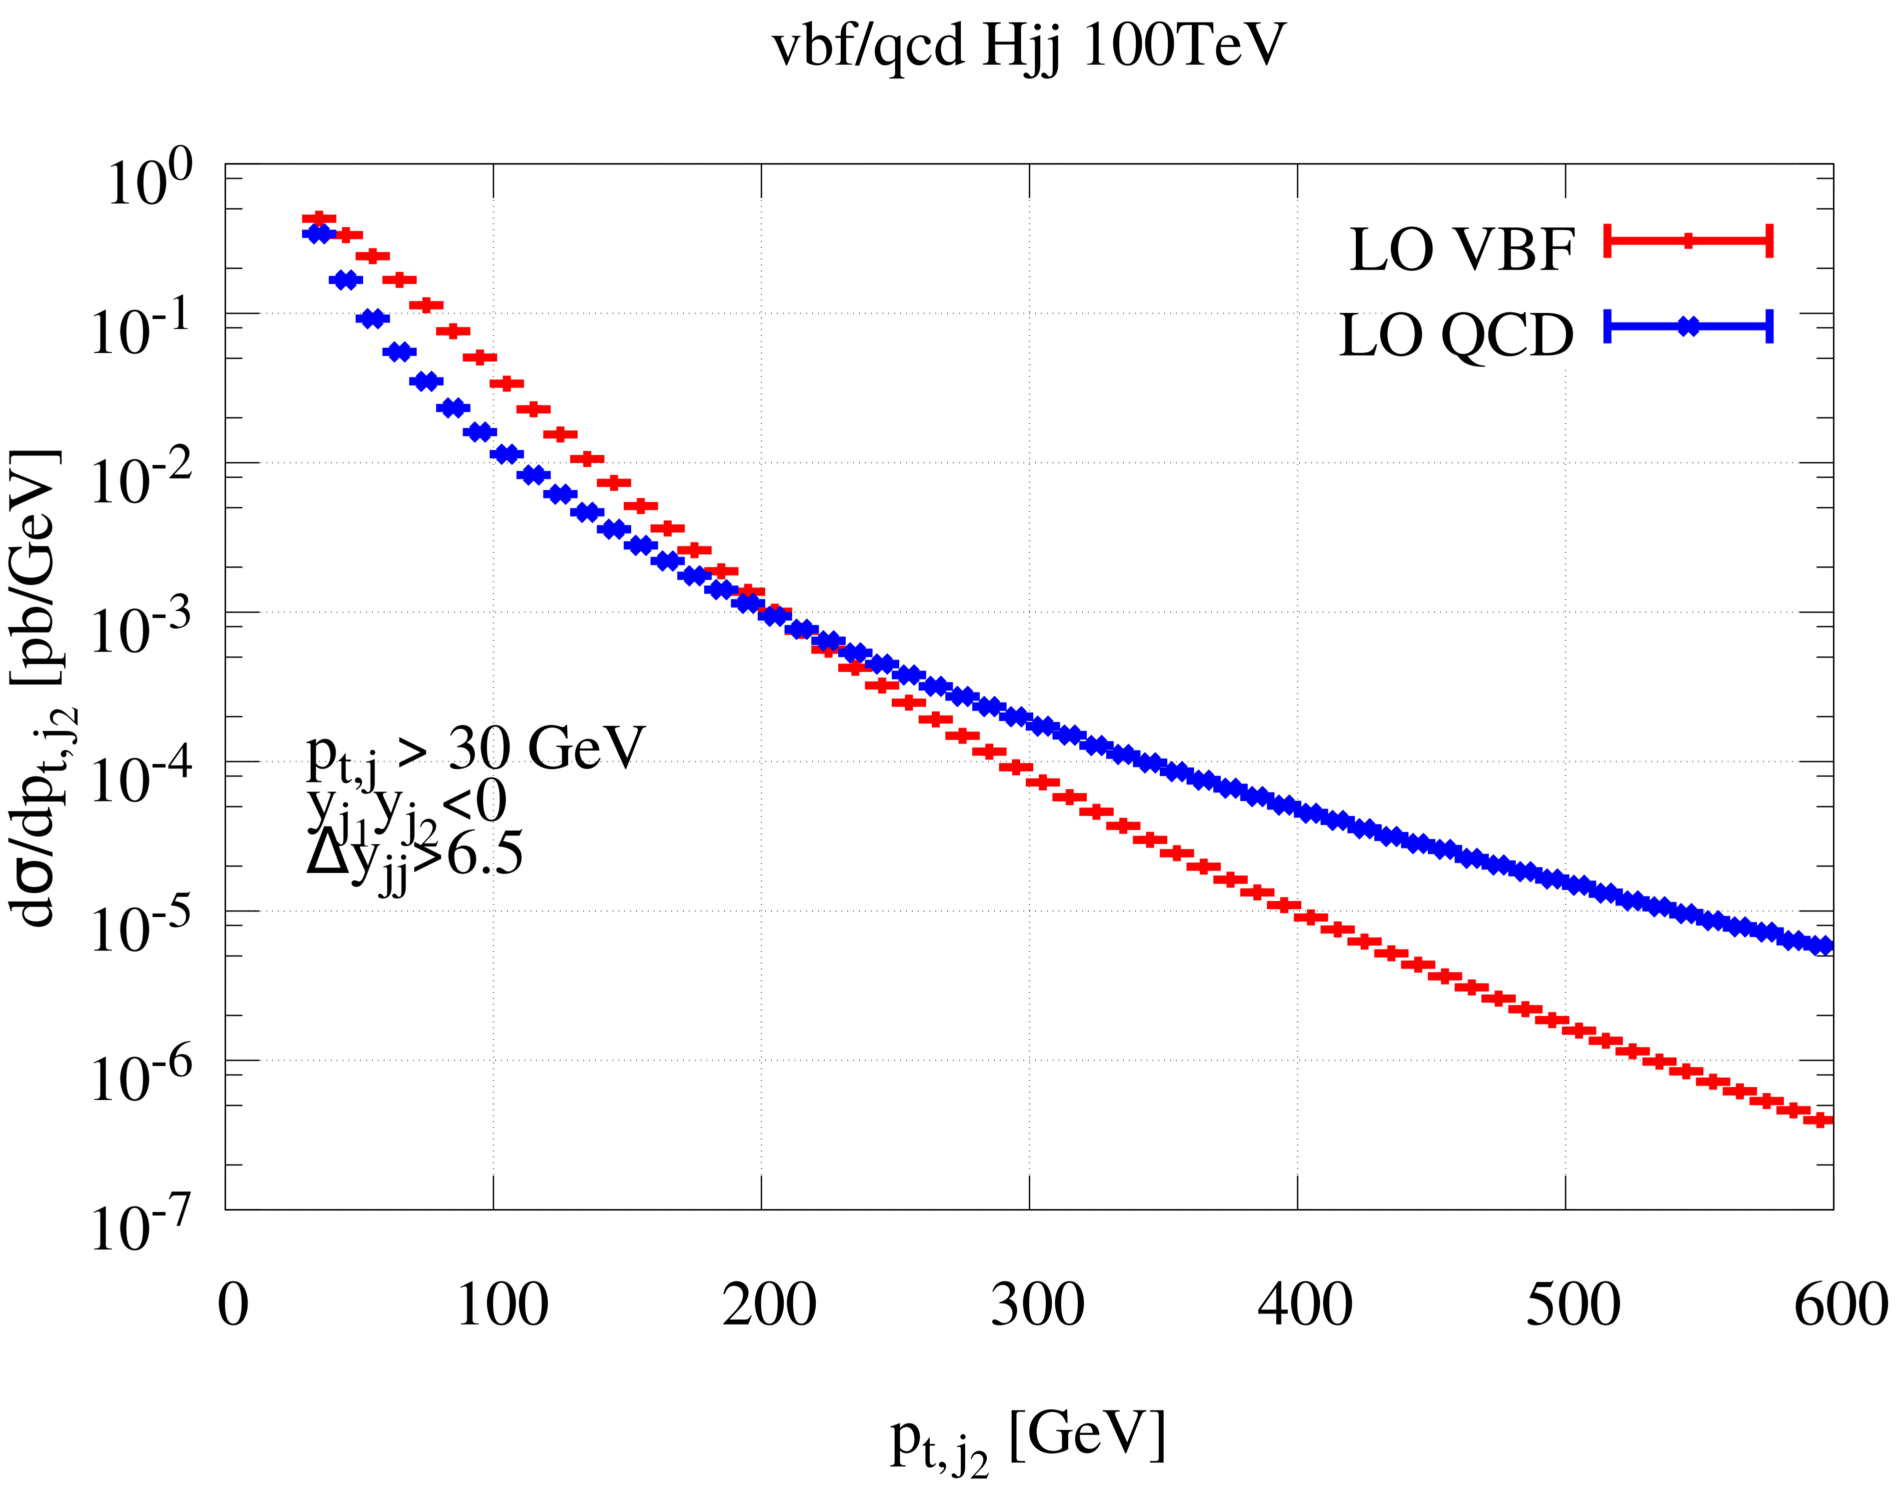

vbf/qcd Hjj 100TeV
LO VBF
LO QCD
$p_{t,j}$ > 30 GeV
$y_{j_1} y_{j_2}$<0
$\Delta y_{jj}$>6.5
$d\sigma/dp_{t,j_2}$ [pb/GeV]
$p_{t,j_2}$ [GeV]
$10^{0}$
$10^{-1}$
$10^{-2}$
$10^{-3}$
$10^{-4}$
$10^{-5}$
$10^{-6}$
$10^{-7}$
0
100
200
300
400
500
600

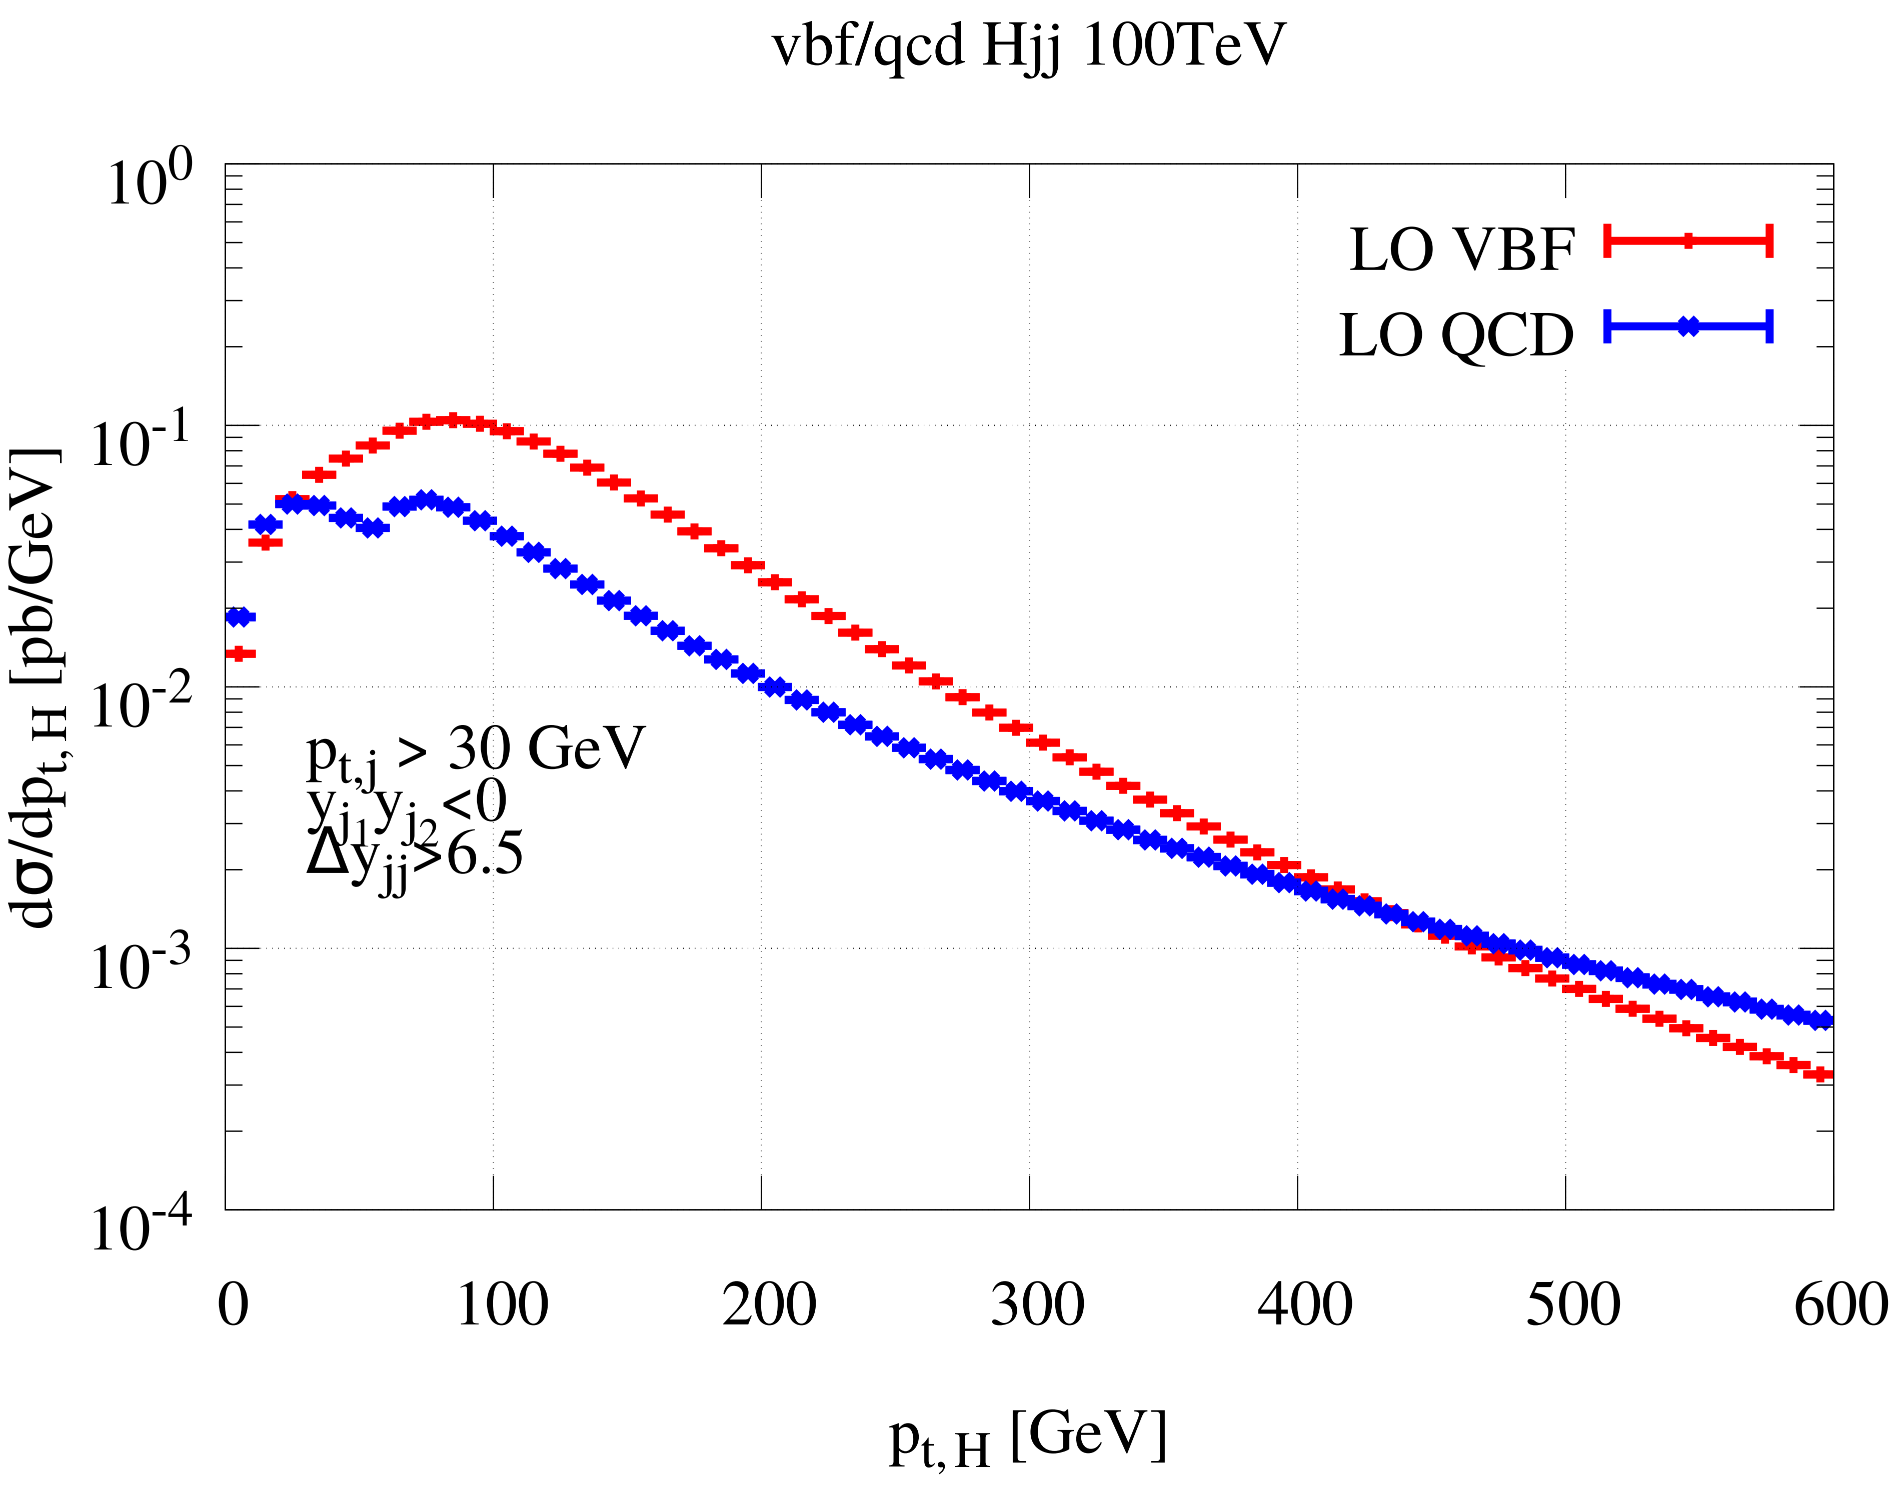

vbf/qcd Hjj 100TeV
LO VBF
LO QCD
$p_{t,j}$ > 30 GeV
$y_{j_1} y_{j_2} < 0$
$\Delta y_{jj} > 6.5$
$d\sigma/dp_{t,H}$ [pb/GeV]
$p_{t,H}$ [GeV]
$10^0$
$10^{-1}$
$10^{-2}$
$10^{-3}$
$10^{-4}$
0
100
200
300
400
500
600

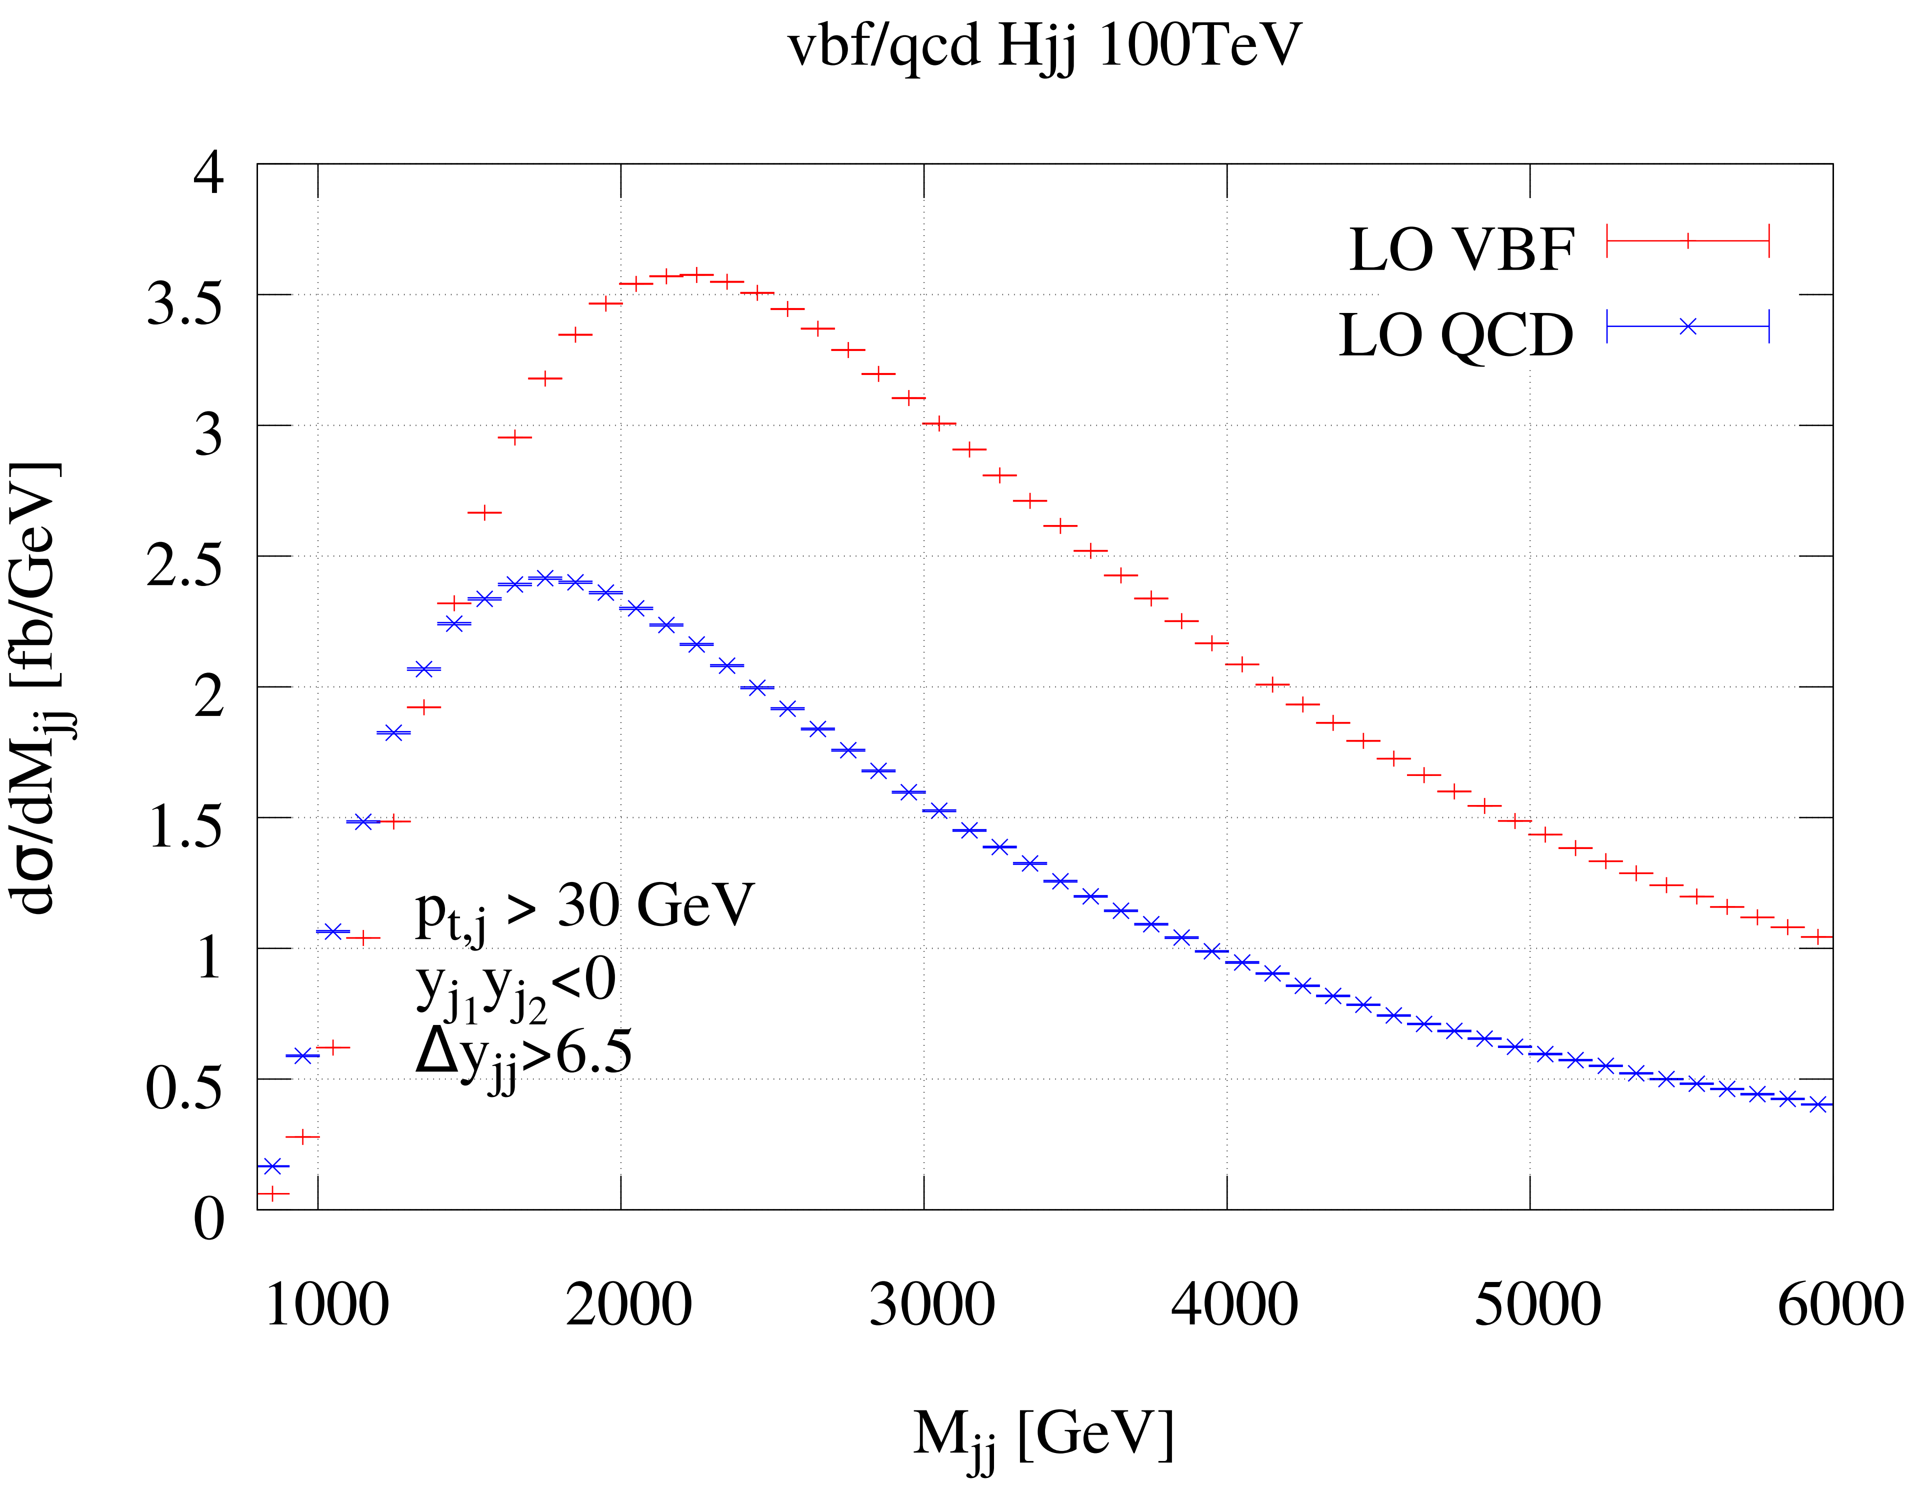

vbf/qcd Hjj 100TeV
LO VBF
LO QCD
$p_{t,j}$ > 30 GeV
$y_{j_1}y_{j_2}<0$
$\Delta y_{jj}>6.5$
$d\sigma/dM_{jj}$ [fb/GeV]
$M_{jj}$ [GeV]
0
0.5
1
1.5
2
2.5
3
3.5
4
1000
2000
3000
4000
5000
6000

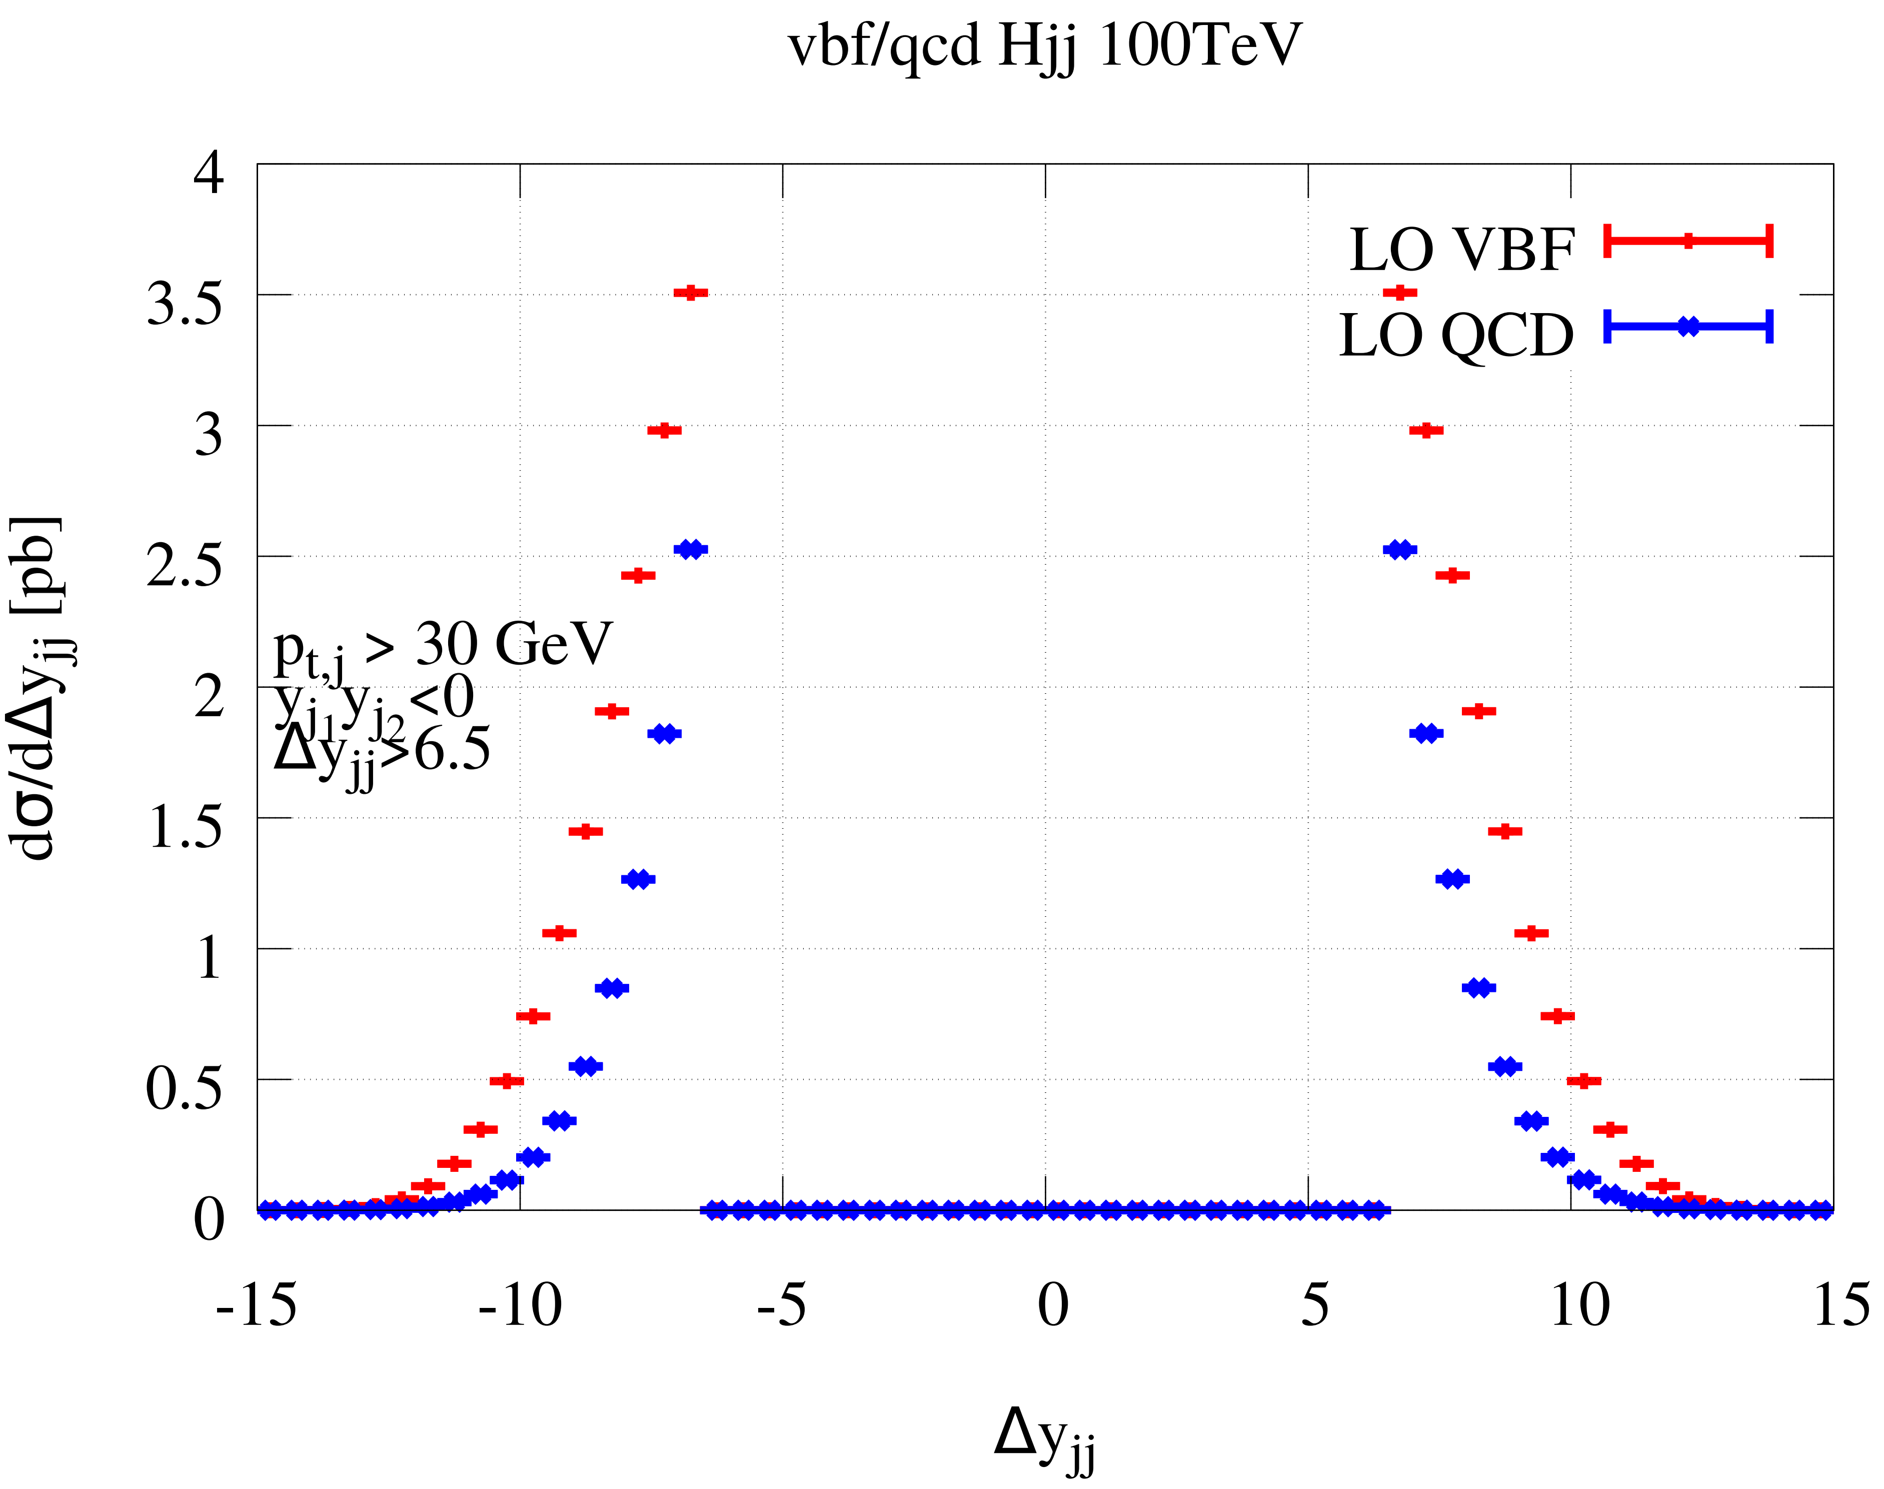

vbf/qcd Hjj 100TeV
LO VBF
LO QCD
$p_{t,j}$ > 30 GeV
$y_{j_1} y_{j_2}$<0
$\Delta y_{jj}$>6.5
$d\sigma/d\Delta y_{jj}$ [pb]
$\Delta y_{jj}$
4
3.5
3
2.5
2
1.5
1
0.5
0
-15
-10
-5
0
5
10
15

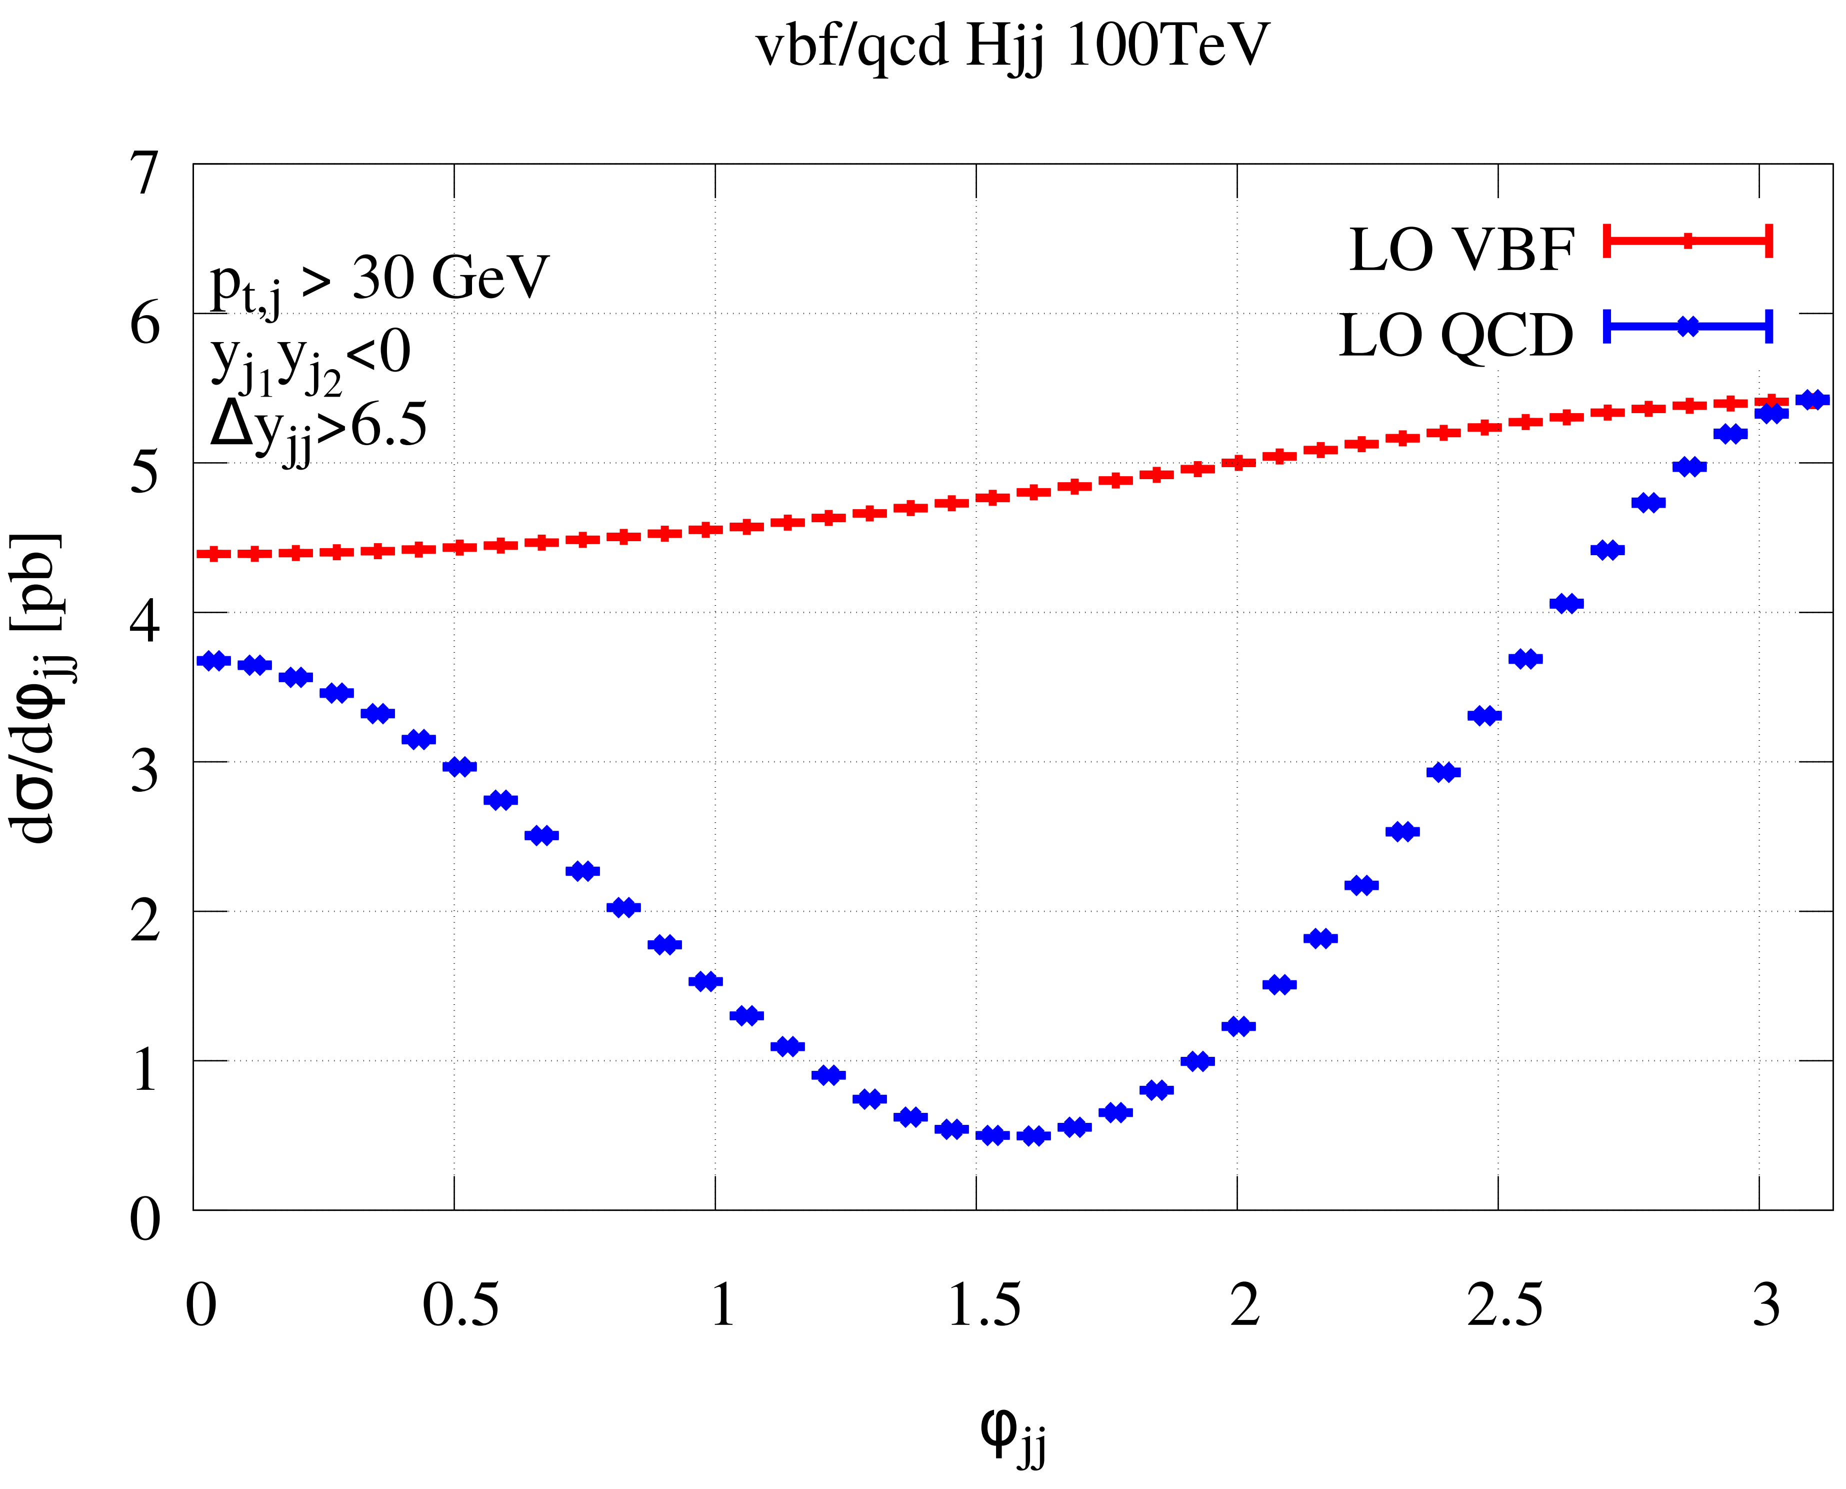

vbf/qcd Hjj 100TeV
$p_{t,j}$ > 30 GeV
$y_{j_1}y_{j_2}<0$
$\Delta y_{jj}>6.5$
LO VBF
LO QCD
$d\sigma/d\varphi_{jj}$ [pb]
$\varphi_{jj}$
0
1
2
3
4
5
6
7
0.5
1.5
2.5

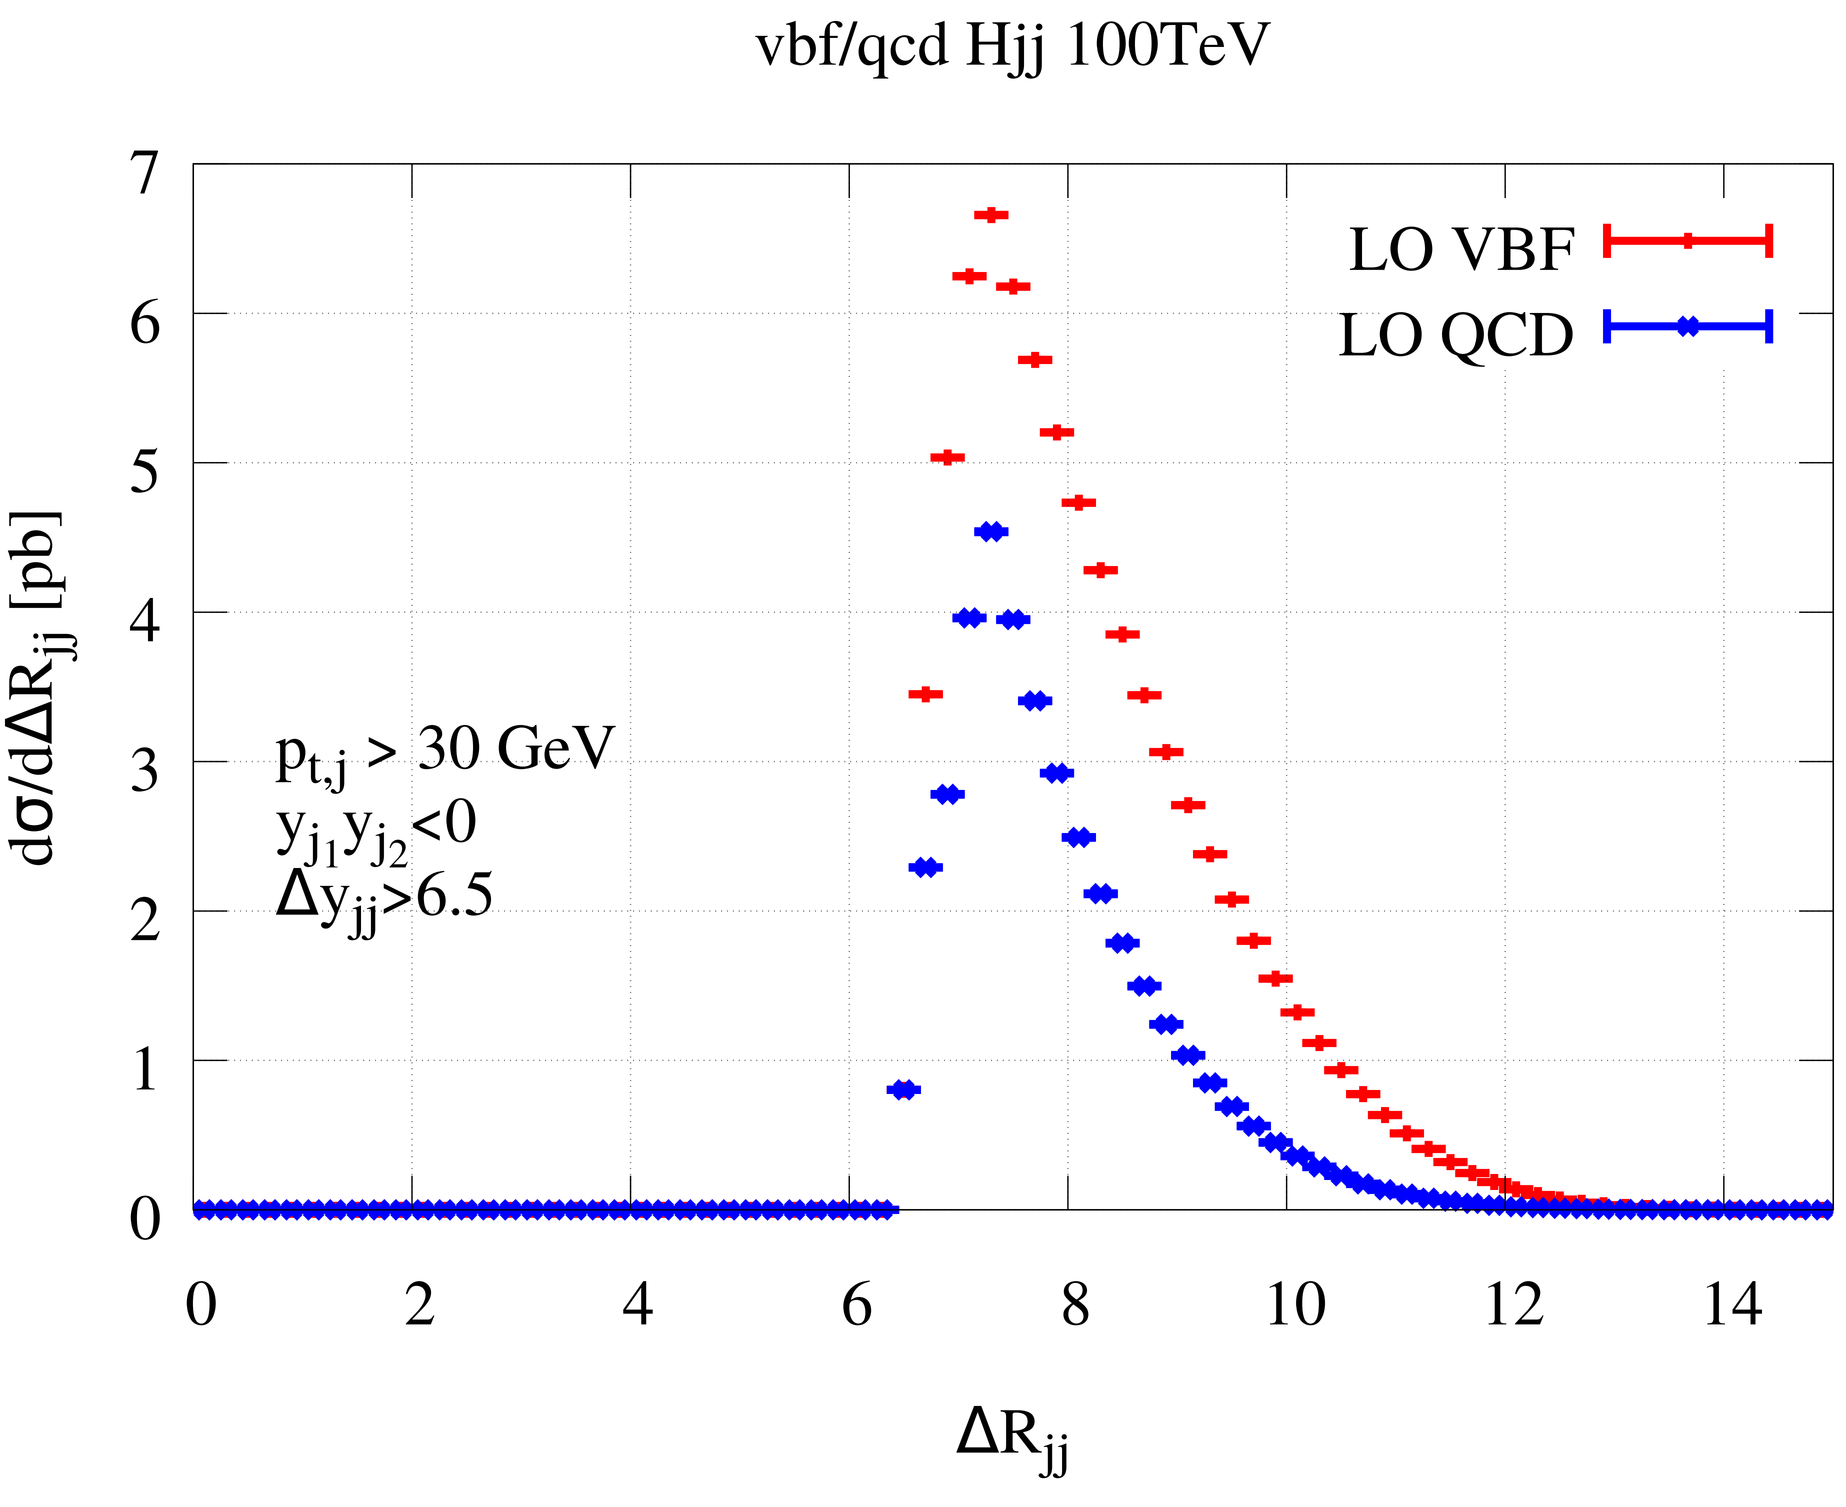

vbf/qcd Hjj 100TeV
LO VBF
LO QCD
$p_{t,j}$ > 30 GeV
$y_{j_1}y_{j_2}<0$
$\Delta y_{jj}>6.5$
$d\sigma/d\Delta R_{jj}$ [pb]
$\Delta R_{jj}$
0
1
2
3
4
5
6
7
0
2
4
6
8
10
12
14

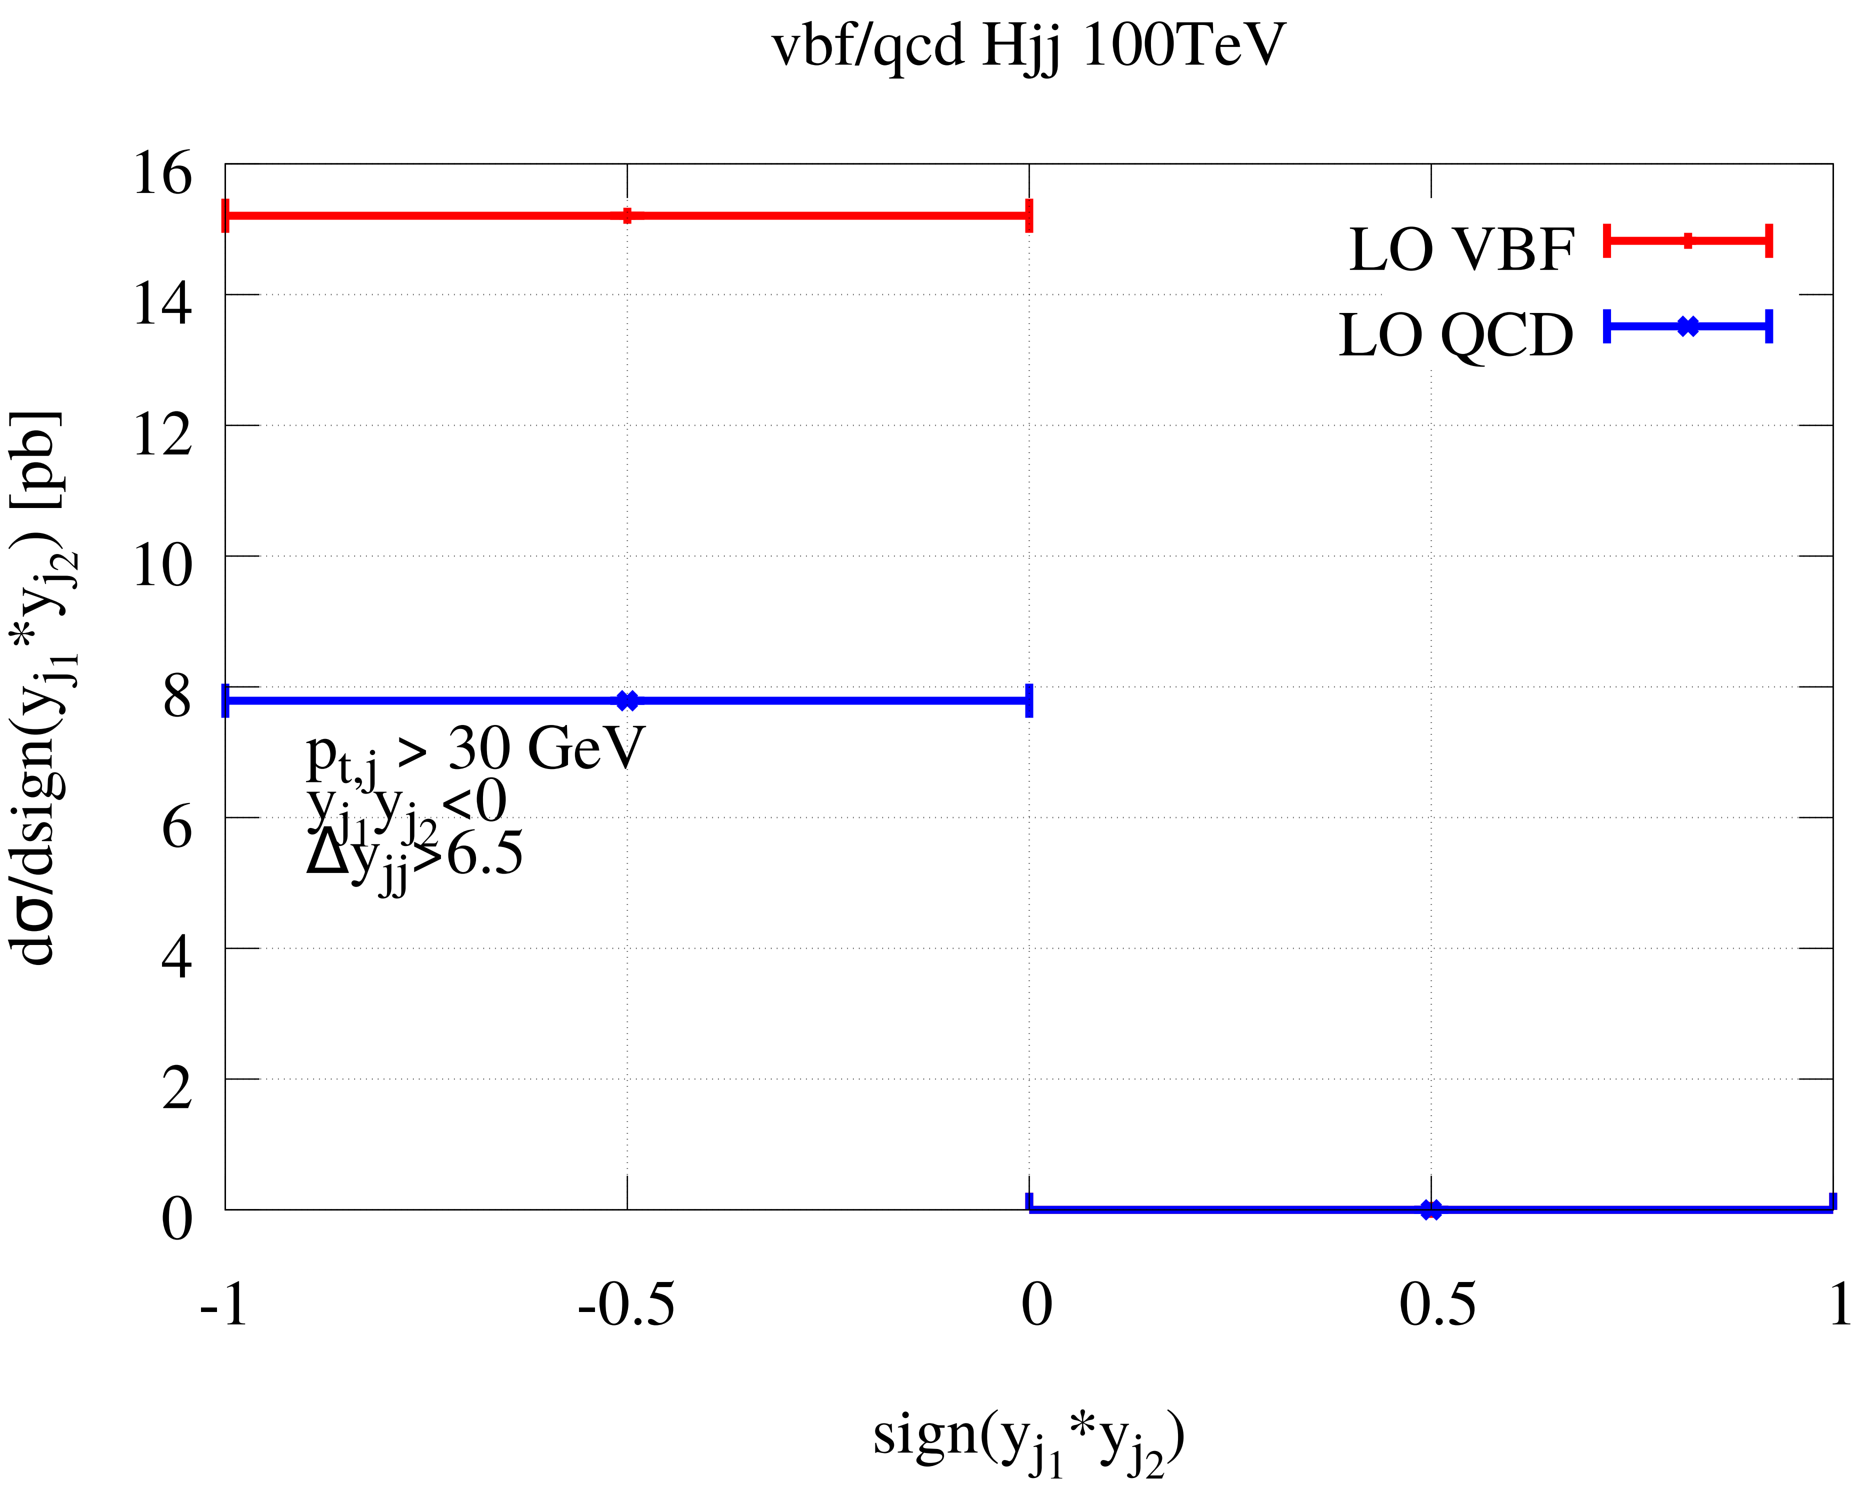

vbf/qcd Hjj 100TeV
LO VBF
LO QCD
$p_{t,j}$ > 30 GeV
$y_{j_1} y_{j_2}$<0
$\Delta y_{jj}$>6.5
$d\sigma/dsign(y_{j_1}*y_{j_2})$ [pb]
$sign(y_{j_1}*y_{j_2})$
16
14
12
10
8
6
4
2
0
-1
-0.5
0
0.5
1

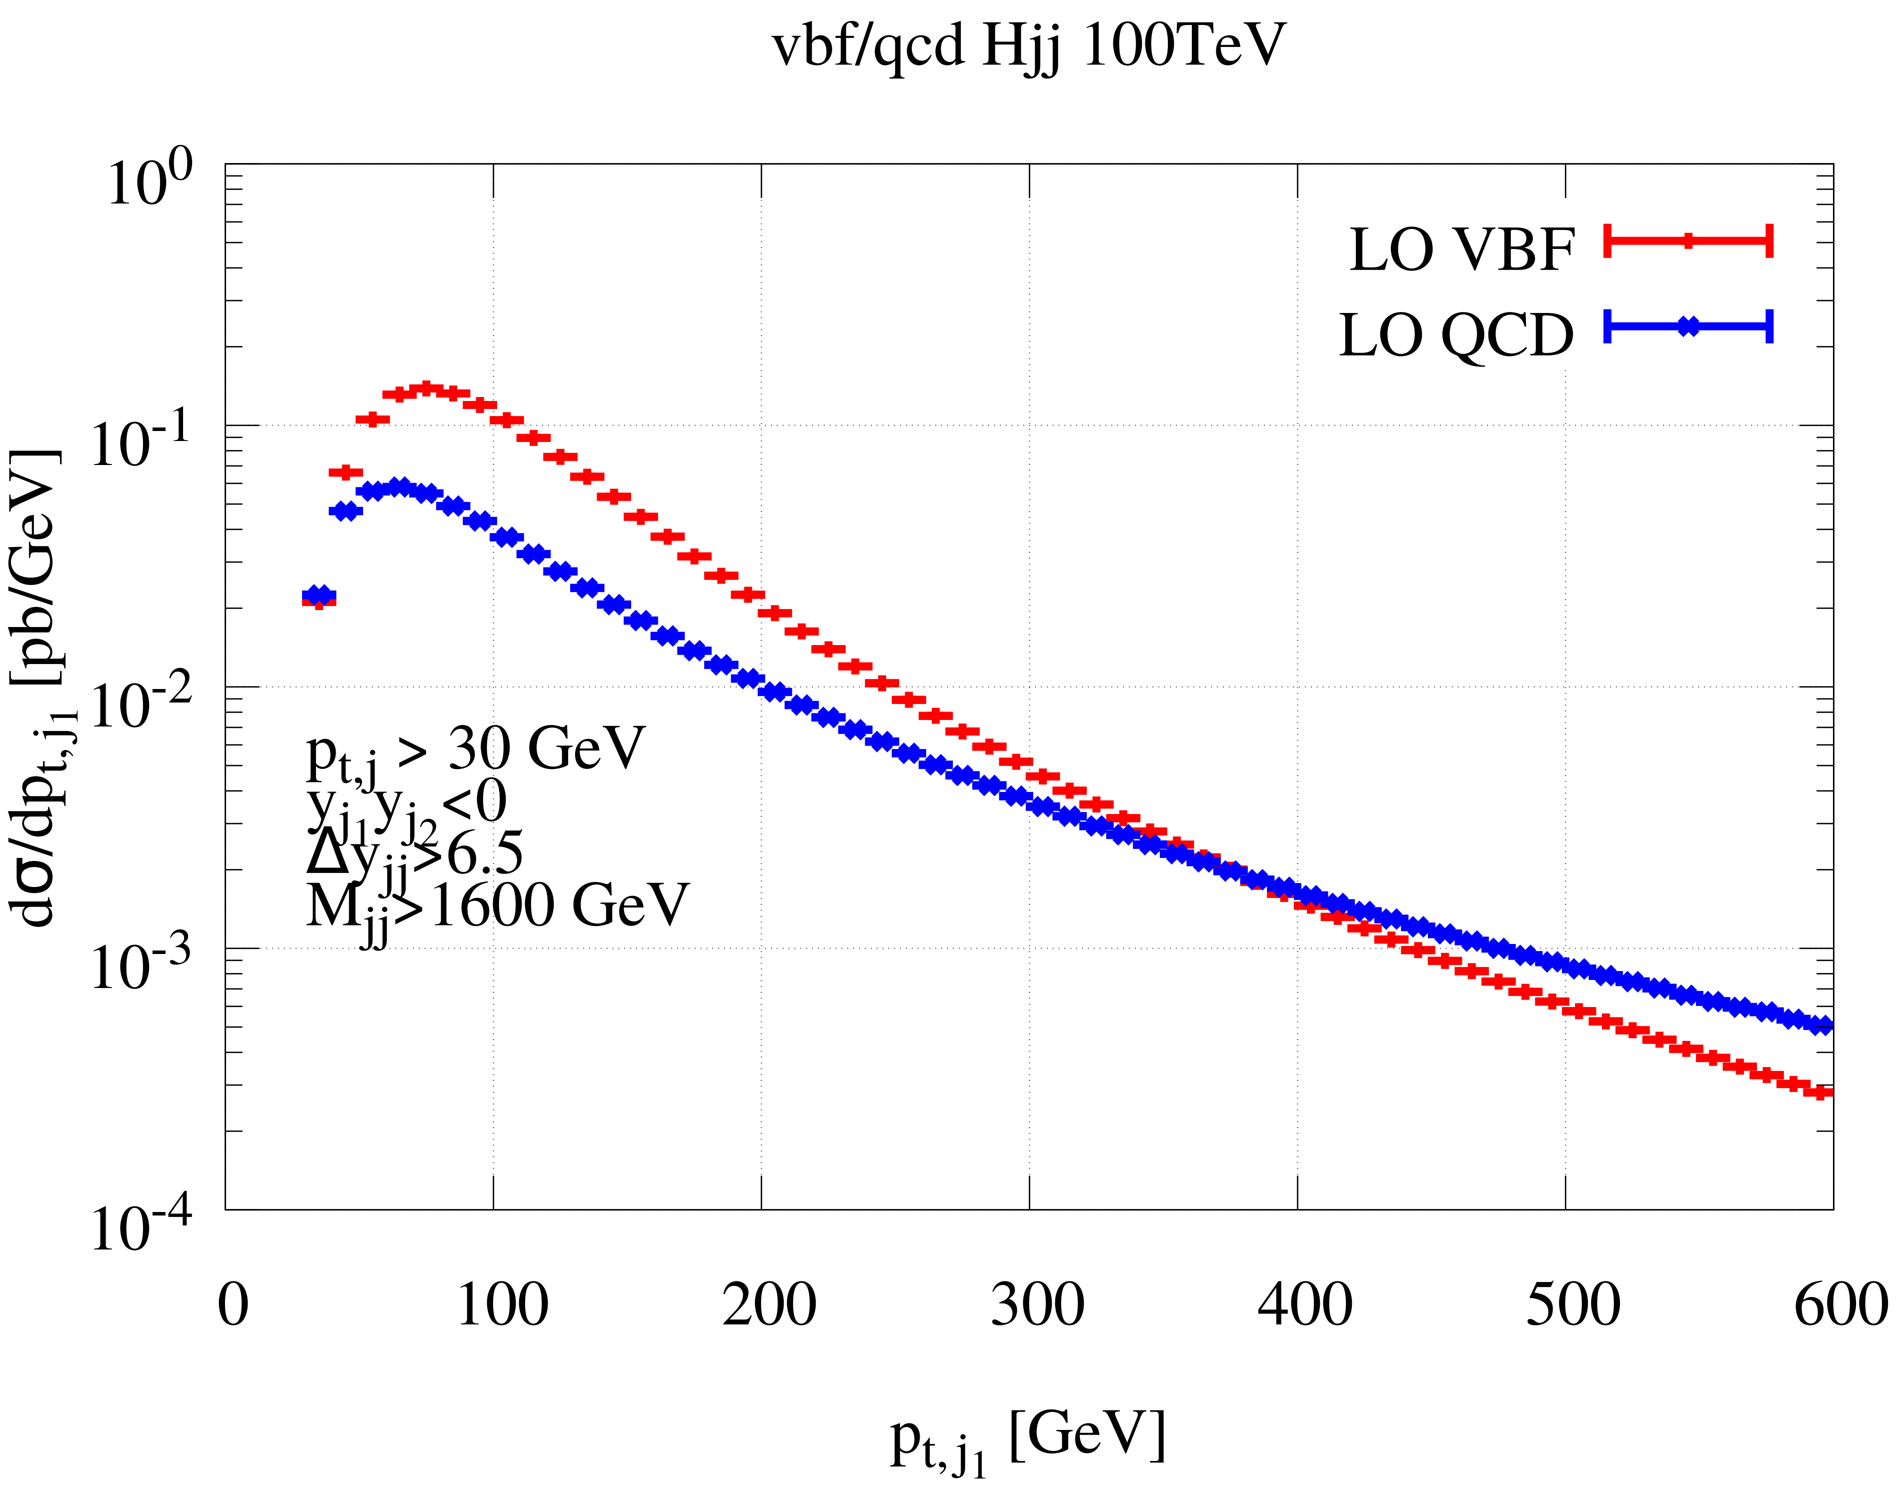

vbf/qcd Hjj 100TeV
LO VBF
LO QCD
$p_{t,j}$ > 30 GeV
$y_{j_1} y_{j_2} < 0$
$\Delta y_{jj} > 6.5$
$M_{jj} > 1600$ GeV
$d\sigma/dp_{t,j_1}$ [pb/GeV]
$p_{t,j_1}$ [GeV]
$10^{0}$
$10^{-1}$
$10^{-2}$
$10^{-3}$
$10^{-4}$
0
100
200
300
400
500
600

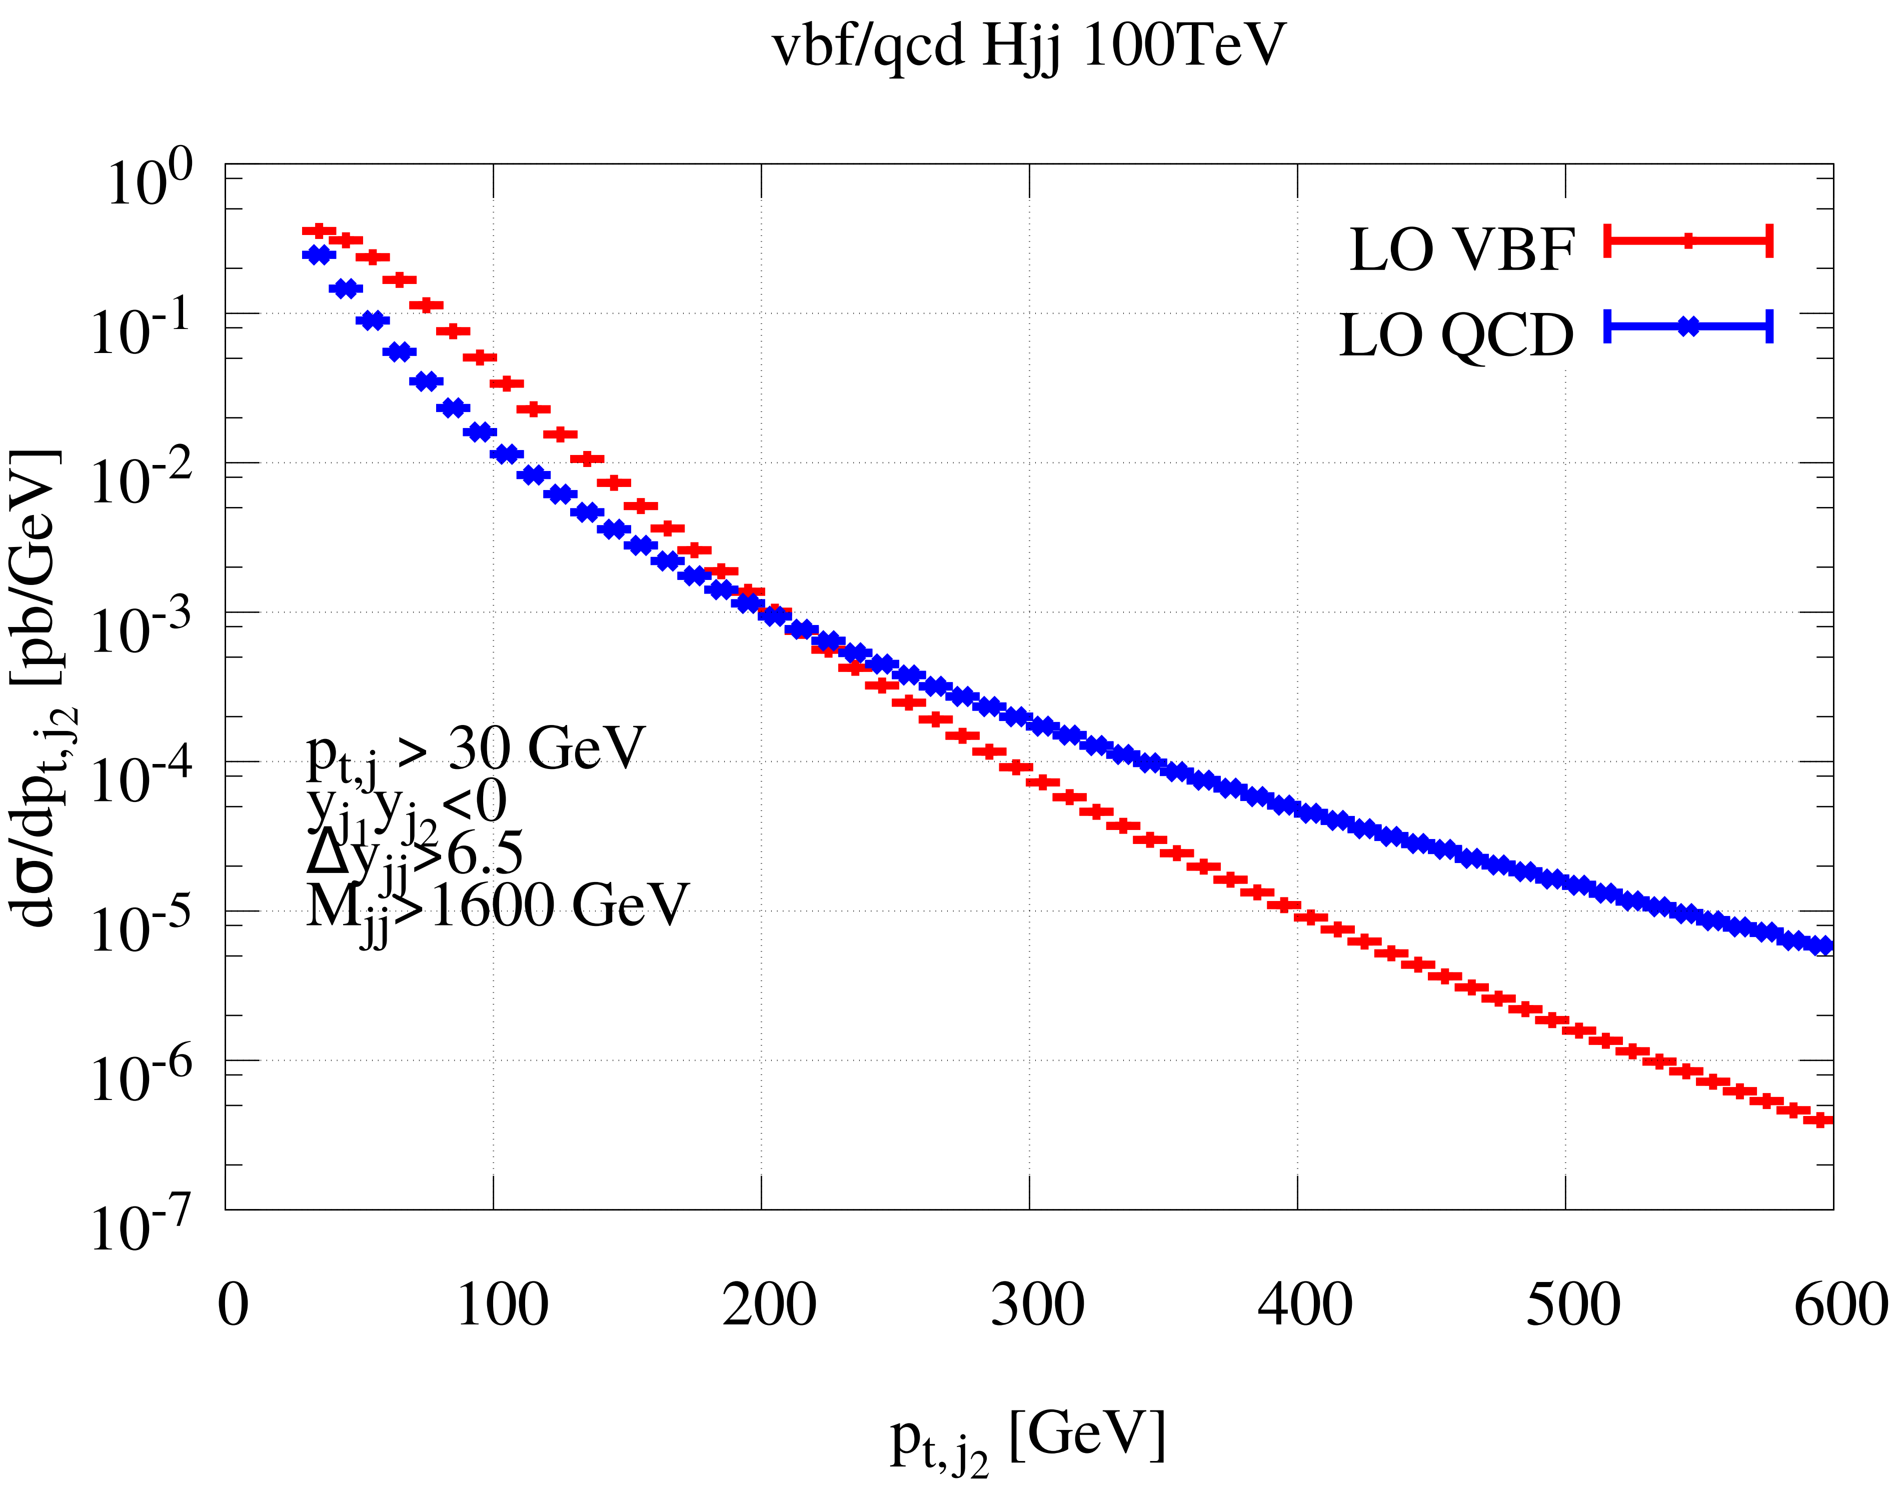

vbf/qcd Hjj 100TeV
LO VBF
LO QCD
$p_{t,j}$ > 30 GeV
$y_{j_1} y_{j_2}$<0
$\Delta y_{jj}$>6.5
$M_{jj}$>1600 GeV
$d\sigma/dp_{t,j_2}$ [pb/GeV]
$p_{t,j_2}$ [GeV]
$10^0$
$10^{-1}$
$10^{-2}$
$10^{-3}$
$10^{-4}$
$10^{-5}$
$10^{-6}$
$10^{-7}$
0
100
200
300
400
500
600

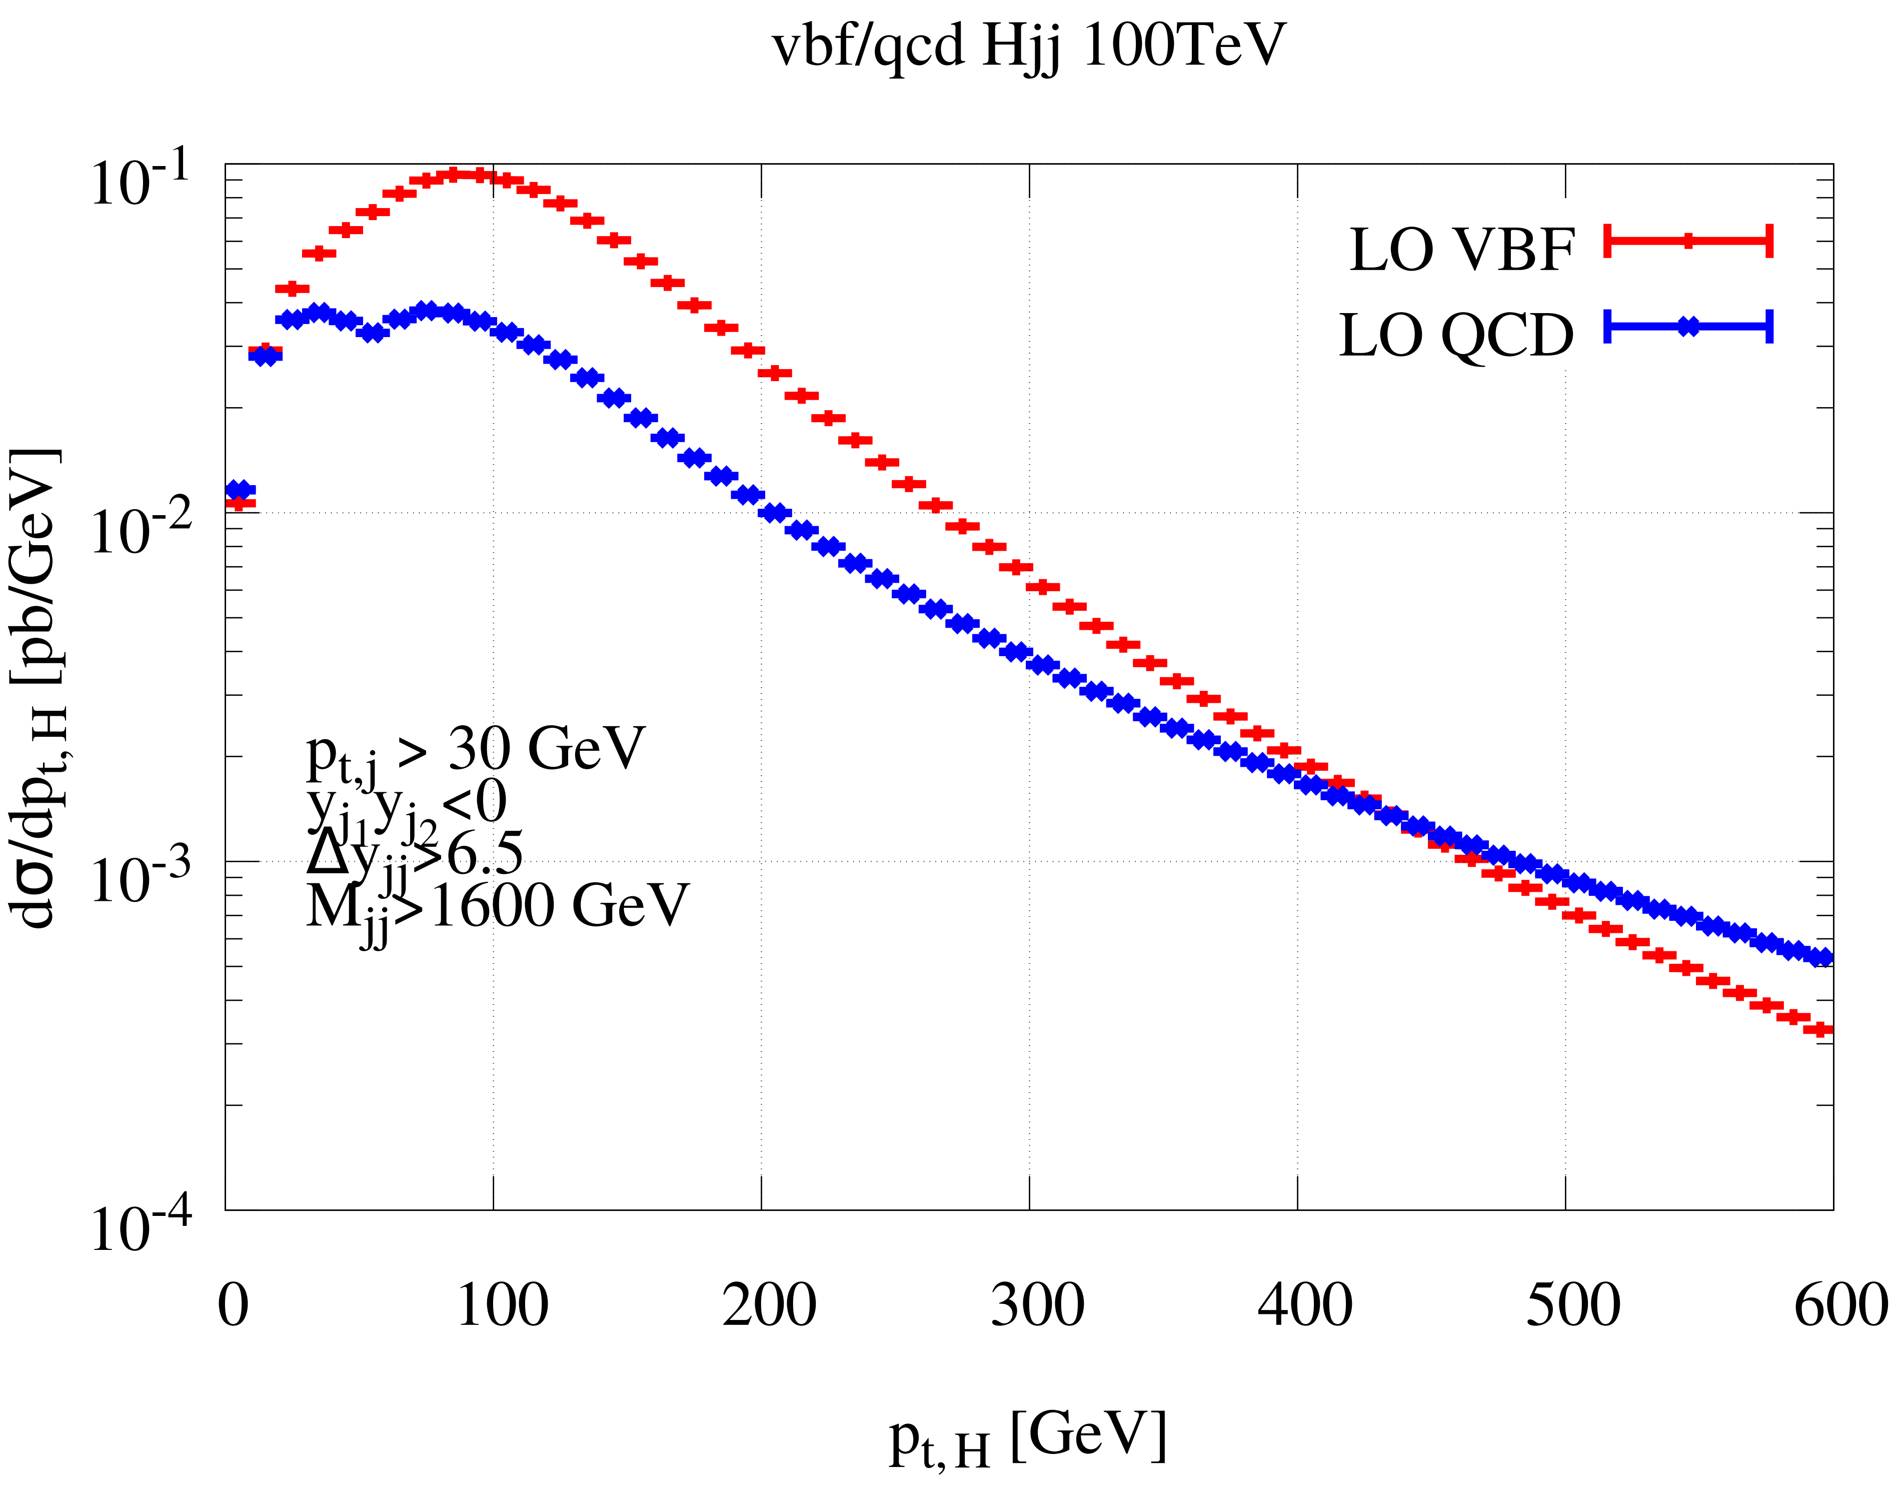

vbf/qcd Hjj 100TeV
LO VBF
LO QCD
$p_{t,j}$ > 30 GeV
$y_{j_1} y_{j_2}$<0
$\Delta y_{jj}$>6.5
$M_{jj}$>1600 GeV
$d\sigma/dp_{t,H}$ [pb/GeV]
$p_{t,H}$ [GeV]
$10^{-1}$
$10^{-2}$
$10^{-3}$
$10^{-4}$
0
100
200
300
400
500
600

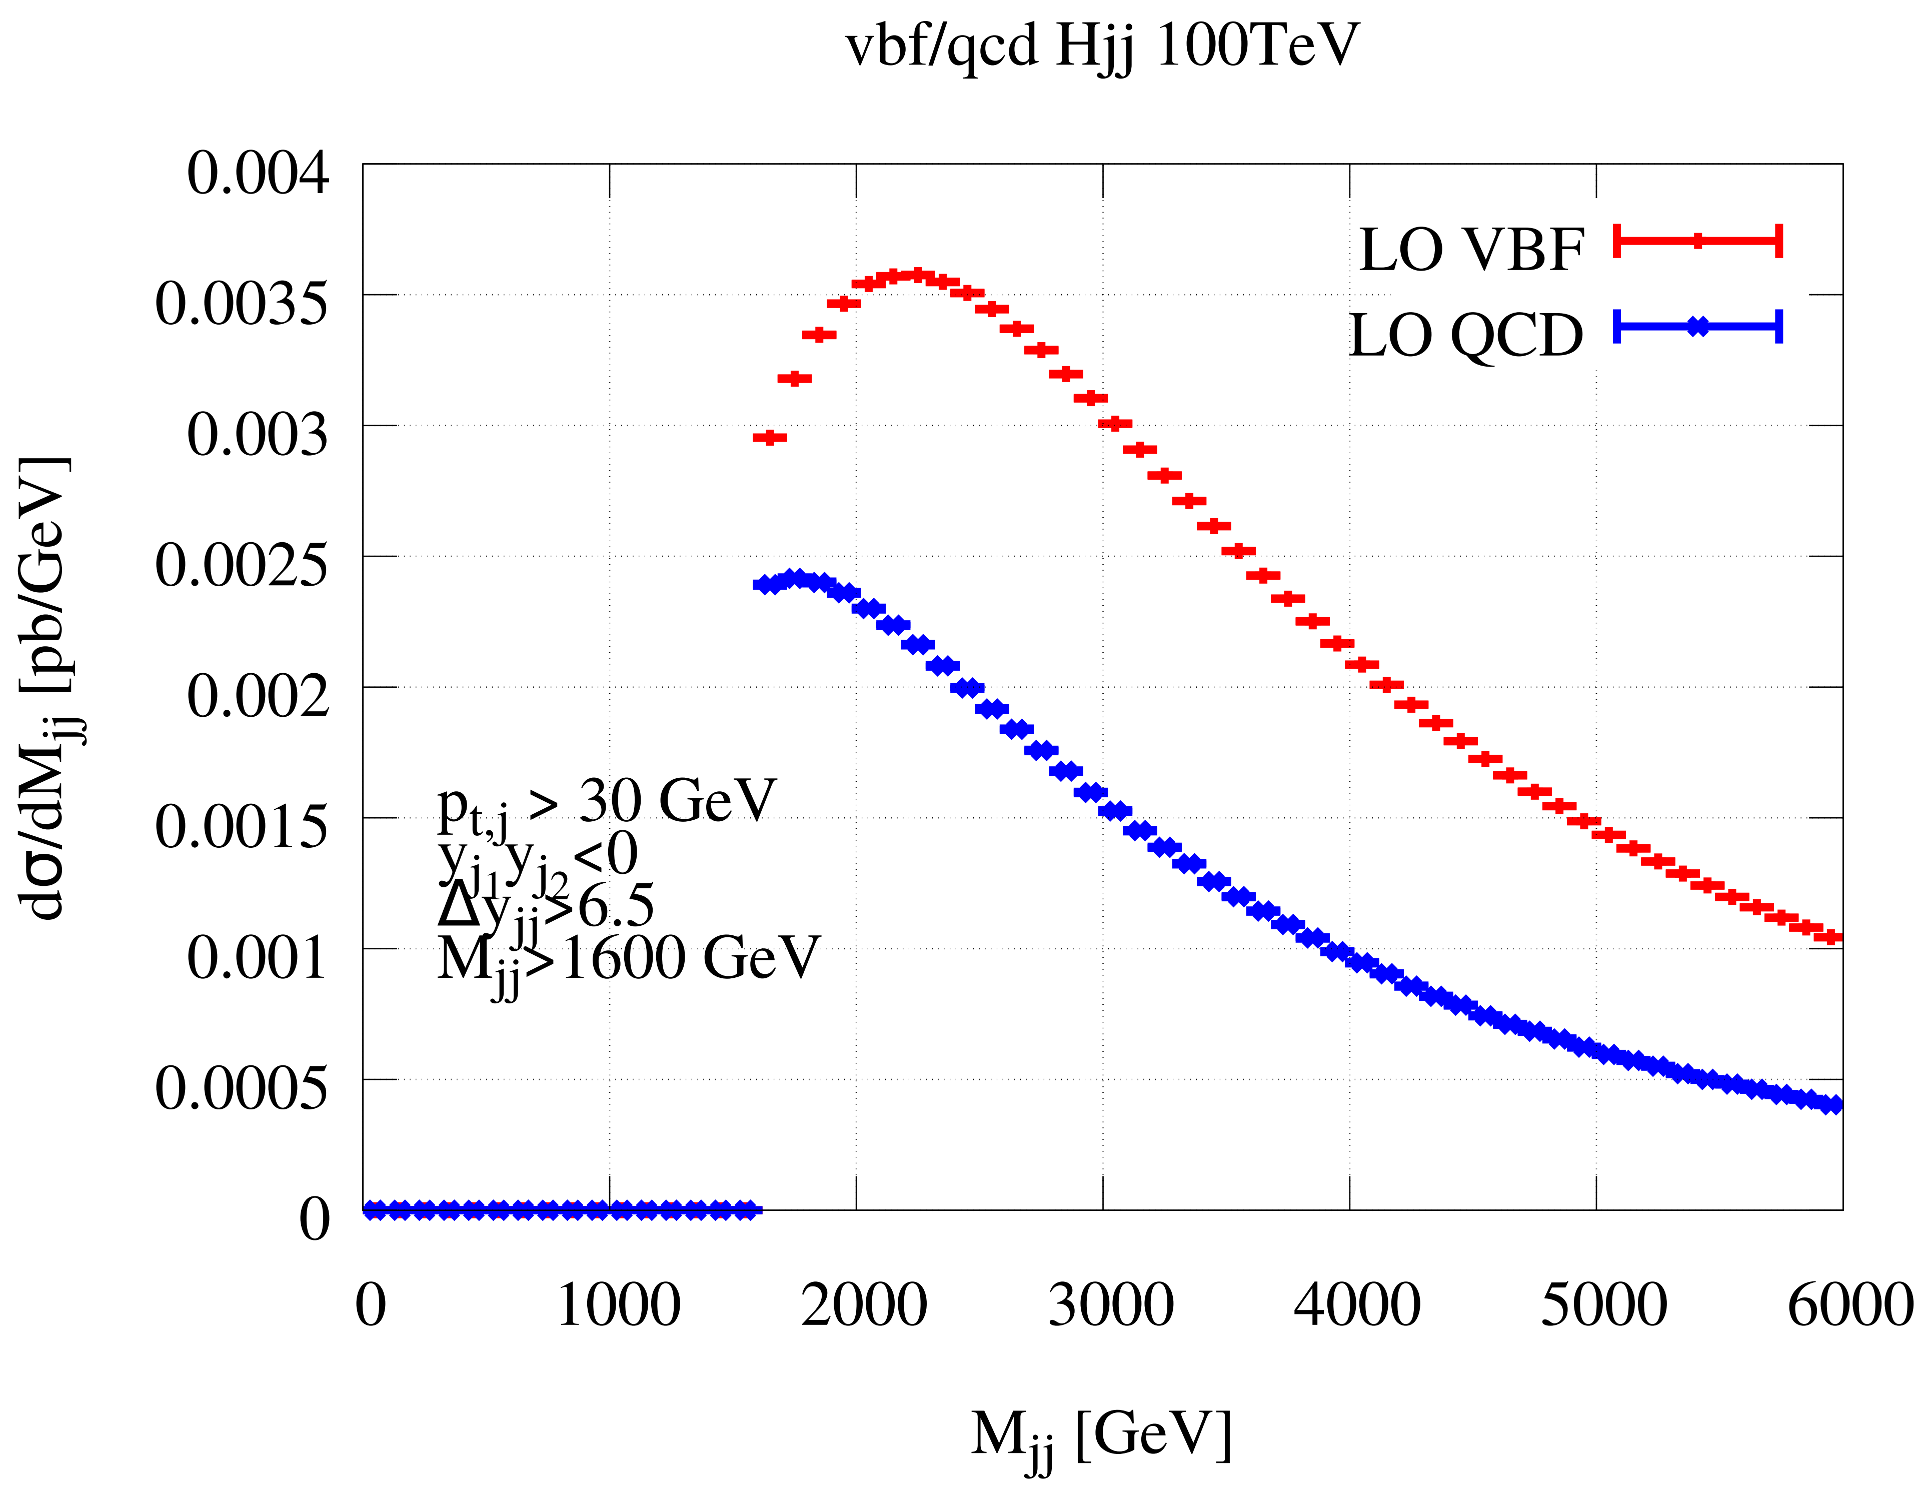
vbf/qcd Hjj 100TeV
LO VBF
LO QCD
$d\sigma/dM_{jj}$ [pb/GeV]
$M_{jj}$ [GeV]
$p_{t,j}$ > 30 GeV
$y_{j_1} y_{j_2}$<0
$\Delta y_{jj}$>6.5
$M_{jj}$>1600 GeV
0
0.0005
0.001
0.0015
0.002
0.0025
0.003
0.0035
0.004
1000
2000
3000
4000
5000
6000

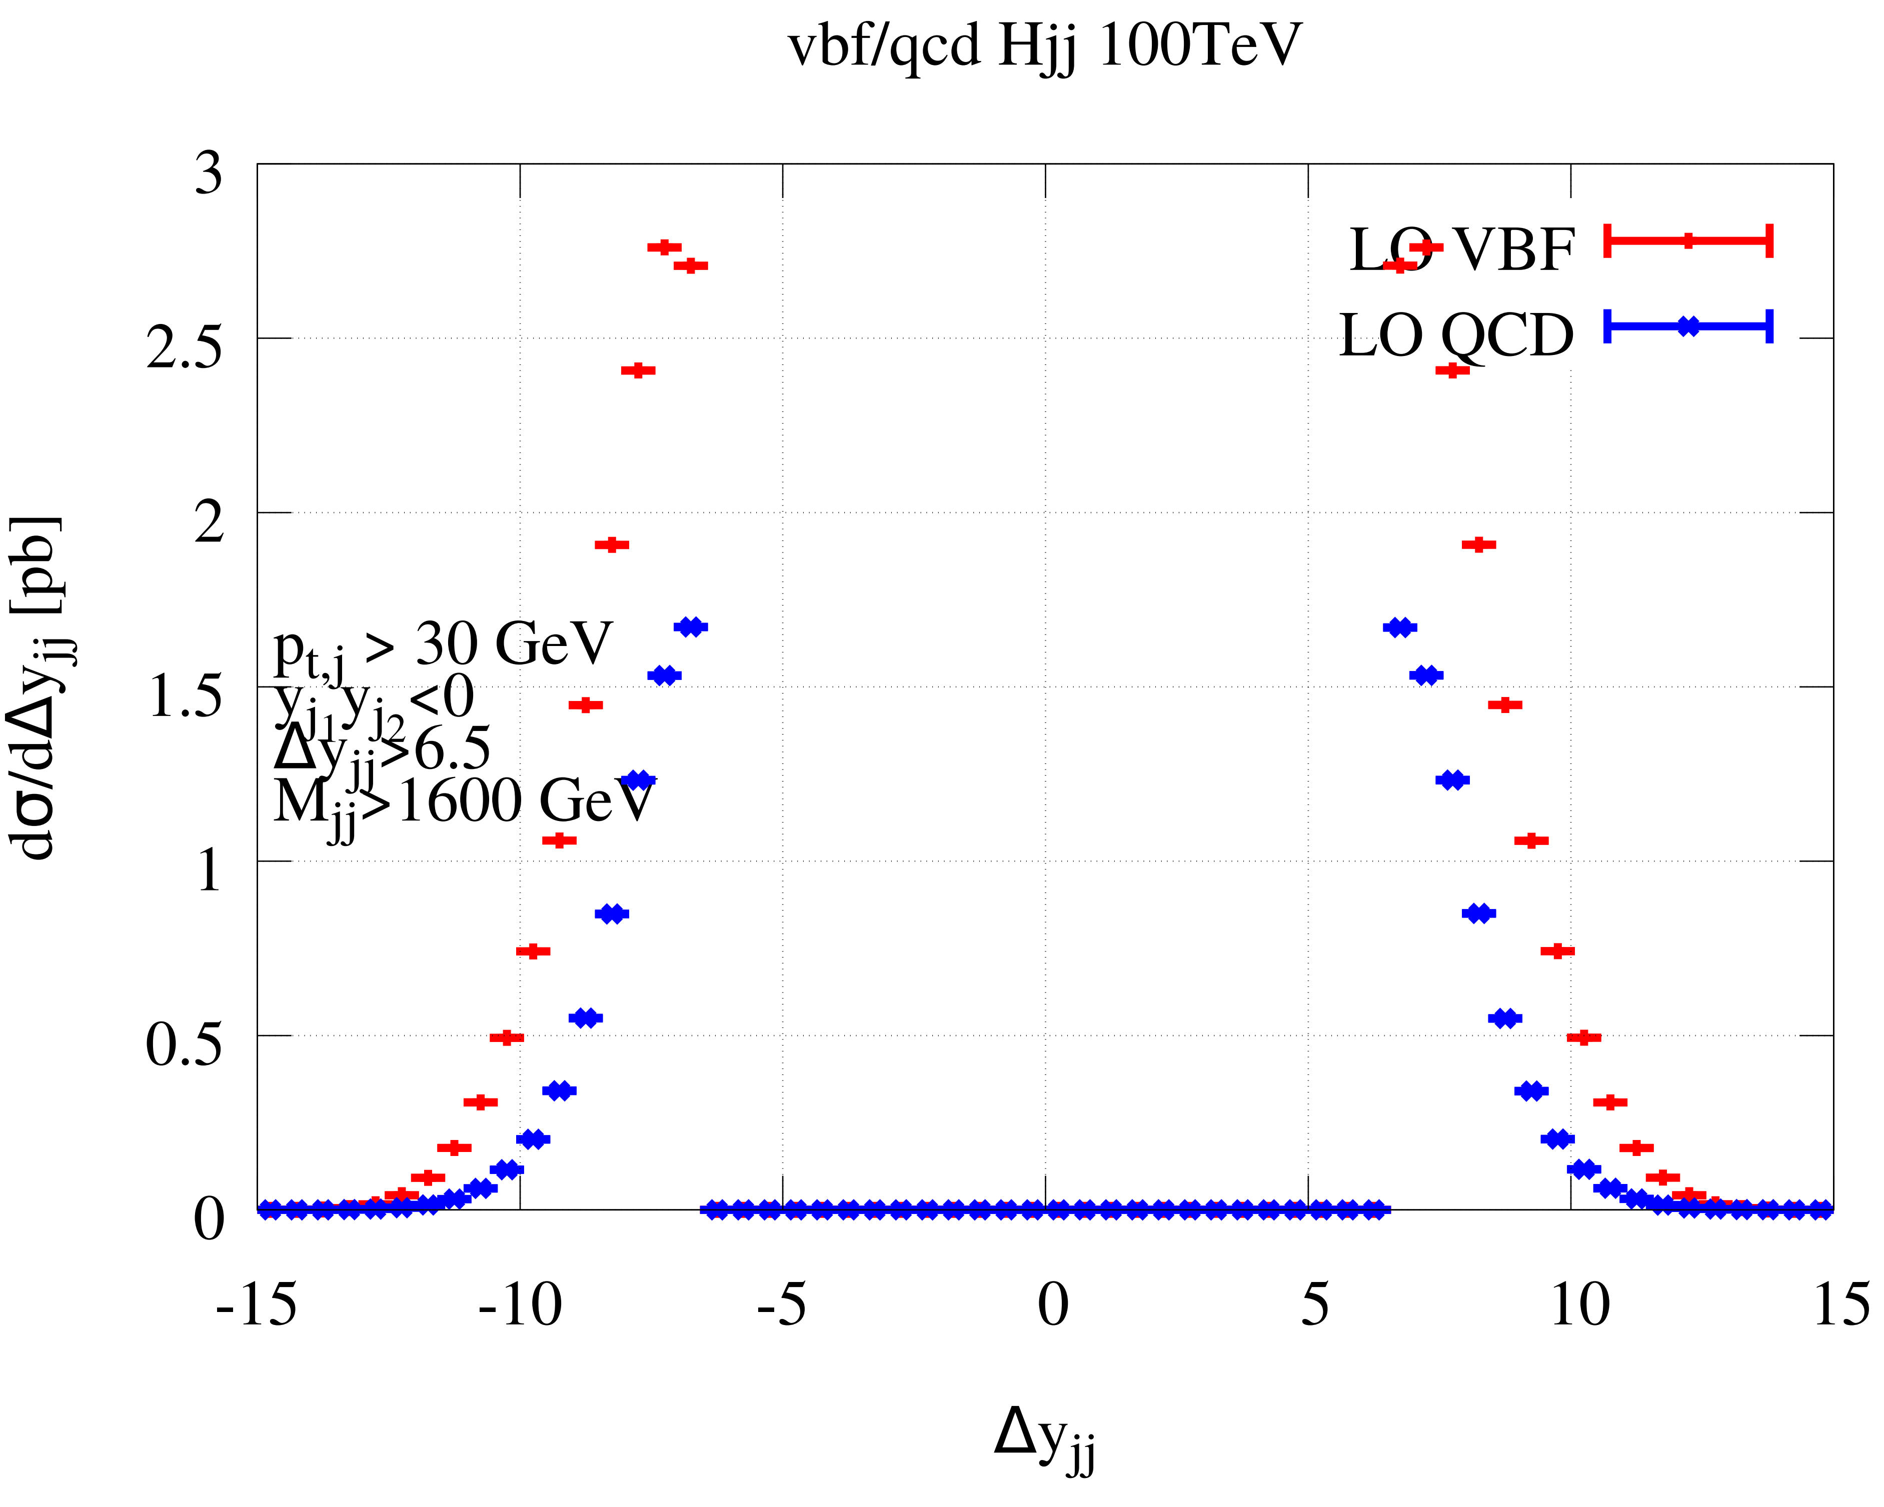
vbf/qcd Hjj 100TeV
LO VBF
LO QCD
$p_{t,j}$ > 30 GeV
$y_{j_1} y_{j_2}$<0
$\Delta y_{jj}$>6.5
$M_{jj}$>1600 GeV
$d\sigma/d\Delta y_{jj}$ [pb]
$\Delta y_{jj}$
3
2.5
2
1.5
1
0.5
0
-15
-10
-5
0
5
10
15

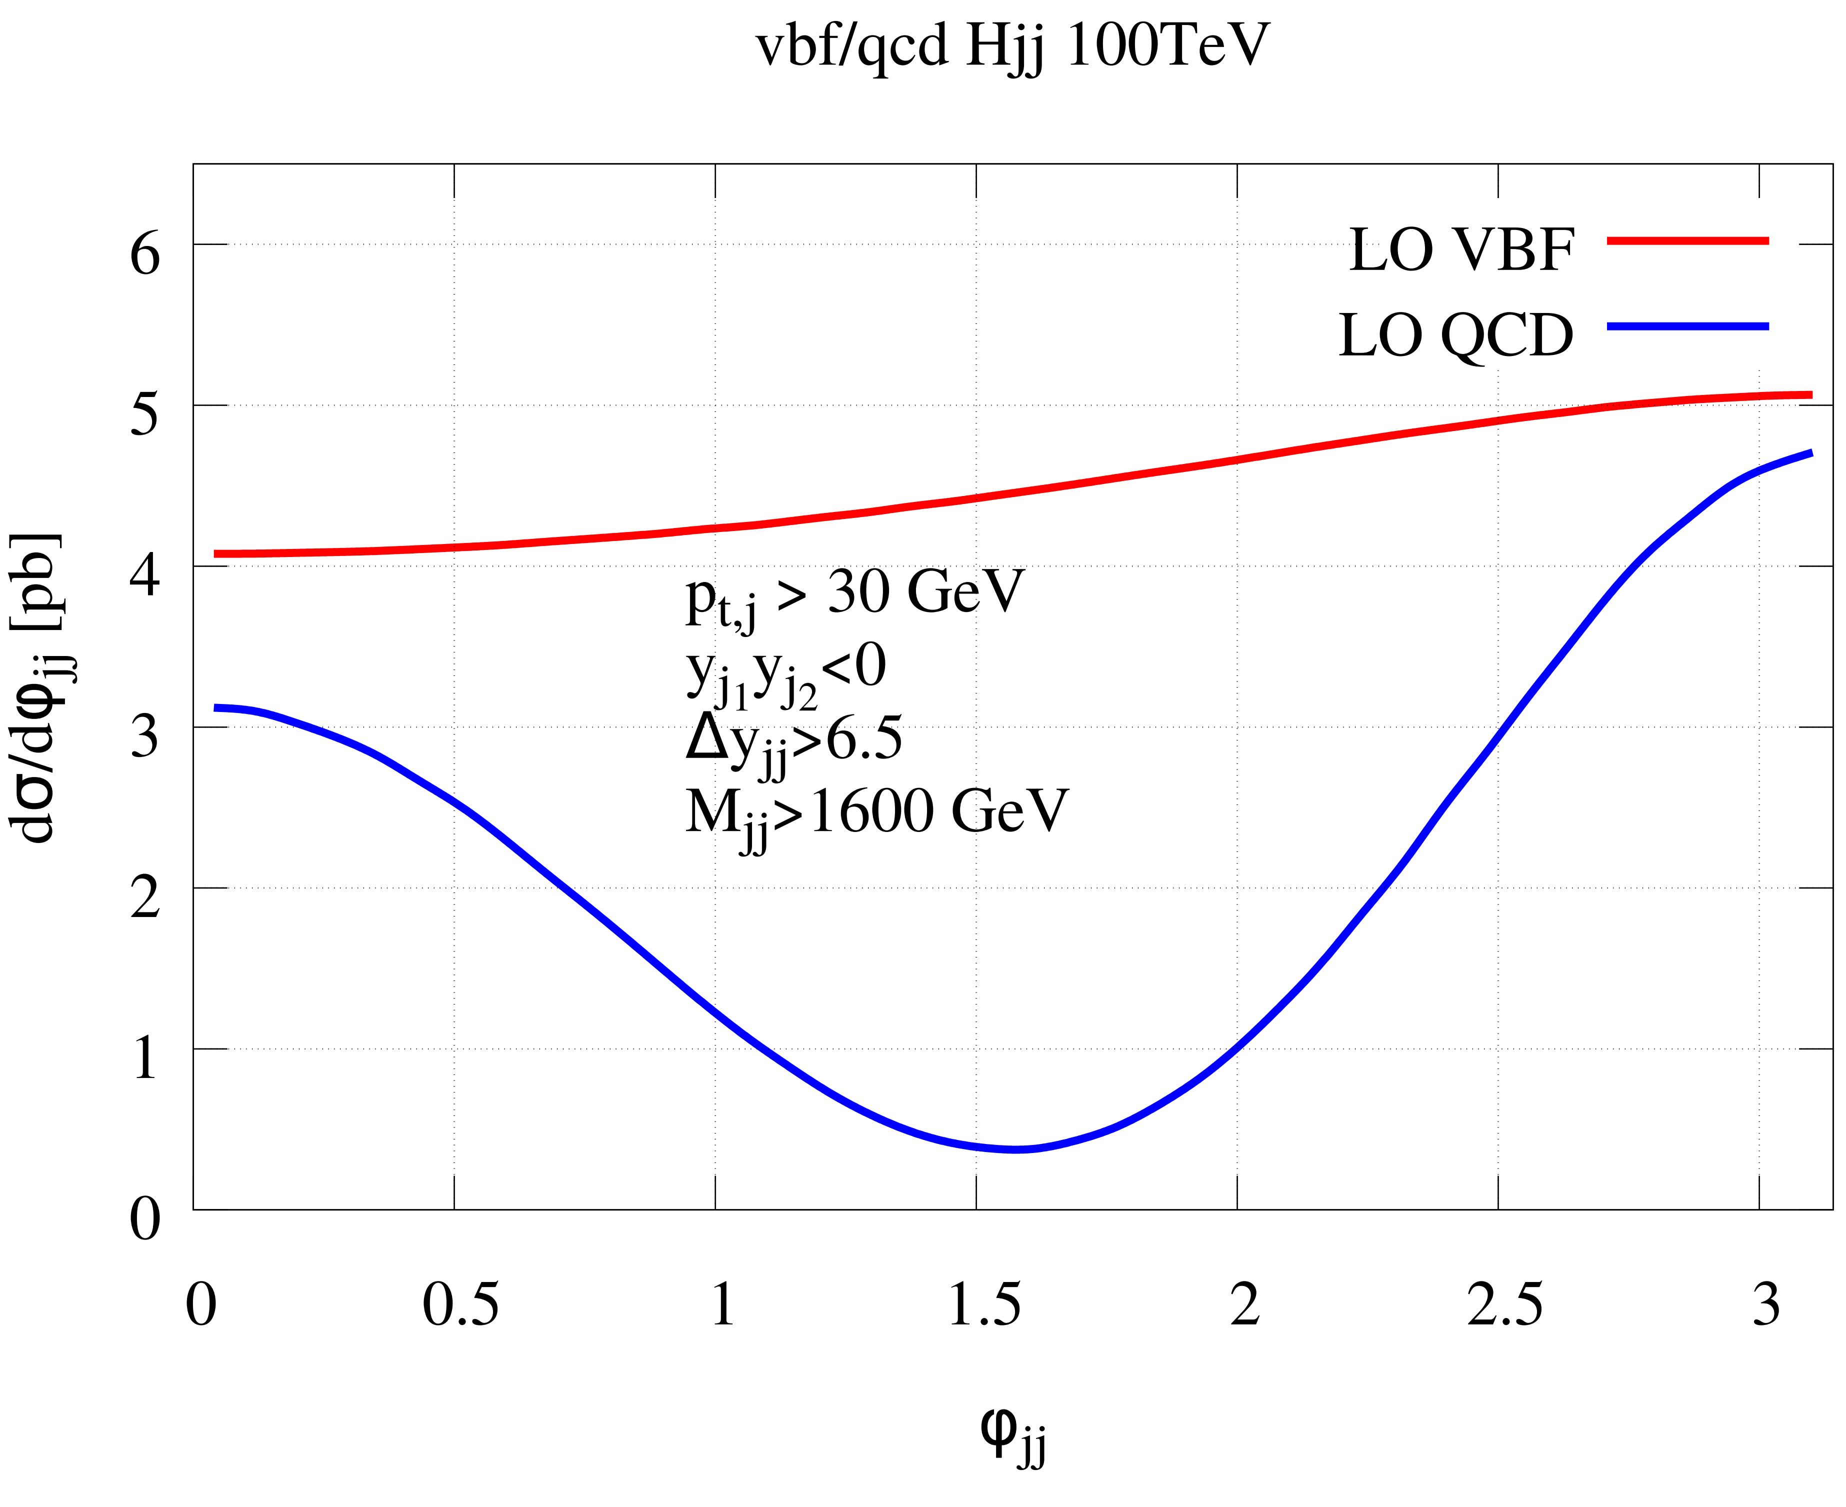

vbf/qcd Hjj 100TeV
LO VBF
LO QCD
$p_{t,j}$ > 30 GeV
$y_{j_1}y_{j_2}$<0
$\Delta y_{jj}$>6.5
$M_{jj}$>1600 GeV
$d\sigma/d\varphi_{jj}$ [pb]
$\varphi_{jj}$
0
1
2
3
4
5
6
0
0.5
1
1.5
2
2.5
3

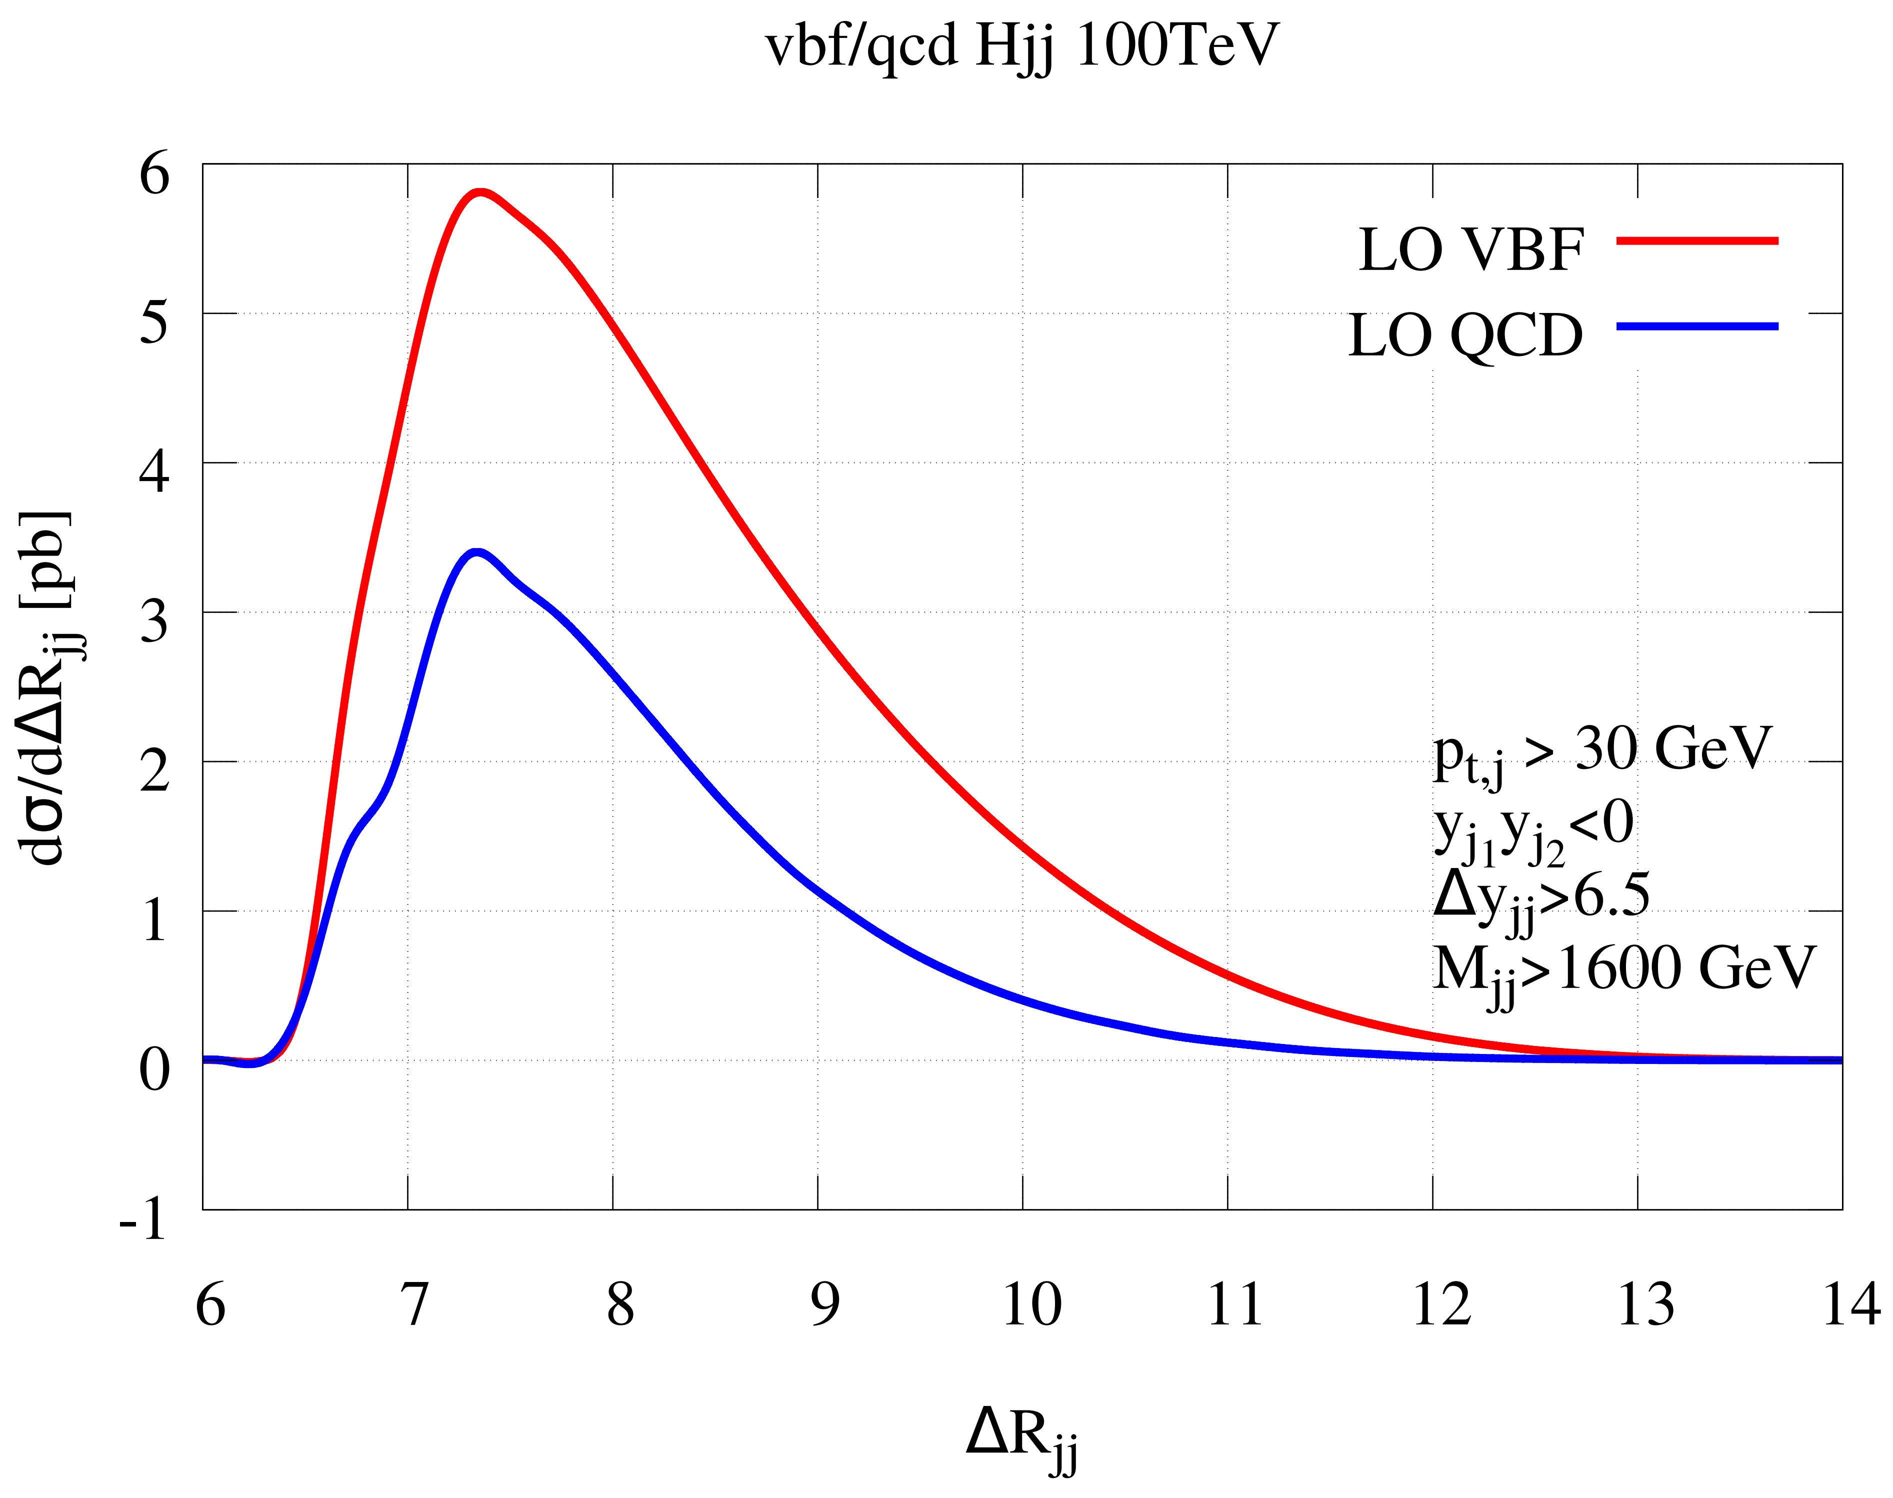

vbf/qcd Hjj 100TeV
LO VBF
LO QCD
$p_{t,j}$ > 30 GeV
$y_{j_1}y_{j_2}<0$
$\Delta y_{jj}>6.5$
$M_{jj}>1600$ GeV
$d\sigma/d\Delta R_{jj}$ [pb]
$\Delta R_{jj}$
6
5
4
3
2
1
0
-1
6
7
8
9
10
11
12
13
14

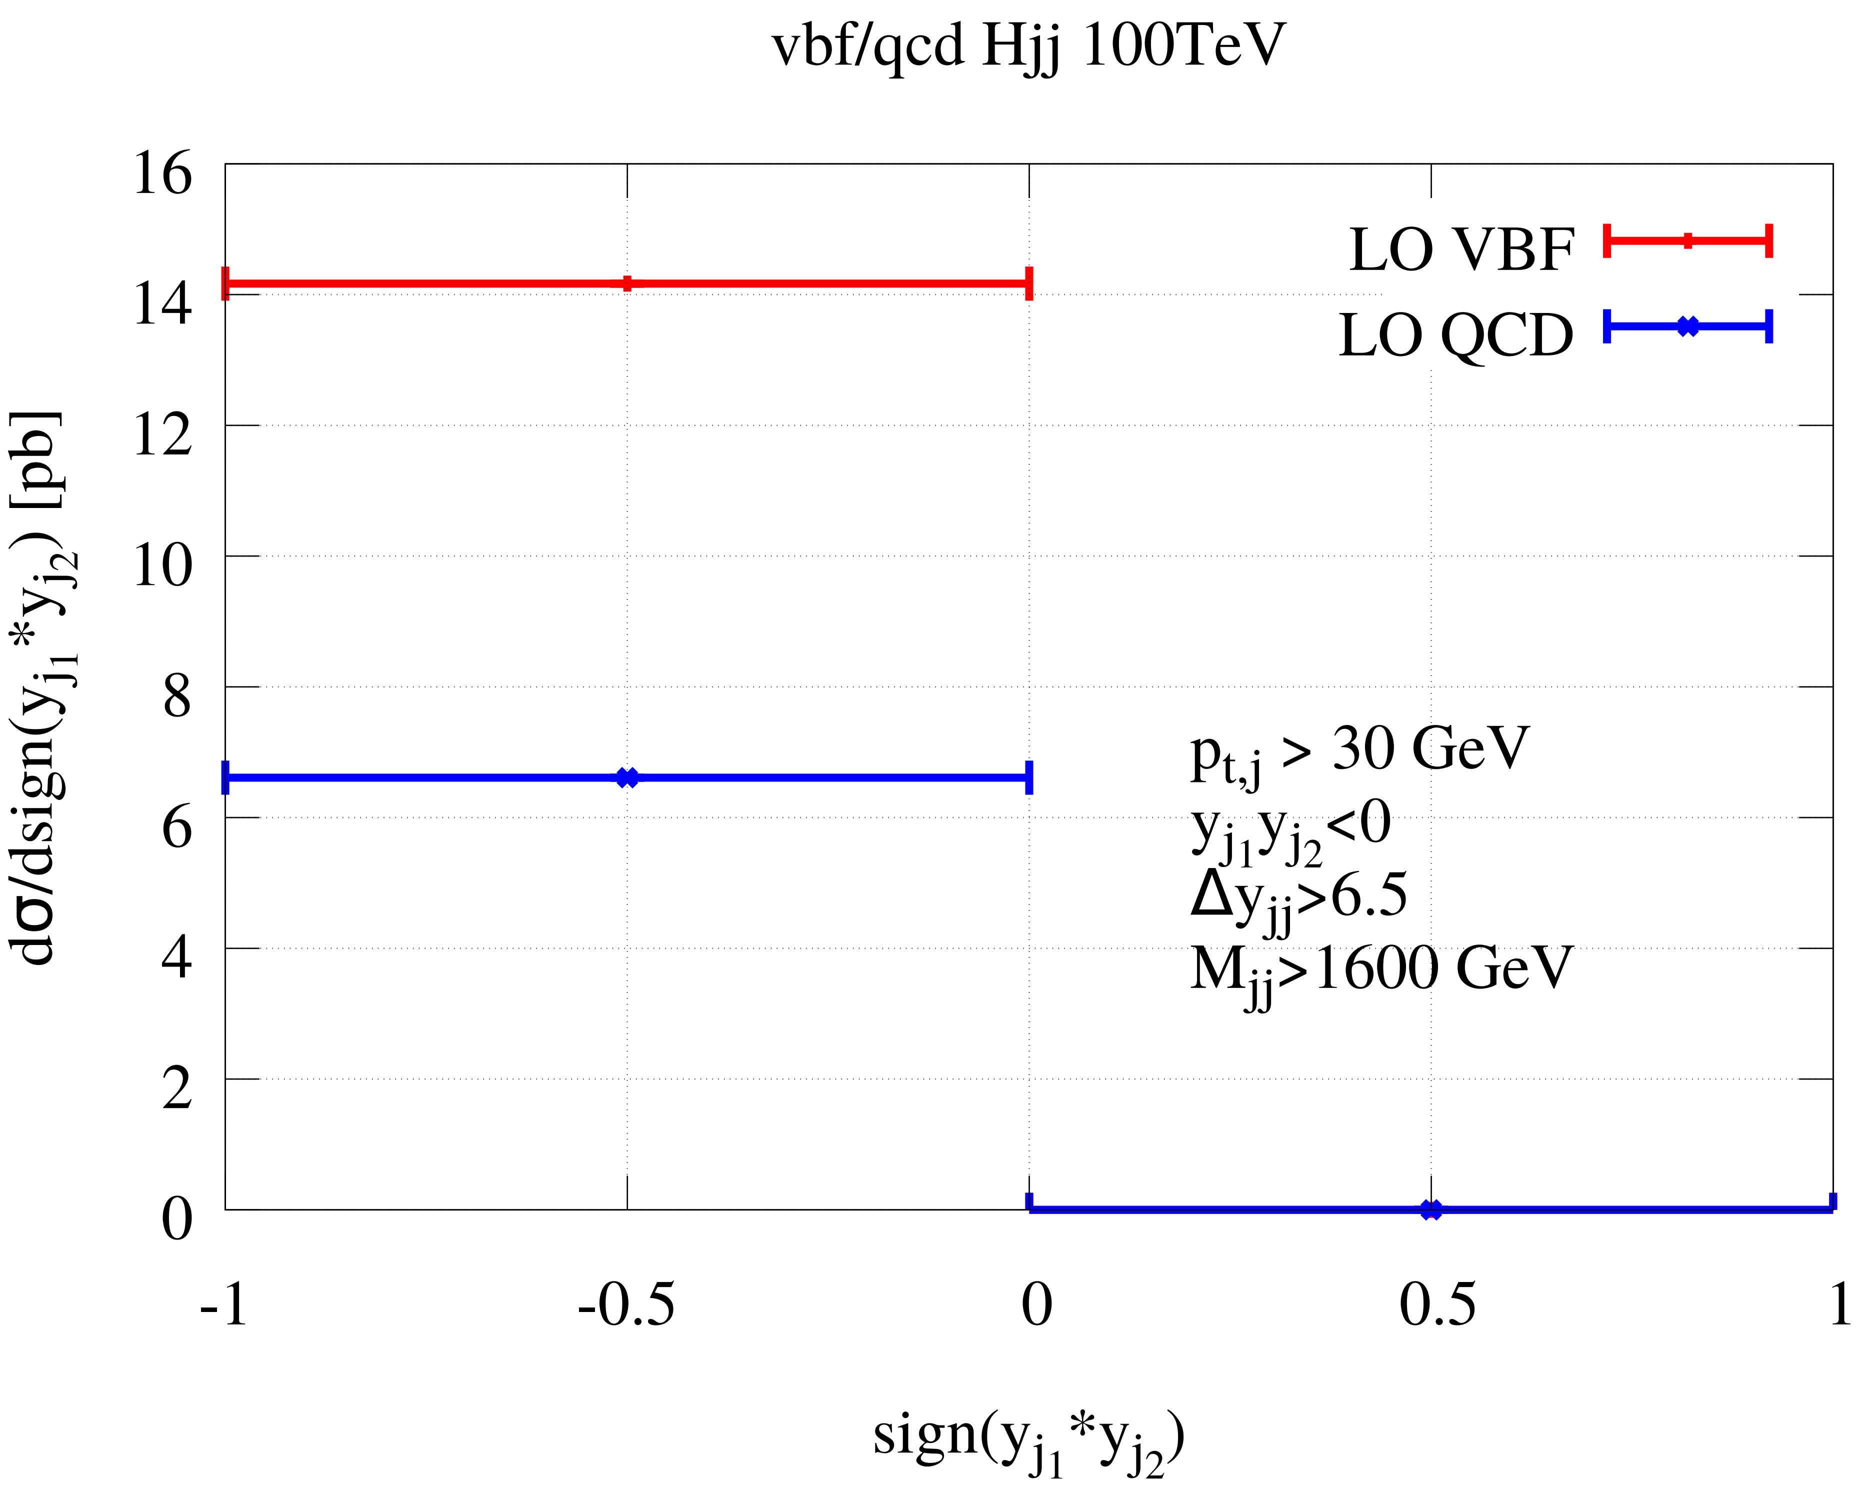

vbf/qcd Hjj 100TeV
LO VBF
LO QCD
$p_{t,j}$ > 30 GeV
$y_{j_1}y_{j_2}$<0
$\Delta y_{jj}$>6.5
$M_{jj}$>1600 GeV
dσ/dsign($y_{j_1}$*$y_{j_2}$) [pb]
sign($y_{j_1}$*$y_{j_2}$)
0
2
4
6
8
10
12
14
16
-1
-0.5
0
0.5
1

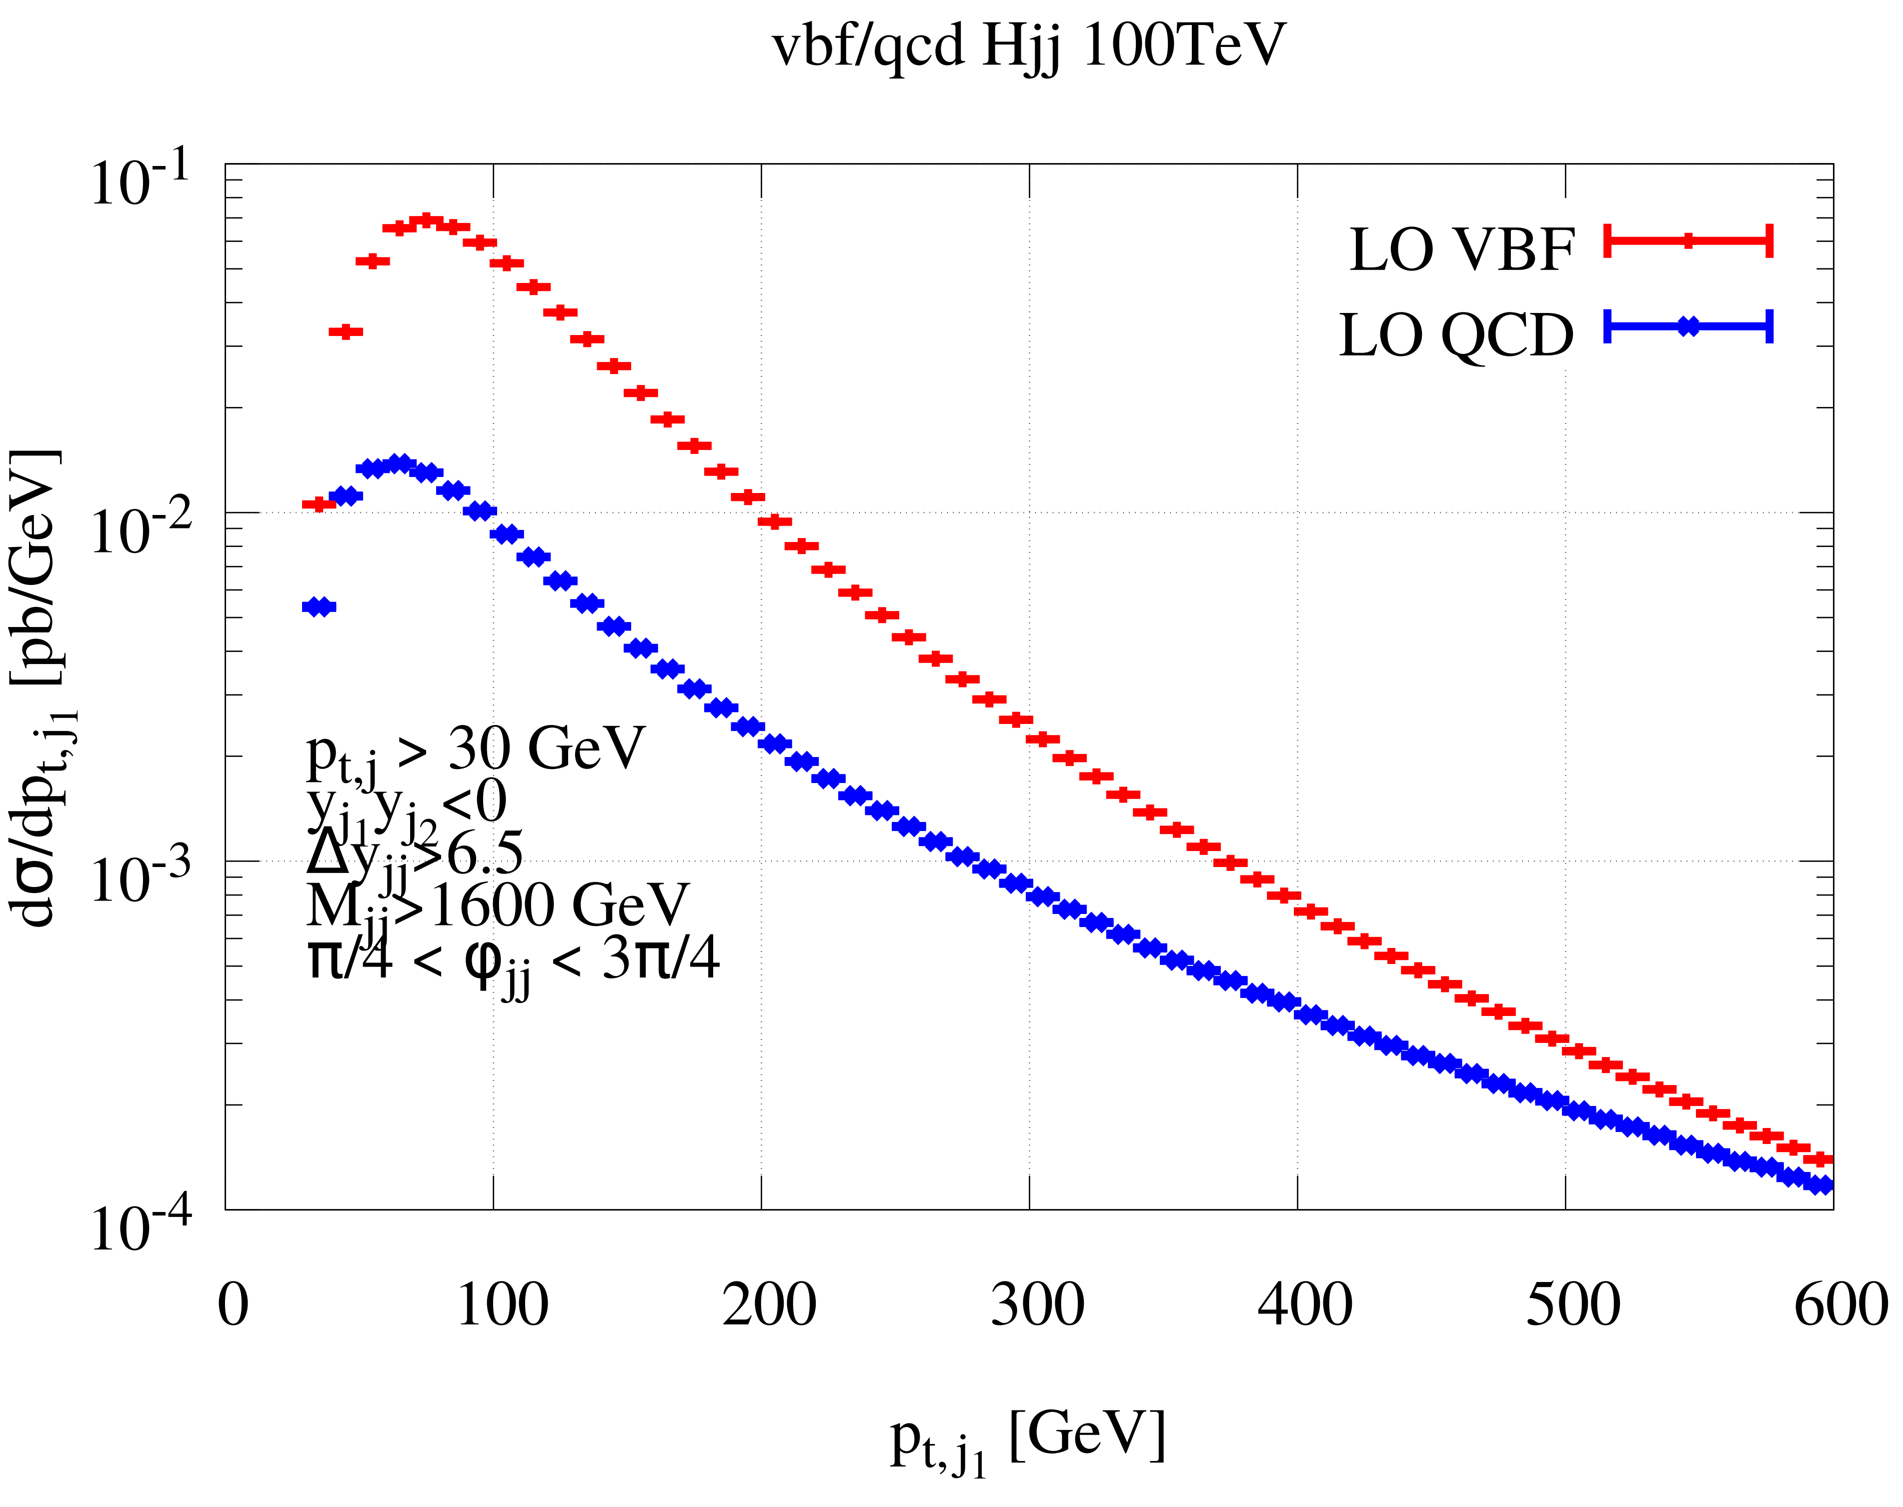

vbf/qcd Hjj 100TeV
LO VBF
LO QCD
$p_{t,j}$ > 30 GeV
$y_{j_1} y_{j_2}$<0
$\Delta y_{jj}$>6.5
$M_{jj}$>1600 GeV
$\pi/4 < \varphi_{jj} < 3\pi/4$
$d\sigma/dp_{t,j_1}$ [pb/GeV]
$p_{t,j_1}$ [GeV]
$10^{-1}$
$10^{-2}$
$10^{-3}$
$10^{-4}$
0
100
200
300
400
500
600

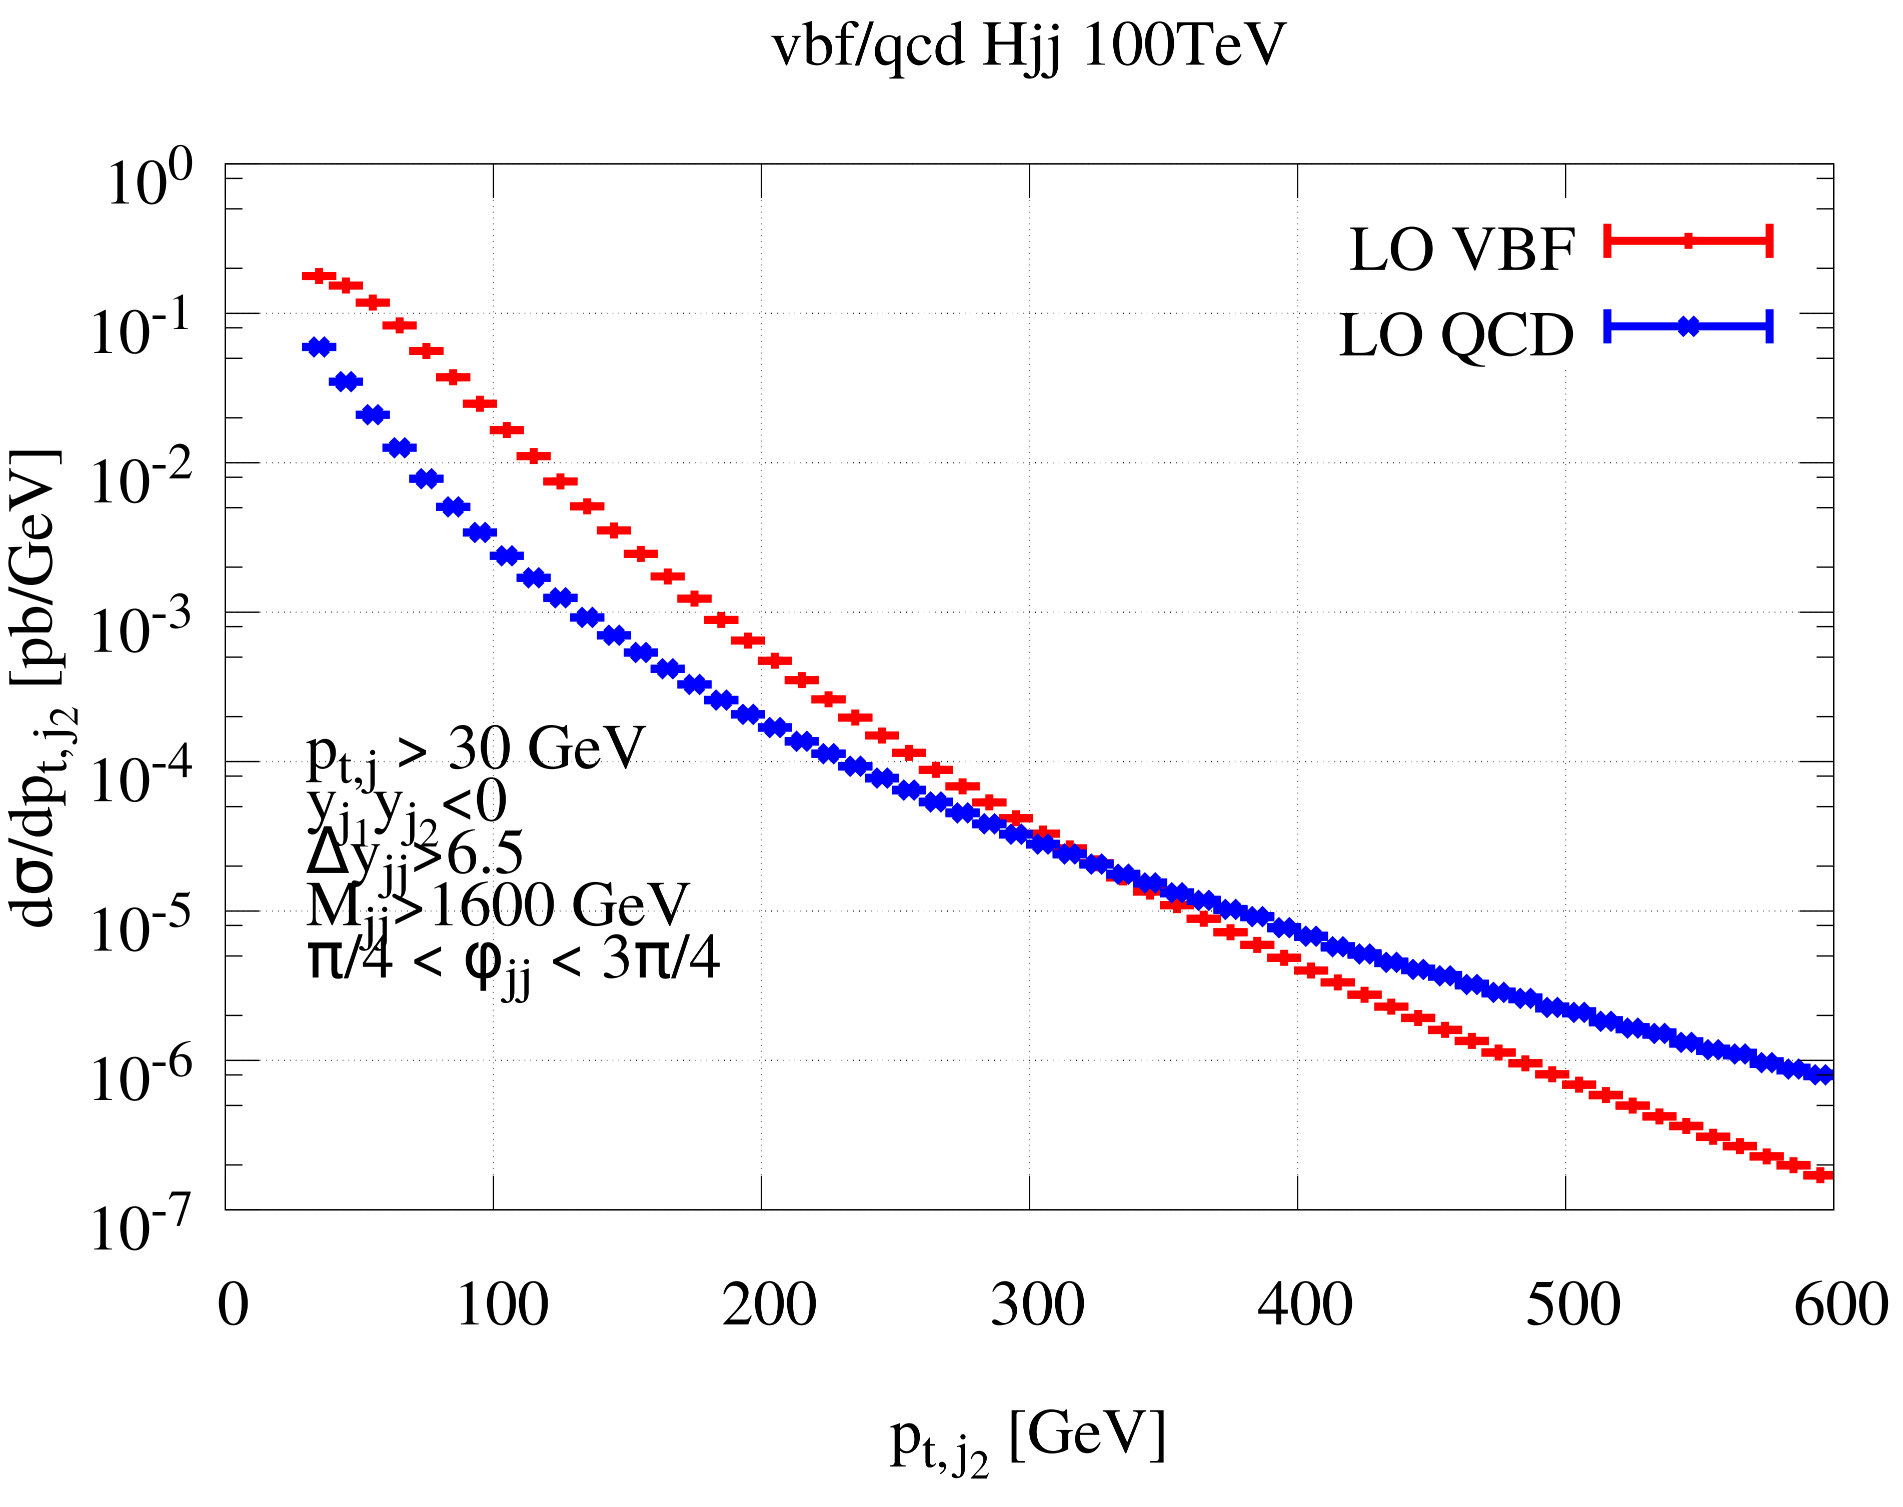

vbf/qcd Hjj 100TeV
LO VBF
LO QCD
$p_{t,j} > 30$ GeV
$y_{j_1} y_{j_2} < 0$
$\Delta y_{jj} > 6.5$
$M_{jj} > 1600$ GeV
$\pi/4 < \phi_{jj} < 3\pi/4$
$d\sigma/dp_{t,j_2}$ [pb/GeV]
$p_{t,j_2}$ [GeV]
$10^{0}$
$10^{-1}$
$10^{-2}$
$10^{-3}$
$10^{-4}$
$10^{-5}$
$10^{-6}$
$10^{-7}$
0
100
200
300
400
500
600

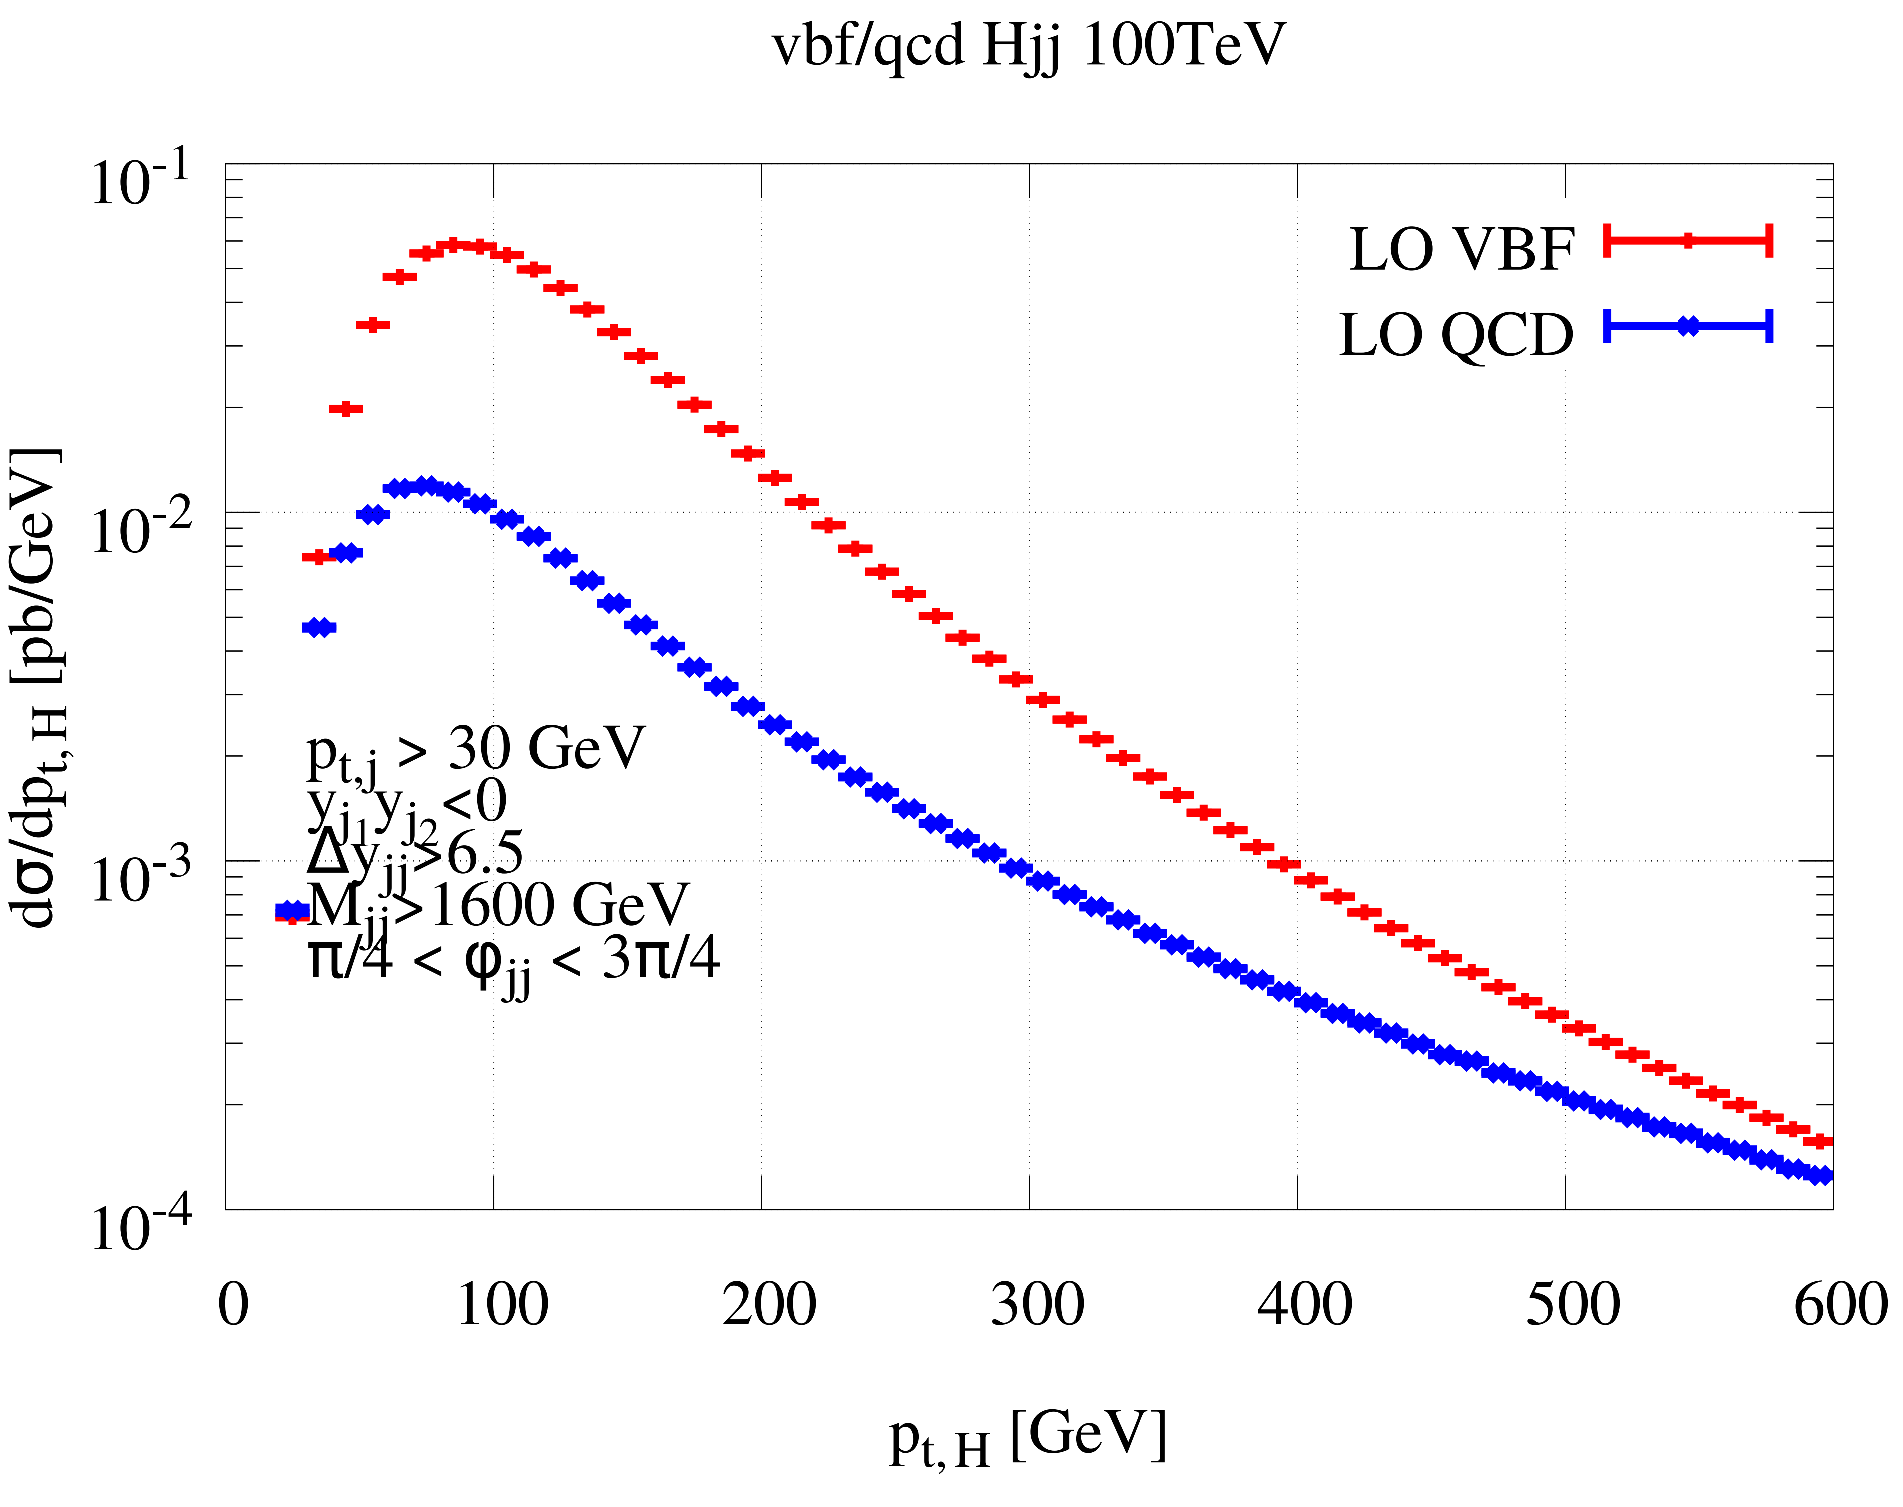

vbf/qcd Hjj 100TeV
LO VBF
LO QCD
$p_{t,j}$ > 30 GeV
$y_{j_1} y_{j_2} < 0$
$\Delta y_{jj} > 6.5$
$M_{jj} > 1600$ GeV
$\pi/4 < \phi_{jj} < 3\pi/4$
$d\sigma/dp_{t,H}$ [pb/GeV]
$p_{t,H}$ [GeV]
$10^{-1}$
$10^{-2}$
$10^{-3}$
$10^{-4}$
0
100
200
300
400
500
600

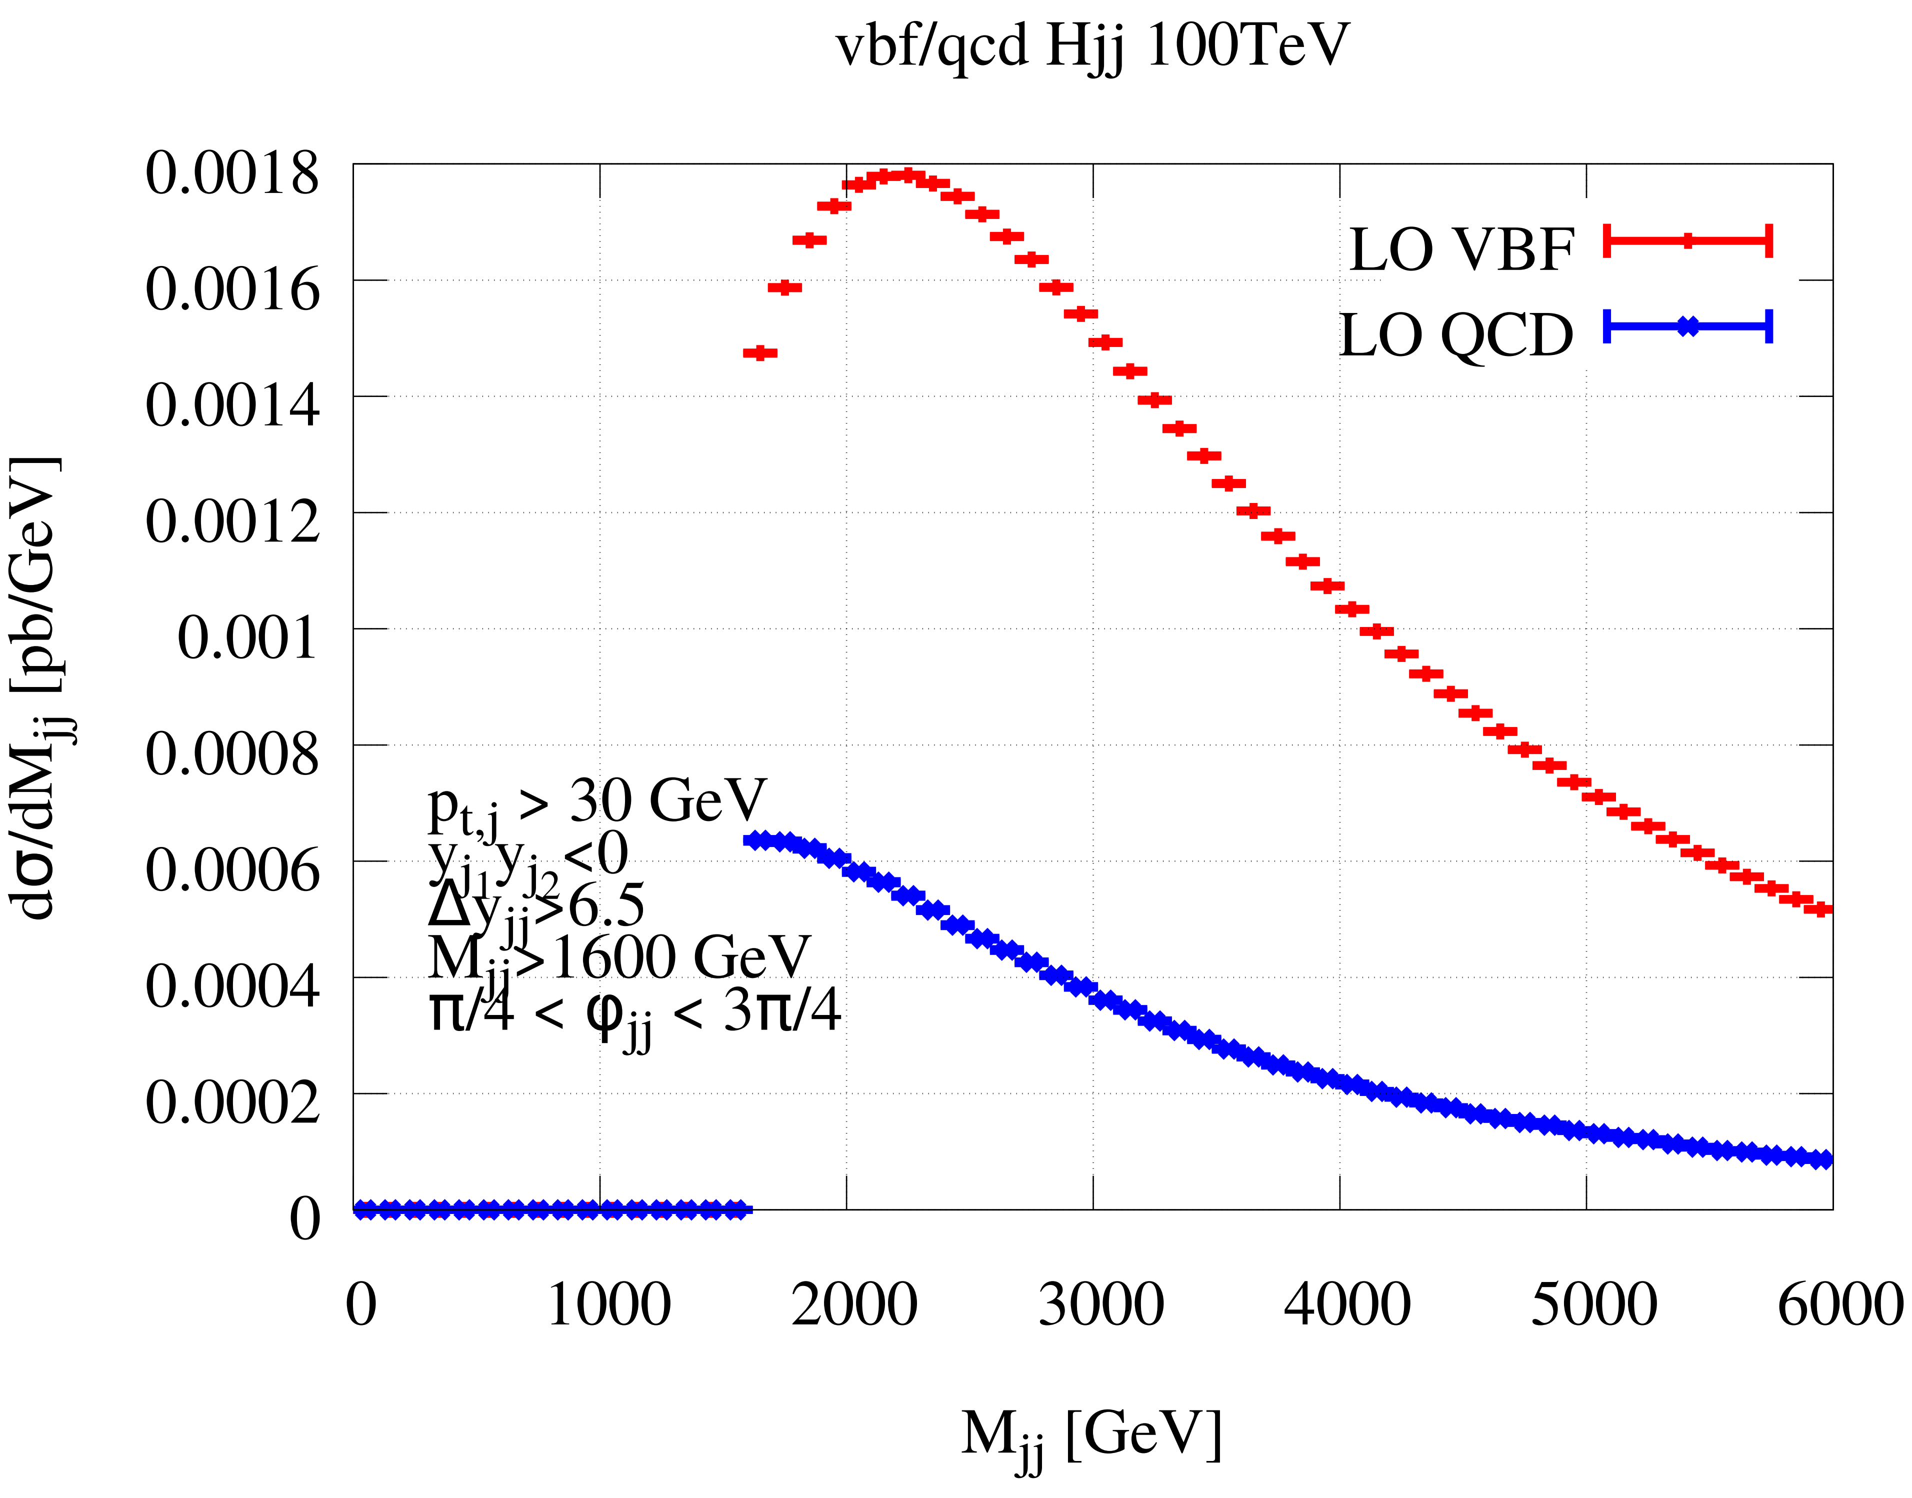

vbf/qcd Hjj 100TeV
LO VBF
LO QCD
$p_{t,j}$ > 30 GeV
$y_{j_1} y_{j_2}$<0
$\Delta y_{jj}$>6.5
$M_{jj}$>1600 GeV
$\pi/4 < \varphi_{jj} < 3\pi/4$
$d\sigma/dM_{jj}$ [pb/GeV]
$M_{jj}$ [GeV]
0.0018
0.0016
0.0014
0.0012
0.001
0.0008
0.0006
0.0004
0.0002
0
0
1000
2000
3000
4000
5000
6000

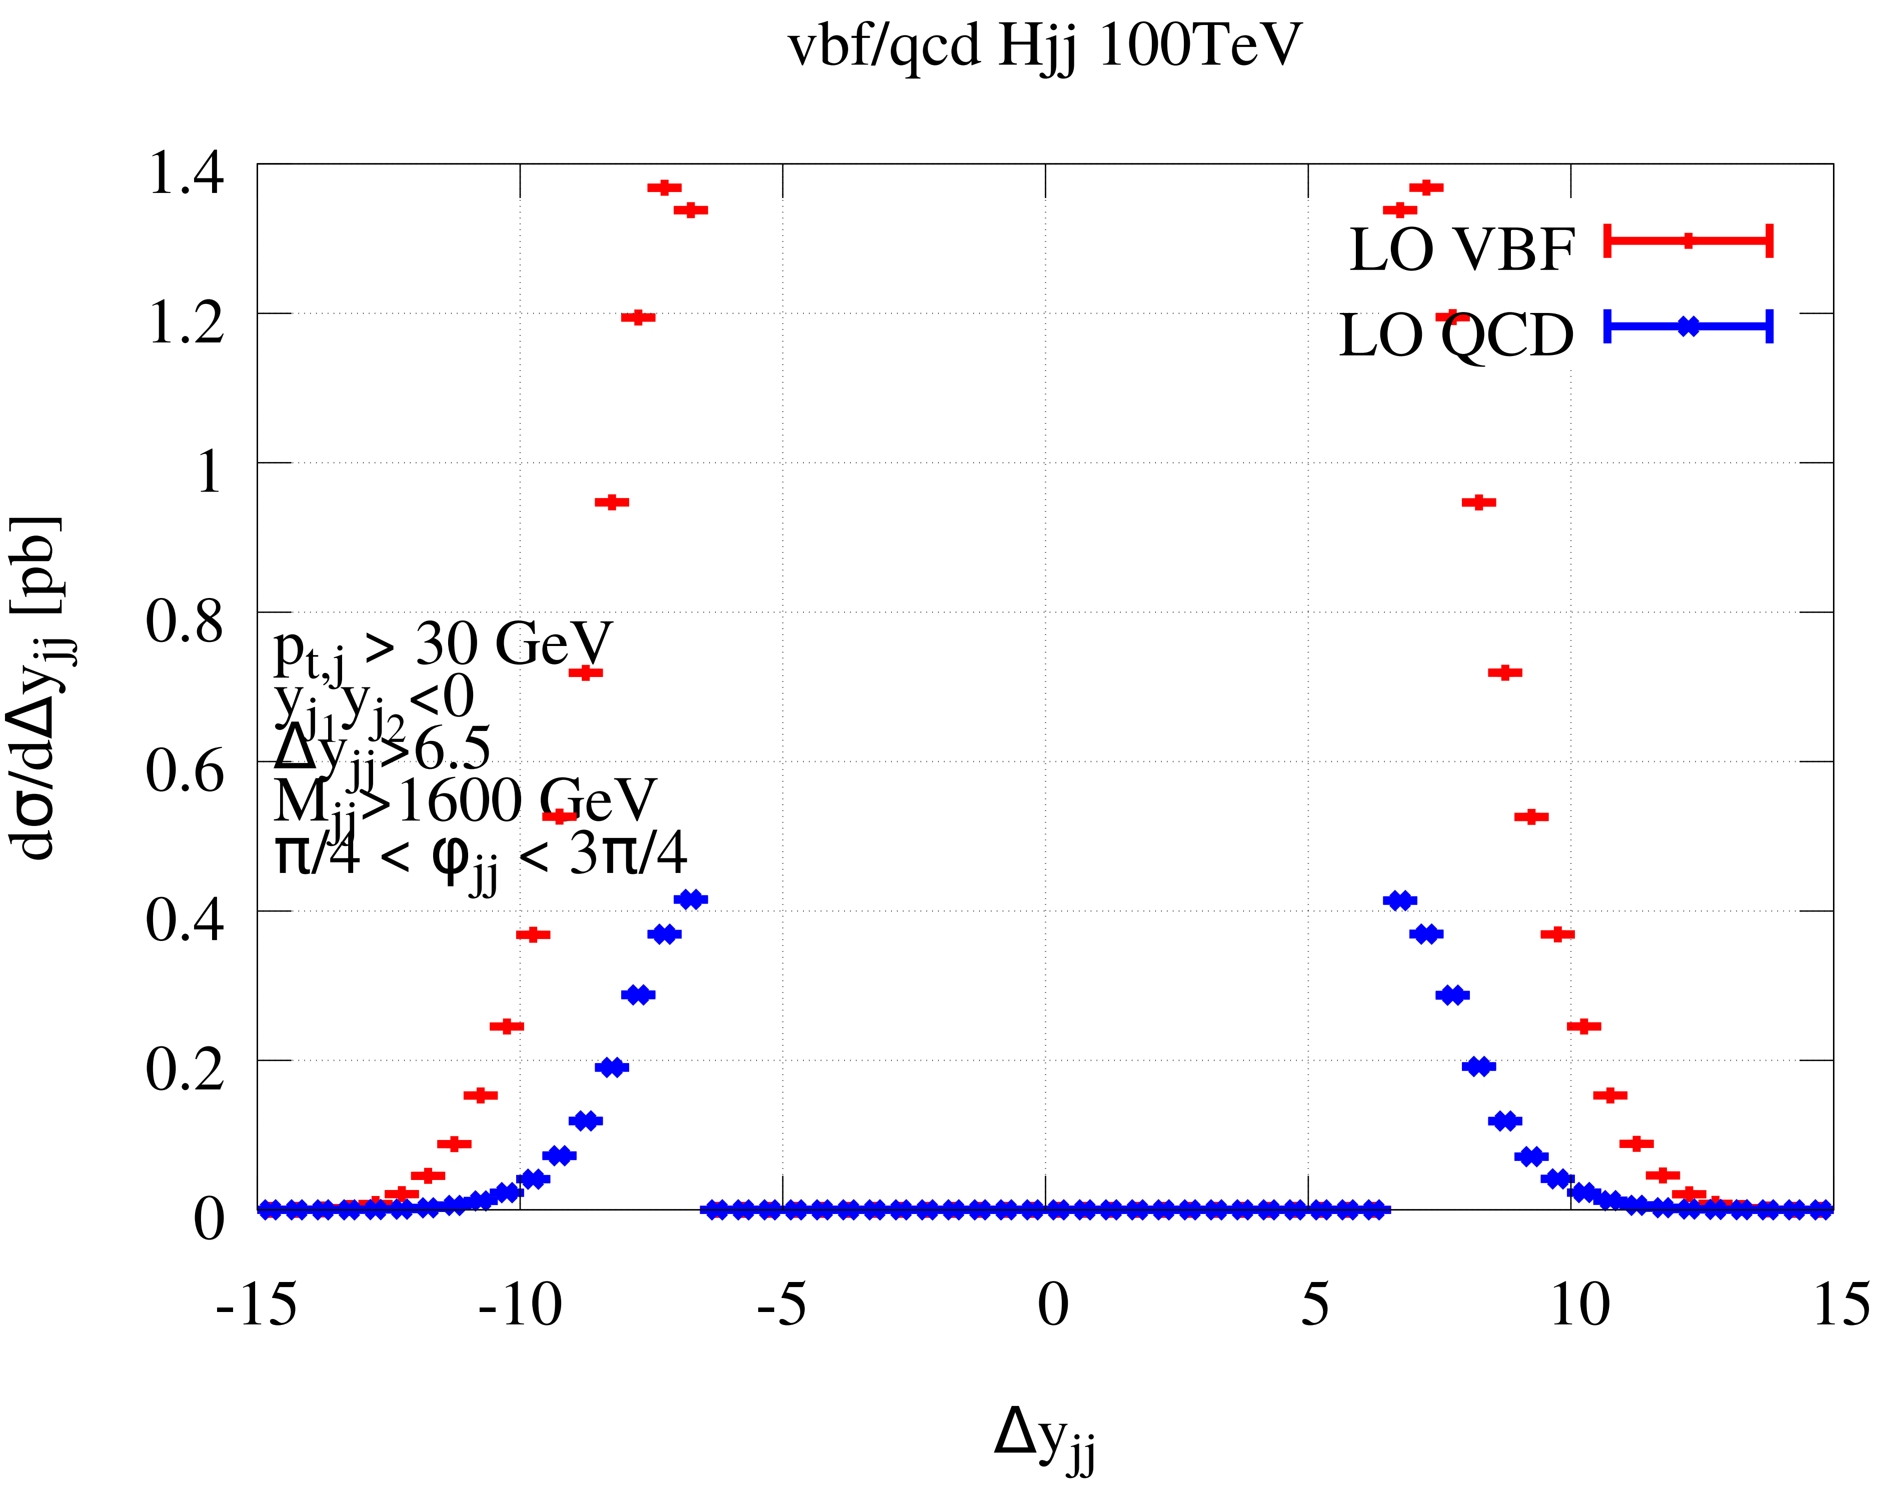
vbf/qcd Hjj 100TeV
LO VBF
LO QCD
$p_{t,j}$ > 30 GeV
$y_{j_1} y_{j_2} < 0$
$\Delta y_{jj} > 6.5$
$M_{jj} > 1600$ GeV
$\pi/4 < \varphi_{jj} < 3\pi/4$
$d\sigma/d\Delta y_{jj}$ [pb]
$\Delta y_{jj}$
1.4
1.2
1
0.8
0.6
0.4
0.2
0
-15
-10
-5
0
5
10
15

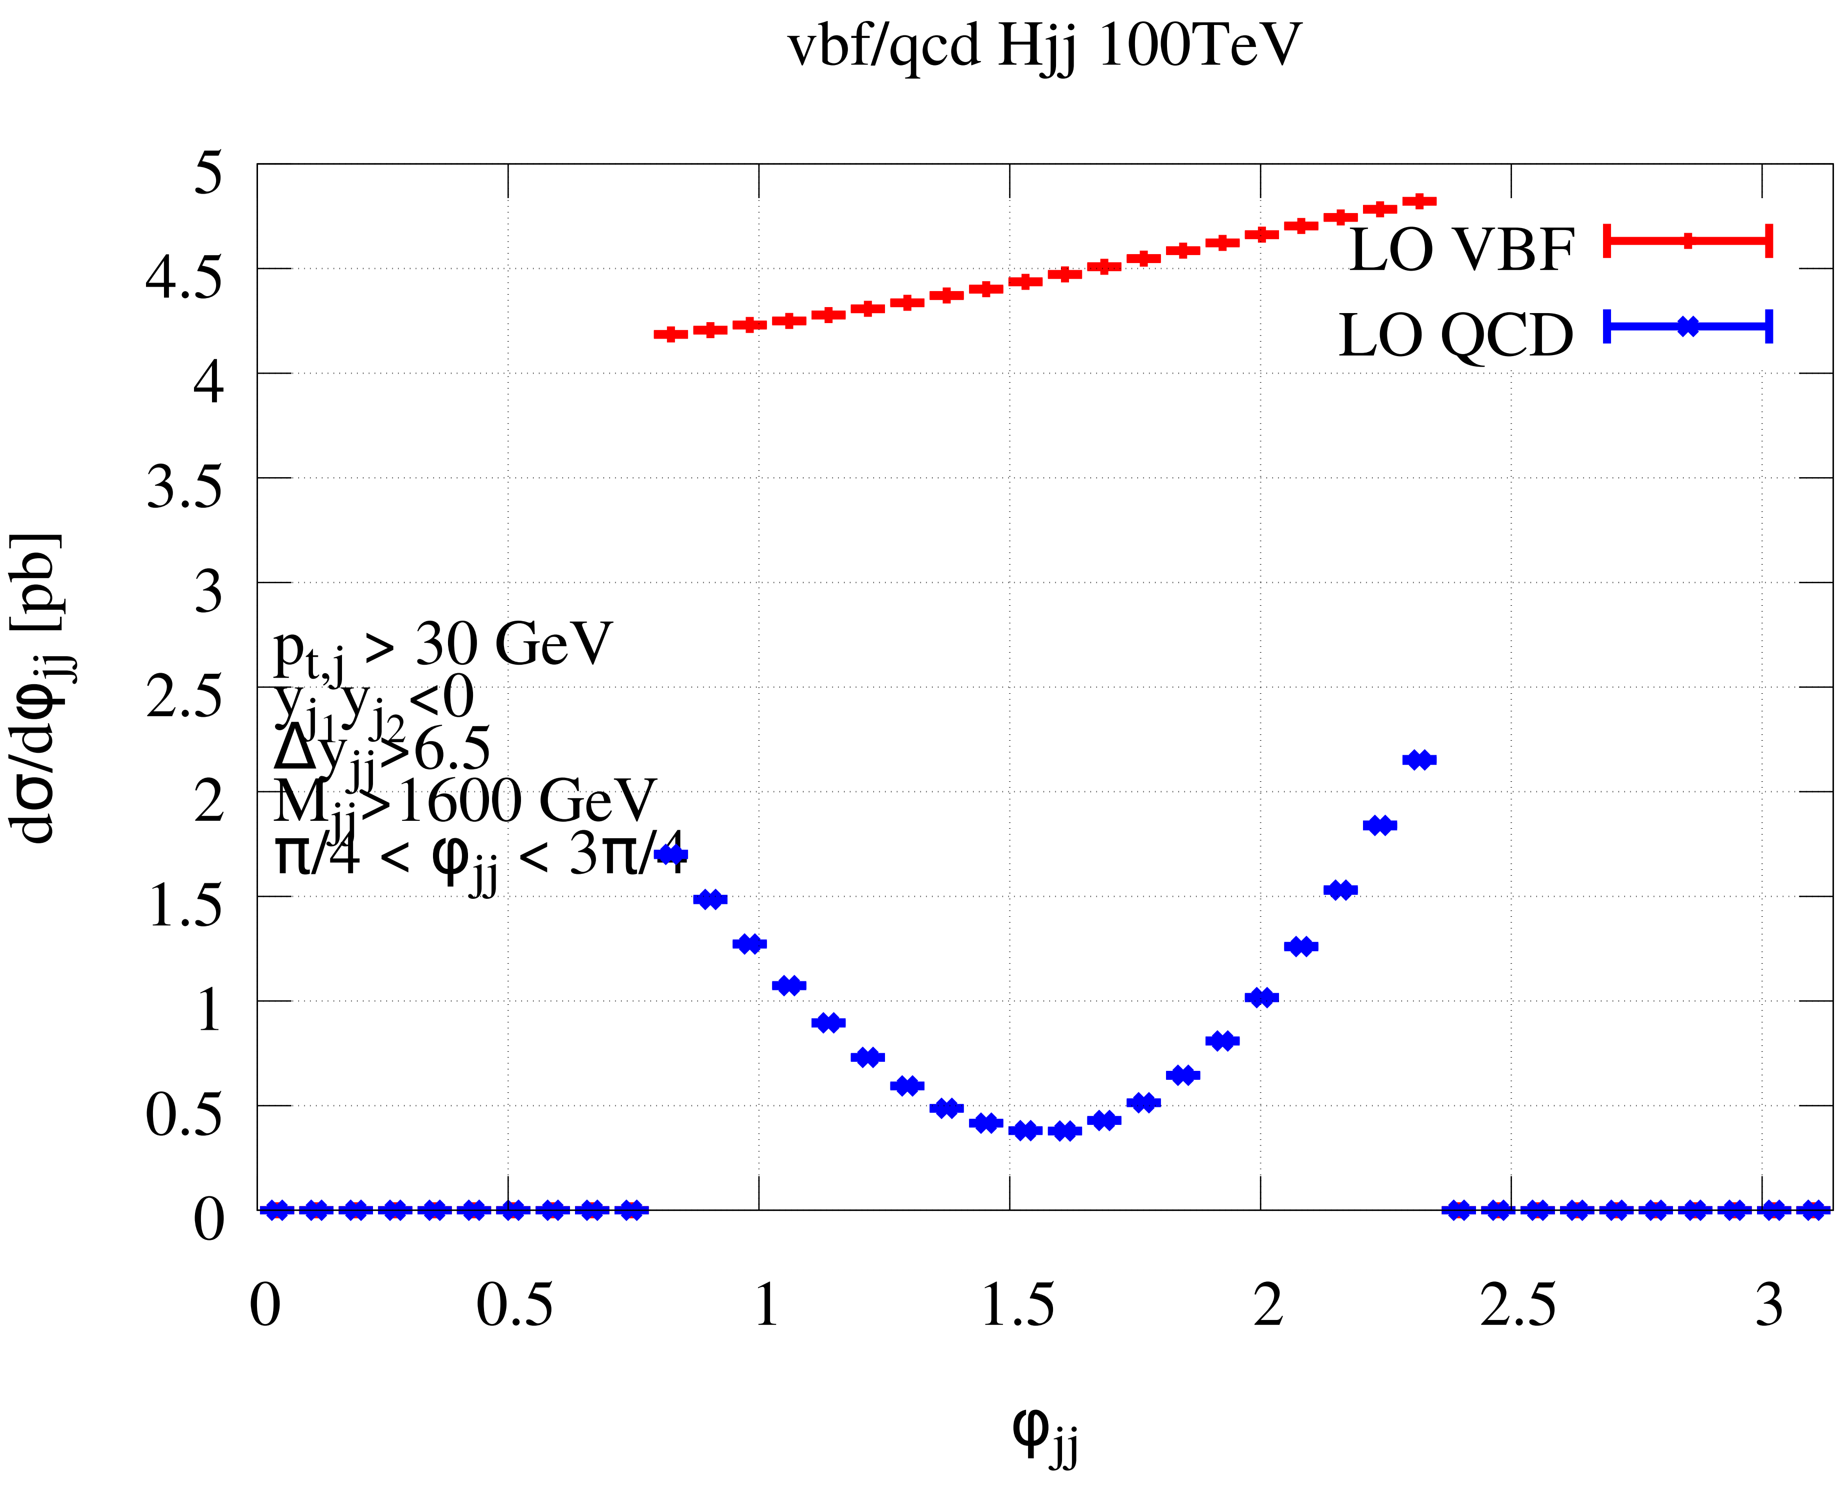

vbf/qcd Hjj 100TeV
LO VBF
LO QCD
$p_{t,j}$ > 30 GeV
$y_{j_1} \cdot y_{j_2}$ <0
$\Delta y_{jj}$>6.5
$M_{jj}$>1600 GeV
$\pi/4 < \varphi_{jj} < 3\pi/4$
$d\sigma/d\varphi_{jj}$ [pb]
$\varphi_{jj}$
0
0.5
1
1.5
2
2.5
3
3.5
4
4.5
5

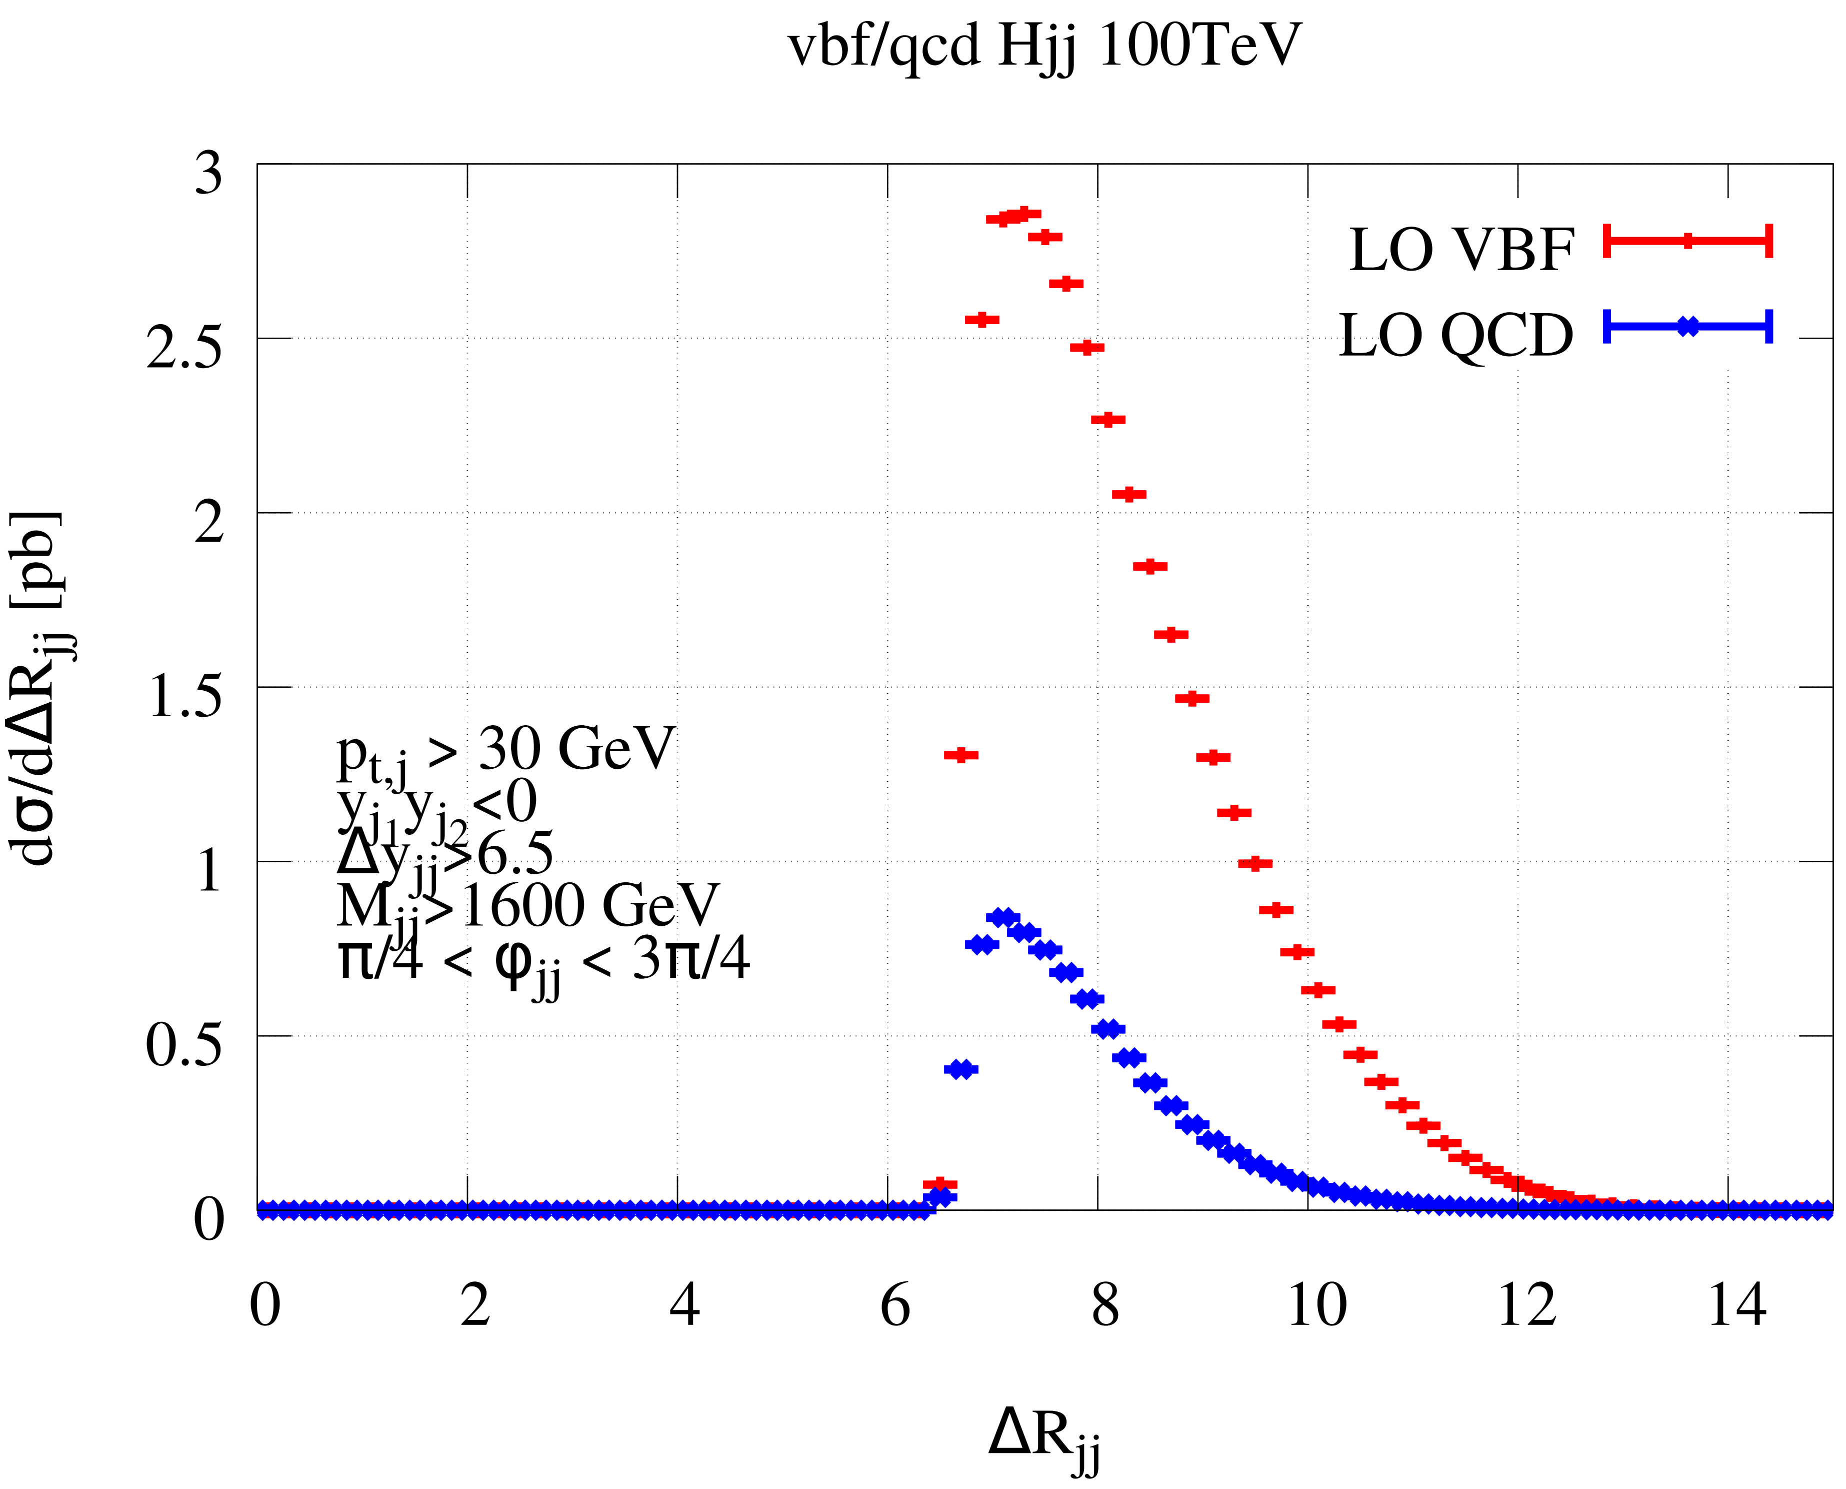

vbf/qcd Hjj 100TeV
LO VBF
LO QCD
$p_{t,j}$ > 30 GeV
$y_{j_1} y_{j_2}$<0
$\Delta y_{jj}$>6.5
$M_{jj}$>1600 GeV
$\pi/4 < \varphi_{jj} < 3\pi/4$
$d\sigma/d\Delta R_{jj}$ [pb]
$\Delta R_{jj}$
0
0.5
1
1.5
2
2.5
3
0
2
4
6
8
10
12
14

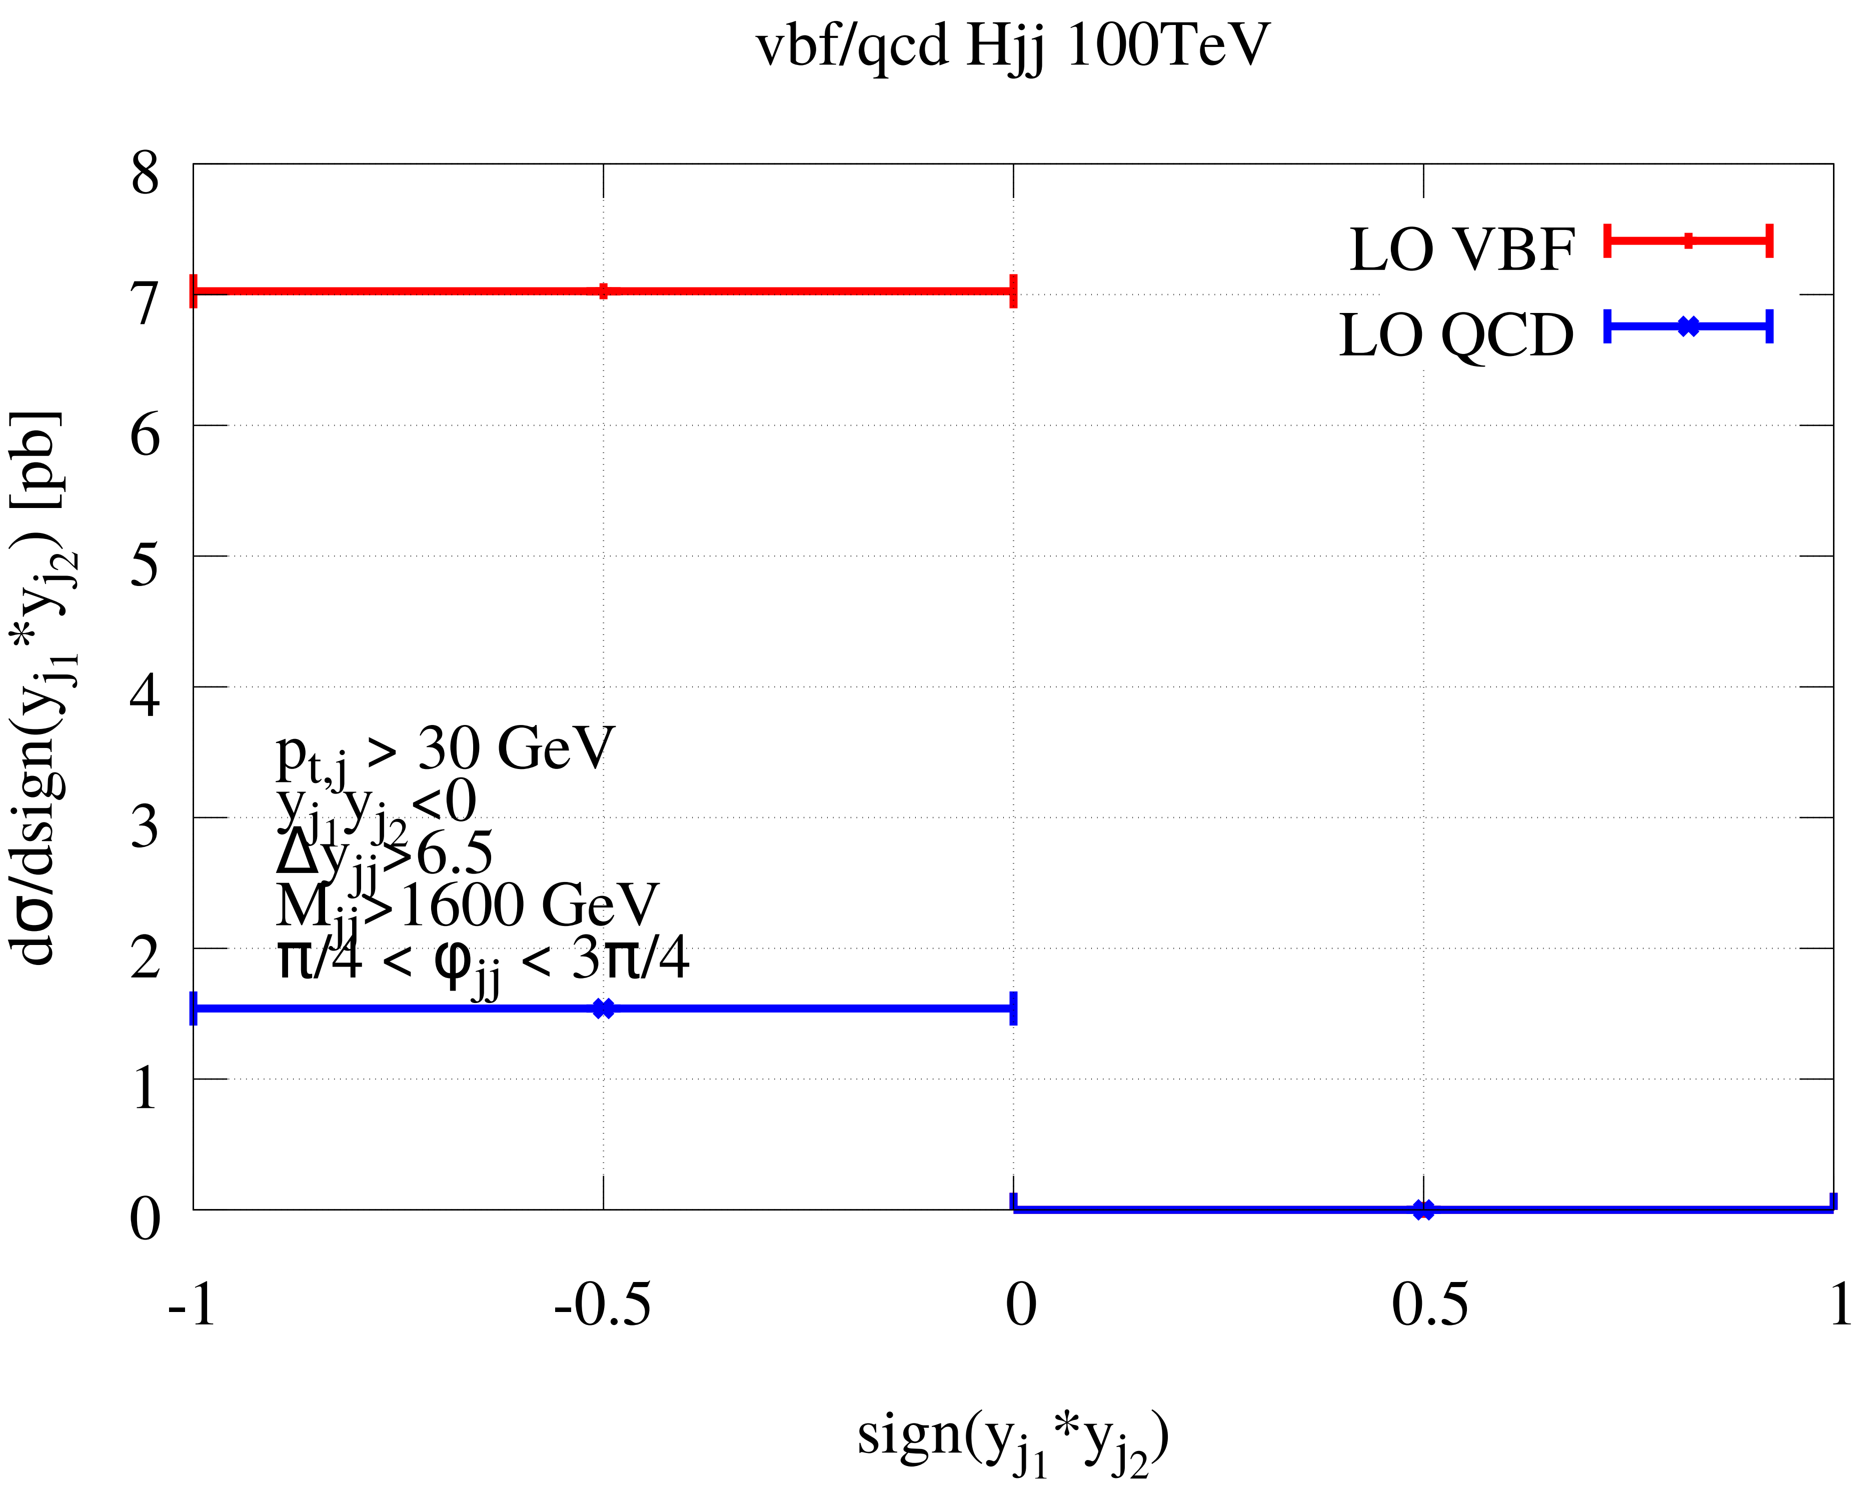

vbf/qcd Hjj 100TeV
LO VBF
LO QCD
$p_{t,j}$ > 30 GeV
$y_{j_1} y_{j_2}$ <0
$\Delta y_{jj}$>6.5
$M_{jj}$>1600 GeV
$\pi/4 < \varphi_{jj} < 3\pi/4$
$d\sigma/dsign(y_{j_1} * y_{j_2})$ [pb]
$sign(y_{j_1} * y_{j_2})$
0
1
2
3
4
5
6
7
8
-1
-0.5
0
0.5
1

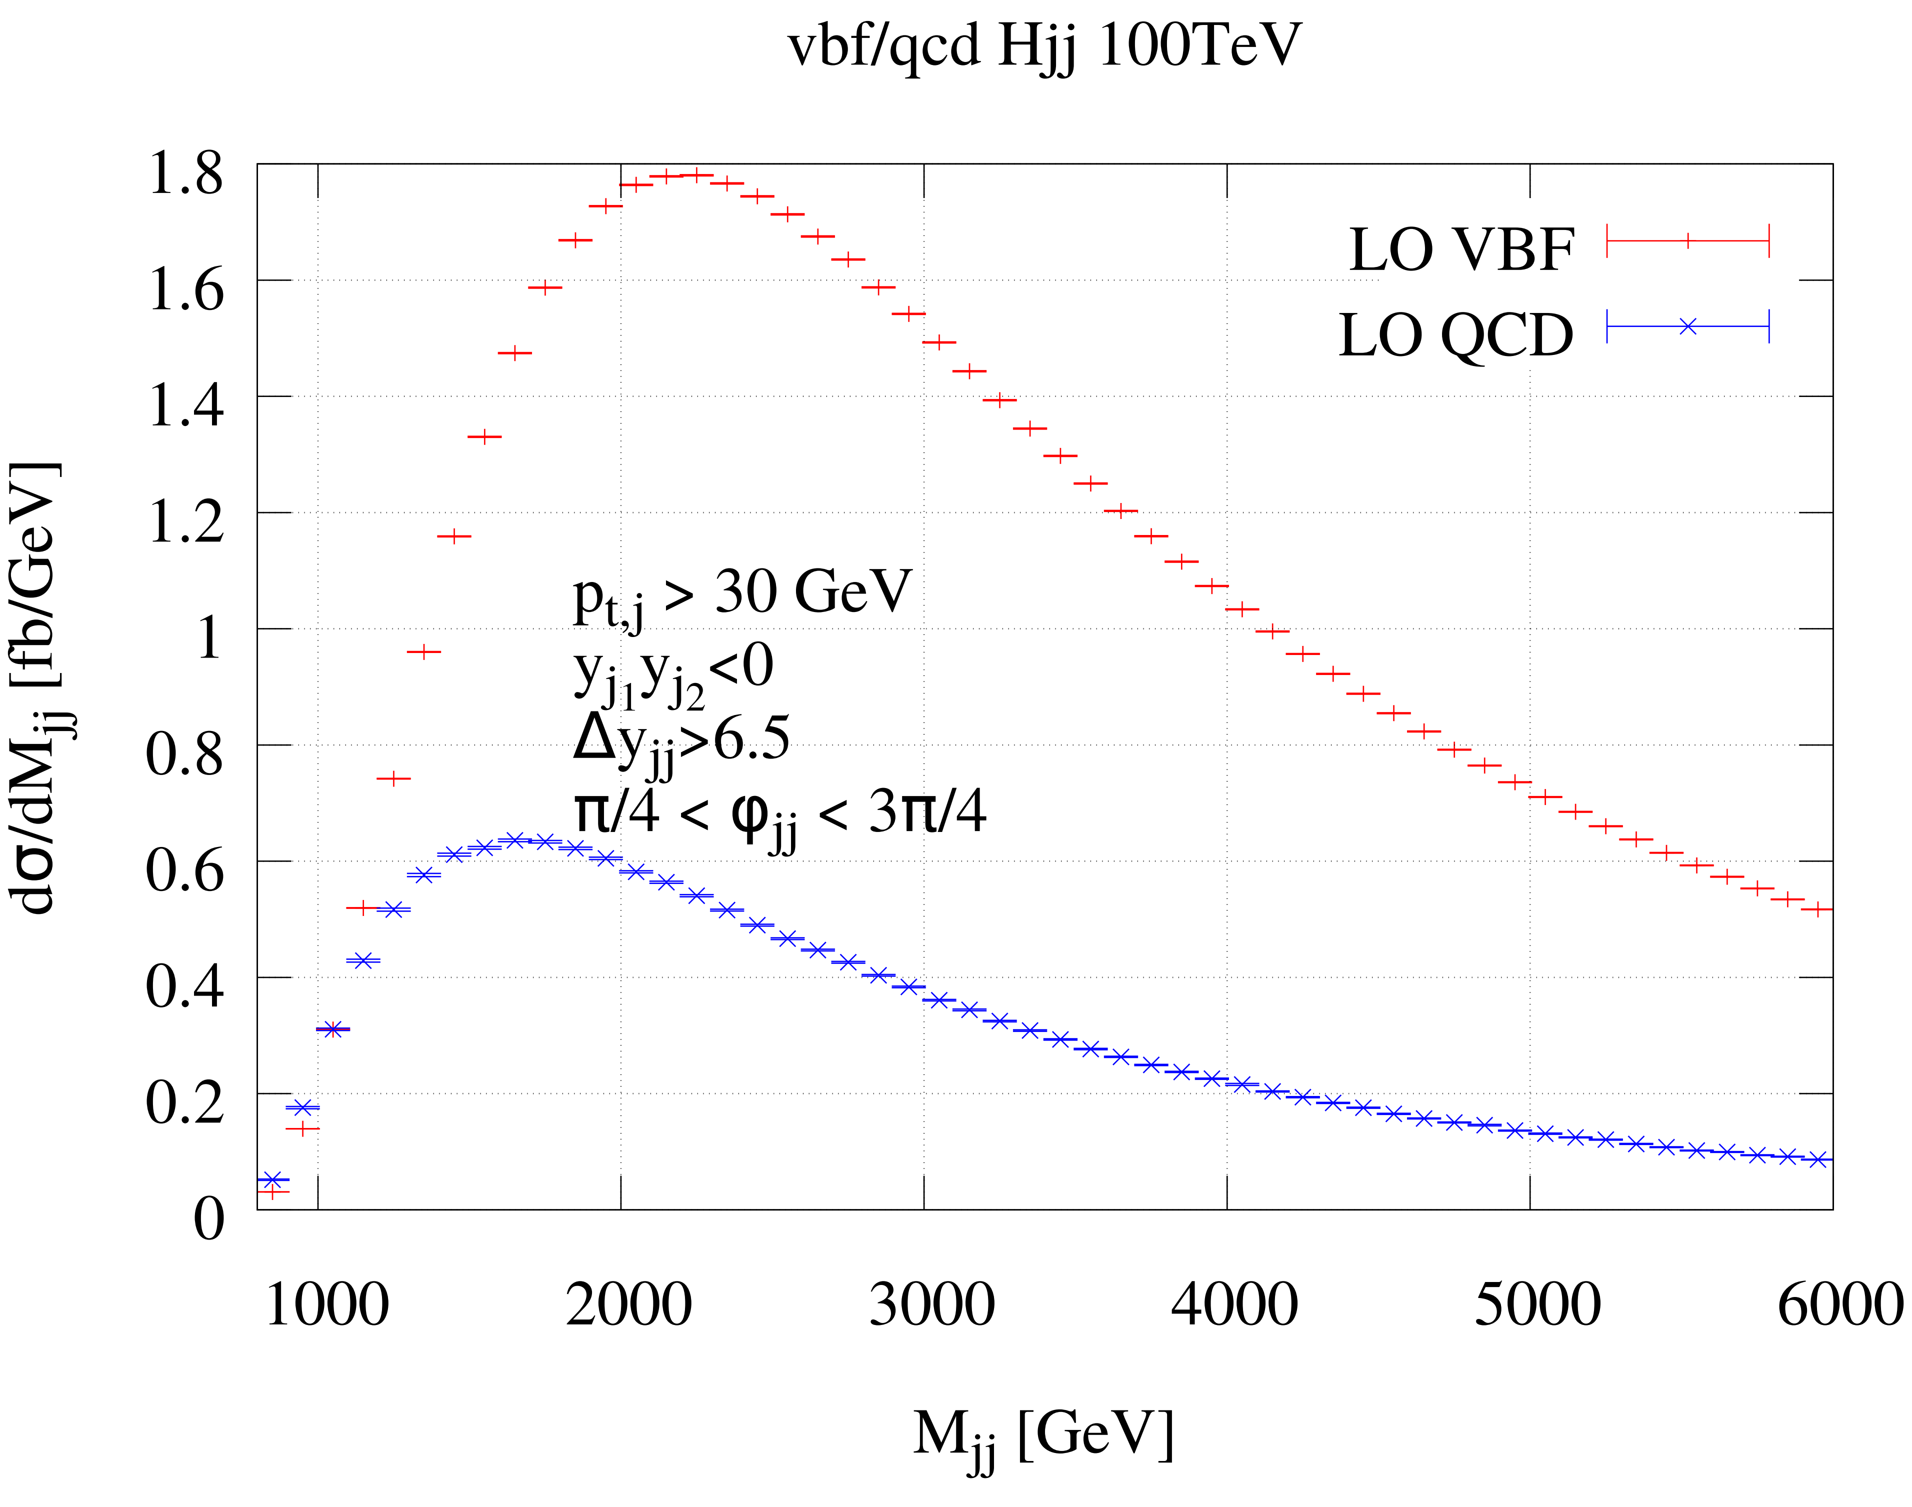

vbf/qcd Hjj 100TeV
LO VBF
LO QCD
$p_{t,j}$ > 30 GeV
$y_{j_1}y_{j_2}$<0
$\Delta y_{jj}$>6.5
$\pi/4 < \varphi_{jj} < 3\pi/4$
$d\sigma/dM_{jj}$ [fb/GeV]
$M_{jj}$ [GeV]
0
0.2
0.4
0.6
0.8
1
1.2
1.4
1.6
1.8
1000
2000
3000
4000
5000
6000

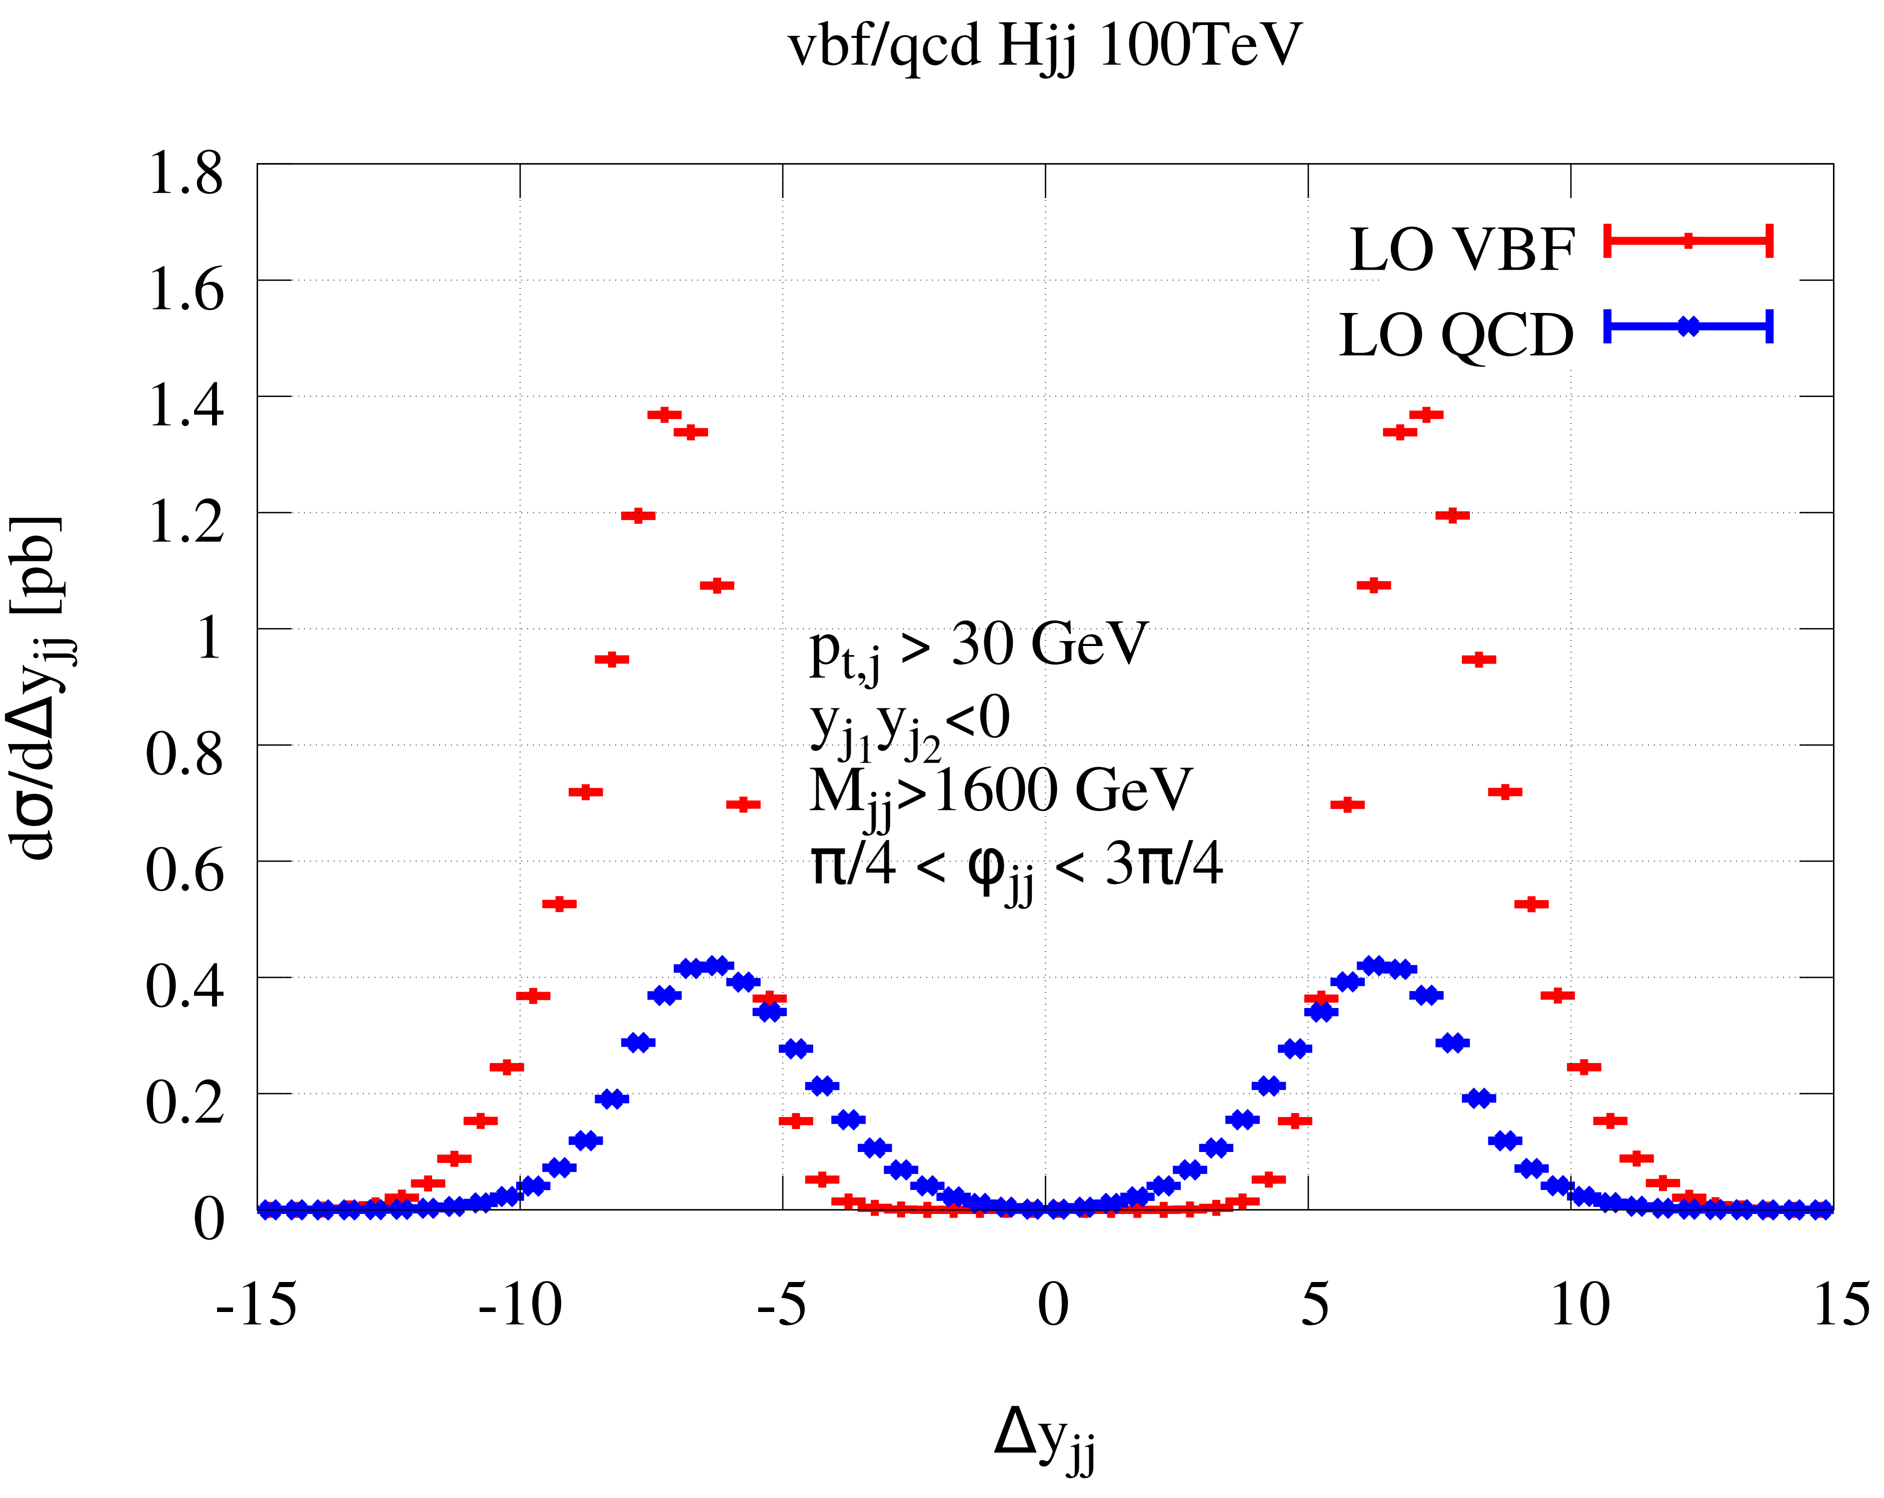

vbf/qcd Hjj 100TeV
LO VBF
LO QCD
$p_{t,j} > 30$ GeV
$y_{j_1} y_{j_2} < 0$
$M_{jj} > 1600$ GeV
$\pi/4 < \varphi_{jj} < 3\pi/4$
$d\sigma/d\Delta y_{jj}$ [pb]
$\Delta y_{jj}$
1.8
1.6
1.4
1.2
1
0.8
0.6
0.4
0.2
0
-15
-10
-5
0
5
10
15

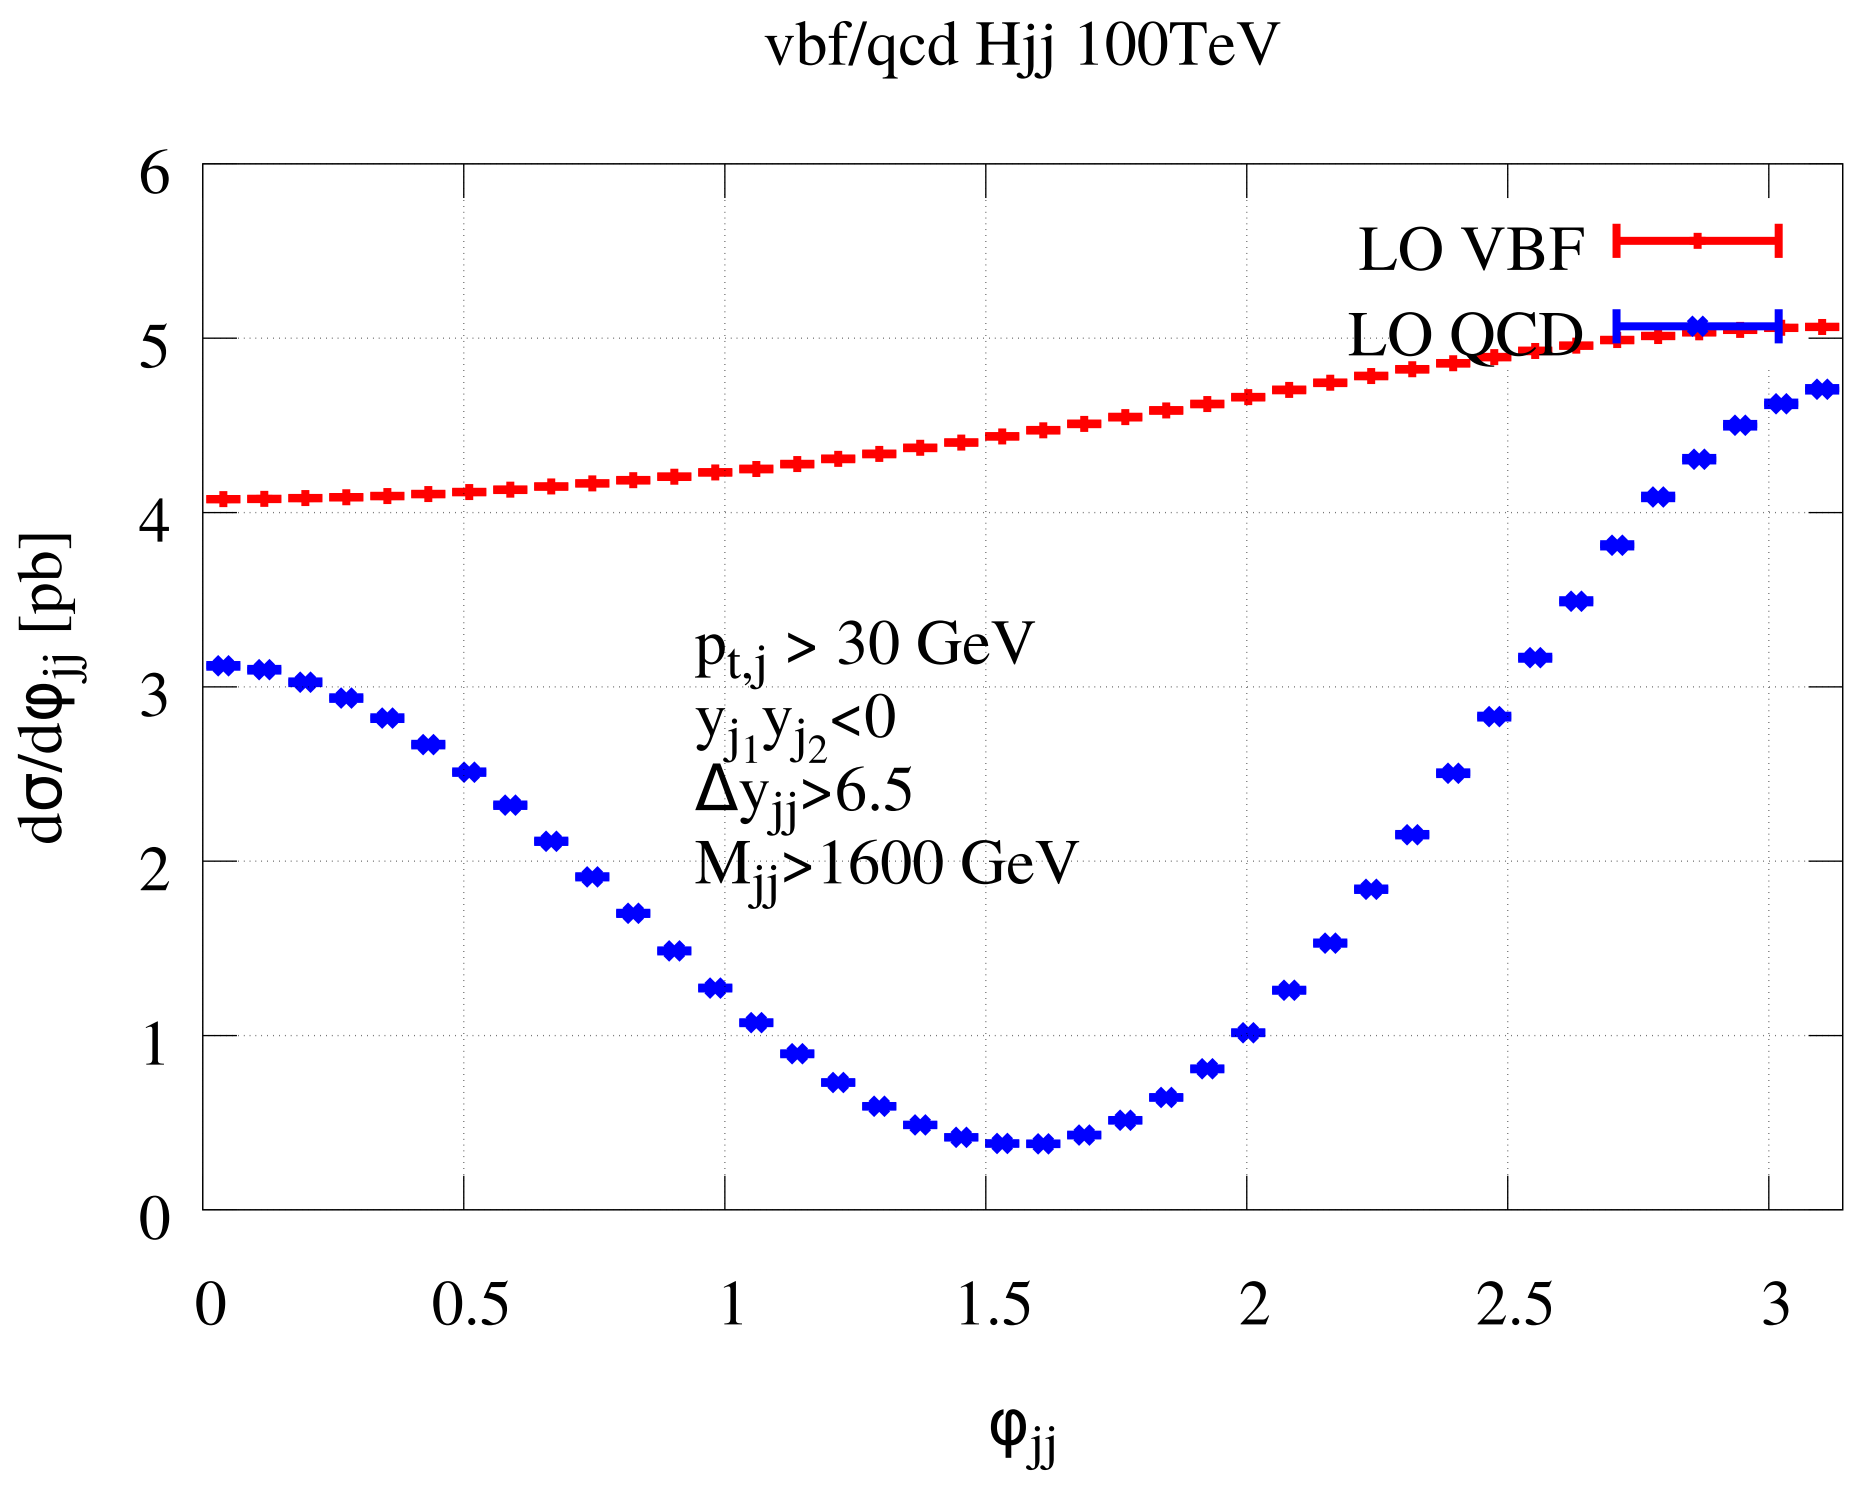
vbf/qcd Hjj 100TeV
LO VBF
LO QCD
$p_{t,j}$ > 30 GeV
$y_{j_1}y_{j_2}<0$
$\Delta y_{jj}>6.5$
$M_{jj}>1600$ GeV
$d\sigma/d\varphi_{jj}$ [pb]
$\varphi_{jj}$
0
1
2
3
4
5
6
0
0.5
1
1.5
2
2.5
3

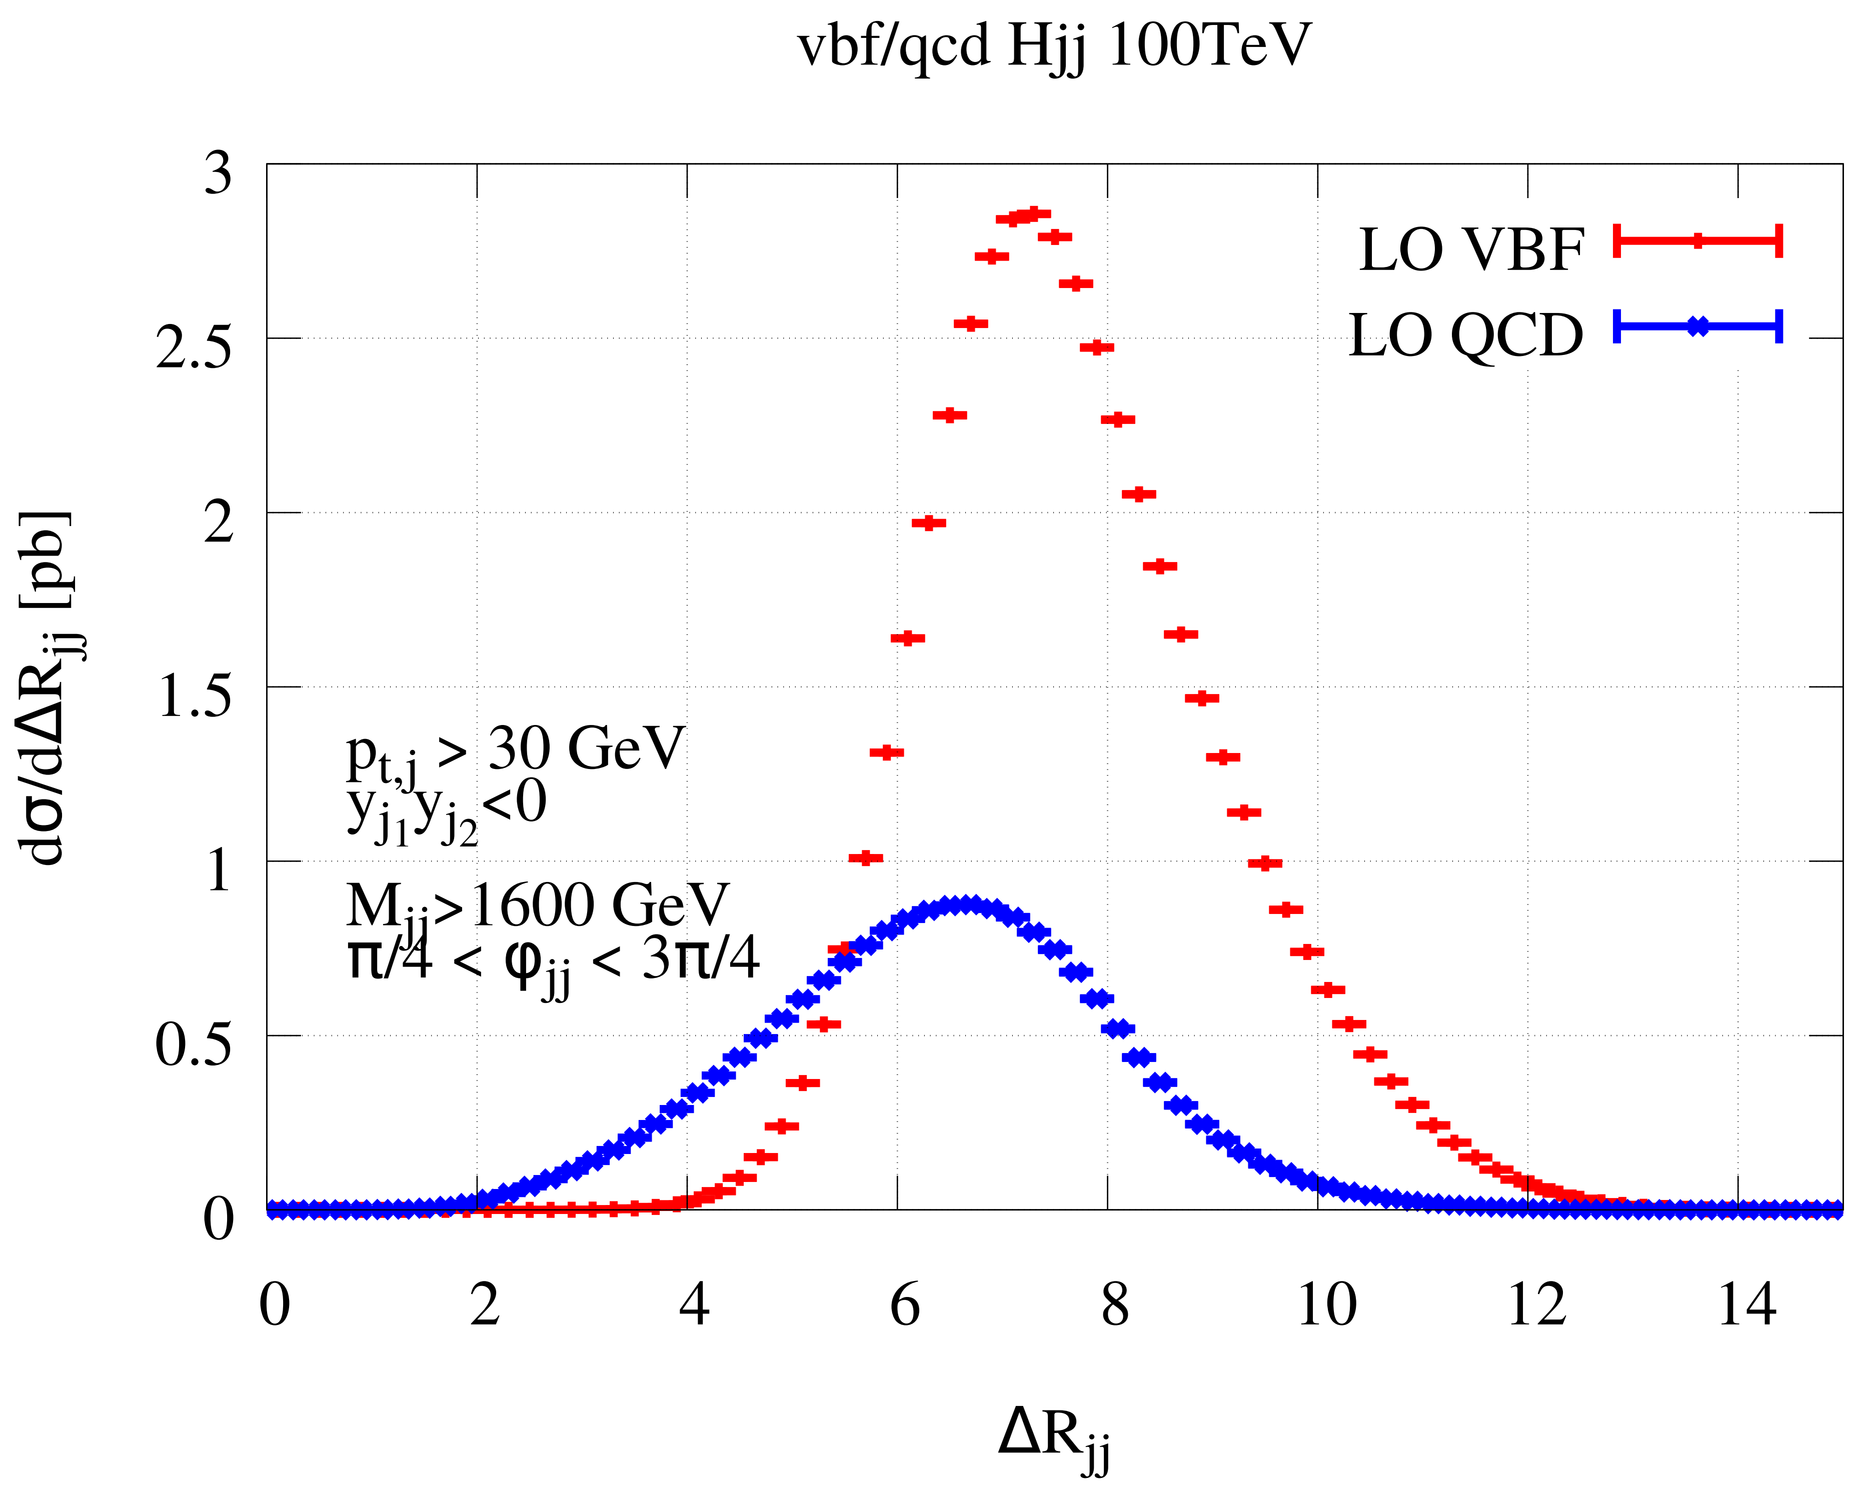
vbf/qcd Hjj 100TeV
LO VBF
LO QCD
$p_{t,j}$ > 30 GeV
$y_{j_1}y_{j_2}$<0
$M_{jj}$>1600 GeV
$\pi/4 < \varphi_{jj} < 3\pi/4$
$d\sigma/d\Delta R_{jj}$ [pb]
$\Delta R_{jj}$
0
0.5
1
1.5
2
2.5
3
0
2
4
6
8
10
12
14

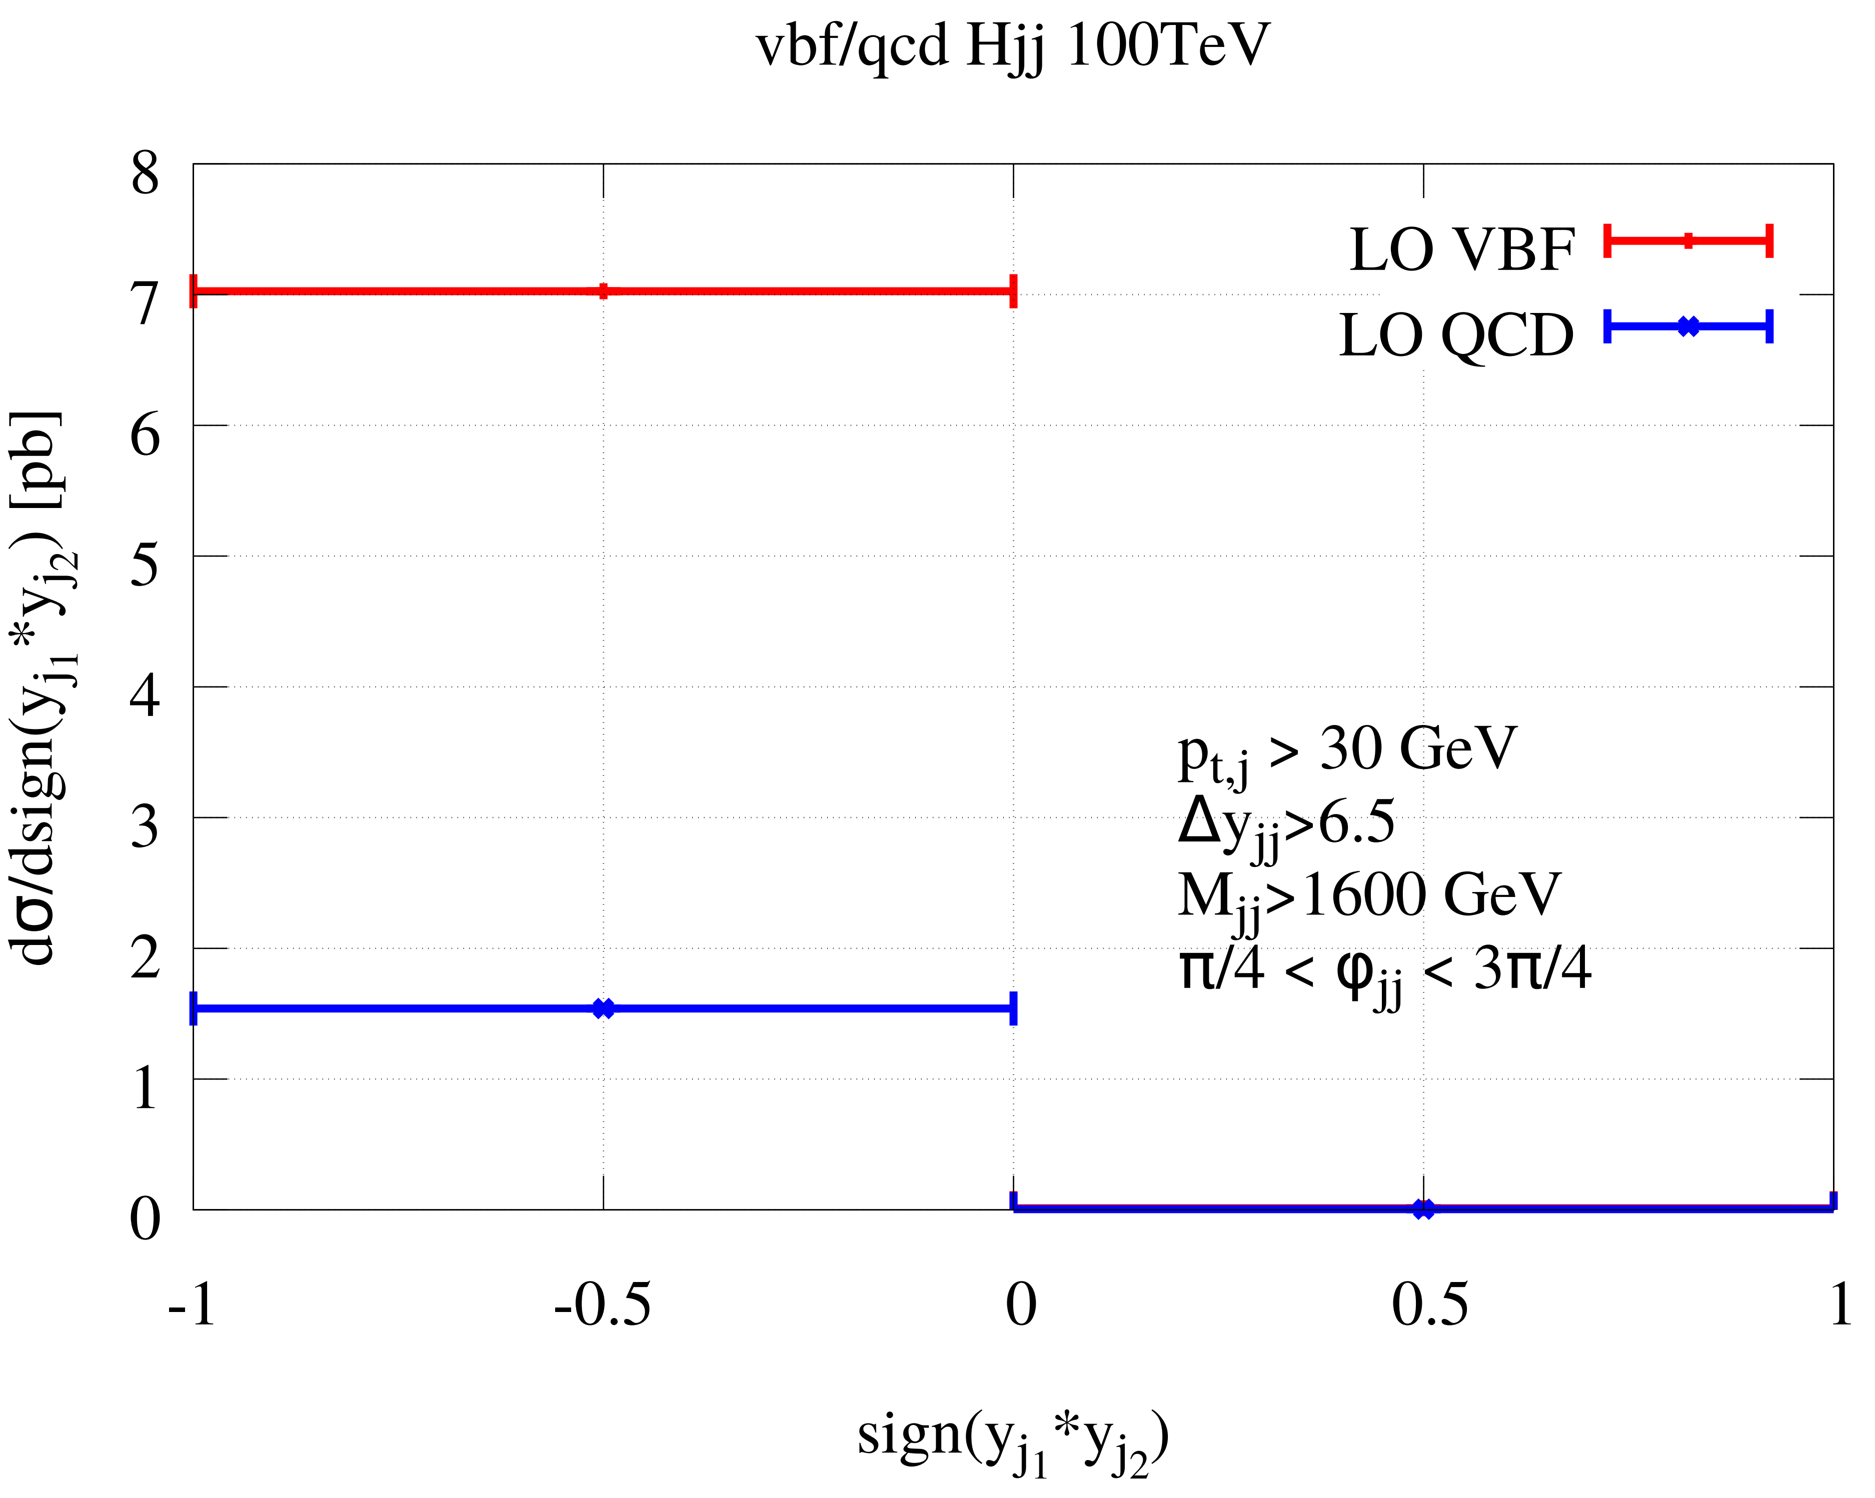

vbf/qcd Hjj 100TeV
LO VBF
LO QCD
$p_{t,j}$ > 30 GeV
$\Delta y_{jj}$>6.5
$M_{jj}$>1600 GeV
$\pi/4 < \varphi_{jj} < 3\pi/4$
$d\sigma/d\mathrm{sign}(y_{j_1}*y_{j_2})$ [pb]
$\mathrm{sign}(y_{j_1}*y_{j_2})$
0
1
2
3
4
5
6
7
8
-1
-0.5
0
0.5
1

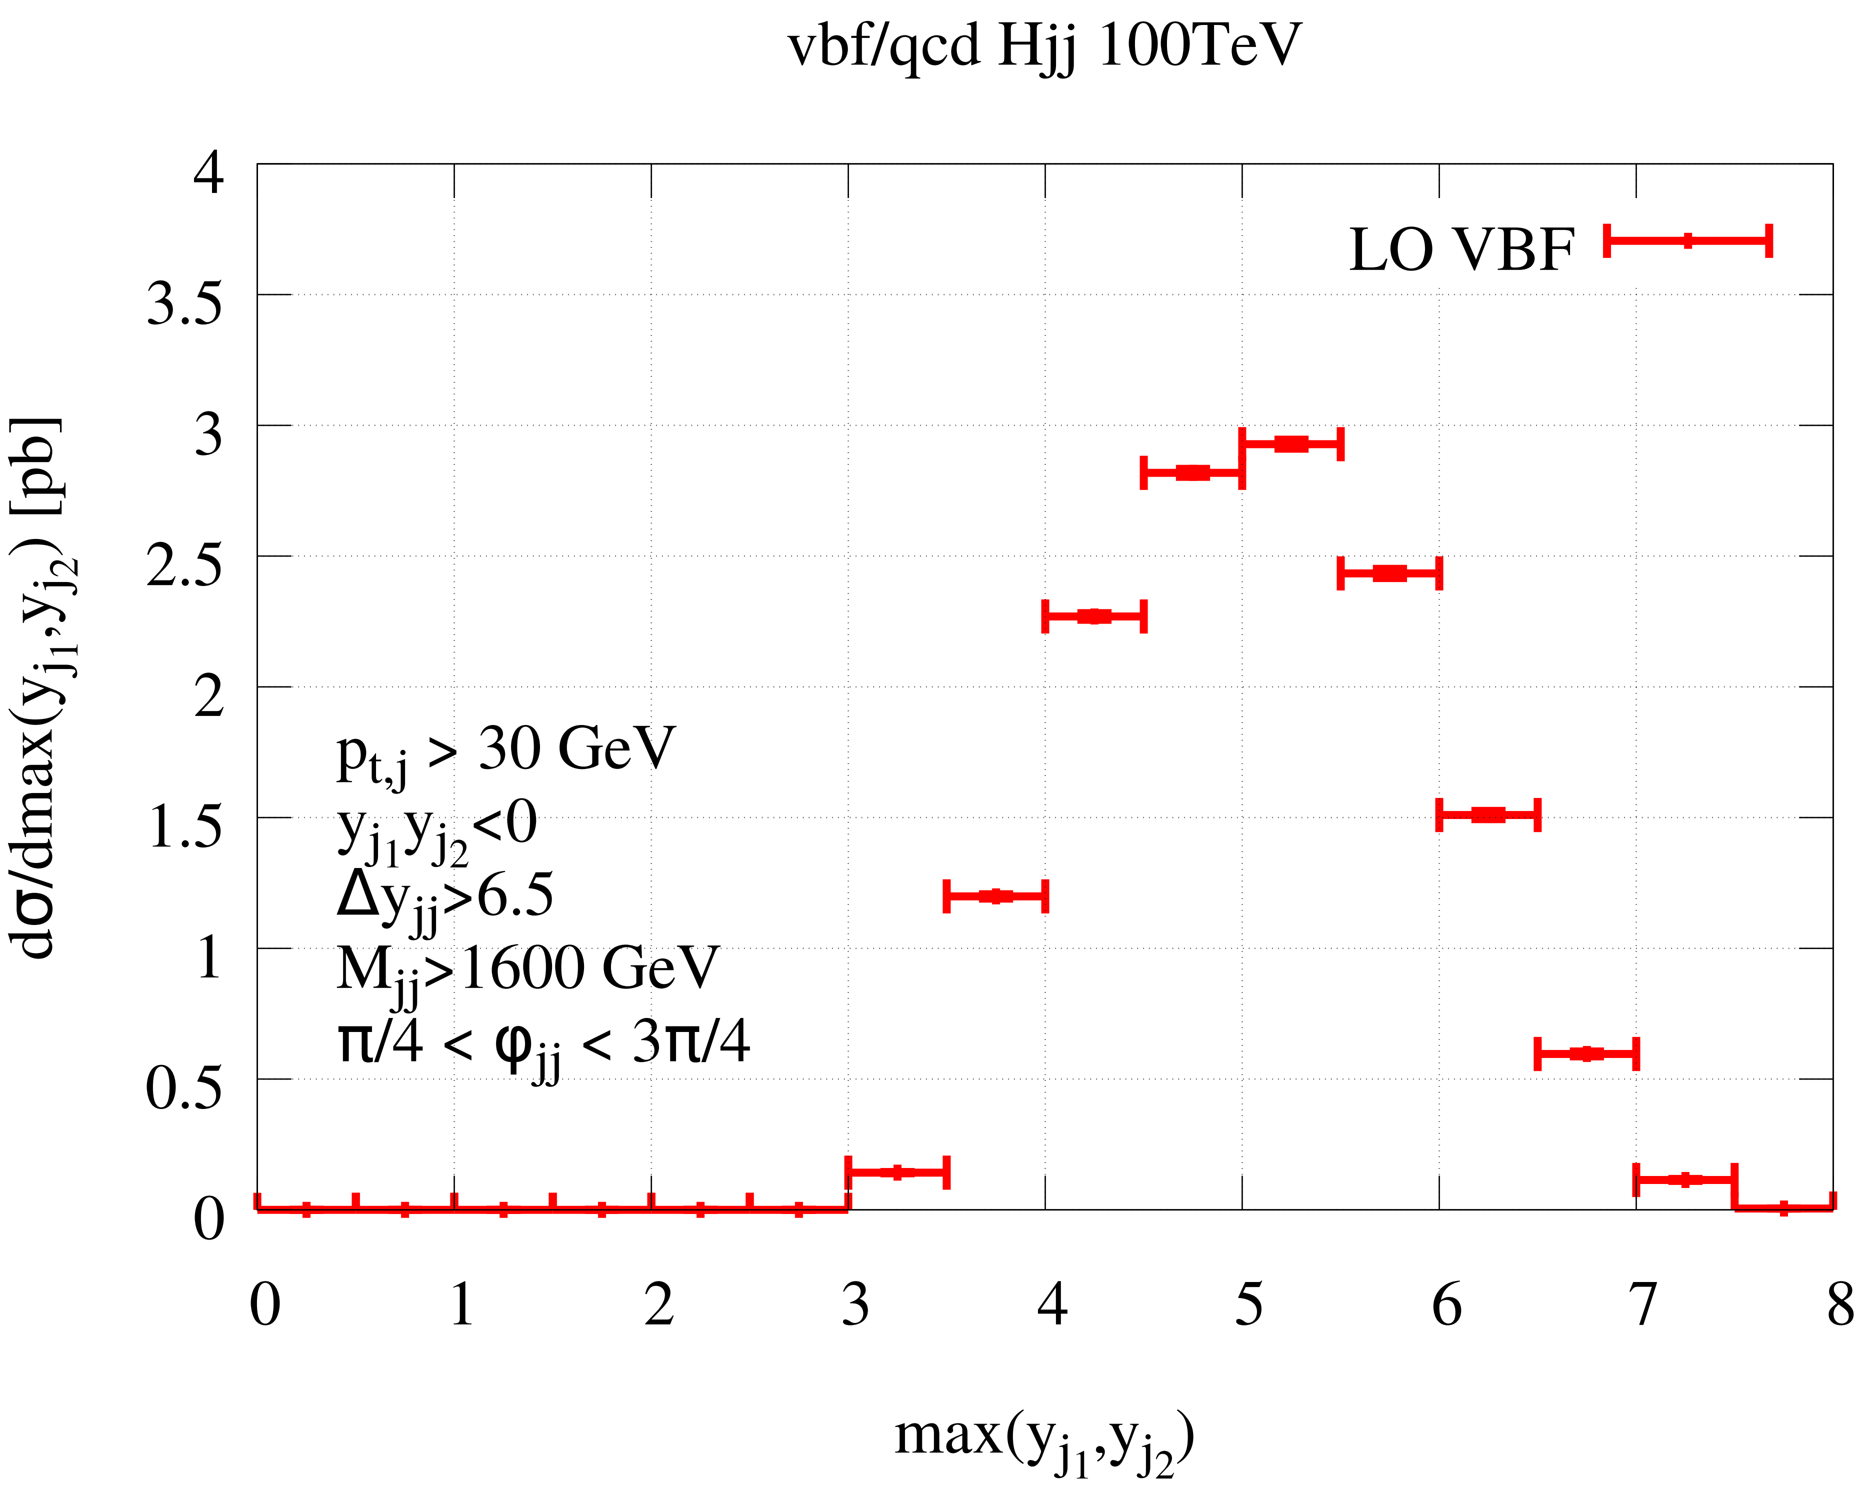
vbf/qcd Hjj 100TeV
LO VBF
$p_{t,j}$ > 30 GeV
$y_{j_1}y_{j_2}$<0
$\Delta y_{jj}$>6.5
$M_{jj}$>1600 GeV
$\pi/4 < \varphi_{jj} < 3\pi/4$
$d\sigma/d\max(y_{j_1},y_{j_2})$ [pb]
$\max(y_{j_1},y_{j_2})$
0
0.5
1
1.5
2
2.5
3
3.5
4
0
1
2
3
4
5
6
7
8
