# Supplementary material for: Physics at a 100 TeV pp collider: Higgs and EW symmetry breaking studies
Source: arXiv:1606.09408 source file (2016-06-30)
Supplement: Supplementary file 2 [file prospects_summary.tex]

\subsection{Final remarks}
The primary goal of the
  studies shown in this Section was to show that, while theoretical systematics in
  hadronic collisions are typically the key limitation to Higgs
  precision physics, there are examples where these can be reduced
  even using today's knowledge, and there are examples where the large
  statistics allows to identify robust observables (e.g. ratios of
  BRs) where the precision can in principle achieve the percent level.
    What must be explored is the extent to which the performance of
    future detectors can match this accuracy.
    The results shown here can then serve as benchmarks for the definition of
  the performance goals of future detectors.

  To first
  approximation, we believe that the basic experimental systematics
  that appear in the extraction of absolute cross sections
  (luminosity, tagging and identification efficiencies for the various
  physics objects, backgrounds) will cancel in the measurement of
  several Higgs production ratios. the
  ${N_H}/{N_Z}$ ratio. Given the cuts we introduced, the $t$,
  $\bar{t}$ and $H/Z$ objects will be separated from each other, and
  have $p_T$ and angular distributions very similar in the $t\bar{t}H$
  and $t\bar{t}Z$ cases. Therefore the leading uncertainties in the
  $b$ or top tagging efficiencies, or in other important quantities
  such as lepton isolation and identification, will cancel. The
  remaining systematics will arise  from the differences
  in detector response due to the slight kinematical differences. We
  find it reasonable to expect that, for a quantity such as the $b$
  tagging efficiency, which is typically known to within few percent,
  it should be possible to control the relative difference between the
  efficiency in $H\to b\bar{b}$ and in $Z\to b\bar{b}$ decays. No
  study at the level of what can be done using the simplified tools
  available to us can give compelling proof of this statement, and we
  propose that studies of systematics for these ratios of efficiencies
  should be interesting goals for more realistic performance studies of
  future detectors.

We would also like to add that the huge rates at 100~TeV will give
  many high-statistics control samples, which can be used for
  data-driven precise determinations of backgrounds or
  efficiencies. As a relevant example, we briefly mention here the
  case of: 
\begin{equation}
 pp \to Z Z \to \ell^+ \ell^- b \bar{b} \; .
\end{equation}
A precision measurement of the corresponding rate, relative to the
$ZZ\to 4\ell$ final state, could allow an absolute measurement of the
$b$-tagging efficiency. With a cross section $\sigma(ZZ) = 200$~pb we
expect $\sim 1.5 \cdot10^7$ ($\sim 0.5 \cdot10^7$)
$ZZ\to\ell^+\ell^-b\bar{b}$ ($ZZ\to 4\ell$) events in 20~\iab.
After including efficiencies, cuts, and even a stiff cut on $p_T(Z \to
\ell^+ \ell^-)$ to boost the recoiling $Z \to b\bar{b}$, it should be
possible to reach a sub-percent-level statistical precision.
