# Supplementary material for: Physics at a 100 TeV pp collider: Higgs and EW symmetry breaking studies
Source: arXiv:1606.09408 source file (2016-06-30)
Supplement: Supplementary file 3 [file report.tex]

% Few simple rules to ensure that we you can pdfplatex your section
% locally, while maintaining the ability to pdflatex the full
% document from the home directory:

% Don't touch any of the calls in this file. 

% If you want to break the section into multiple subsection files, embed
% the \input{subsectionX} calls into the file section.tex

% Subsection files must then stay in the same folder as section.tex,
% and their figures should all stay in the figs/ subdirectory

% All references should included using the bibtex format, and must be
% added to the master report.bib file sitting in the main directory

% If you want to add new tex macros (mostly definitions or new
% commands), include them in your local section.tex file. But first
% make sure you are not overriding the macros already included in the
% main_macros.tex file sitting in the home directory. When processing
% the whole report, each subsection will then call properly its own
% macros, and properly use the master macros

% If you want to collect your macros in a file, you should then input
% it from the file section.tex or 
% from the subsection files, but it should NOT be called
% ``main_macros.tex'' (e.g. call it sectionname_macros.tex)

\input{../header}
\input{../title}
\input{../main_macros}

\input{section}

\bibliographystyle{../report}
\bibliography{../report}

\end{document}
