# Supplementary material for: Physics at a 100 TeV pp collider: Higgs and EW symmetry breaking studies
Source: arXiv:1606.09408 source file (2016-06-30)

# VBFH 100TeV

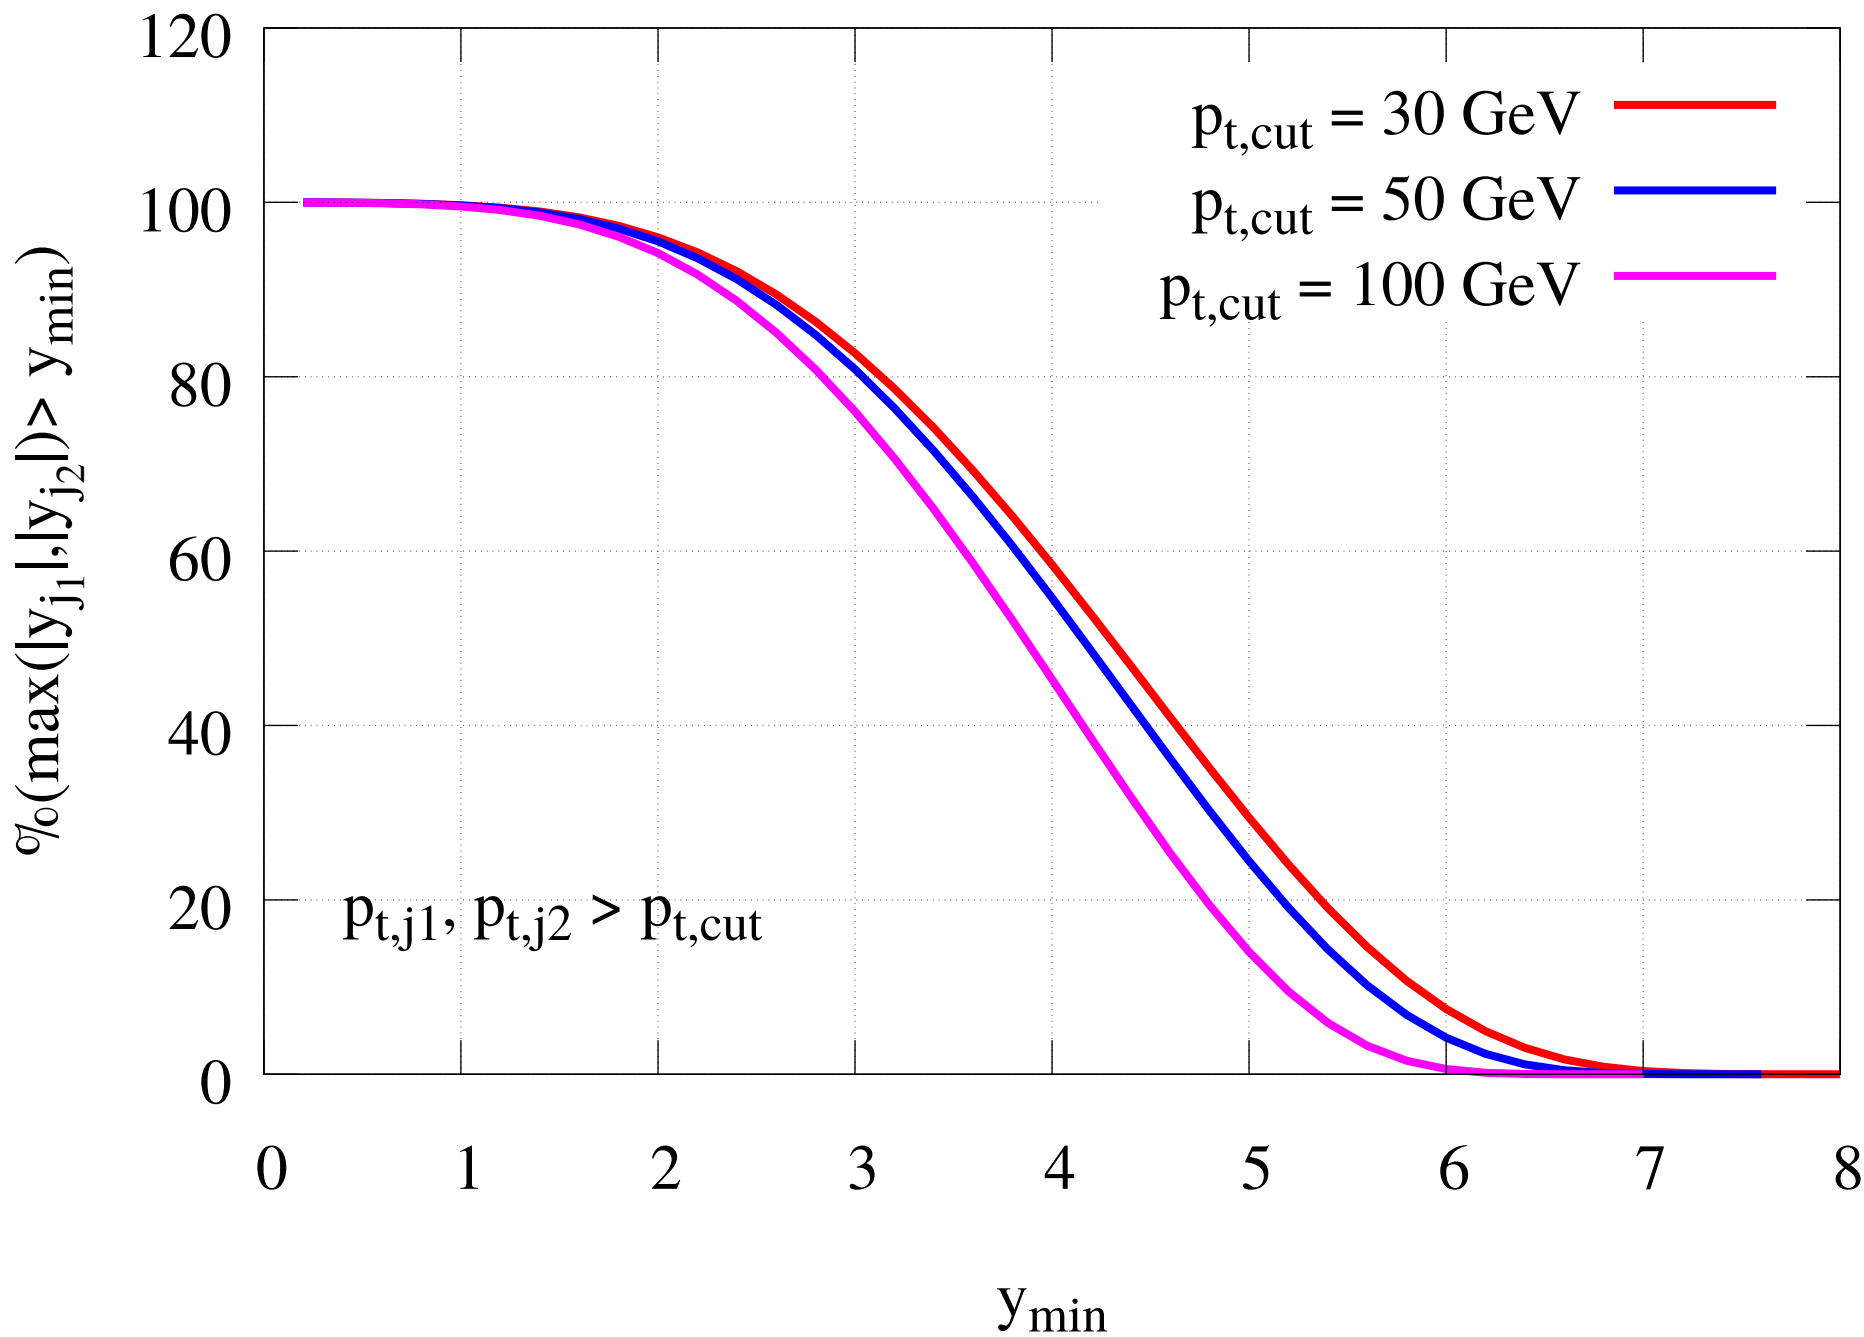

# VBFH 100TeV

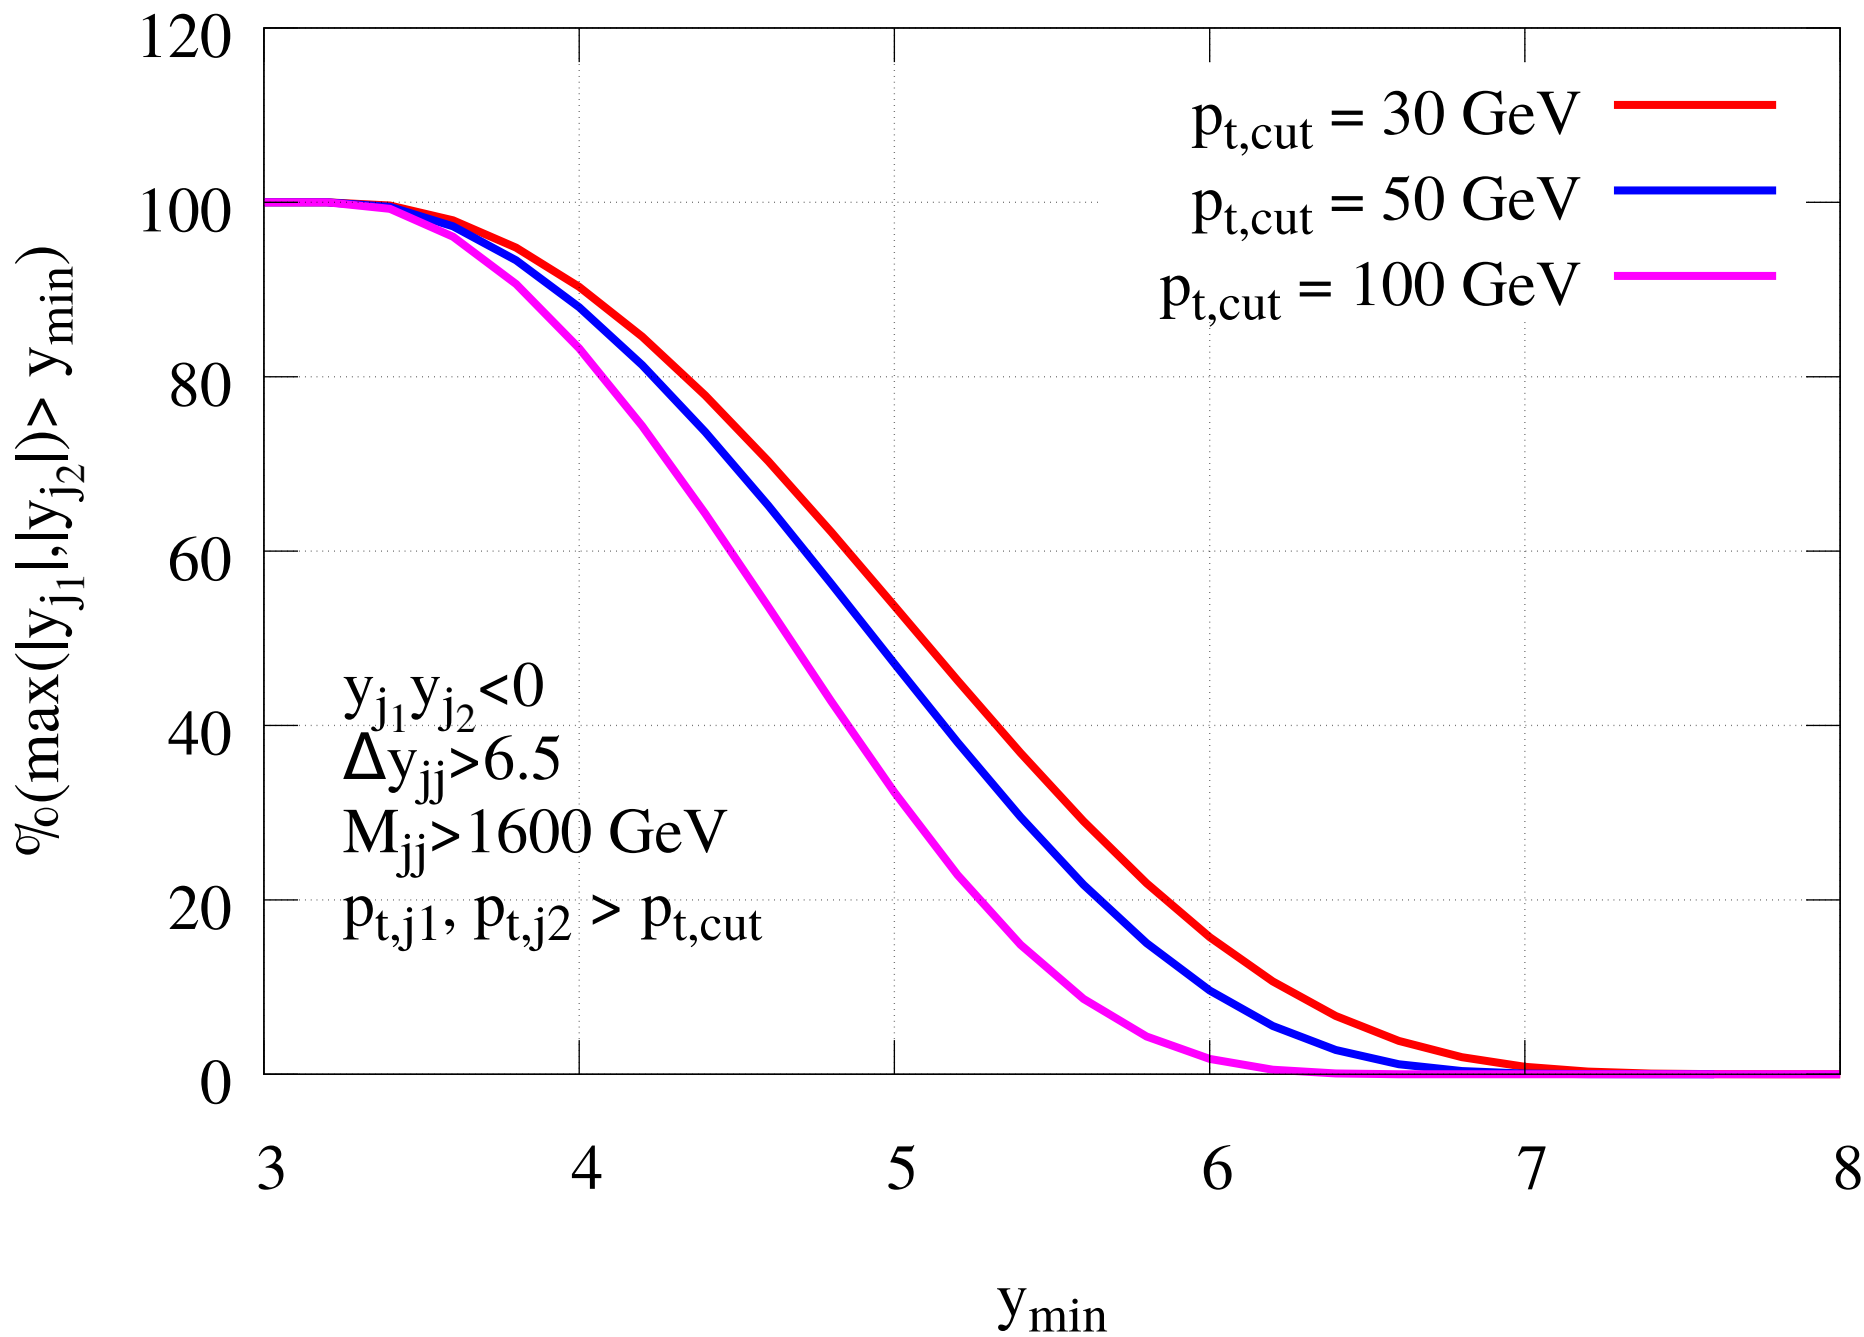

# VBFH 100TeV

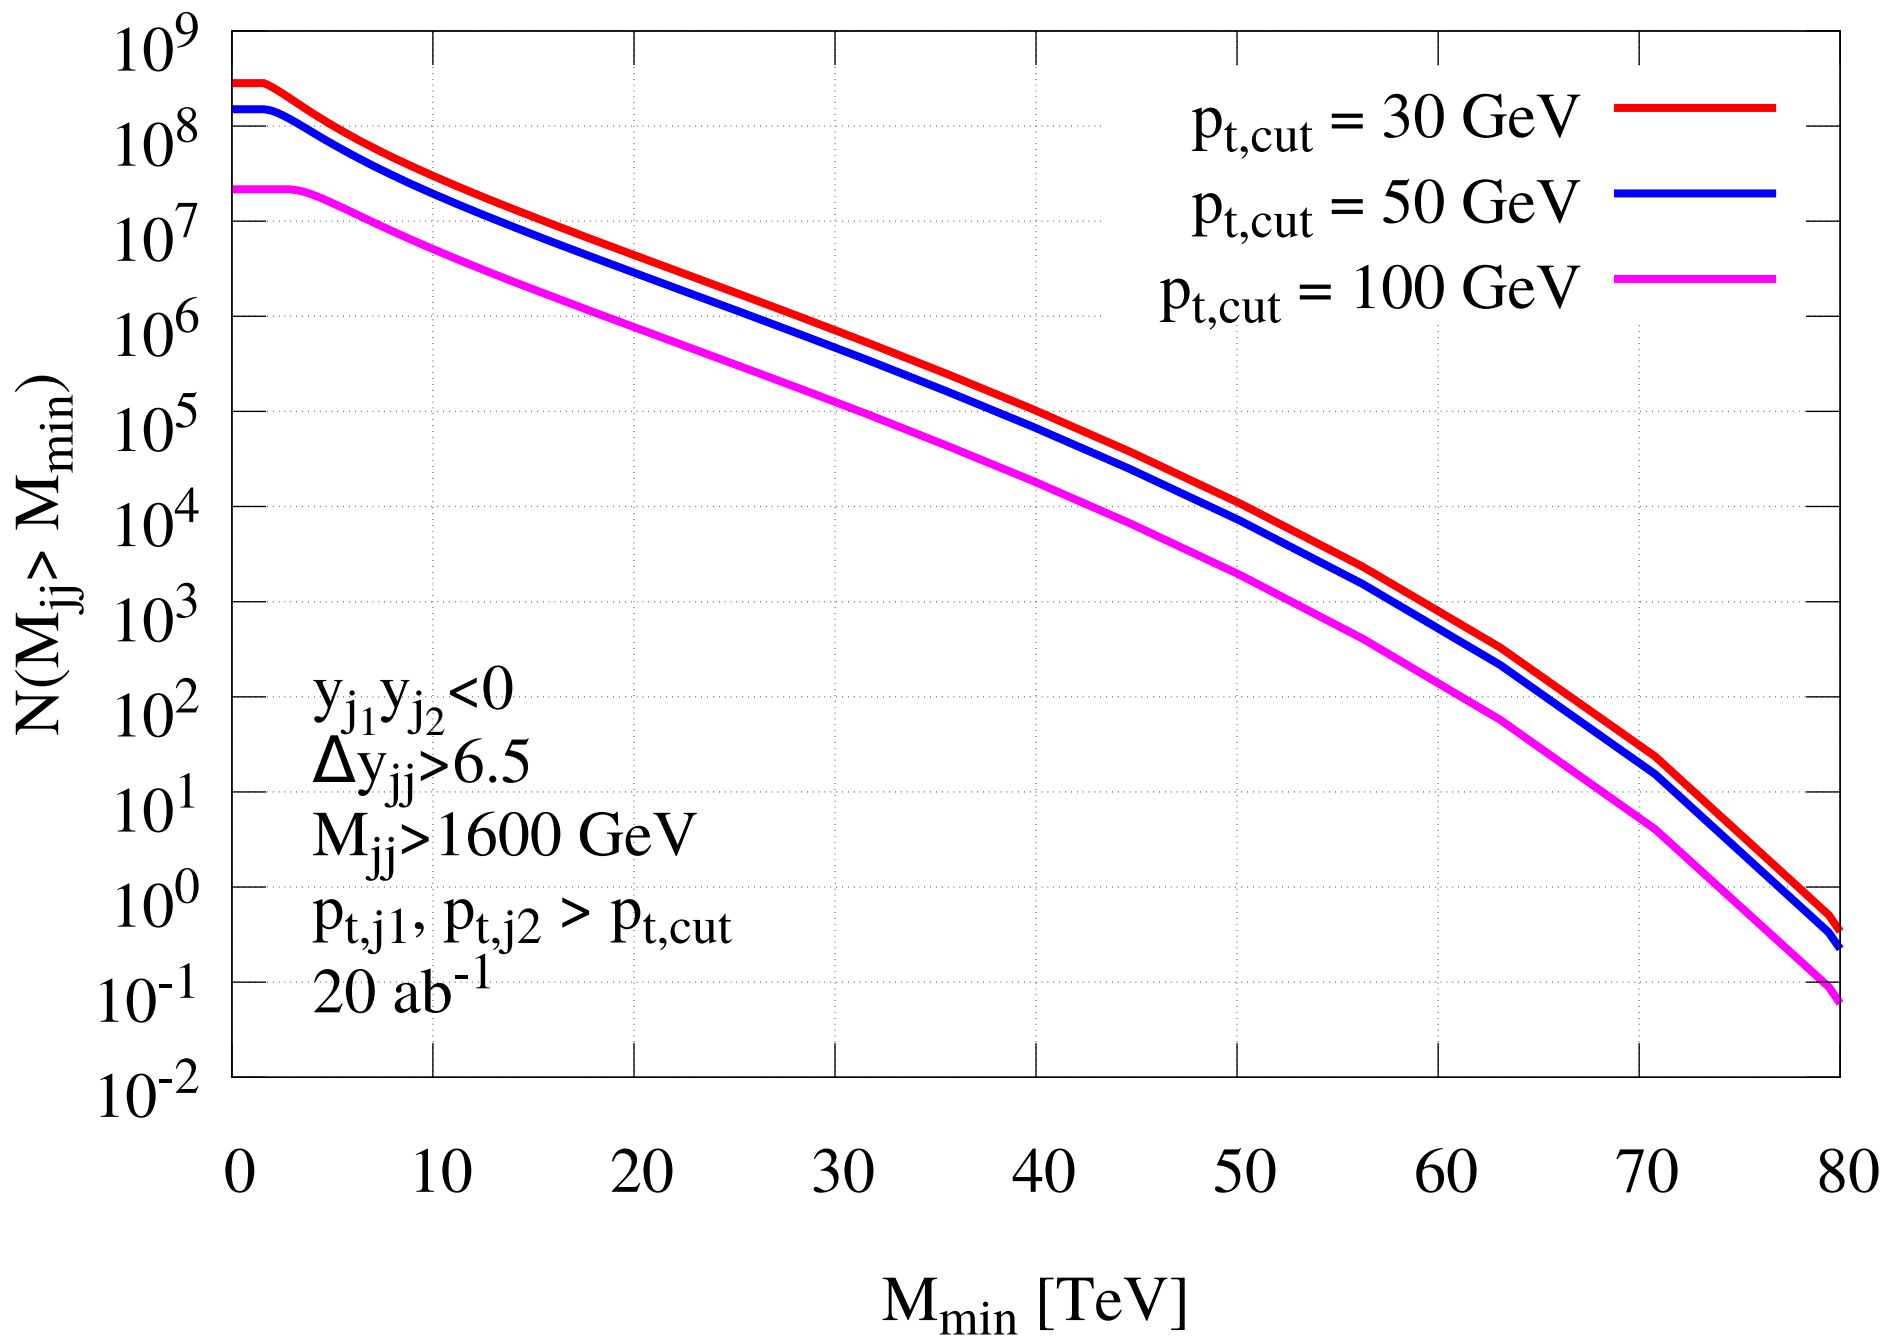

# VBFH 100TeV

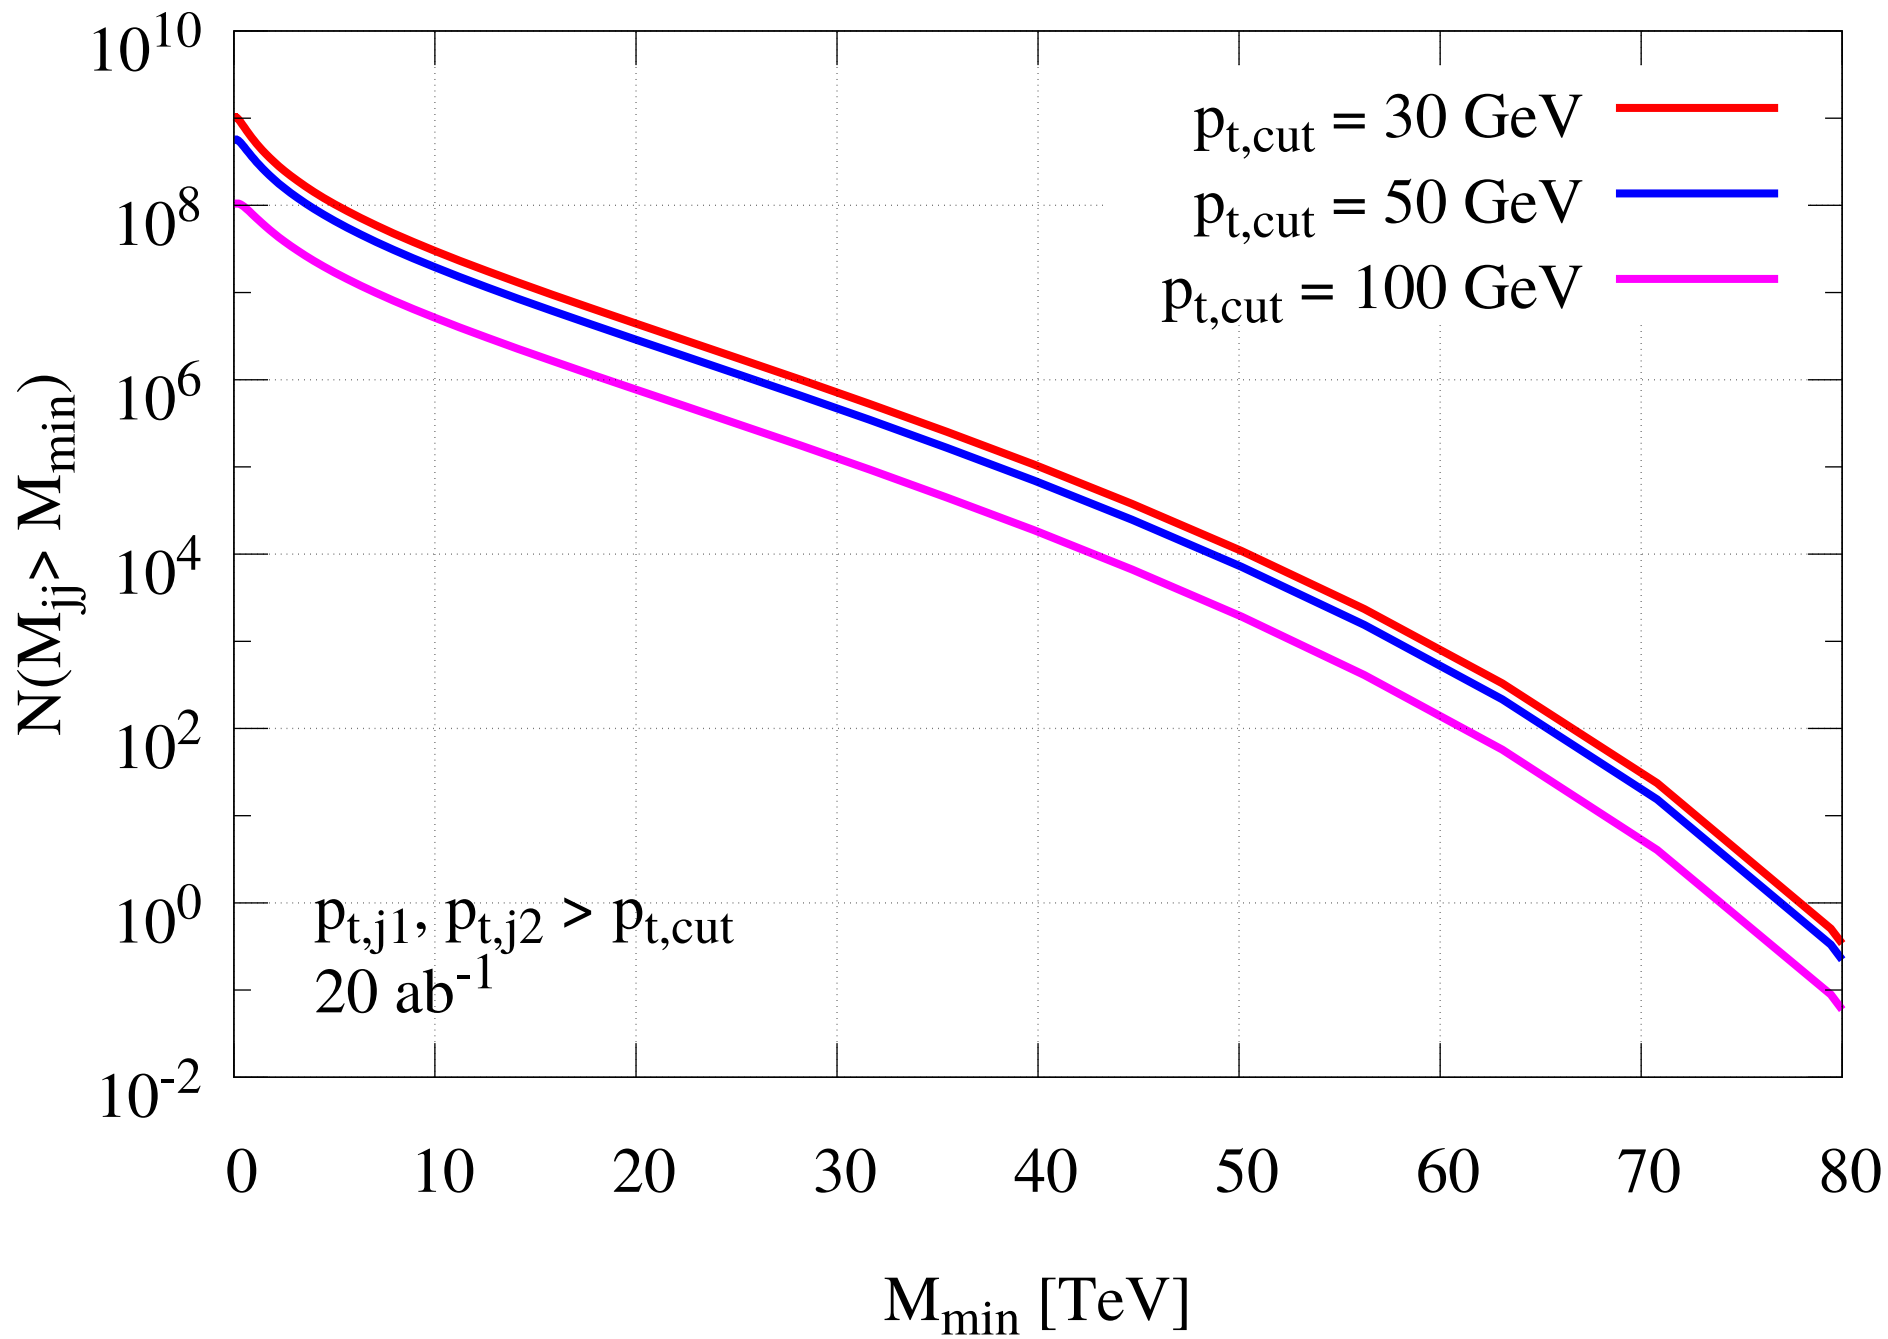

# VBFH 100TeV

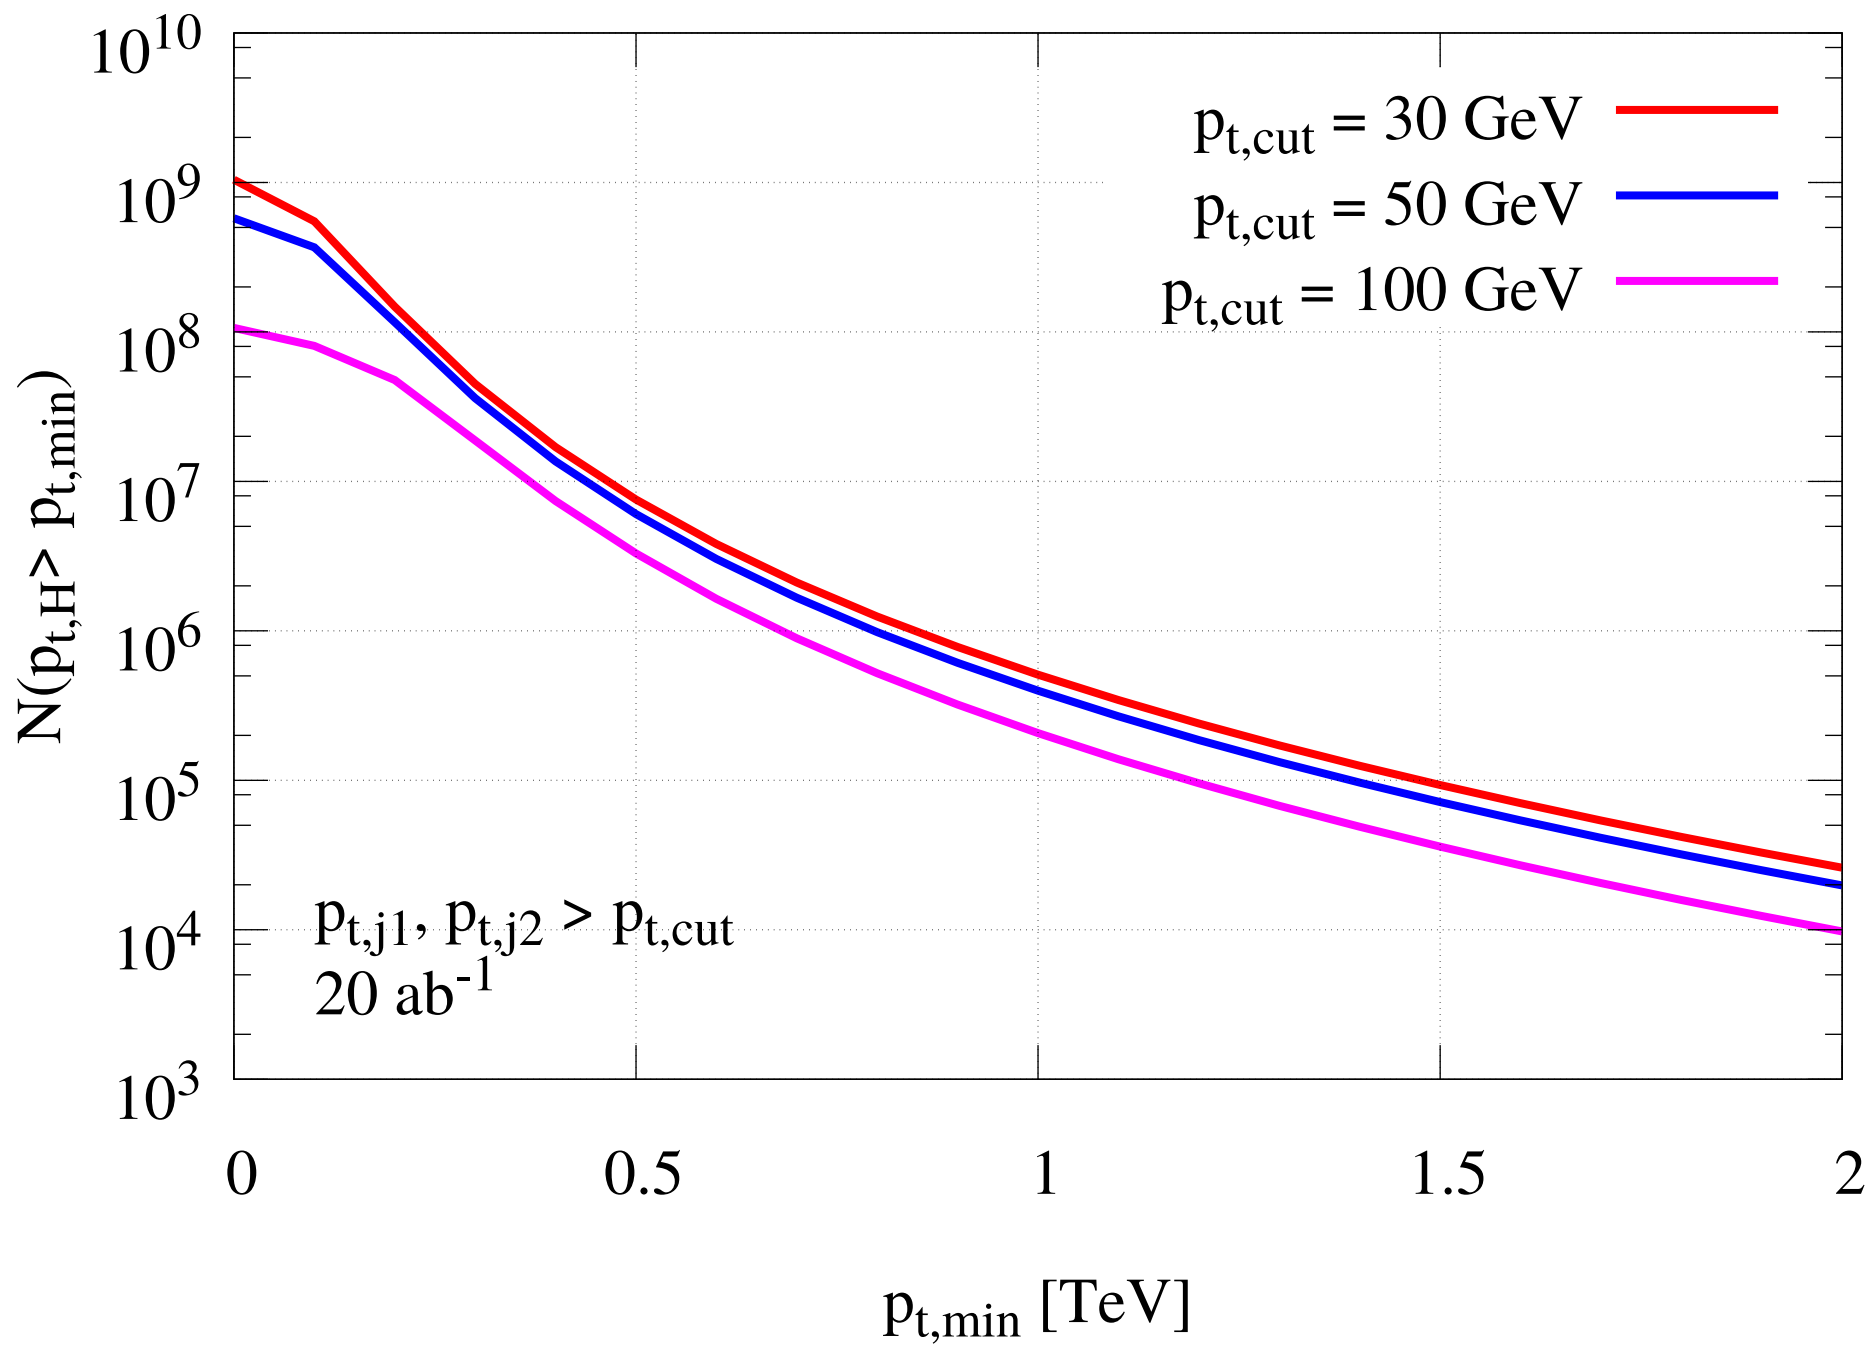

# VBFH 100TeV

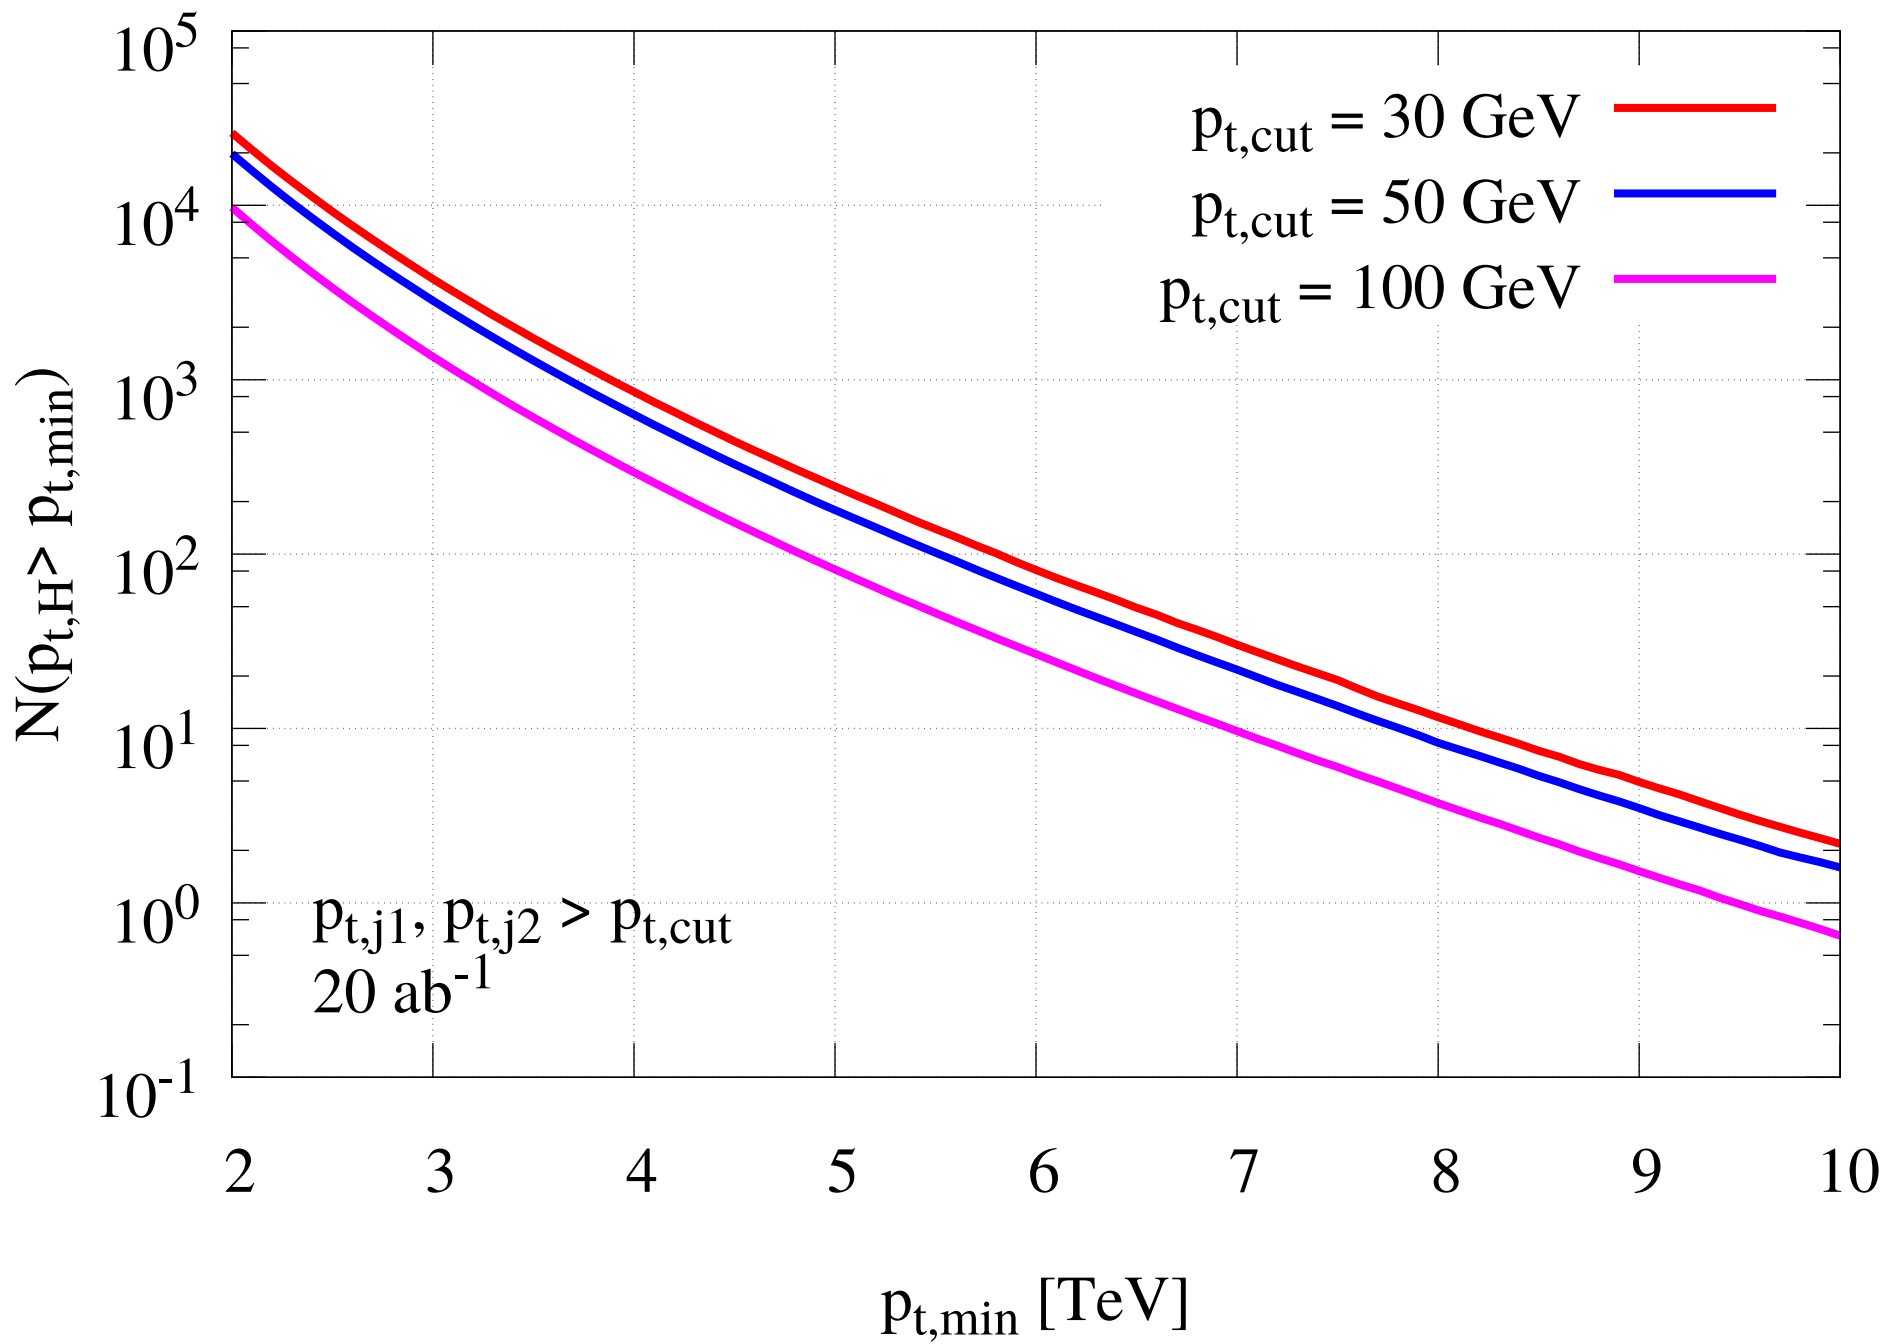

# VBFH 100TeV

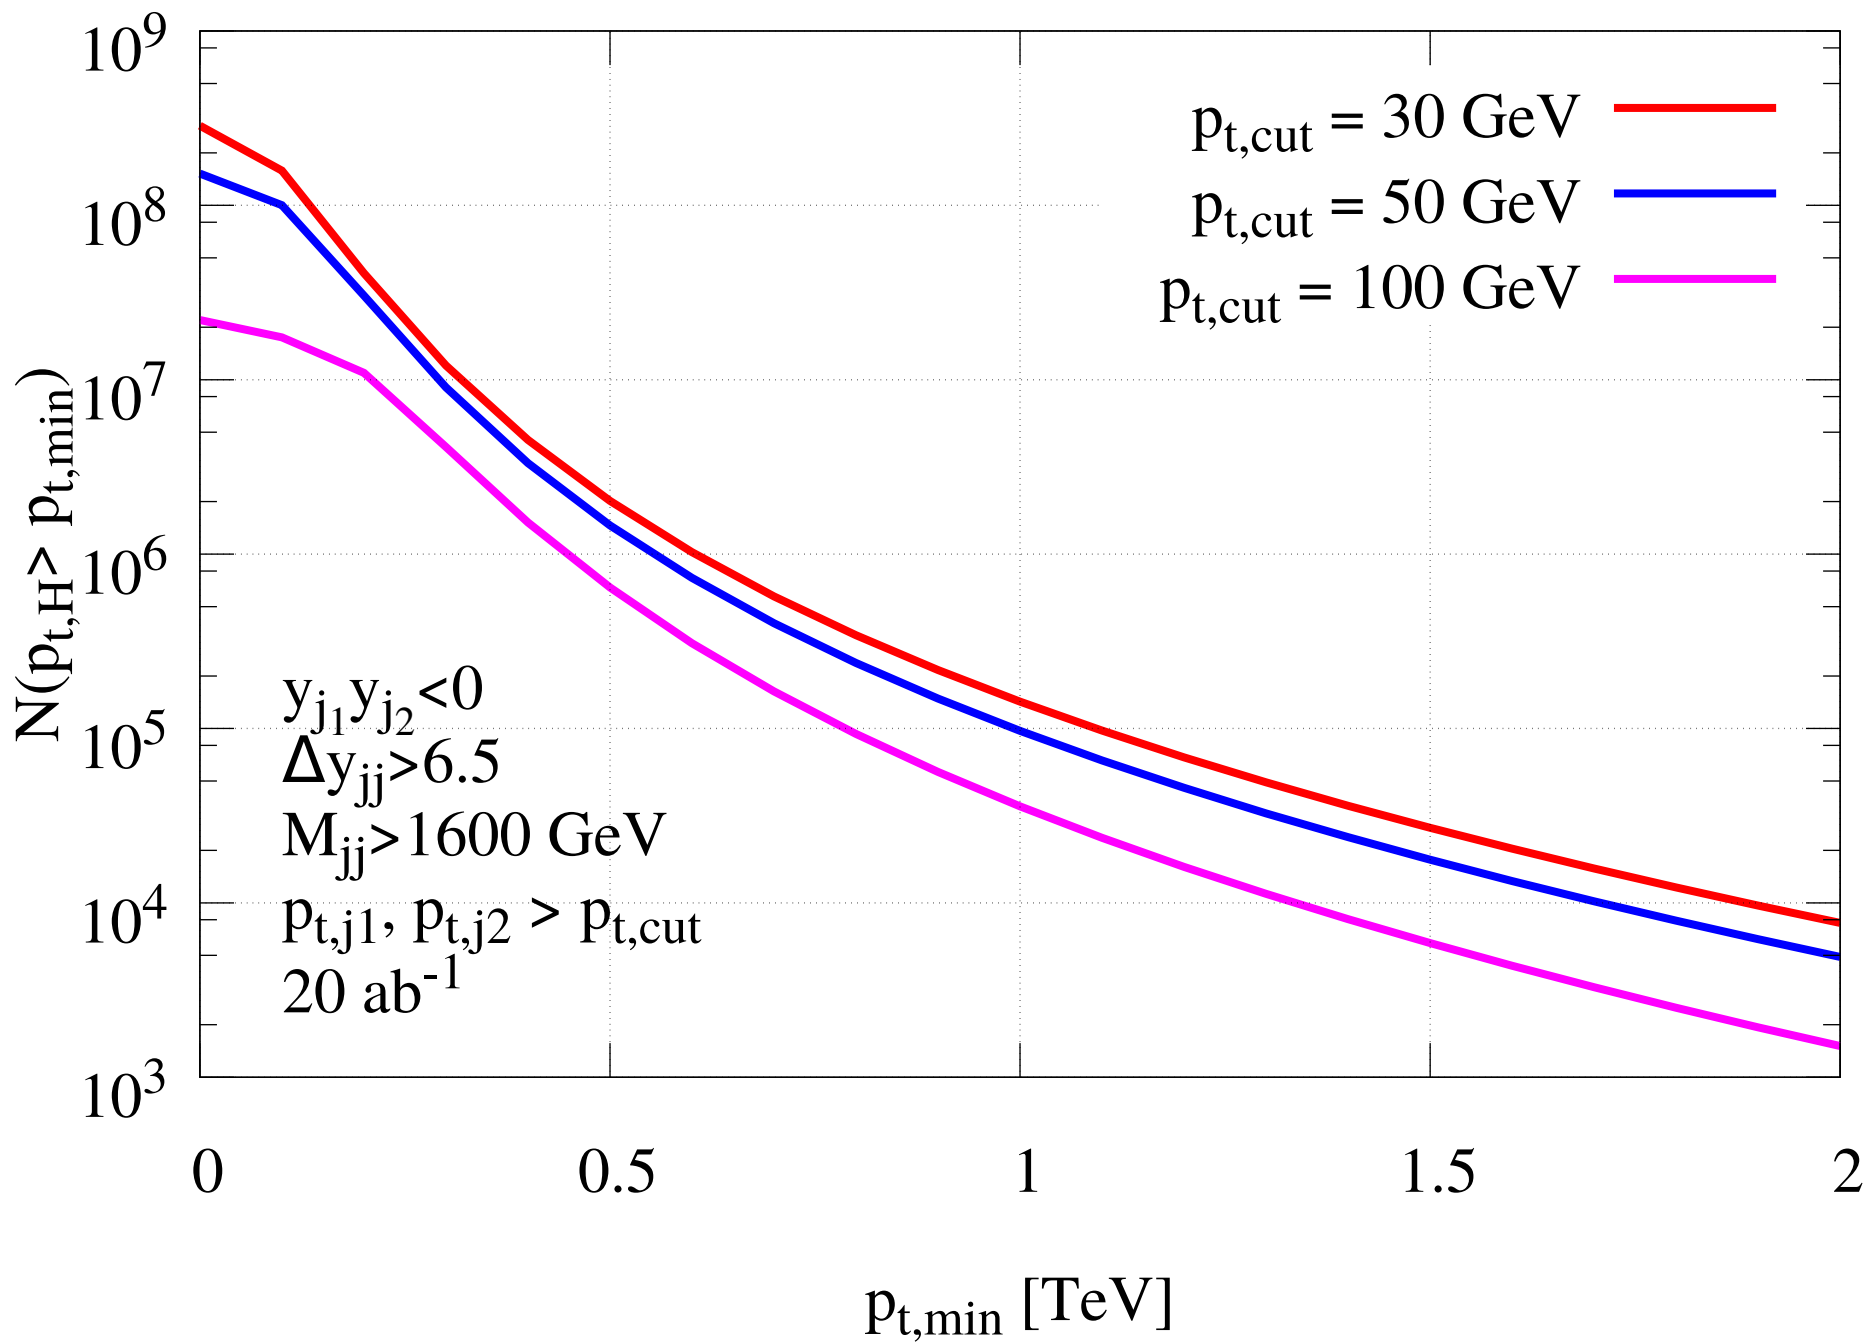

# VBFH 100TeV

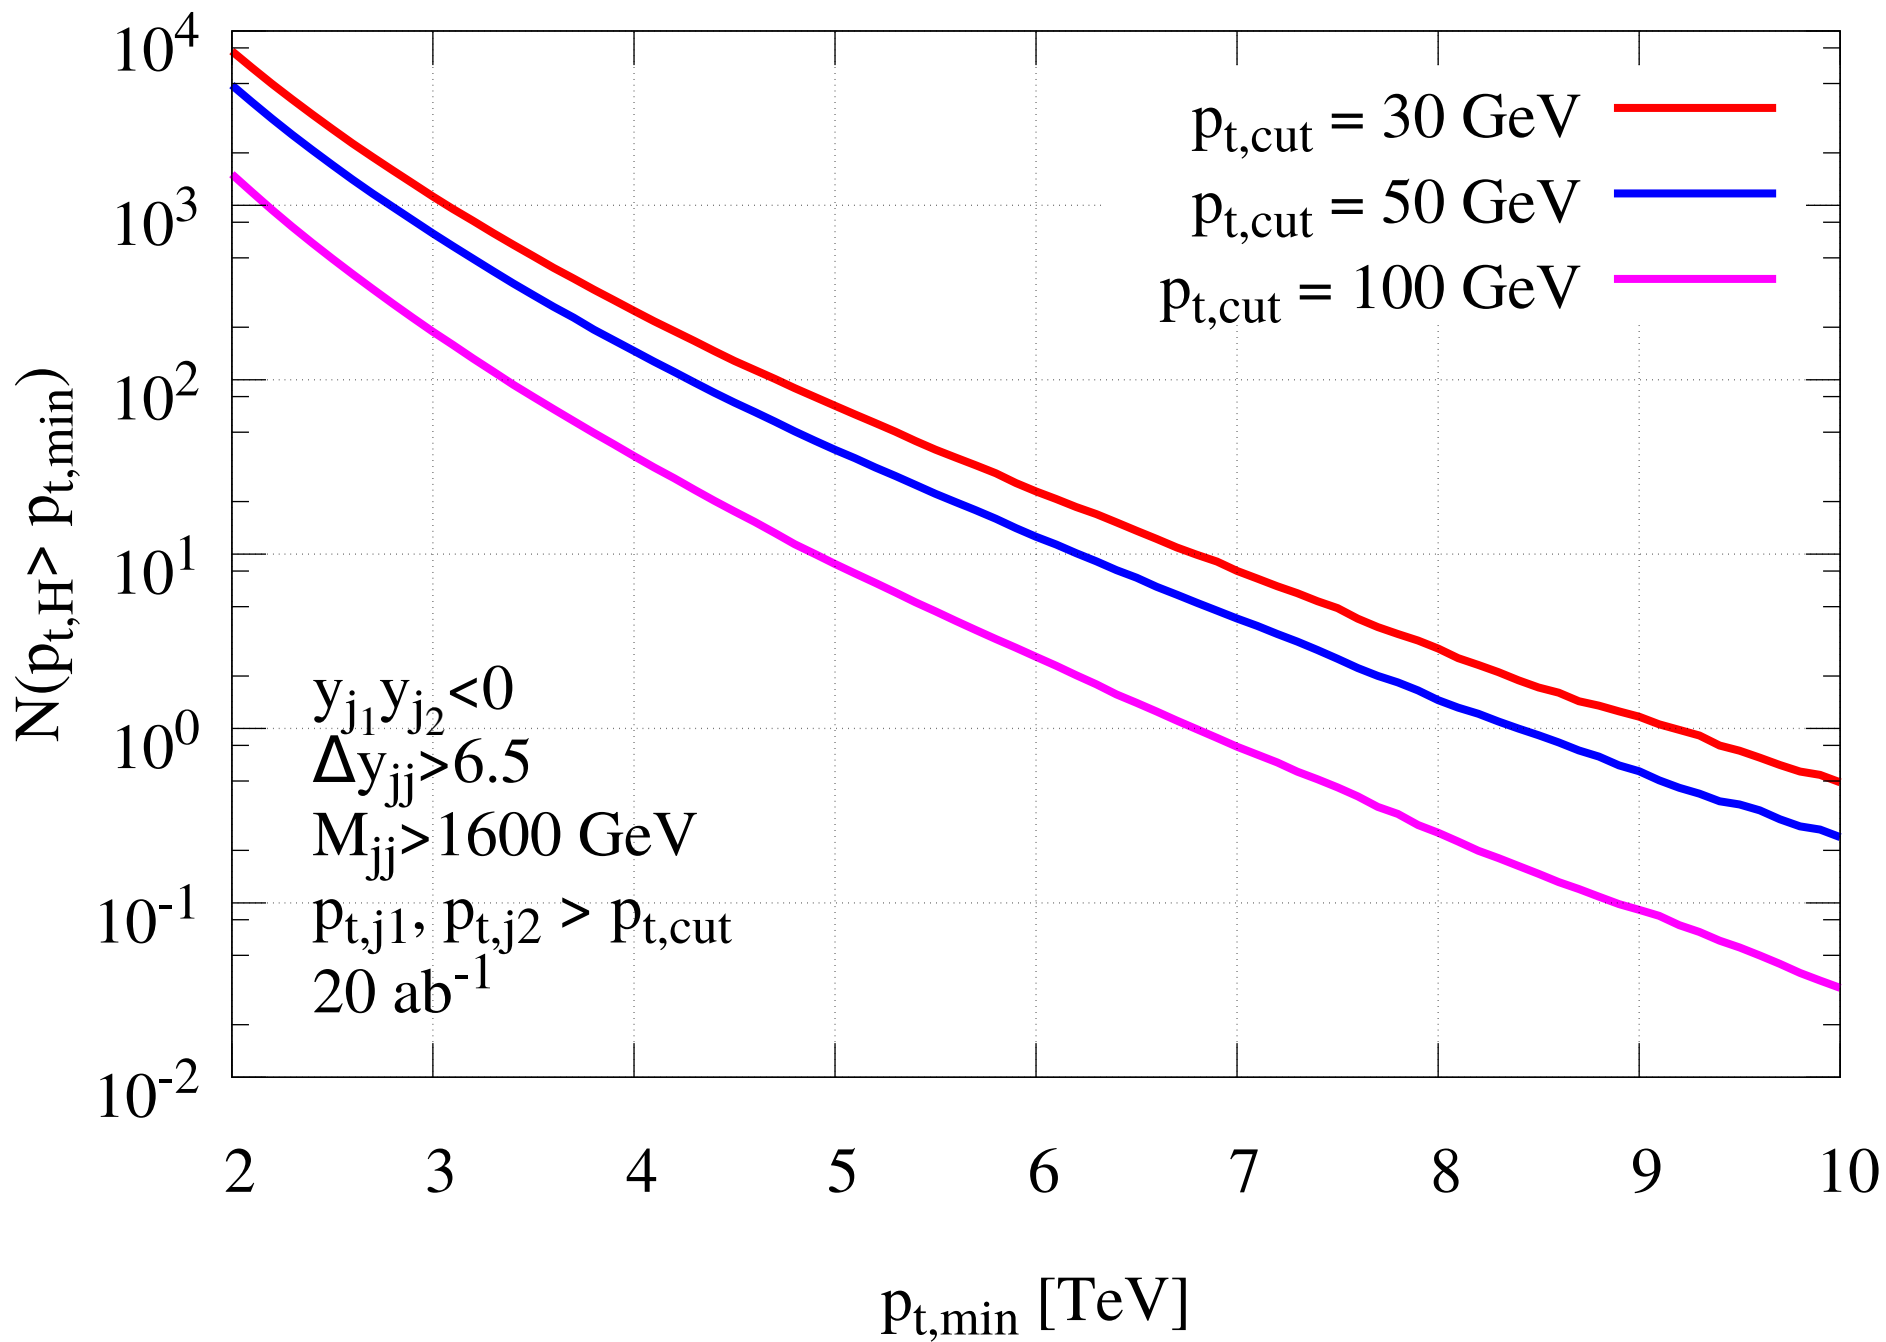



# VBFH 100TeV

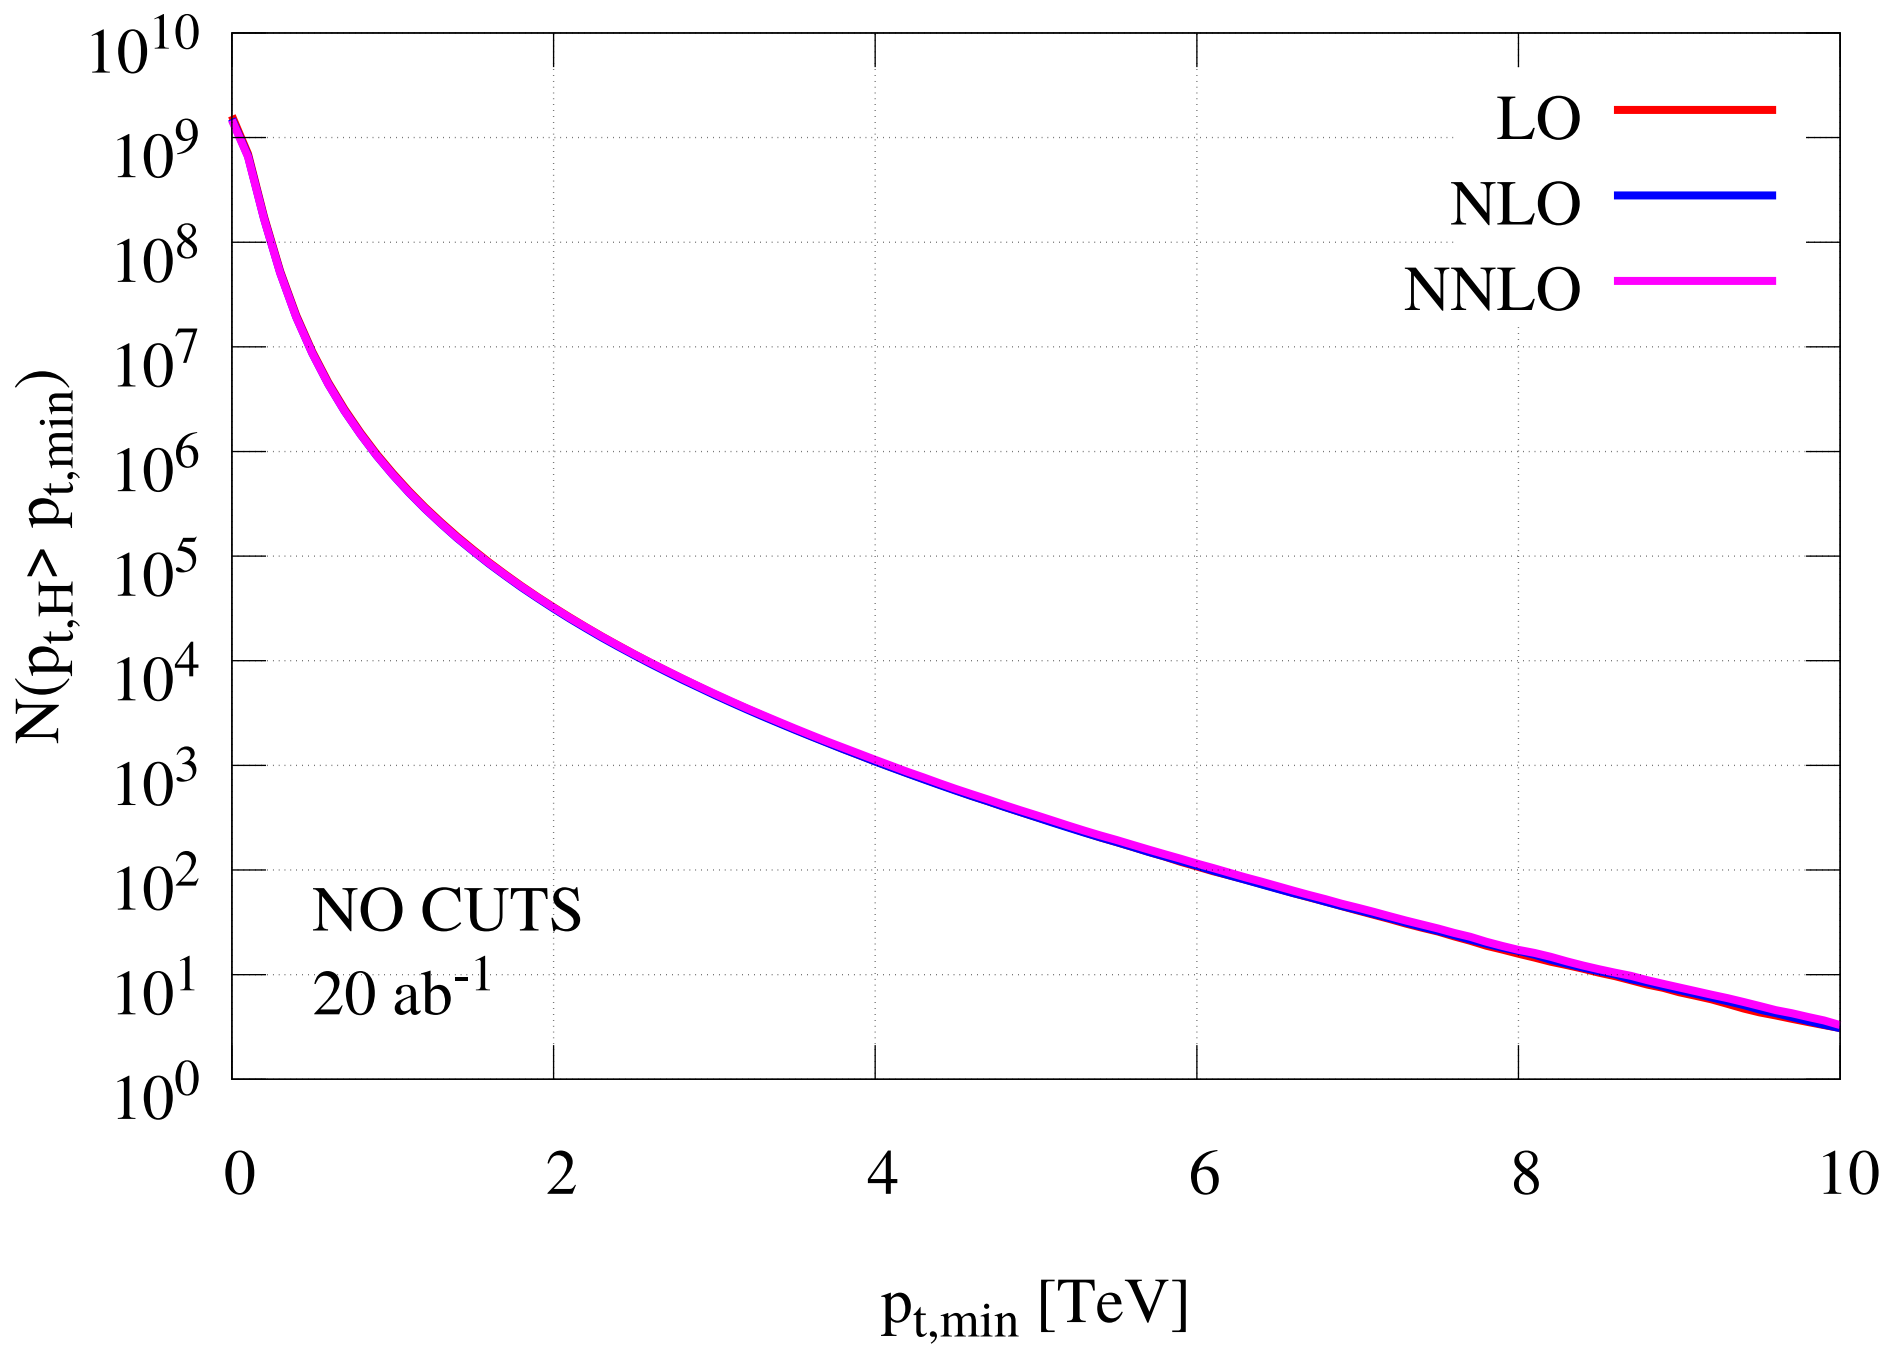

# VBFH 100TeV

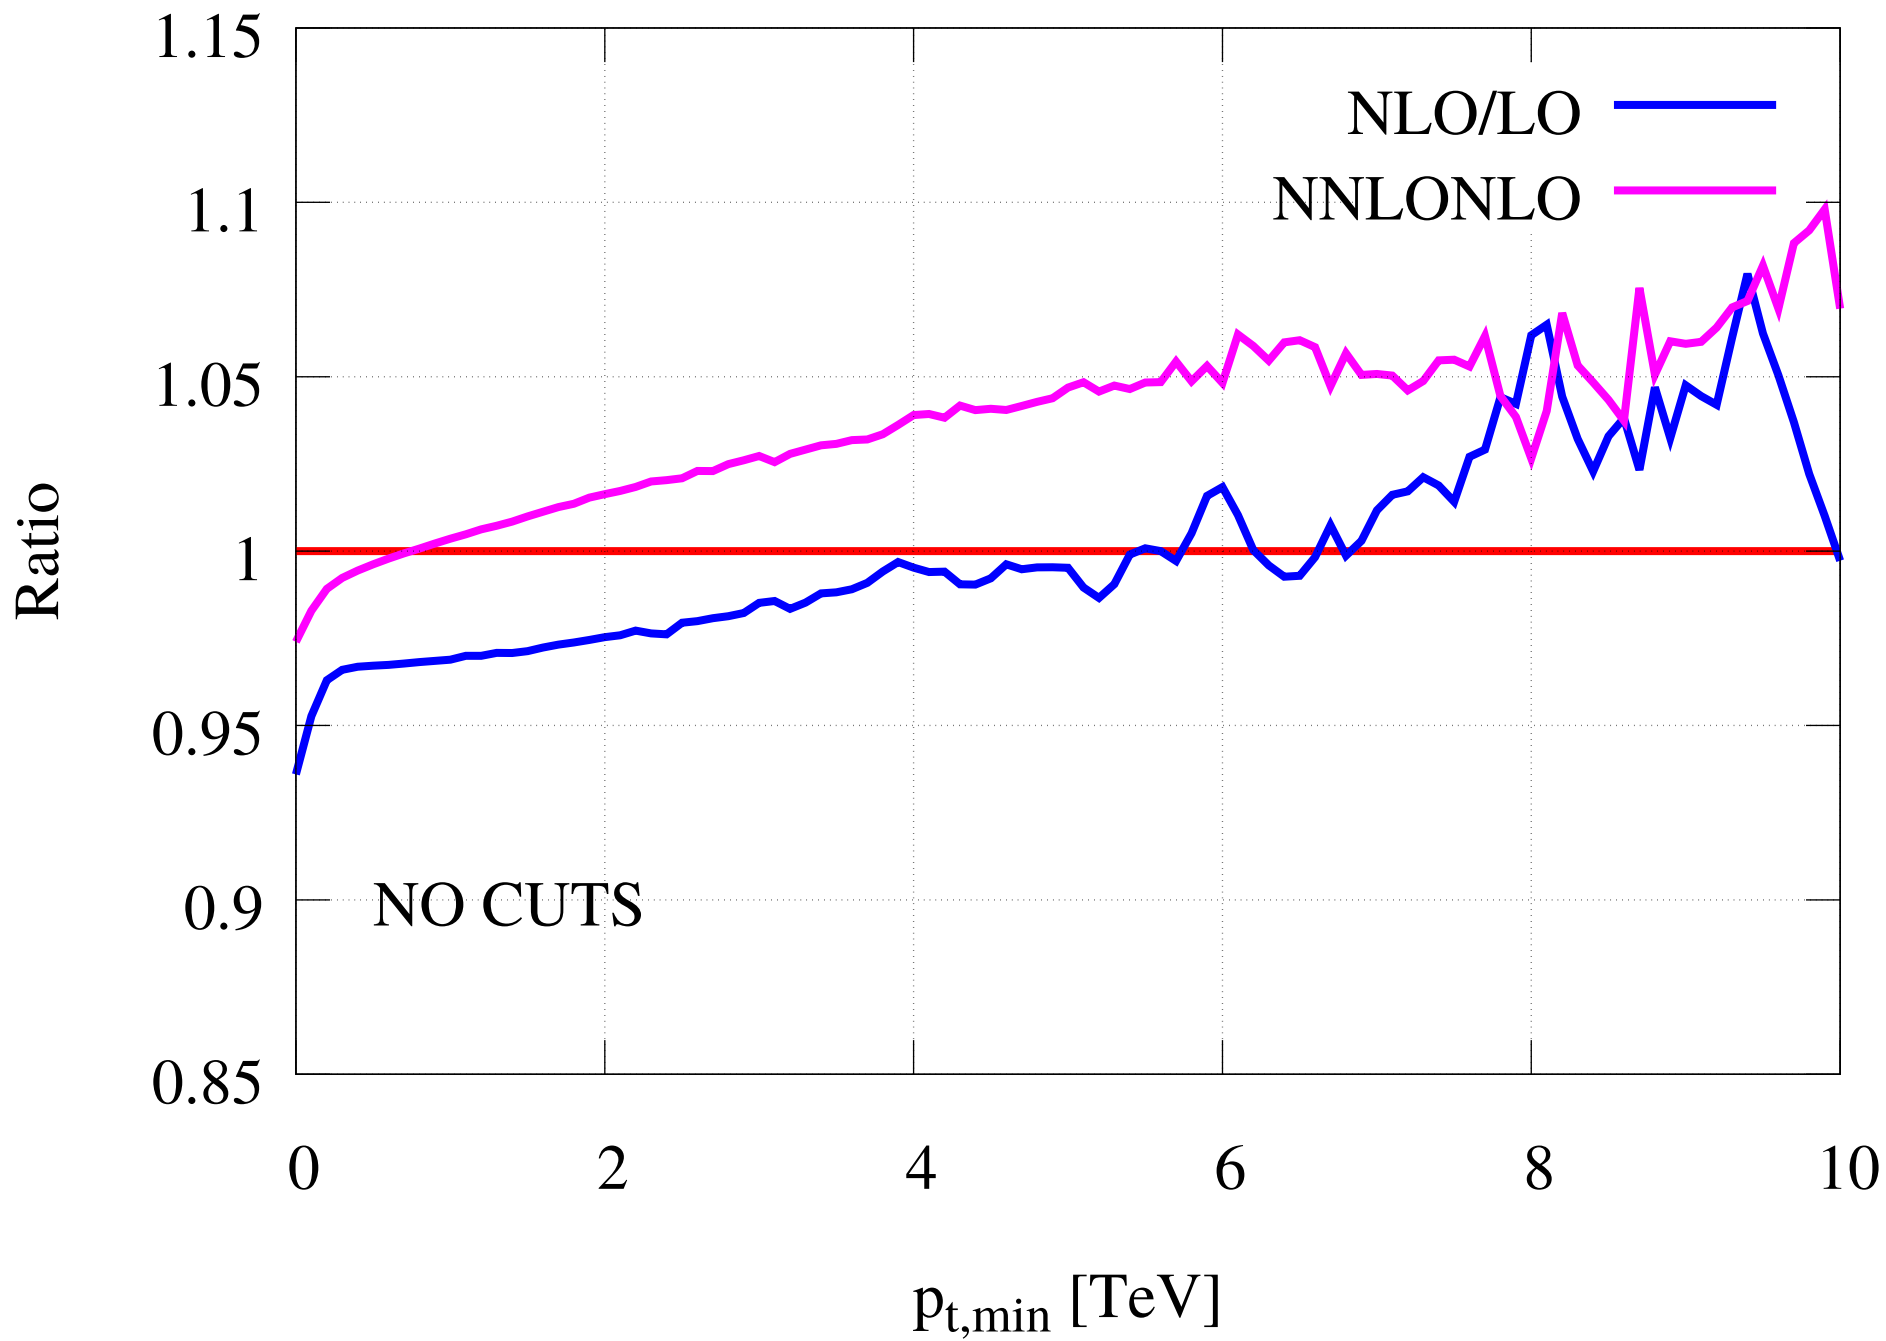

Supplement: Supplementary file 4 [file vbf_100TeV_accumulated.pdf]
