# Supplementary material for: Physics at a 100 TeV pp collider: Higgs and EW symmetry breaking studies
Source: arXiv:1606.09408 source file (2016-06-30)

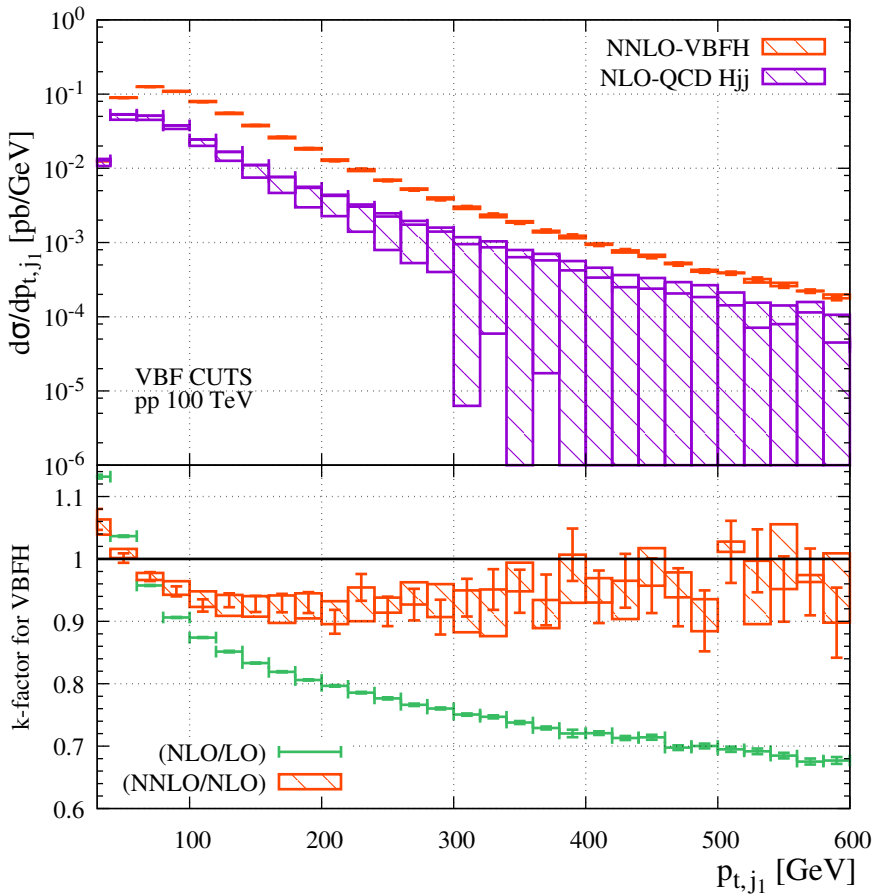

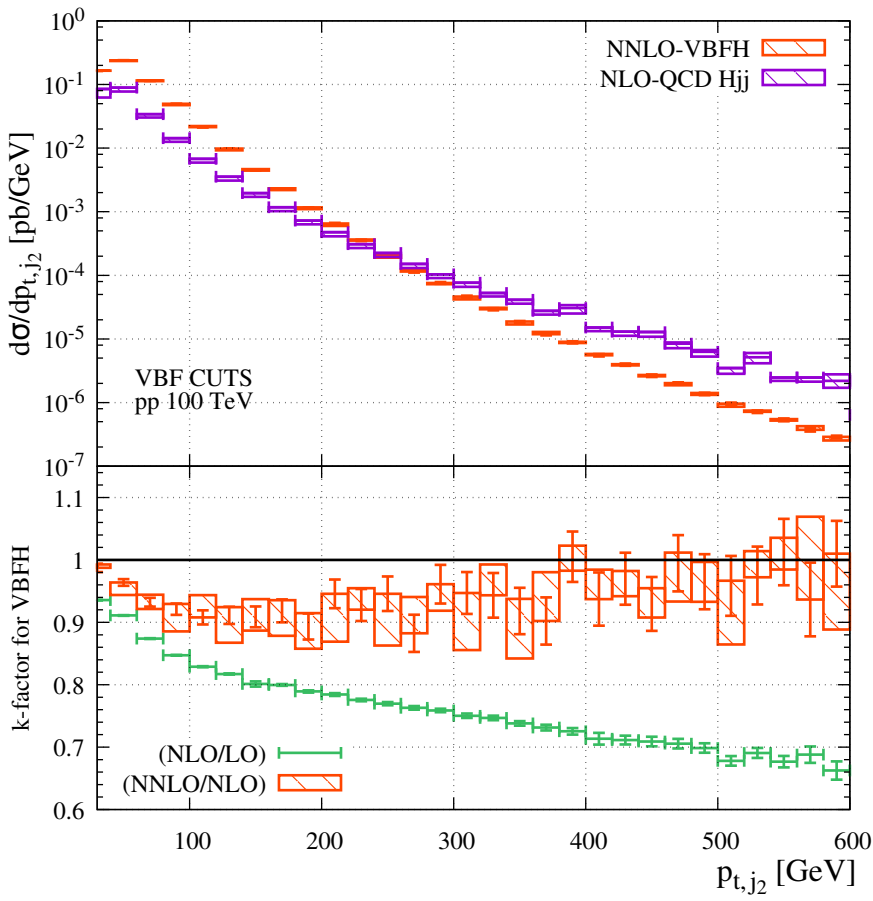

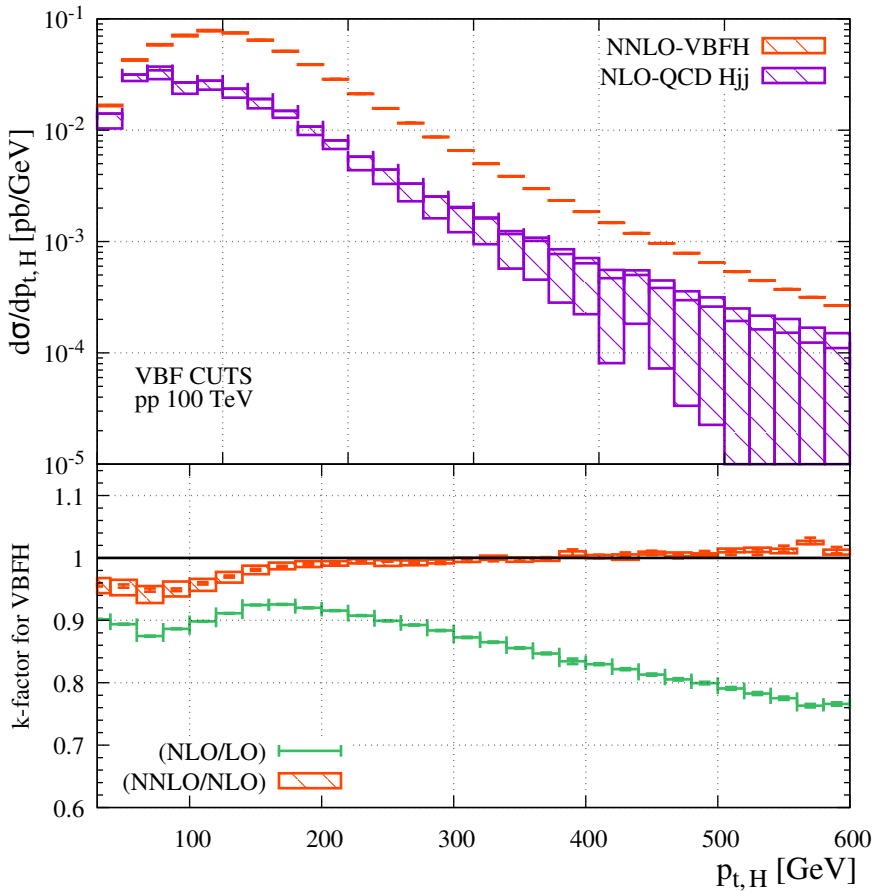

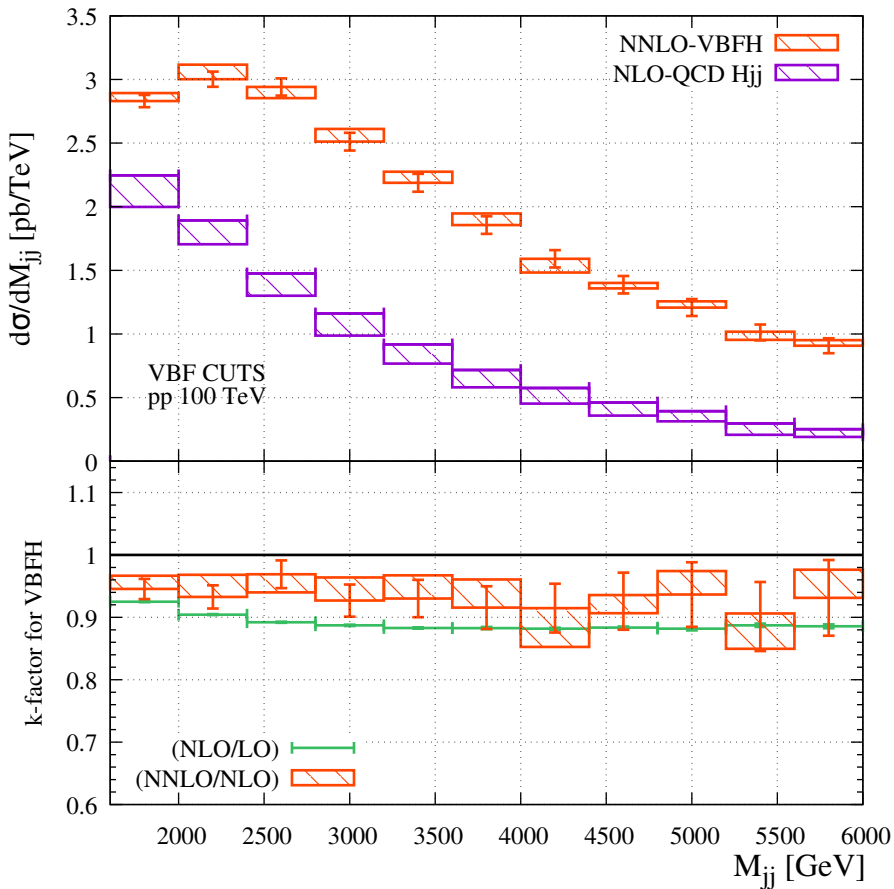

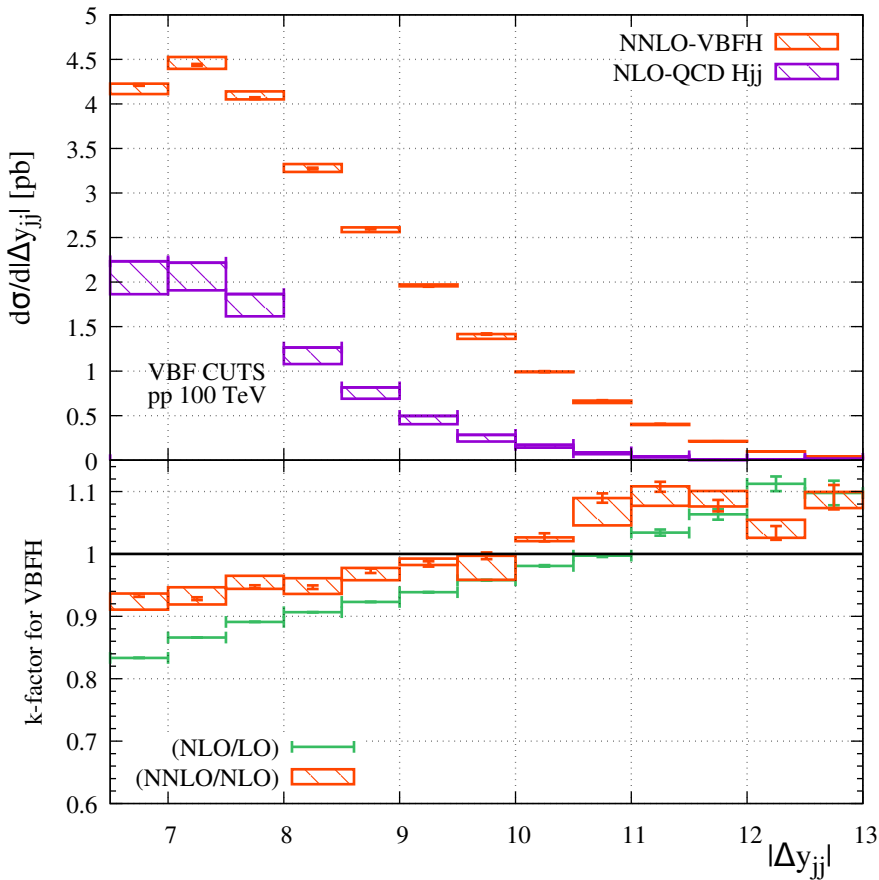

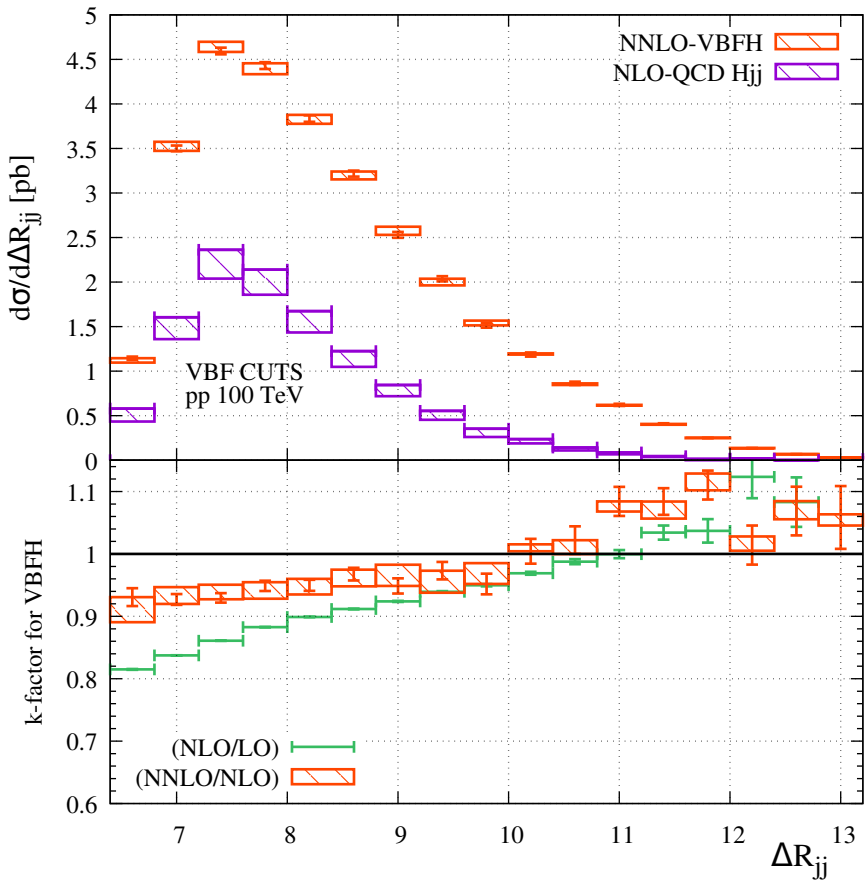

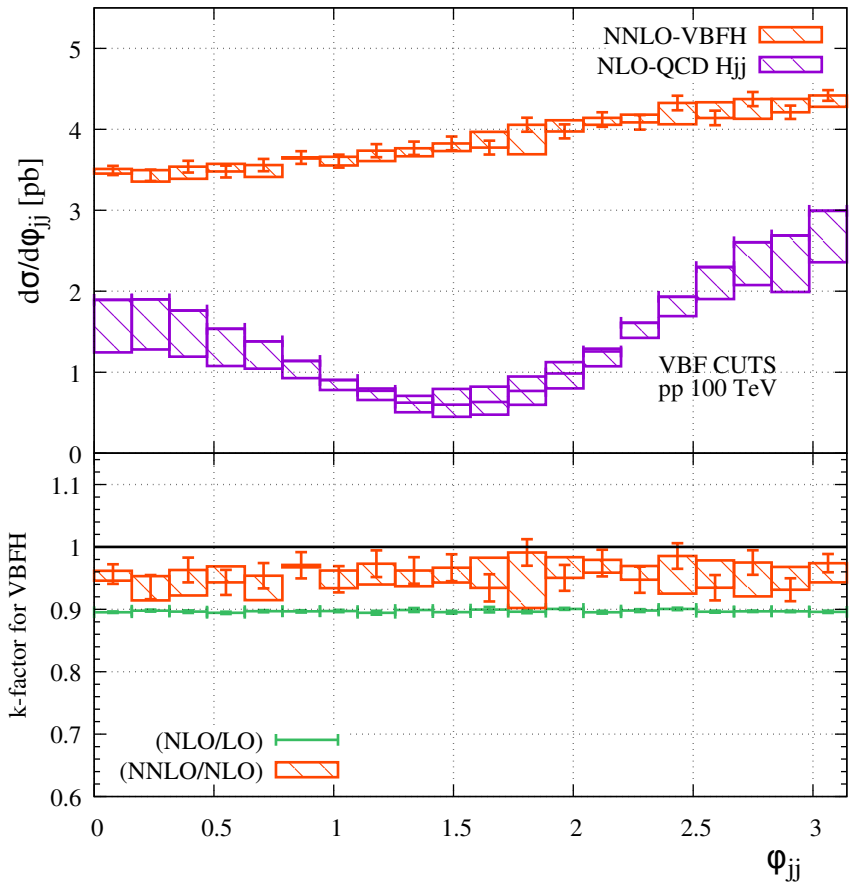

Supplement: Supplementary file 6 [file diff-plots-100TeV-new.pdf]
